# Supplementary material for: Complexity from Adaptive-Symmetries Breaking: Global Minima in the Statistical Mechanics of Deep Neural Networks
Source: arXiv:2201.07934 source file (2022-01-03)
Supplement: Supplementary file 1 [file supplementary_material.pdf]

**SUPPLEMENTARY MATERIAL**

**CONTENTS**


I. Introduction 1
A. Outline 3
1. Statistical-mechanical model of DNN complex system 3
2. Extended symmetry breaking of DNNs 3
3. Problem setting 4
4. Related works 4
B. Notations 5

II. Main results 5
A. Umwelt: system that does statistical inference on hierarchical events 5
1. Boltzmann distribution, disorganized complexity, complex biotic systems and DNNs 5
2. The Umwelt statistical-inference system, and its biological motivation 6
B. Stochastic, or Bayesian-probabilistic-graphical, definition of DNNs 8
C. Self-organization of DNNs 9
1. Ising model and self-organization 9
2. Self-organization of DNNs through a feedback-control loop composed of coarse-grained variable and hierarchical circuits 10
D. Adaptive symmetries in the feedback-control loop 12
1. From conservative-symmetry in physics to adaptive-symmetry in biology 12
2. Circuit symmetry in DNNs 13
3. Statistical assembly methods 15
E. Order from fluctuations, or order from adaptive symmetry 16
1. Order in physics and self-organization 16
2. Order of DNNs 17
F. Plasticity phase, extended symmetry breaking, and benign pathways on the risk landscape 18
1. Phase space in physics 19
2. Hypothesis on a phase of DNNs with stable circuit symmetries 19
3. Symmetry-stability analysis through Hessian 19
4. Coarse-grained effect of circuit symmetries on Hessian entries 20
5. Plasticity phase, extended symmetry breaking, and benigh pathways of DNNs 21
G. Theoretical setting 24

III. Discussion: complexity from adaptive-symmetries breaking 24

References 25

Supplementary Material 35

A. Further related works 35
A. Stochastic DNNs 35
1. Umwelt and stochastic DNNs 36
2. Bayesian Neural Networks 37
B. Circuits of DNNs 38
C. Symmetries of DNNs 38
D. Risk landscape and phase space of DNNs 39
1. Disorder in large DNNs 40
2. Empirical results on risk landscape 41
3. Retrograde DNNs to linear models 42
4. Remold DNNs to statistical fields 42
5. Frustration phase of DNNs 44
6. Phases of DNNs 45

B. Formal results 45
A. Notation and terminologies 45
B. Umwelt: system that does statistical inference on hierarchical events 46
1. Set-theoretical formalism of environment 46
2. The emergence of an Umwelt as a statistical inference problem 47
3. Statistical supervised learning problem, and observed environment 48
4. Umwelt: hierarchical probability measure-coarse-graining system 48
5. Umwelt emergence through hierarchical maximum entropy learning 49
6. Dual problem of maximum entropy problem, and exponential family distributions 50
7. Learning of Umwelt 50
C. Stochastic, or Bayesian-probabilistic-graphical, definition of DNNs 51
1. Conventional functional definition of supervised DNNs 51
2. Hierarchical parameterization of Umwelt 52
3. Forward propagation as approximation inference 52
4. Back propagation maximizes approximate loglikelihood 53
5. Forward and backward propagation is expectation-maximization algorithm 53
6. Stochastic definition of DNNs 54
7. Loglikelihood and surrogate risks 55
8. The restricted class of loss function analyzed in this work 56
D. DNN self-organization through a feedback-control loop composed of coarse-grained variable and hierarchical circuits 56
1. Variational free energy minimization in informational self-organization of DNNs 56
2. Coarse-grained variables computed by DNNs 57
3. Hierarchical circuits in DNNs 58
4. Neuron assemblies, perturbations of basis circuits and derivatives of assemblies in DNNs 59

5. Adaptive feedback-control loop between coarse-grained variables and hierarchical circuits in DNNs 61
E. Adaptive symmetries in the feedback-control loop 62
1. Self-organization in physics: conservative symmetries and their breaking 62
2. Weight symmetries: stochastic, heterogeneous symmetries in DNNs 62
3. Symmetry and scale: stability of circuits 63
4. Circuit symmetry: composite adaptive symmetry from weight symmetry 63
5. Circuit-symmetry breaking in the feedback-control loop 65
6. Hypothesis: self-organizing of DNNs as an extended symmetry-breaking process with stable macroscopic adaptive symmetries 66
F. Order from fluctuations, or order from adaptive symmetry 68
1. Order and plasticity order parameter of DNNs 68
2. Experimental study on the order of DNNs: nonzero order parameter and symmetry of gradients 69
G. Plasticity phase and benign pathways on the risk landscape 70
1. Perturbations of basis circuits of order two that compute Hessian 70
2. Coarse-grained effect of circuit symmetry on Hessian entries 70
3. Control parameters, and assembly assumptions of DNNs 71
4. Symmetry of Hessian eigenspectrum, or plasticity phase theorem of DNNs 73
5. Benign pathways to zero-risk attractors on the risk landscape of DNNs 73
6. Experimental validation of the assembly-symmetry assumption, and symmetric distributions of Hessian entries 74
7. Experimental validation of the assembly-diversity assumption 75
8. Plasticity phase of DNNs 76
H. Formal version of the plasticity phase theorem 77
1. High-dimensional-probability analysis of the random Hessian matrix with correlations 77
2. Assembly-diversity assumption 78
3. Regularity assumptions 79
4. Preliminary definitions 80
5. The plasticity phase theorem 81

C. Extended discussion: complexity from adaptive-symmetries breaking 82
A. From spin glasses to DNNs by increasing potential complexity 82
1. Symmetry breaking and spin glass phase of spin glasses 82
2. Spin glasses to DNNs by increasing potential complexity 83
B. Extended criticality of DNNs 84
1. From criticality in physics to extended criticality in biology 84
2. Edge of chaos and extended criticality of DNNs 85
3. Experimental support for the extended criticality and edge-of-chaos phenomenon of DNNs 85
C. Extended phase transition of DNNs 88
1. Frustration phase of DNNs 88
2. Extended phase transitions between plasticty phase and frustraion phase 89
D. Complexity from adaptive-symmetries breaking 90

D. Epistemology and methodology, from disorganized complexity to organized complexity 91
A. From conservative-symmetry breaking to adaptive-symmetry breaking 91
B. From coarse-graining of conservative-symmetry to coarse-graining of adaptive-symmetries in feedback-control loop composed by hierarchical circuits 92
C. Definition of phase and order parameter through symmetries 93
1. Phase and phase space 93
2. Elementary excitation and order parameter 94
D. From symmetries to assumptions and control parameters 95
E. Hessian analysis on stability of symmetries and on local geometry of potential function landscape 96
F. From singular criticality to extended criticality 96
1. Criticality and timescale of symmetry breaking 96
2. Edge of chaos and extended criticality 97

E. Proofs of properties of circuits 98
A. Proofs of properties of circuit calculus 98
B. Proofs of circuit symmetry and broken circuit symmetry of basis circuits 99
1. Proof of circuit symmetry 99
2. Proof of broken circuit symmetry 102

F. Review of results from random matrix theory 104
A. Preliminaries 104
1. Cumulants 104
2. Matrix Dyson Equation 105
3. Cumulant norms 106
B. Eigenspectrum of symmetric random matrices with sparse dependency 107

G. Technical supplements of the plasticity phase 107
A. Problem decomposition 107
1. Decomposition of Hessian 107
2. Speculation on the proof of the general setting 108
3. Rationale of the restriction of the problem 108
B. Proof of plasticity phase theorem and its corollary 108

1. Hessian of a DNN is a large random matrix 108
2. Symmetry in Matrix Dyson Equation 109
3. Proofs of the plasticity phase 110

H. Experiment setting 111
A. Experiment details of the eigenspectrum computation 111
B. Model, training protocols and dataset 111

I. Bootstrapping methods in experiments 112
A. Boostrapping sampling of Hessian entries 112
B. Bootstrapping estimation of non-zero cumulants 113
1. Statistics/cumulants in the experiments 113
2. Bootstrapping estimation of non-zero cumulants 113
3. Hypothesis test on correlations through bootstrapping 113
C. Experiment settings 115
1. Parameters in the bootstrapping algorithms 115
2. Thresholds of hypothesis tests 116

# A. FURTHER RELATED WORKS

## A. Stochastic DNNs

Instead of only learning a blackbox function approximator as a deterministic DNN, a stochastic DNN is probabilistic graphical model that learns a complex probabilistic distribution specified by a multi-layer graph of random variables. The available of a probability distribution has the potential benefits of improved generalization, interpretability, and uncertainty quantification. However, the learning of such networks is NP-hard, and approximate methods are needed, which introduces trade-offs that make the networks less practical, and not deliver the potential benefits. As a result, it is not the mainstream techniques compared with supervised deterministic DNNs.

As introduced in section II B, the stochastic definition of DNNs in this work interprets existing deterministic DNNs (i.e., supervised DNN with ReLU activation funtion) as a multi-layer Bayesian probabilistic graphical model, thus synthesizes the deterministic and stochastic DNNs, and could potentially enjoy the benefits of both approaches.

However, the investigation of the benefit of stochasticity is not the focus of this work. The stochastic definition is proposed such that the hierarchical interaction of neurons could be analyzed statistically as an organized complex system in a way that is a counterpart to the statistical mechanics of disorganized complex system. Thus, this stochastic definition should be appreciated as a contribution that addresses the analytical difficulties of existing DNNs (i.e., higher-order Boltzmann machines and supervised DNNs), more specifically, through the circuit formalism, circuit symmetry, and statistical assembly method introduced in this work, and thus enables the study of the symmetry-breaking in DNNs training.

Therefore, in this related-works discussion, we would not compare the stochastic definition with other types of stochastic DNNs, in term of properties such as generalization, uncertainty quantification, etc, but focus on difference in the models and training algorithms. More specifically, in supp. A A 1, we shall discuss related works of the stochastic definition in the general context of stochastic DNNs; and in supp. A A 2, we shall discuss the definition in the specific context of Bayesian DNNs.

### 1. *Umwelt and stochastic DNNs*

From a model perspective, (feedforward) stochastic DNNs are simple and neat: they are just factorized probabilities where the high-dimensional joint probabilities are factorized into multiplication of probabilities according to the statistical dependence of the random variables in the networks. However, except for cases where the random variables at higher layer are of conjugate distributions with the variables at lower layers—that is, variables at lower layers are conjugate priors of the ones at the higher layer—such as Gaussian distributions, the inference and learning of such networks are NP-hard and thus intractable. Therefore, approximation methods are needed for inference and learning, which introduce complications. In a broad stroke, two types of approximation methods are available: variational inference and Monte Carlo (MC) sampling [96]. Variational inference approximates intractable distributions with the simple ones mentioned previously, such as Gaussian distribution, while MC sampling approximates distributions by, as the name suggests, by MC sampling.

Because the complications mostly lie in designing approximation methods, most works focus on designing better approximation methods that, for example, reducing bias and variance of the variational approximation [153], exploration of variational schemes [154–156], better computational tractability [154, 155], or more efficient MC sampling [157]. Yet, our stochastic definition is designed for a relatively orthogonal purpose, and could be appreciated as improving the model: it is a continuation of model design and a synthesis of deterministic and stochastic DNNs in the sense that the definition is a deep higher-order Boltzmann machine whose inference could be performed by rather naive MC sampling, which at low temperature operationally is the ReLU activation function. Therefore, given the vast space of stochastic DNNs, and the orthogonality in purpose, we refer to surveys [158–160] for a broad discussion of existing models, approximation algorithms and their trade-off, and we would focus on the continuation of the stochastic definition from deep Boltzmann machine and supervised feedforward DNNs in the following.

Deep Belief Network (DBN) is a probabilistic graphical model composed by hierarchically stacked restricted Boltzmann machine, and is also the first trainable DNNs that suggested the potential of deep models. It was designed as a generative model motivated by heuristic motivations: "an efficient way to learn a complicated model is to combine a set of simpler models that are learned sequentially"[161]. And back then, the motivation for a hierarchical model was justified from methods such as Boosting [161, p. 1535]. As a hierarchical model, DBN actually models higher-order statistical dependency but states the dependency through recursive second-order dependency. Later works, such as Deep Boltzmann Machine [162] and higher-order Boltzmann machine [163] are continuation of this line of physics-motivated works.

The effort to design higher-order Boltzmann machines is not mainstream now because the manual design of the higher order interaction and learning such higher-order generative models are both difficult [31]. More particularly, as generative models, the randomly initialized weights parameterize a vast high-dimensional probability space of the hidden variables, and without a ground truth, the MC sampling methods that are used to train the network take far too long to reach equilibrium. Therefore, initially, layer-wise greedy methods were designed to train the network [161]. The thrust is largely marginal now because each layer of DBN could be converted from an undirected graphical model (i.e., RBM) to a discriminative model—the conversion is not performed in a principled way, and is mostly for engineering purposes—and further finetuned through supervised training for better discriminative performance, and in this case, the training of DBN becomes a pre-train stage of Feedforward DNNs. And the community later found out that even without the pre-training of DBN, supervised Feedforward DNNs can be trained [95], the pre-training

stage of DBN had been dropped and supervised networks became the zeitgeist of Deep Learning [10].

However, it is not mandatory that a stochastic model has to be learned as a generative model. To appreciate the statistical inference system given by our stochastic definition, we could reason from the concept of Umwelt. It is rather metabolically expensive and time-consuming to learn a generative model that could reconstruct the environment. Instead, it is more efficient and perhaps the only tractable way to capture coarse-grained regularities of the environment that has evolutionary consequences; for example, whether a type of flower nectar could be made into honey, or not, based on the color and texture, and shape of the flower. Therefore, for a biotic system in its niche, it learns a specific model of the world that captures such coarse-grained signals instead of faithfully reconstructing the environment—though this leads to another open problem on where the feedback signals come, and this problem is considered future works.

From the formalism of our stochastic definition, the randomly initialized weights are simply a scheme of coarse-graining that characterizes a particular coupling between a hierarchy of events, and the learning of the system is to learn an informative coarse-graining such that the hierarchical coupling serves as a useful model for decision making, e.g., classifying a flower with particular hierarchical coupling of pixels (textures and color) is honey-making or not. In such a statistical inference system, the drifting in high-dimensional latent variable space is not an issue because the feedback signals (labels) are available to provide the ground truth of the probability distribution of the coarse-grained variable that characterizes the coarse-grained event, e.g., a particular follower is honey-making or not.

Therefore, our stochastic definition is not intended (at least for the time being) as a generative model, but as a statistical inference system that estimates the probability measure of a coarse-grained random variable whose realizations are labels in supervised learning; and thus is a supervised DNN by design. Under this stochastic definition, ReLU activation function are Monte Carlo (MC) sampling that does approximate inference of the realizations of random variables in the network. The stochastic definition is derived from the dual problem of a hierarchical maximum entropy problem, and is a graphical model belonging to the exponential probability distribution family that is known as deep higher-order Boltzmann machines. More specifically, the graphical model is a multilayer graphical model where random variables at layer $l$ could potentially be of $l$-order statistical dependency with all random variables of layers below layer $l$—this dependency results from the hierarchical coupling constraints in the hierarchical entropy maximization.

To conclude, from the preceding sense, that the stochastic DNN is a deep higher-order Boltzmann machine whose marginals could be computed by a MC approximation method that operationally is the forward propagation of Feedforward DNNs, the stochastic definition synthesizes deep Boltzmann machine and supervised Feedforward NNs. And such statistical characterization of DNNs shall enable the analysis of symmetries in DNN training of this work.

### 2. *Bayesian Neural Networks*

The stochastic definition of DNNs is also a Bayesian DNN, but not from the conventional sense that it is learned through Bayesian inference, but because the hypothesis space is endowed with a probability measure. We discuss the Bayesian aspects of the stochastic definition in the following.

The Bayesian DNNs is a subcategory of stochastic DNNs that refer to directed probabilistic graphical models whose parameters are random variables and are typically learned with Bayesian inference. It is envisioned to have the same benefits of stochastic DNNs (e.g., better generalization, and interpretability). In addition to the same effort in the field of stochastic DNNs (i.e., designing better models and approximation algorithms), the finer distinctions in Bayesian DNNs also induce efforts in designing better prior distributions to achieve better posteriors [164], for example, in term of generalization, or uncertainty quantification. Yet, similar to the relationship between our stochastic definition and most efforts in stochastic DNNs, the Bayesian aspects of our definition also does not aim for these potential benefits of Bayesian DNNs, but is a formalism for analysis. Therefore, we refer to the survey [159] for a detailed discussion of models, approximation algorithms and trade-off of Bayesian DNNs. And in the following, we explain the Bayesian aspects of the definition.

Our stochastic definition of DNNs is qualified as a Bayesian DNN not because it utilizes Bayesian inference, but because the endowment of a prior distribution on weights induces concentration of measure phenomena that are characterized as microscopic circuit symmetries and macroscopic adaptive symmetries in this work, and are the Bayesian-probabilistic phenomena underlying the symmetry-breaking in DNN training—that is, the probabilistic structure of the hypothesis space undergird the behaviors of the hypotheses. We elaborate further as follows. To refer a DNN as a Bayesian DNN, the convention typically refers to a DNN with the following structure: a choice of a prior distribution over the DNN's weight, and the use of Bayesian inference—that is, the use of Bayes' rule to infer and learn posterior probabilities. In our Bayesian definition of DNNs, though the DNNs could be learned with Maximum A Posteriori, and infer by computing posteriori, it is the fact, that the hypothesis space is also a probability measure space, that qualifies the definition as a Bayesian DNN. And given that we would like to study the current practice of DNNs (i.e., point estimation), the DNN is actually training by minimizing the surrogate risk that surrogates likelihood. Yet, though decoupled with the Bayesian inference, the Bayesian characterization of DNN is critical in that the probabilistic structure endowed by the prior distribution would induce concentration of measure phenomena mentioned previously.

The Bayesian definition might be better appreciated by analogizing to the difference between Einsteinian physics and Newtonian physics. While the underlying phenomenon stays the same, the Bayesian definition characterizes the phenomenon differently from the functional definition of DNNs where a DNN is a randomly initialized function approximator: in simple linear models like logistics regression, it does not make a difference to define the parameters as random variables

or not (as in the low speed macroscopic phenomenon under Newtonian physics), however, when the number of parameters becomes large (as the speed of objects approaches that of the light), a critical difference emerges as a result of concentration of measure, where the behaviors of the DNNs are statistically close to certain stable behaviors.

### B. Circuits of DNNs

Circuit is now a household concept popularized by information technology that have been overloaded with varied denotations in different contexts. To avoid confusions, we also briefly discuss an existing denotation of circuits in the context of DNNs, though it is only remotely related to the circuits in this work.

A formalism of probabilistic circuit has been developed to characterize and implement tractable probabilistic inference without explicitly computing probability distributions by applying transformation on samples, and has also be applied to interpret the operation of DNNs [165, 166]. However, the probabilistic circuits are intentionally stated as *not* probabilistic graphical models, and the nonlinearity in DNNs has been interpreted as certain atoms operators such as logarithm or exponential [165]. In contrast, the nonlinearity in our circuit formalism is to approximately compute the probability distributions of hidden random variables (e.g., exponential), and compute the metric between probability distributions (e.g., logarithm). The circuit formalism introduced in section II C is a technique that analyzes stochastic definition of DNNs, i.e., multilayer probabilistic graphical model, and thus *is* a probabilistic graphical model.

Another series of rather preliminary works [167] have been attempting to break the DNN down into tensor products, similar to the circuit formalism proposed in this work. The focus is by now is mostly interpretability: the information processed by the circuits are mapped to data to understand the features activating the circuits. However, it approaches in a brutal force manner without understanding the structure discussed in this work, i.e., the statistical inference of Umwelt, the expectation-maximization algorithm of DNN training, the microscopic and macroscopic feedback-control loops composed by the basis circuits, the circuit symmetry, the elementary excitation, the plasticity phase, and etc. It could be understood as an exploratory work slightly overlaps with the circuit formalism in this work.

### C. Symmetries of DNNs

From the perspective of the philosophy of science, existing works that endow symmetries in DNNs are different from the adaptive symmetries in this work: they are either proposed in the paradigm of reductionism in the sense of linear science, or in the paradigm of disorganized complexity, in the sense of the conservative symmetries in physics, while the symmetries characterized by this work are under the emerging paradigm of organized complexity, in the sense of biological symmetries. We elaborate in the following.

First, we discuss the application of the concept of symmetries to DNNs under the paradigm of reductionism in linear science. T. Körner wrote in his book *Fourier Analysis*, “it is sometimes said that the great discovery of the nineteenth century was that the equations of nature were linear, and the great discovery of the twentieth century is that they are not.” [168, p. 99]. Linear science is the great achievement of 19th century that discovers phenomena like heat and electromanetic propagation could be reduced into the linear superposition of basis functions. The reduction was first applied to study heat propagation by Jean B. J. Fourier non-rigorously, and is the famous Fourier Analysis. The rigorous formalism of such reduction was found by David Hilbert, and is the famous Hilbert space. In signal processing, Fourier analysis is not good at analyzing transient and multi-scale signals, and to analyze such signals, Wavelet Analysis [169] was invented. DNNs are signal processing system that process high-dimensional signals such as images, therefore, under the paradigm of linear science, a series of works [170–177], referred as Scattering Networks, try to characterize DNNs as hierarchically stacked modules where each module is a set of wavelet basis functions generated by symmetries (e.g., rotation, translation symmetry) that reduce/scatter the incoming signal into linear superposition of the wavelets. These scattering networks extract features invariant to transformation of symmetry groups composed hierarchically with simple groups, and thus achieves invariance to smooth shape deformation (i.e., diffeomorphism) to a certain degree—thus the symmetry groups are composite conservative symmetries. Therefore, they perform almost perfectly on data with strong but simple symmetries [172, 175]; and also achieve superior parameter efficiency in certain particular settings [177] because of the strong prior endowed. However, the scattering networks are manually designed feature extractors, and cannot learn from data, and thus do not characterize DNNs in practice—this is stated even from the scientific point of view: the manual design does not characterize how the symmetries emerge from learning.

Meanwhile, the concept of conservative symmetries in disorganized complexity (i.e., statistical physics) has also been adapted to design DNNs, justified by generalization benefits. For an introduction to the conservative symmetries, we refer readers to section II D. Similar to the spins in spin glasses that are of conservative symmetries (e.g., rotation and translation symmetry) that conserve free energy, the neurons in DNNs are designed to be of symmetries such that conserve the output of the network in certain ways; for example, to be invariant, or equivariant (depending on the goals) to transformation of the symmetries group. Such invariance or equivariance is a strong prior that reduces the size of hypothesis space, exempts DNNs to learn the symmetries (if they are present in the data), and thus improves generalization. The earliest design is the Convolutional Neural Networks that endow translation symmetry on neurons [143, 178]. Then, further symmetries are endowed on neurons; for example, rotation symmetry [179–181] and gauge symmetry [182]. The conservative symmetries are critical in Graph DNNs because the hypothesis space is exponentially

larger without permutation symmetry [183]. And the unifying language provided by symmetry groups to describe types of DNNs (e.g., CNN, RNN) induces the concept of Geometric Deep Learning [183].

Recall in section II C, we introduce that DNNs minimize variational free energy, therefore, the preceding conservative symmetries adapted to DNNs are also symmetries that conserve variational free energy. However, as explained in section II D, the symmetries we formalize are adaptive symmetries that are invariant of variants, and are not conservative symmetries that are invariant of invariant, where the system conserves free energy. The conceptual difference has been introduced in section II D, and thus we only further provides some examples that point out the conceptual difference in the following.

The following three examples, ranging from inorganic systems to simple organisms and complex organisms, *speculatively* suggest that symmetry breaking is an interactive process between innate symmetry of the system and the energy/informational perturbations from the environment: in absence of relevant perturbations/signals, the system would pose in a symmetric state, which in response to feedback from the environment, would break and the system would acquire asymmetric macroscopic features, which for biotic systems, typically have evolutionary consequences.

1. First, the symmetry-breaking of water molecule systems is different in different environments. For a system situated in a homogeneous heat bath where the heat propagation is homogeneous, water would crystallize into ice as we know it, which is a phase-transition induced by energy perturbations from the environment. Yet, in an environment where the heat propagation is not homogeneous, the initial ice crystals nucleate as roughly spherical crystals of ice with six-fold symmetry, and as the crystal grows, the tips of the crystal dissipate heat faster than the center, which makes the tips crystallize faster. As a result, snowflakes are formed [35, p. 330]. These are roughly two processes where the snowflakes form in the sky and ice forms in the river, while microscopically both processes break rotational symmetry and acquire a six-fold symmetry. Therefore, even for the same broken symmetries, the difference in environments would result in the different macroscopic manifestation of the broken symmetries.

2. Second, a similar phenomenon exists in microbiology. Cell locomotion is a major invention in evolution, which denotes the phenomenon that by default, a cell would perform a Brownian random walk as a result of thermodynamics, however, in response to food (e.g., glucose) gradient—technically referred as chemotactic gradient—the random walk would be aligned with the gradient through physicochemical mechanism [184, 185]. The phenomenon is conceptually formalized as a symmetry-breaking process [45, 184], where the symmetry of movement is broken by the perturbation of the food molecules.

3. Third, we give an speculative example, the formation of faces, which is a morphogenesis process that might be a diachornic symmetry-breaking process. In the process, because weak force is not relevant in biological phenomena, and thus evolutionarily relevant signals do not exist to break the mirror symmetry, a macroscopic mirror-symmetric system would form with features evolved through interaction with environments in the diachronic evolutionary process. And severe asymmetric of a face indicates a pathological morphogenesis process, and thus facial symmetry is selected as a strong fittness signal that is culturally known as beauty [186].

Therefore, the adaptive symmetry formalized and studied in this work is fundamentally a different kind of symmetries with the conservative symmetries in physics: it characterizes the emergent process of organized complexity in DNNs that is referred as an island between order (linear science) and disorder (disorganized complexity), while conservative symmetries could be appreciated as fundamental physical regularities in the feedback signals that break the adaptive symmetries, which when properly endowed on the DNNs, could improve the generalization ability of DNNs. Adaptive symmetries are the foundation where we analyze the risk landscape of DNNs.

### D. Risk landscape and phase space of DNNs

Both statistical physical systems and DNNs are systems that constituent a great number of units. Thus, the free energy landscape is a high-dimensional space parameterized by a great number of states. Despite the great number degrees of freedom, the collective behaviors of statistical-physical systems could be compactly described as a few macroscopic phases in a phase space parameterized by order and control parameters, many of which are distinctive macroscopic phenomena that could be directly perceived by humans (cf. section II F 1). The phase space of, for example, spin glasses is a *regionalization* of the free energy landscape according to symmetries. Under such a context, the plasticity-phase result in this work identifies a region of a DNN's risk landscape through stable symmetries where informational perturbation could be absorbed, and thus zero risk be reached. Thus, the plasticity phase is both a characterization of local geometry of risk landscape, and of a region of the risk landscape. Furthermore, as we are studying complex systems, it implies that the system consists of a large of units, which in our cases, is a DNN with a large number of neurons and weights: as introduced in section II F 5, the plasticity phase requires a DNN to be hierarchically large such that the concentration of measure phenomena could manifest.

Therefore, this work could be contextualized in the works that study the risk landscape under the *overparameterized* regimen, and the phases of DNNs. In this section, we discuss related works in this context. Meanwhile, we also clarify that there are a panorama of works on the optimization of DNNs—for example, the relationship between risk landscape and generalization, the convergence of optimization, and algorithmic considerations such as saddle-point avoidance—which are not within the scope of this work and would not be discussed. Theoretically, we also focus on global-minima results for large deep multilayer neural networks, and note that there are also many works that study shallow networks with one hidden layer [187–198], but they are not within the scope of this discussion. For these not discussed aspects, we refer interested readers to existing surveys [199–202]

We outline the discussion as follows. First, we discuss the fundamental difference between this work and existing works. As the difference in symmetries introduced in supp. A C, existing works on risk landscape also are constrained within conceptual apparatus either from reductionism of linear science, or from disorder in the disorganized complexity, while the plastic phase in this work results from the self-similarity emerging from coarse-graining of circuit symmetries in *hierarchical* disordered systems within the organized-complexity paradigm. This is elaborated in supp. A D 1. Second, in supp. A D 2, we discuss existing empirical works on the risk landscape of DNNs, which corroborate our results. Third, we discuss the theoretical works that study the global minima of deep multilayer networks under the overparameterized regimen in supp. A D 3 and A D 4. In supp. A D 3, we discuss the approach that studies the global minima of DNNs from reductionism in linear science by retrograding DNNs back to linear models. The assumptions made in this approach is mostly argued as a post-hoc verifiable condition, instead of a characterization of the behaviors of DNNs, and thus provide limited insights into optimization/learning process of DNNs. In supp. A D 4, we discuss the approach that remolds DNNs into a disorganized complex system either by direct assumptions or by pumping massive amount of disorder through infinite-width assumptions. Both the approaches from linear reductionism and from disorganized complexity require DNNs to be overparameterized in a way that is away from the current practice; and efforts that try to relax the assumptions also dissipate the disorder created by overparameterization, and could not maintain the global-minima results. Our results could be also appreciated as improvements over these works, for example, by considering hierarchical disorder in hierarchical large DNNs, and thus keeping the disorder needed by these existing works without requiring large width—some details are provided at the end of each subsection. Fourth, in supp. A D 5, we discuss certain existing works that show local minima with risk higher than global minima exist for some networks, to clarify that small networks, or merely largeness alone could not lead to plasticity phase. Lastly, in supp. A D 6, we discuss existing denotations of "phases" in the literature. Existing denotations of "phase" typically make an analogy with certain behaviors of physical systems that are associated with phases of these systems. Though our denotation of phase could also be stated as such, we are extending/analogizing the epistemology of physics, where phases are defined by stable symmetries (cf. section II F). These discussed existing works also include empirical works that corroborate the interpretation that the region of risk landscape identified in this work is a phase of DNNs.

### 1. *Disorder in large DNNs*

To begin with, we review the empirical observations that large DNNs perform better, and the setting known as **overparameterized** regimen in the literature. A marvelous observation in the earlier days of Deep Learning is that the larger the network, the better the performance of the network on the data: this could be seen in the series of works [11, 75, 145] that improve the performance on Imagenet [203]. Later, this correlation was discovered to be of scaling laws, e.g., Kaplan *et al.* [204], but we are getting ahead of ourselves. However, no theoretical understanding was available for such a phenomenon. Then, Zhang *et al.* [23] empirically found that unlike the prediction made by classic statistical learning theory, overparameterization does not lead to overfitting for DNNs—overparameterization qualitatively means more parameters than necessary are employed, and quantitatively means (in the DNN literature) more parameters are employed than the size of the sample. This observation motivated, or legitimized the approaches that study DNNs in a regime that is away from how DNNs is currently practiced: the width of at least one intermediate layer needs to be larger than the number of training examples, or even larger, an literally infinite width. This regime is referred as the overparameterized regime.

Such overparameterization pumps massive amount of degree of freedom, or disorder into a DNN, and induces phenomena of disorganized complexity that could be characterized by methods in linear science, or statistical physics: from the perspective of linear reductionism, because the width of a layer could be made as large as desired, linearly independent features of training examples are always obtainable by adding more neurons and perturbating these neurons to be independent; and from the perspective of disorganized complexity, because the width is approaching infinite and a neuron at a higher layer is the weighted sum of activation of neurons at a lower layer, by central limit theorem, such addition would be a Gaussian distribution. Based on more sophisticated versions of these facts, results on minima of DNNs are obtained.

However, such an overparameterized regime is not how DNNs are used in practice, and the appealing optimization behaviors discovered in existing works might be illusive—though this work could also be appreciated as a continuation of the disorganized complexity approach where hierarchical interactions are analyzed through a synthesis of statistical field theory and statistical learning theory—this aspect would be further discussed in supp. A D 3 and supp. A D 4. In this work, we instead study the effect of such largeness from the perspective of organized complexity, and characterize that the stable optimization behaviors of DNNs emerge from certain hierarchical/organized disorder in a large complex system, as shortly explained in the following.

First, we do seek a certain reductionism, but not in the sense of the reductionism in linear science. A DNN (of depth $L$) is reduced to the summation of a large number of basis circuits (introduced in section II C), that each characterizes a $L$-order interaction of $L$ neurons from the bottom layer to the top layer (i.e., hierarchical interaction). Unlike the orthogonality that the reductionism in linear science typically implies, the basis circuits are of sparse statistical dependence with the rest of basis circuits. More specifically, a basis circuits is composed by $L$ neurons, and thus for two basis circuits, if a strong correlation exists between the two circuits, the $L$ neurons of one circuit need to be of strong correlation with all the $L$ neurons of another. Consequently, the correlation between the two basis circuits has an exponential decay w.r.t. depth, and there are only sparse dependence among basis circuits for large DNNs.

And despite such weak interactions, organized interaction exist in the higher order interaction within basis circuits and sparse correlation among circuits, and the cooperation among basis circuits could enable the detection of the macroscopic patterns.

Then, at the granularity of basis circuits, this sparse dependence is similar to the sparse interaction among spins in spin glass models, and thus when the size the network is large in a hierarchical sense, the coarse-graining of the circuit symmetries (introduced in section II D) would manifest as concentration-of-measure phenomena that are self-similarity between the microscopic scale (basis circuit) and the macroscopic scale (neuron assemblies, introduced in section II C)—this is similar to the self-similar induced by translation and rotation symmetry between the microscopic scale and the macroscopic scale in statistical-physical systems—and one of such concentration-of-measure phenomenon is the plasticity phase introduced in section II F. More specifically, when a DNN is hierarchically large (cf. section II F 5 for what hierarchical largeness means; it is also the number of parameters), a large number of basis circuits would be of microscopic adaptive symmetries (i.e., circuit symmetries) and are of sparse correlation with one another (cf. section II F 3 for a detailed introduction). The sparse correlation among basis circuits characterizes a low degree of interference with one another, and thus each circuit is able to respond to the feedback signals relatively freely. Then, a self-similarity between the microscopic and the macroscopic—the coarse-graining of such microscopic adaptive symmetries—manifests such that the system could respond to feedback signals in an adaptive-symmetric way, and thus reach zero risk eventually. This is a concentration-of-measure phenomenon, and is characterized by a non-asymptotic probability bound.

To emphasize, the largeness does not come from very wide layers, but is a hierarchical largeness that is an interaction of both depth and width; more verbosely, the largeness can be achieved by adding more layers, instead of just enlarging the width. And even the smallest DNNs currently are rather large: the DNN we use in experiments has $\sim 10^7$ parameters, and recall that concentration-of-measure phenomena such as normal distributions and semi-circle law of random matrices manifest even with a few hundreds example (for normal distributions), or dimensions (for semi-circle law).

#### 2. *Empirical results on risk landscape*

The first explicit discussion of the empirical observation that large DNNs do not have local minima are made by Dauphin *et al.* [20]. The further study of stationary points were pursued by empirically computing the eigenvalue distributions (i.e., eigenspectrum) of Hessian [139, 140, 205–210]. The empirical works show a picture roughly as follows, and details could be found in Papyan [210]. The Hessian is the addition of two matrices, a Wigner-type and a Wishart-type matrix. After a DNN is trained, the Wigner-type matrix is symmetrically distributed against $y$-axis, and is close to zero for training examples, but not for test examples. The Wishart-type matrix, which is positive definite, has $c$ large eigenvalues far away from the bulk of the eigenspectrum, where $c$ is the number of classes. These large eigenvalues have been studied to relate to the convergence of SGD [211], or the generalization of minima [212], but these properties are not the concerns of this work. The existing of negative eigenvalues as a result of the symmetry of the nonzero Wigner-type matrix implies the DNNs in experiments could further decrease risk of test examples.

For binary classification with hinge loss, the setting studied in this work, the Wishart-type matrix disappears, and only the Wigner-type matrix stays. This simplifies the problem. The simplified setting is the first problem of two interdependent problems of the general setting, and the setting has been explained in section II G. To briefly explain, the negative eigenvalues of stationary points could only come from the Wigner-type matrix because the Wishart-type matrix is positive definite, and thus the Wigner-type matrix is the first milestone to analyze if we are to understand the local geometry of the risk landscape. We theoretically and experimentally find that the symmetry of the Wigner-type matrix, which is the Hessian in our setting, holds throughout training, in addition to existing works Papyan [139, 210] that observe it holds at the end of the training. This region of the parameter space where such a symmetry holds is referred as the plasticity phase.

We also note that in our analysis, the circuit symmetries hold only for ReLU-family activation, and do not hold for activation function like Sigmoid. And in practice, activation functions like Sigmoid need to be tuned to an approximate linear, and the neuron activation needs to be tuned in a symmetric regime (i.e., zero mean and unit variance) before training could proceed, either through careful initialization [19, 213], or online normalization such as Batch Normalization [214]. And thus the behaviors of these activation function are close to piecewise linear function like ReLU when they work. Therefore, in general, the adaptive symmetries in this work do not hold for any activation function; for example, Geiger *et al.* [215] observe that in certain simplified settings, networks with tanh activation has a slightly distorted symmetrically distributed eigenspectrum. Actually, the adaptive symmetries might not occur for ReLU activation, if the coarse-grained adaptive symmetries formalized as assumptions (cf. section II F) in this work do not hold.

This work also corroborates other existing empirical works that study the so called *large-scale structure* of DNNs' risk landscape. It has been shown [216–219] that DNNs could be optimized in low-dimensional manifold than the parameter space without performance penalties. It also has been shown [220–222] that minima of DNNs are connected by simple curves where the risk is nearly constant. Fort *et al.* [223] found that the training dynamics of DNNs could be divided into two stages: the first stage is a chaotic stage where different initialization would lead to minima with low loss in different basin (i.e., different regions of the risk landscape that is separated by an barrier), and after the chaotic stage, the minima are linearly connected. Yang *et al.* [224] found that the well-behaved properties of risk landscape correlate with the size of a network and the quality of data: large networks with high quality data lead to better performance and well-connected landscape, and vice versus. The plasticity phase corroborates these existing

results. When the potential complexity of a DNN's reservoir of circuit symmetries exceeds the complexity of the dataset, first, a redundancy of circuit symmetries exist in the DNN, and thus these redundant symmetries are not broken during training, resulting that the optimization only happens in a low-dimensional manifold; second, because the adaptive symmetry (i.e., symmetrical distribution of both gradient and Hessian eigenspectrum), abundant directions with near zero perturbation to risk exist, and results in the simple curves connecting different minima, but such connectivity only exists locally, and networks spawned in the early stage of training probably reach different local areas and manifest the phenomenon observed by Fort *et al.* [223]; third, the redundancy of circuit symmetries are relative to the complexity of dataset, and when the quality of the data is poor, or the network is small, the complexity of the data would exceed the redundancy (i.e., potential complexity) of the DNN, and thus poor performance and connectivity ensue. However, we also note that this is a non-rigorous and informal discussion on the relationship between this work and previous empirical observations, this rich phenomenology has not been systematically studied and discussed in this work.

Meanwhile, existing theoretical explanations of the previous phenomenology approach either from the linear-science, or from the disorganized-complexity paradigm mentioned in supp. A D 1. The detailed discussion on existing works in those two paradigms is given in supp. A D 3 and supp. A D 4, and here we briefly discuss the existing theoretical analysis that relates to the connectivity of minima here. Freeman and Bruna [225] show that the connectivity non-asymptotically increases with width through linear-algebraic analysis that considers neural weights as atoms, and thus the technique could only apply to network with one hidden layer so far. Nguyen [226] proves that sublevel sets of DNNs are connected by formalizing the idea that if the activation function is strictly monotonic, the weight matrices are of full rank, and at a specific layer features of all training examples are linearly independent (which requires overparameterization), the difference between two point on the risk landscape could be morphed into the difference of parameters in one layer, and the convexity of the parameter space in a single layer makes a risk landscape where sublevel sets are connected. The shortcoming of this approach is discussed in supp. A D 3. Kuditipudi *et al.* [227] assumes that if a DNN is stable in the sense that the neurons could be switched off randomly (i.e., dropout) without changing the loss, then connecting path could be found among low cost solutions on the landscape. The result makes sense intuitively, however, it takes the stability as an assumption, and does not study why it is stable. Existing works that analyze the stability, for example Shevchenko and Mondelli [228], still rely on the approach that analyzes the disorganized interaction pumped into the network by large width. The shortcoming of this approach is discussed in supp. A D 4.

### 3. *Retrograde DNNs to linear models*

To begin with, we introduce the core idea of the linear reductionism approach. As discussed in supp. A C, the reductionism in linear science reduces an object into the linear superposition of basis elements that are independent with one another. The core idea of the approach is that if the features of an intermediate layer (typically the last) of all training examples are linearly independent with one another, then when the gradients are zero, the risk would be zero (because the features are nonzero, and thus the only possibility is the losses are zero). For such an assumption to hold, the number of the feature vectors needs to be larger than the size of the sample, and thus the network is overparameterized—though architectures that share parameters could overcome this limitation, this is not the major problem of this approach, as described next. However, the usefulness of linear reduction is that the object could be decomposed into components that could be studied separately, then put together linearly again to recover the object, and thus reach a understanding of the object: for example, light could be decomposed by frequency through Fourier analysis, and be further analyzed. This is not true for DNNs, the feature space is a blackbox, and thus the linear independence is a condition that is applied on feature space out of convenience, or intellectual inertia, instead of analyticability. Heuristically, it characterizes the phenomenon that if linearly distinguishable features can be created for all examples at an intermediate layer of a DNN, and the distinctions can be almost linearly passed onto the output layer, then these examples can be properly mapped to labels. This is likely not how DNNs work. As a result, it is mostly argued as a post-hoc verifiable condition, instead a characterization of the behaviors of DNNs, and thus provide limited insights into optimization/learning process of DNNs, which shares the same problems with the scattering network discussed in the linear science paradigm in supp. A C.

More specifically, this approaches started from linear DNNs, and gradually moved to nonlinear DNNs by making the previously linear independent conditions—we do not aim to give a complete survey, but to give a rough developmental narrative in the following. Kawaguchi [229] proves all local minima of a deep linear NN are global minima when some rank assumptions of the weight matrices are held. Hardt and Ma [230] show that all local minima are global minima for linear ResNet. Nguyen and Hein [231] prove that for the squared loss function, if in a certain layer of a nonlinear DNN, it has more neurons than training samples, which makes it possible that the feature maps of all samples are linearly independent, then the network can reach zero training errors. Nguyen and Hein [232] and Nguyen *et al.* [233] extend the result to Convolutional NNs and Residual DNNs, respectively. Liang *et al.* [234] improves the results specifically for binary classification. Laurent and von Brecht [235] extend the result to arbitrary loss functions. Yun *et al.* [236] gives necessary and sufficient conditions for a stationary point to be a global minimum. Kawaguchi and Huang [237] reduces the requirement on width such that the network is less overparameterized. Kawaguchi [238] designs an algorithm that verifies the independence condition to ensure global minima. Jagtap *et al.* [239] reduce the overparameterization required by global minima by designing a tensor parameterization that reduces the number of parameters—this work actually moves closer to the parameterization of Umwelt that leads to DNNs: at layer $l$, the network is actually pa-

rameterized by $l$-order tensors, which are computed through dynamical programming (cf. supp. B C 2).

### 4. Remold DNNs to statistical fields

Another collection of works approach from the paradigm of disorganized complexity by turning neurons are statistical fields, either by direct assumptions, by making network infinitely wide, or by approximate perturbative characterization. We discuss this approach in this subsection.

In physical systems, a field is a coarse-grained characterization of a collection of particles, and it is a good formal model of the particles' collective behaviors because the disorganized interaction among particles, unraveled through a timescale orders of magnitude larger than the thermodynamic timescale, results in statistically stable, homogeneous behaviors of this collective—which mathematically is a concentration of measure phenomenon. As a result of the disorganized interaction, the behaviors of a particle typically could be characterized by a Gaussian distribution. A typical example would be the mean-field models, which we refer to supp. D D for a review. As the reductionism of linear science, statistical field methods is one of most successful enterprise in science that studies disorganized complexity such as spin glasses.

A collection of works therefore assume neurons are of Gaussian distributions, or assume disorganized complexity that induces some concentration-of-measure phenomena (e.g., Gaussiand distributions), and proceed from there to analyze the behaviors of DNNs [31, 240, 241]. However, the field methods are meant to analyze disorganized complexity, implying it studies homogeneous systems that either have no long range interaction, or homogeneous long range interaction (at criticality), while as introduced in section II C 2, the interaction of DNNs are spatially and temporally heterogeneous, and are local yet hierarchically coupled in response to feedback signals; or in other words, neurons could have no interaction with some neurons, but also have long range interaction with some other neurons. Therefore, the disorganized-complex assumptions characterize theoretical models that is also away from current practice of DNNs. We discuss works of this approach as follows.

To begin with, we give a short summary of the development. This approach first directly assumes independent Gaussian distribution on individual neurons [146, 209, 242–244]. Then, some concentration of measure phenomena (e.g., Gaussian distributions) are coalesced on neurons by assuming that layers have infinite width [129, 130, 245–251]. Note that any probability distributions with only up to the second-order statistics are Gaussian distributions, and thus further works pursue finite-width corrections of the previous phenomena by incorporating higher order statistics (perturbations) [76, 252–255]. We also discuss a closely related approach that studies the global convergence of DNN training [256–258].

The first sets of works assume that the neuron activation is independent with data, and prove that local minima of large DNNs are close to global minima. More specifically, by assuming, among some other assumptions, that neuron activation is independent with neuron inputs, and the input is a random vector that each is a standard normal distribution, Choromanska *et al.* [146] transform a DNN to a spin glass model, and show that local minima are close to global minima for large networks. Later, they acknowledged the assumptions are unrealistic [259]. By assuming, among some other assumptions, weight, data and error residuals are independent normal distributions, Pennington and Bahri [242] derive an analytic expression for the eigenvalue distribution of Hessian at critical points, where the Wigner-type matrix is the Hessian in our setting (cf. section II G), and thus give a phenomenologically close conclusion to risk landscape characterized in section II F. Under similar independent assumptions, Fort and Ganguli [209] derive a phenomenological model that reproduce empirical observed phenomena of the risk landscape. Apr and Building [243] generalize Choromanska *et al.* [146] to general activation functions but still make the unrealistic assumption that neuron activation is independent with weights. Under the assumptions of Choromanska *et al.* [146], Becker *et al.* [244] further study the effect of depth, and find that fixing the number of parameters but increasing depth, the minima becomes more clustered, and thus more close to global minima. As could be seen, the independent assumptions made in this approach characterize a phenomenon where the activation of neurons are uncorrelated with one another, and thus in the theoretical model no useful information could be learned; that is, neurons are not fields in the sense that they are statistically homogeneous/indistinguishable units resulted from disorganized interaction.

As the directly assumed Gaussian distributions are unrealistic, the second sets of works assume that each layer of a DNN is of infinite width, which pumps disorder into the network, and thus induces Gaussian distribution of neurons, and then prove that global minima could be reached by gradient descent. Recall that the weights of neurons are randomly initialized, typically to Gaussian distributions, and thus neurons at initialization are of independent Gaussian distribution; by creating a huge number of such neurons, there would be a great number of uncorrelated random neurons in the network, and thus a great amount of disorder; then, even during training, by central limit theorem, neurons would be of Gaussian distributions, as a result of such disorganized interaction. In such a setting, a DNN is a Deep Gaussian Process (GP) [245]. And for a given layer, the output of neurons are well approximated by its first order Taylor expansion [260], and thus higher order interactions beyond second order are turned off, and exact inference is possible because the network could be exactly characterized by the mean vector and covariance matrix of multivariate Gaussian distributions. As a result of such huge amount of disorder, the network is close to some fixed networks throughout training [246, 248] and thus would reach global minima through gradient descent: different fixed limit networks would result from different initialization, and two of the more known are the *Neural Tangent Kernel* (NTK) (or lazy learning) regimen [246], and *Mean-Field* (or feature learning) regimen [248].

A closely related approach from the perspective of convergence also works by pumping disorder into the network [256–258]. By increasing the width to a very large polynomial, the update of a gradient to the weight matrices of a DNN would

negligently small, and thus global minima could be reached within a certain number of gradient descent iterations. However, the width required by the works is very large: the lastest result [258] requires the width is at least $\Omega(n^{14}L^{16}/\phi^4)$, where $n$ is the number of training examples, $L$ is the number of layers, and $\phi$ is the minimal distance between inter-class examples.

However, networks with very large width have limited representational power, and the results at infinite width do not generalize to finite width. Empirically, wide networks under-perform the narrower networks in practice [76, 261, 262]. Theoretically, with a particular choice of prior, Pleiss and Cunningham [263] prove that an infinitely wide DNN is a Deep GP that converges to a Gaussian processes, and thus effectively becomes a shallow model; and in the NTK regimen, the neural tangent kernel associated with the infinite width networks is equivalent with shallow kernels [264, 265], and thus composite or depth does not bring advantage: the results are intuitive because the random transformation of random features would only lead to random features. Furthermore, at finite width, NTK is not constant [266]; and for DNNs used in practice, the NTK that is assumed to be constant in the NTK regimen changes significantly during training [223]. In addition, there are data distributions that normal DNNs used in practice could learn better than the infinite-width setting [260, 267–270].

The negative results in the infinite width regimen lead to the search for different ways the infinite is reached, by exploring different training protocol [247], or by studying the effect of different priors [249–251]; or to exactly characterize the effect of priors on DNNs, e.g., ReLU DNNs [271] or to combine infinite-width networks with finite bottleneck layers that increase feature flexibility [272]. In these settings, results on minima of DNNs are absent.

To move beyond the infinite-width setting, finite-width corrections are made by a third set of works, but no results on minima of DNNs have been reached yet. The influence of higher order statistics has been calculated to correct the second order statistics for network outputs [76, 252–254], or for features in the hidden layers [255]. However, this thread of works revert from the deep nonlinear multilayer setting in the works that assume infinite-width, and back to earlier settings where either toy data are used in analysis, or simplified networks like linear or toy nonlinear networks are analyzed: for example, the result of Cohen *et al.* [76] only hold when data are uniformly distributed in a hypersphere; the result of Dyer *et al.* [253] only holds when data are equal in all dimensions; Naveh and Ringel [254] analyze linear networks, or networks with quadratic activation function after they are already trained, all of which have only two layers; Zavatone-Veth *et al.* [255] analyze linear networks, or network with a single nonlinear layer, and only reach some qualitative and speculative results in the later setting; Yaida [252] derives a quite general but complicated recursive formula, yet the complication of formula prevents any analytical insights and the formula needs to be studied numerically: in experiments, it has only been applied to data that only have one dimension, and thus has the problem of analyticality, scalability, and verisimilitude.

Overall, the limitation of such finite-width correction reflects a deeper problem: the disorder of statistical physical systems might not even exist in the organized interaction of DNNs. As discussed in the beginning of this subsection, analytic tractability is possible because of the massive disorder pumped into the network by assuming infinite depth. And when this disorder is not assumed, the disorganized complexity of statistical physical systems disappears in DNNs. Therefore, to analyze such finite-width networks, the networks need to be homogenized by assuming uniform data, or homogeneous interaction (i.e., linear networks), such that along with the uniform parameter initialization, the homogenization would induce homogeneous neurons. Such homogenization creates some artificial conservative symmetries [273]. Consequently, techniques like Feynman diagram or integration in renormalization group could lead to analytic results. Otherwise, only numerical results are possible, which has the problem of analyticality, scalability and verisimilitude. Furthermore, recall that we discuss at the beginning of this subsection that the characteristics of DNNs are the spatially and temporally heterogeneous, local yet hierarchical coupling among neurons. Thus, a neuron might be statistical dependent with specific neurons scattered across the network, which make such perturabative analysis questionable: such finite-size correction typically only considers statistics within a layer—recall the goal is to correct for the non-negligible statistics resulting from the finite width of a layer, which is previously zero because it is divided by an infinite width.

Therefore, we might need to move beyond disorganized complexity, and in this work, under the paradigm of organized complexity, we pursue a different kind of disorder (i.e., hierarchical disorder), a different kind of symmetries (i.e., adaptive symmetries), and a different kind of statistical characterization (i.e., statistical assemblies) of the complex system of DNNs. The difference in disorder has been discussed in supp. A D 1, the difference in symmetries has been discussed in supp. A C, and the difference in statistical characterization has been discussed in section II D 3.

#### 5. *Frustration phase of DNNs*

Many existing works have also shown that DNNs in many settings, even when DNNs are overparameterized, there exist local minima that are not global minima. This regimen has been tentatively classified as frustration phase in this work in the discussion section, supp. C C. Though a thorough study of the frustration phase is not within the scope of this work, the relationship between the plasticity phase and frustration phase discussed in existing works might be confusing. In this subsection, we clarify existing works that relate to the frustration phase, which also corroborate the characterization that without stable adaptive symmetries, a DNN could not be in the plasticity phase.

First, the stable adaptive symmetries could only exist in large network, as there is no stable macroscopic magnetization for a few magnetic molecules. When a network is small, counterexample could be constructed where local minima that are not global minima [274]. Second, the hierarchical disorder might not exist when strong correlation exists in neurons. For example, He *et al.* [275] construct networks that have local

minima that are not global minima by making the activation of all layers positive. Therefore, without largeness, or merely largeness alone could not ensure the phenomenon where local minima are global minima. Because this relate-works discussion aims to discuss works that study global minima of large multilayer networks, which is known as the overparameterized regimen, we would not further discuss the panorama of results on optimization behaviors of neural networks, and further works could be found in the existing surveys [199–202].

### 6. *Phases of DNNs*

To begin with, we discuss related works that corroborate that interpretation of our results as identifying a plasticity phase. Hinge loss incentivizes that examples of different classes should not be too close. Under such a setting, the optimization of DNNs have been analogized to the jamming in physics where phase transitions exist when particles that are getting too close. Under this analogy, Geiger *et al.* [215] empirically observe that a sharp transition manifests in the classification errors when a network is trained with random data uniformly sampled from a hyper-sphere, and has roughly the same number of parameters with the number of training examples. However, the transition is less sharp for a subsampled MNIST dataset. Geiger *et al.* [215] refers the two regimens as the underparameterized and overparameterized regimens. In this work, these two phases are referred as frustration phase and plasticity phase, respectively—we have described why overparameterization is a misleading qualifier in supp. A D 1. And we discuss that the optimization process of a DNN is an extended symmetry breaking process, where heterogeneous symmetries are being broken: more specifically, certain training examples would require breaking symmetries of certain circuits, and if such circuits do not exist, the network would frustrate on these particular examples. From this perspective, the sharp transition observed in Geiger *et al.* [215] could be speculated to result from homogenization of data—that is, all examples are uniformly sampled from a sphere—and as a result, the network would frustrate on all the examples simultaneously, and manifests the sharp transition. Correspondingly, the transition is less sharp because the subsampled MNIST dataset is less homogeneous, though is still rather simple. In addition, Baity-Jesi *et al.* [21] empirically show that for more practical DNNs on typically used datasets in practice, small networks frustrate (i.e., manifest glassy behaviors) and could not reach zero risk, while large networks do not, and reach zero risk; and thus suggesting there are two phases of DNNs depending on networks' size. However, we note that the speculation has not been studied in this work, and is merely a clarification that our results do not conflict, instead corroborate with Baity-Jesi *et al.* [21] and Geiger *et al.* [215]. Furthermore, we characterize the hierarchical interaction among neurons that are analogized with the particle interaction as neuron circuits and assemblies, and the diversity assumption deduced from coarse-grained circuit symmetries could be appreciated as formalizing the condition where the neurons are not "jammed".

There are other mentioning of phases of which the relationship with the plasticity phase is subject to future study: there could be multiple types of symmetries in DNNs, as there are translation and rotation symmetry in spin glasses to break simultaneously or separately, or the phases are not related to symmetries and are simply analogies. We briefly discuss these mentioning of phases in the following. The *double descent* phenomenon [134, 135] has also been discussed as a phase transition: the generalization error of random Fourier feature model [276] manifests a singularity when the model transits from underparameterized to overparameterized. The overparameterized phase is further divided into feature learning phase and lazy learning phase sometimes [224, 277, 278], justified by the theoretical phenomenon in the infinite-width setting that in the feature learning phase, parameters change after training, while in the lazy learning phase, they do not. The relationship between the overparameterized phase and the plasticity phase has been discussed from supp. A D 1 to supp. A D 4. Feng and Tu [279] interpret the training of DNNs as a non-equilibrium statistical-physical process, and divides the into phases by the alignment of the gradients with their mean amplitude. The classification of phases are justified by its utility in cleansing mislabeled data. Kunin *et al.* [280] consider the weight space as the phase space by analogizing weights with particles as in classic mechanics. These two denotations of phases are not directly related to minima of DNNs.

## B. FORMAL RESULTS

### A. Notation and terminologies

To begin with, we note that a few words that we shall use interchangeably in this paper: environment and dataset; training, optimization, self-organization, and risk minimization.

*a. Notations of mathematical objects.*

1. Normal letters denote scalar (e.g., $f$); bold, lowercase letters denote vectors (e.g., $\boldsymbol{x}$); bold, uppercase letters denote matrices, or random matrices (e.g., $\boldsymbol{W}$); normal, uppercase letters denote random elements/variables (e.g., $H$). $:=$ denotes the "define" symbol: $x := y$ defines a new symbol $x$ by equating it with $y$.

2. A set of nonnegative integers up to $L$ is denoted as $\mathbb{L} := \{0,\ldots,L\}, L \in \mathbb{N}^{+}$—this is to conveniently denote $L+1$ layers of a DNN, including the input layer. A sequence of positive integer is also conveniently denoted as $[N] := \{1,\ldots,N\}$.

3. To conveniently index entries of a matrix, let $\mathbb{J}$ denote $[N]$, and let $\mathbb{I}$ denote $[N] \otimes [N]$, the Cartesian product between two $[N]$. For $\alpha \in \mathbb{I}, A \subseteq \mathbb{I}, i \in \mathbb{J}$, given a matrix $\boldsymbol{W}$, $w_{\alpha}, \boldsymbol{W}_{A}, \boldsymbol{W}_{i,:}, \boldsymbol{W}_{:,i}$ denote the entry at $\alpha$, the vector that consists of entries at $A$, the $i$th row, $i$th column of $\boldsymbol{W}$, respectively. Correspondingly, for $A \subseteq \mathbb{J}$, $\boldsymbol{W}_{A,:}$ denotes the submatrix consisting of the columns indexed by $A$; similarly does $\boldsymbol{W}_{:,A}$; for $A \subseteq \mathbb{J}, B \subseteq \mathbb{J}$, $\boldsymbol{W}_{A,B}$ denotes the submatrix that consists of rows of $\boldsymbol{W}$ indexed by $A$, and for each of the rows, only the elements in columns indexed by $B$ are retained. Occasionally, $\boldsymbol{W}_{ij}$ also denotes $w_{ij}$ ad hocly, and should be self-clear in the context. But, for random matrices, both bold and normal matrices use the same

notation, except when indexing the entries: given $i, j \in \mathbb{I}$, for scalar, upper case denotes random variable $W_{ij}$, while lower case denotes scalars $w_{ij}$. $\mathrm{dg}(\boldsymbol{h})$ denotes a diagonal matrix whose the diagonal is the vector $\boldsymbol{h}$.

4. Because a DNN is a multilayer network, we need the indices to denote the layers. When the lower index is not occupied, we use the lower index to denote a layer; for example, random vector at layer $l$ is denoted $H_l$. Otherwise, we put the layer index onto the upper index; for example $H_i^l$ denotes $i^{th}$ component of $H_l$. If matrices are indexed, we move the index up when indexing its entries, i.e., $w_{ij}^1$ denotes the $ij$th entry of $\boldsymbol{W}_1$.

*b. Notations of operations.*

1. Given two matrices $\boldsymbol{A}, \boldsymbol{B}$, the curly inequality $\preceq$ between matrices, i.e., $\boldsymbol{A} \preceq \boldsymbol{B}$, means $\boldsymbol{B} - \boldsymbol{A}$ is a positive definite matrix. Similar statements apply between a matrix and a vector, and a matrix and a scalar. $\succeq$ is defined similarly. tr denotes matrix trace. $\mathrm{dg}(\boldsymbol{h})$ denotes the diagonal matrix whose diagonal is the vector $\boldsymbol{h}$. $\langle \boldsymbol{x}, \boldsymbol{y} \rangle := \boldsymbol{x}^T y$, $\langle \boldsymbol{A}^T \boldsymbol{B} \rangle := \mathrm{tr}\ (\boldsymbol{A}^T \boldsymbol{B})$.

2. $\kappa(\cdot,\cdot)$ denotes covariance: for example, e.g., $\kappa(w_\alpha, w_\beta)$ denotes the covariance between $w_\alpha, w_\beta, \alpha, \beta \in \mathbb{I}$, and $\kappa(f(\boldsymbol{W}_A), g(\boldsymbol{W}_{A'})), A, A' \subseteq \mathbb{I}$ denotes covariance between functions $f, g$ of entries in $\boldsymbol{W}$. $\kappa(\alpha, \beta) := \kappa(w_\alpha, w_\beta)$. $\kappa$ also denotes cumulants.

3. $||\cdot||$ denotes 2-norm if not specified otherwise. $\Re$ and $\Im$ take the real and imaginary part of its operand (a complex number), respectively. The upper arrow on operations denotes the direction: for example, $\overrightarrow{\Pi}_{i=1}^n \boldsymbol{W}_i, \overleftarrow{\Pi}_{i=1}^n \boldsymbol{W}_i, i < n, i, n \in \mathbb{N}$ denote $\boldsymbol{W}_1 \ldots \boldsymbol{W}_n, \boldsymbol{W}_n \ldots \boldsymbol{W}_1$, respectively. $\mathscr{L}'(\cdot)$ denotes the derivative of a function $\mathscr{L}$ w.r.t. the input. $\otimes$ denotes Cartesian product. $\Theta$ denotes the asymptotic rate notation. $\mathrm{supp}\mu$ denotes the support of a function $\mu$.

*c. Notations of less widely used mathematical objects.*

1. $\bar{l}$ denotes a sequence (e.g., $(1,2,3)$) that accepts a partial order: given two sequences $\bar{l}_1, \bar{l}_2$, $\bar{l}_1 \leq \bar{l}_2$ implies the largest element of $\bar{l}_1$ is smaller than the smallest element of $\bar{l}_2$. $\overrightarrow{\otimes}_{l \in \bar{l}} [n_l]$ denotes the Cartesian products are performed sequentially according to the order of $\bar{l}$. This notation applies to a domain (e.g., $\mathbb{L}^+$), as well a sequence $\bar{l}$.

2. $\underline{\alpha}$ denotes a multiset (e.g., $\{0,0,3\}$), and the definition of multiset is reviewed at definition 32 in supp. F A 1. Note that a vector is also a sequence.

3. $\boldsymbol{i}_{p:q}$ denotes the subvector of $\boldsymbol{i}$ that is sliced from the $p^{th}$ component to $q^{th}$ (exclusive; that is, $i_q$ is excluded). This is the conventional in most programming languages to slice arrays. If the ending index is omitted, e.g., $\boldsymbol{i}_{p:}$, it denotes the subvector sliced from the $p^{th}$ component until the end (inclusive); similarly, if the starting index is omitted, e.g., $\boldsymbol{i}_{:q}$, it denotes the subvector sliced from the beginning (inclusive) until the $q^{th}$ component (exclusive).

All the remaining symbols are defined when needed, and should be self-clear in the context.

## B. Umwelt: system that does statistical inference on hierarchical events

In supp. B B 1, we shall present a set-theoretical formalism of an environment that could be perceived by biotic systems. In supp. B B 2, we formulate the emergence of an Umwelt as a statistical inference problem, where probability measures are endowed on the set-theoretical formalism. A system interacts with the environment through action, and observations of the events in the environment. The observations are formalized as samples from a probability space in supp. B B 3. The formalism also formalizes the problem setting of this work, and because we shall study DNNs, the environment is simply a supervised learning problem in Statistical Learning Theory [121], where a conditional measure $\mu(y|\boldsymbol{x})$ of the supervised labels $y$ conditioned on the input instance/examples $\boldsymbol{x}$ needs to be estimated from a sample. An algorithmic formalism of Umwelt is given in supp. B B 4, which creates a probability measure space recursively from the set-theoretical formalism of an environment given in supp. B B 1. This formalism formalizes the emergence of a Umwelt as a statistical inference process on hierarchical events (cf. the emergence of hierarchical boundaries and niches previously). The probability measure space supports a set of random variables that form a hierarchy. The probability distributions of these random variables are estimated from an algorithm given from supp. B B 5 to supp. B B 7. More concretely, the algorithm estimates a probability measure composed by a series of measures that form a hierarchy, through hierarchical maximum-entropy maximization subject to constraints that characterize hierarchical event coupling—the hierarchical event coupling refers to the phenomenon that the measures in the higher scales of the hierarchy coarse-grain statistical behaviors of groups of events (or in other words, coarser-grained events) that are composed by the events in the lower scales of the hierarchy. These measures gives an estimation of the conditional measure $\mu(y|\boldsymbol{x})$, which characterizes the chances that a group of hierarchically coupled events occur.

### 1. Set-theoretical formalism of environment

In this section, we present a set-theoretic characterization of the environment that emphasizes a hierarchical structure. From this set-theoretic characterization, a probability measure space could be defined later as the Umwelt.

**Definition 1** (Perceptual Event Space; Perceptual Event). *Let $(P, \mathscr{P})$ be a measurable space, and more specifically, a Souslin space*[1] *$P$ equipped with its Borel $\sigma$-algebra $\mathscr{P}$. We refer the measurable space as the* **perceptual event space**, *and refer $E \in \mathscr{P}$ as* **perceptual events**, *or simply events.*

The definition formalizes the events perceived by the sensors of a system set-theoretically. To give an example, an event

[1] The space is defined as a Souslin space for the technical reason, for example, that we want sets created by countable set operations to be measurable. It could be understood as $\mathbb{R}^n$ without losing of critical information.

could be a particular electronically excited pattern of a CMOS, or a biotic eye, in response to photon collisions, that represents an image of an apple—thus, a digital image is also an event. And a dataset in Machine Learning is a set of events.

An event $E$ is recursively composed, and we formalize the events of the smallest scale as follows.

**Definition 2** (Event Atom)**.** *Let $(P,\mathscr{P})$ be a perceptual event space. An* **event atom***, or atoms, of $\mathscr{P}$ containing an event $p \in P$ is defined as*

$$[p]_{\mathscr{P}} := \bigcap_{p \in E \in \mathscr{P}} E. \tag{21}$$

*And the set of atoms of $\mathscr{P}$ is referred as*

$$At(\mathscr{P}) := \{[p]_{\mathscr{P}} | p \in P\}. \tag{22}$$

For example, a particular value range of a pixel in an image could be an event atom.

An event at a higher scale is composed of events at lower scales, and the events of all scales constituent the environment of a system, as defined in the following.

**Definition 3** (Events at Scale $s$)**.** *Let $\mathscr{E}_0 = At(\mathscr{P})$, which we refer as the perceptual event of scale 0. A set of perceptual events at scale $s \in \mathbb{N}$ is generated recursively as follows. Let*

$$E_i^s := \bigcup_{E \in \Omega_i \subseteq \mathscr{E}_{s-1}} E, i \in [n_s]; \tag{23}$$

*that is, $n_s \in \mathbb{N}$ sets that each is the union of events at scale $s-1$. The set of events at scale $s$ is given by*

$$\mathscr{E}_s = \{E_i^s\}_{i \in [n_s]}. \tag{24}$$

*$\mathscr{E}_s$ are referred as* **events at scale** *$s$.*

Perceived events at all scales are referred as the *environment* of the system, defined as

**Definition 4** (Environment)**.** *An* **environment** *of a system is defined as*

$$\mathscr{E} := \bigcup_{s \in \mathbb{N}} \mathscr{E}_s. \tag{25}$$

### 2. *The emergence of an Umwelt as a statistical inference problem*

All the observations made by a system compose a collection of the events in the perceptual event space. And recall that in section II A, we introduce that evolution could be interpreted as an inferential process. From this interpretation of evolution, the emergence of a Umwelt could be formalized as a statistical inference problem that estimates the probability measures of events in the environment $\mathscr{E}$, such that the uncertainty of future events are reduced. In this subsection, we give an informal introduction to the problem, where in response to certain observed coarse-grained events, the system estimates the probability measure of a hierarchy of events and represents them with random variables.

To begin with, we first clarify the stage of the statistical problem by endowing a probability measure on the perceptual event space, and refer it as the *perceptual probability space.*

**Definition 5** (Perceptual Probability Space)**.** *Let $(P,\mathscr{P})$ be a perceptual event space, a* **perceptual probability space** *is the tuple $(P,\mathscr{P},\mu)$, where $\mu$ is a probability measure on the $\sigma$-algebra $\mathscr{P}$.*

The definition formalizes the uncertainty in the inferential process probabilistically: the past observations and future observations are assumed to be realizations of a certain random variable $X$ supported on $(P,\mathscr{P},\mu)$, and the uncertainty reduction problem is formalized to estimate $\mu$. From now on, we shall assume $P = \mathbb{R}^n$ for clarity, though generally it could be any suitable function space. And $\mathscr{R}^n$ denotes the $\sigma$-algebra of $\mathbb{R}^n$.

From the perceptual probability space, a hierarchy of random variables are created, as mostly informally described in the following.

First, we represent event atoms with a random vector $X$ as follows. We refer $X$ as the random variable at scale 0.

**Definition 6** (Sensor Random Variable)**.** *Let $(\mathbb{R}^n,\mathscr{R}^n,\mu)$ be a perceptual probability space. A* **sensory random variable** *$X$ is a random variable supported on $(\mathbb{R}^n,\mathscr{R}^n,\mu)$, where an event atom $[p]_{\mathscr{P}}$ is mapped to an event $E \in \mathscr{R}^n$ such that*

$$\mu(\boldsymbol{x} \in E) = \mu([p]_{\mathscr{P}}).$$

For example, suppose that $X$ is an image, the event $E$ could characterize the event that the first pixel of the image is of value in a certain range.

Corresponding random variables at higher scales are created hierarchically/recursively as follows. To bootstrap the hierarchical process, we first create a set of random variables $\{H_i^1\}_{i \in [n_1]}$ that represent the events at scale 1, which are referred as event random variables at scale 1. A random variable $H_i^1$ is created and is of the law given as,

$$\begin{aligned} \mu(h_i^1 = 1) &= \mu(\boldsymbol{x} \in \bigcup_{E \in \Omega_i \subset \mathscr{R}^n} E) \\ \mu(h_i^1 = 0) &= \mu(\boldsymbol{x} \notin \bigcup_{E \in \Omega_i \subset \mathscr{R}^n} E). \end{aligned} \tag{26}$$

The set of random variables belong to a probability space $(\mathbb{B}^{n_1},\mathscr{B}^{n_1},\mu)$, where $\mathbb{B} := \{0,1\}$. For example, a special spatial configuration of pixels is the union of the events where the individual pixels are of certain values, and such a spatial configuration could be known as an edge. Thus, a random variable $H_i^s$ characterizes the probability of such a union of events, i.e., the probability that an edge is observed.

The event random variables at higher scales are created recursively. Let $(\mathbb{B}^{n_{s-1}},\mathscr{B}^{n_{s-1}},\mu)$ denote the probability space that support the event random variables of scale $s-1$. A probability space at scale $s$ is created such that it supports a set of random variables $\{H_i^s\}_{i \in [n_s]}$ where

$$\begin{aligned} \mu(h_i^s = 1) &= \mu(\boldsymbol{h}_{s-1} \in \bigcup_{E \in \Omega_i \subset \mathscr{B}^{n_{s-1}}} E), \\ \mu(h_i^s = 0) &= \mu(\boldsymbol{h}_{s-1} \notin \bigcup_{E \in \Omega_i \subset \mathscr{B}^{n_{s-1}}} E). \end{aligned} \tag{27}$$

And the variables belong to the probability space $(\mathscr{B}^{n_s}, \mathscr{B}^{n_s}, \mu)$. For example, through such a hierarchical procedure, $H_i^s$ could characterize the probability that a union of edges are observed, which is known as a texture of a surface. And the process goes on recursively.

Note that the preceding description is rather vague; for example, we do not discuss, (1) which group of events (i.e., subsets of $\sigma$-algebra at each scale, e.g., $\Omega_i \subset \mathscr{R}^n$ at scale 0) is represented by a random variable, and (2) how to assign numerical values to the measures. Roughly, the measures are assigned through a probability estimation procedure, from which the probability measures provide a probability estimation that agrees with co-occurrence of the observed coarse-grain events (i.e., events at relatively high scales), and the group of hierarchical events that compose the coarse-grained events.

To conclude, we have mostly informally introduced a statistical inference problem, where in response to observed coarse-grained events, a Umwelt of a system emerges from a probability estimation process where the probability measure are estimated for groups of events in the Umwelt that form a hierarchy. The formal characterization of such a process is the subject of the rest of supp. B B.

### 3. *Statistical supervised learning problem, and observed environment*

In supp. B B 2, we informally describe the process where the event random variables emerge from a statistical-inference system. And recall that the theoretical construction is to investigate the theoretical foundation of DNNs. Therefore, in this subsection, we present the problem setting of a typical supervised DNNs in statistical learning theory, which formalizes the concept of *observed environment* of the system.

**Definition 7** (Observed environment)**.** *The* **observed environment** *is a tuple $(Z, S_m)$ that consists of a random variable $Z := (X, Y)$ with an unknown law $\mu$, and a sample $S_m = \{z_i = (\boldsymbol{x}^{(i)}, y^{(i)})\}_{i \in [m]}$ of size m (i.e., observed events). X is the sensory random variable given at definition 6 in supp. B B 2, and Y is referred as the* **label random variable***.*

In this formalism, the sample of labels $\{y_i\}_{i \in [m]}$ are the observed coarse-grained events, and the sample of instances $\{\boldsymbol{x}_i\}_{i \in [m]}$ are the sensed event atoms (in other words, realizations of the sensor random variable) introduced in supp. B B 2.

In addition, an observed environment is simply a dataset in the typical sense in statistical learning. Therefore, we describe some usual notations and an assumption. let $\mathscr{X}, \mathscr{Y}$ denote the domains of the measurable spaces of $X, Y$, and are referred as *instance space* and *label space*, respectively. Also, in this work, we assume that the examples in the sample are independent realizations of random variables $Z$; that is, the examples are independently and identically distributed.

The goal of the statistical-estimation system is to obtain a probability measure that is an estimation of the true law $\mu$ from the sample $S_m$, which we turn to next.

### 4. *Umwelt: hierarchical probability measure-coarse-graining system*

As introduced in supp. B B 2, to solve the statistical learning problem given in supp. B B 3, we shall design a system that learns to organize events into groups that are represented by a set of event random variables, and the event random variable at the top scale is the label random variable given in supp. B B 3, such that the estimated law of the label random variable is a good estimation of the unknown law $\mu$. In this subsection, we present the formalism through which the event random variables are created. Also, note that a biological motivation has been discussed in section II A 2.

More specifically, the random variables $H_i^s$ in supp. B B 2 have been given as an end product that coarse-grains the probability measures of random variables of lower scales without characterizing the process where the probability space $(\mathbb{B}^{n_s}, \mathscr{B}^{n_s}, \mu)$ is created, and the process where the random variable are created on such a probability space. In this section, we characterize the procedure, which creates *extensions*[2] of the perceptual probability space defined at definition 5 that support the new random variables that we would refer as *object random variables*.

The random variables $H_i^s$ are created through a procedure that hierarchically coarse-grains probability measures of random variables of lower scales, and is formally defined as follows.

**Definition 8** (Umwelt; Hierarchical Measure-coarse-graining System)**.** *A* **Umwelt***, or more descriptively, a* **Hierarchical Measure-coarse-graining System**[3]*, is a probability measure space created by the procedure given in algorithm 1 that creates random variables hierarchically through probability space extension.*

[2] A systematic presentation of the formalism of probability space extension could be found in Thorisson [281].

[3] Algorithm 1 only characterizes a feedforward structure between random variables of different scales. However, with a graph formalism, the algorithm could further generalize to DNN architecture such as Deep Residual Neural Networks [282]. But for clarity and to simplicity, we would not pursue this direction in this work.

**Algorithm 1** Umwelt.

**Input:** A perceptual probability space $(\mathbb{R}^n, \mathscr{R}^n, \mu)$ that supports a sensory random variable $X$; an integer $S \in \mathbb{N}^+$; and a set $\{Q_s\}_{s\in[S]}$ of probability kernels.

**Output:** A perceptual probability space $(\mathbb{R}^n \otimes_{s=1}^S \mathbb{B}^{n_s}, \mathscr{R}^n \otimes_{s=1}^S \mathscr{B}^{n_s}, \mu)$ that supports a set of random variables $\{X\} \cup \{H_s\}_{s\in[S]}$.

Initialization: $P_0 \leftarrow \mathbb{R}^n, \mathscr{P}_0 \leftarrow \mathscr{R}^n, \mu_0 \leftarrow \mu, s \leftarrow 0, \mathscr{O}_0 \leftarrow \{X\}$
**while** $s <= S$ **do**
$P_{s+1} \leftarrow P_s \otimes \mathbb{B}^{n_{s+1}}, \mathscr{P}_{s+1} \leftarrow \mathscr{P}_s \otimes \mathscr{B}^{n_{s+1}}$
Extend the probability space $(P_s, \mathscr{P}_s, \mu_s)$ to $(P_{s+1}, \mathscr{P}_{s+1}, \mu_{s+1})$ that supports an object random variable $H_{s+1}$ on $(P_{s+1}, \mathscr{P}_{s+1}, \mu_{s+1})$, where

$$\mu_{s+1}(E, \boldsymbol{h}_{s+1}) := \int_E Q_s(\mathscr{O}_s, \boldsymbol{h}_{s+1}) \mu_s(d\mathscr{O}_s), E \in \mathscr{P}_s, \boldsymbol{h}_{s+1} \in \mathbb{B}^{n_{s+1}}. \tag{28}$$

$\mathscr{O}_{s+1} \leftarrow \mathscr{O}_s \cup \{H_{s+1}\}$
$s \leftarrow s+1$
**end while**

**Remark 1** (Measure coarse-graining and coupling)**.** *For conceptual clarity, we refer the procedure, where the probability measure of a new random variable supported on extended probability space is obtained through eq.* (28)*, as* **measure coarse-graining***. And we refer the relationship characterized by $Q_s$ among $H_{s+1}$ and $\mathscr{O}_s$ as* **coupling***.*

Note that the extension of probability space created by a Umwelt still satisfies the definition of perceptual probability space, and thus is still a perceptual probability space. The new perceptual space formalizes the previous relationship between the probability measure space of perceptual events of different scales described in supp. B B 2. Also, note that the probability kernels $\{Q_s\}_{s\in[S]}$ are unspecified. A kernel $Q_s$ characterize the coupling among $H_{s+1}$ and $\mathscr{O}_s$, such that the integration over $\mathscr{O}_s$ is coarse-graining. The kernels are specified in supp. B B 5.

We refer the random variables created by a Umwelt as object random variables, and to emphasize we give the following definition.

**Definition 9** (Object Random Variable)**.** *Let $(P, \mathscr{P}, \mu)$ be a perceptual probability space created by a Umwelt. The random variable $\{H_s\}_{s\in[S]}$ supported on $(P, \mathscr{P}, \mu)$ are referred as* **object random variables***, and $H_s$ are referred as object random variables of scale $s$.*

We elaborate the definition of Umwelt with object random variables of scale 1. Let $n_1 \in \mathbb{N}^+$, and $Q(\cdot,\cdot)$ be a $((\mathbb{R}^n, \mathscr{R}^n), (\mathbb{B}^n, \mathscr{B}^n)))$ probability kernel. Then, according to definition 8, an extended probability space $(\bar{P}, \bar{\mathscr{P}}, \bar{\mu})$ of $(\mathbb{R}^n, \mathscr{R}^n, \mu)$ is given as

$$\begin{aligned} \bar{P} &:= P \otimes \mathbb{B}^{n_1}, \\ \bar{\mathscr{P}} &:= \mathscr{P} \otimes \mathscr{B}^{n_1}, \\ \bar{\mu}(E, \boldsymbol{h}) &:= \int_E Q(\boldsymbol{x}, \boldsymbol{h}) \mu(d\boldsymbol{x}), E \in \mathscr{P}, \boldsymbol{h} \in \mathbb{B}^{n_1}. \end{aligned} \tag{29}$$

And it supports an object random variable $H$ whose joint distribution with $X$ is given by $\bar{\mu}$. Note that the marginal probability of $H$ is computed through

$$\int_{\mathbb{R}^n} \bar{\mu}(\boldsymbol{x}, \boldsymbol{h}) d\boldsymbol{x} = \int_{\mathbb{R}^n} Q(\boldsymbol{x}, \boldsymbol{h}) \mu(d\boldsymbol{x}),$$

and thus each object random variable integrates over a continuous range of possible sensor random variable values; that is, an integration over the measure of a set of event atoms. Therefore, the measure of event union in eq. (26) is characterized by the integration in eq. (29), and an object random variable coarse-grains over sensory random variables, which represents the co-occurrence of a set of event atoms—for example, a spatial configuration of pixels known as an edge.

### 5. *Umwelt emergence through hierarchical maximum entropy learning*

In this subsection, we describe a design of the probability kernels based on the maximum entropy principle [283] that would derive DNNs.

To begin with, we discuss the design of the probability kernels at a high level. At each scale $s$, the possible events $\mathscr{E}_s$ in a Umwelt is exponentially large because an exponential number of configurations of event at scale $s-1$ exist to compose an event $E_i^s$ at scale $s$; and the size of samples is limited to estimate probability measures of all $E \in \mathscr{E}_s$. Thus, it is efficient, and also perhaps the only tractable way, to only estimate the probability of co-occurrence of event groups that are observed, and are relevant to the system. Meanwhile, the observed events are decomposed into a hierarchy of events of smaller scales, and the probability estimation process estimates not only the probability measure $\mu_S$ that assigns a probability to the events at the scale of the observed event, but also a hierarchy of probability measures $\{\mu_s\}_{s\in[S]}$ that assign probability to a hierarchy of events that compose the observed events. These preceding ideas are implemented through the probability kernels $Q_s(\mathscr{O}_s, \boldsymbol{h}_{s+1})$ in algorithm 1, which we describe as follows.

The probability kernels of a Umwelt are estimated by solving a series of probability estimation problems that maximize entropy subjecting to constraints that characterize the coupling among object and sensor random variables. And for clarity, we define it as the *enclosed maximum entropy problem* as follows, reflecting that random variables in a Umwelt characterize sub-systems with their own internal dynamics.

**Definition 10** (Enclosed Maximum Entropy Problem)**.** *Let $(P, \mathscr{P}, \mu)$ be a perceptual probability space created by a Umwelt. Recall that $\mu$ could be factorized into conditional probabilities as*

$$\mu(\mathscr{O}_S) = \prod_{s=1}^S \mu_s(\boldsymbol{h}_s | \mathscr{O}_{s-1}),$$

*where $\mu_s(\boldsymbol{h}_s|\mathscr{O}_{s-1}) = Q_{s-1}(\mathscr{O}_{s-1}, \boldsymbol{h}_s)$. Each $\mu_s(\boldsymbol{h}_s|\mathscr{O}_{s-1})$ is estimated by solving an entropy maximization problem, referred as* **enclosed maximum entropy problem***, given as follows.*

$$\max - \sum_{\boldsymbol{h}_s \in \mathbb{B}^{n_s}} \mu_s(\boldsymbol{h}_s|\mathscr{O}_{s-1}) \log \mu_s(\boldsymbol{h}_s|\mathscr{O}_{s-1})$$

*subject to*

$$\sum_{\boldsymbol{h}_s \in \mathbb{B}^{n_s}} \mu_s(\boldsymbol{h}_s|\mathscr{O}_{s-1}) = 1$$

$$\mathbb{E}_{\mu_s(\boldsymbol{h}_s|\mathscr{O}_{s-1})}[\prod_{s'=1}^{s} h^{s'}_{i_{s'}} x_{i_0}] = \tau^s_{\boldsymbol{i}}, \forall \boldsymbol{i} \in \otimes^s_{s'=0}[n_{s'}], \tag{30}$$

*where* $\{\tau^s\}_{\boldsymbol{i}\in\otimes^s_{s'=0}[n_{s'}]}, \tau^s \in \mathbb{R}$ *parameterizes the coupling among random variables, and* $n_s \in \mathbb{N}^+$ *is the number of object random variable, that each represents an event at scale s, as described in supp. B B 2.*

*Furthermore, the conditional measure of the top-scale object random variable* $\mu_S(\boldsymbol{h}_S|\boldsymbol{x})$ *is the parametric estimation of the conditional law* $\mu(y|\boldsymbol{x})$*, where* $Y, X$ *are label random variable and sensory random variable, respectively, given in supp. B B 3.*

We elaborate the equality constraints eq. (30) with the simple example where $s = 1$. In this case eq. (30) is given as

$$\mathbb{E}_{\mu_1(\boldsymbol{h}_1|\boldsymbol{x})}[h^1_{i_1} x_{i_0}] = \tau^1_{i_1 i_0}, \forall i_0 \in [n_0], i_1 \in [n_1].$$

Recall that in supp. B B 2, we have described at eq. (26) that the goal is to assign measure to $H_1$ such that

$$\mu(h^1_i = 1) = \mu(\boldsymbol{x} \in \bigcup_{E\in\Omega_i\subset\mathscr{R}^n} E).$$

Given a sample $\{H^{(j)}, X^{(j)}\}_{i\in[m]}, m \in \mathbb{N}^+$ of $H_1, X$—where parenthesized upper indices are used to distinguish it from scale indices—a set of examples $\{X^{(j)}\}_{j\in I\subseteq[m]}$ would co-occur with an event $H^1_{i_1} = 1$ (i.e., $\forall j \in I, (H^1_{i_1})^{(j)} = 1$). For example, $\{X^{(j)}\}_{j\in I}$ could be variants of edges of a certain orientation. Then, the left side of eq. (30) computes the average of the set $\{X^{(j)}\}_{j\in I}$ (e.g., the average "shape" of the edges), that characterizes the statistical coupling between $X_{i_0}$ and $H^1_{i_1}$. More concretely, first, notice that,

$$\mathbb{E}_{\mu_1(\boldsymbol{h}_1|\boldsymbol{x})}[H^1_{i_1} X_{i_0}] = \mu_1(h^1_{i_1} = 1|\boldsymbol{x}) x_{i_0}.$$

Suppose that the edge does not want that pixel, when the event of such an edge occurs (i.e., $H^1_i = 1$), $x_{i_0}$ should be close 0; on the other hand, when $x_{i_0}$ is nonzero, $\mu_1(h^1_{i_1} = 1)$ is close to 0 because the probability that edge co-occurs with nonzero $x_{i_0}$ is small; as a result, the multiplication $\mu_1(h^1_{i_1} = 1|x_{i_0}) x_{i_0}$, or the average $\mathbb{E}_{\mu_1(\boldsymbol{h}_1|\boldsymbol{x})}[H^1_{i_1} X_{i_0}]$ is small. Through such equality constraints, statistical coupling between sensor random variables and object random variables are enforced, where multiple realizations of $X_{i_0}$ are coupled with the event $H^1_{i_1} = 1$, and thus the events $E \in \mathscr{R}^n$ are grouped into a coarse-grained event $H^1_{i_1}$; and the coupling would be reflected in the solution $\mu_1$ to the problem.

However, we do not give how the parameters $\{\tau^s_{\boldsymbol{i}}\}_{s\in[S],\boldsymbol{i}\in\boldsymbol{i}\in\otimes^s_{s'=0}[n_{s'}]}$ are obtained—notice that in the supervised learning problem given in supp. B B 3, the intermediate object random variables $H_s, 0 < s < S$ are not observed. These parameters are specified in supp. B B 7, after we discuss the dual problem of the maximum entropy problem in supp. B B 6.

Consequently, the solution $\mu_S(\boldsymbol{h}_S)$ to the recursive composed problem characterizes the chances that a group of hierarchically coupled events occur, and the conditional measure $\mu_S(\boldsymbol{h}_S|\boldsymbol{x})$ is a parametric estimation of the conditional measure $\mu(y|\boldsymbol{x})$. Therefore, to estimate a conditional measure $\mu(y|\boldsymbol{x})$, the system estimates a hierarchy of conditional measures that characterize the co-occurrence of the observed coarse-grain events (i.e., events at relatively high scales), and the group of hierarchical events that compose the coarse-grained events (cf. supp. B B 2).

### 6. *Dual problem of maximum entropy problem, and exponential family distributions*

We shall present a learning algorithm of Umwelt in supp. B B 7 that solves the hierarchy of enclosed maximum entropy problems through solving their *dual* problems. Therefore, before presenting the learning algorithm, we introduce the dual problem, and the associated exponential family distributions, in this subsection.

The enclosed maximum entropy problem defined at definition 10 is a classic statistical problem whose solution belongs to the well known exponential families [54]. The proof is the same with the classic maximum entropy problem with equality constraints—the difficulty here lies in identifying the problem, not getting the solution—and thus we state the result as a lemma, and refer readers to the proof in, for example, Cover and Thomas [284, Chp 12].

**Lemma 1.** *The solution to the enclosed maximum entropy problem defined at definition 10 is of the following parametric form:*

$$\mu_s(\boldsymbol{h}_s|\mathscr{O}_{s-1}) = \frac{1}{Z} e^{\sum_{\boldsymbol{i}\in\otimes^s_{s'=0}[n_{s'}]} \lambda^s_{\boldsymbol{i}} \prod^s_{s'=1} h^{s'}_{i_{s'}} x_{i_0}}, \tag{31}$$

*where*

$$Z = \sum_{\boldsymbol{h}_s\in\mathbb{B}^{n_s}} e^{\sum_{\boldsymbol{i}\in\otimes^s_{s'=0}[n_{s'}]} \lambda^s_{\boldsymbol{i}} \prod^s_{s'=1} h^{s'}_{i_{s'}} x_{i_0}}, \lambda^s_{\boldsymbol{i}} \in \mathbb{R}. \tag{32}$$

Note that in eq. (31), the variables in $\mathscr{O}_{s-1}$—that is, the variables other than $\boldsymbol{h}_s$—are given, instead of variables because $\mu_s(\boldsymbol{h}_s|\mathscr{O}_{s-1})$ conditions on $\mathscr{O}_{s-1}$. It is a classic result that an one-to-one mapping exists between $\tau^s_{\boldsymbol{i}}$ and $\lambda^s_{\boldsymbol{i}}$ (e.g., Wainwright and Jordan [54, Theorem 3.3]) under some regular conditions[4]. Therefore, the coarse-grained measures characterized by the equality constraints in definition 10 are of the exponential family parameterized by the $\{\lambda^s_{\boldsymbol{i}}\}_{\boldsymbol{i}\in\otimes^s_{s'=0}[n_{s'}]}$.

Under the same condition that ensures the preceding one-to-one mapping, the measure $\mu_s$ that solves an entropy maximum

---

[4] Because our Umwelt is actually parameterized by $\lambda^s_{\boldsymbol{i}}$ instead of $\tau^s_{\boldsymbol{i}}$, and thus the probability measure are restricted to the ones that have such one-to-one mapping, the satisfaction of the conditions is automatic. Therefore, we do not digress to discuss the conditions.

problem in definition 10 also solves the maximum-likelihood problem—and vice versa—given as follows (see, e.g., Wainwright and Jordan [54, section 3.4.2], for details),

$$\max_{\{\lambda_{\boldsymbol{i}}^s\}_{\boldsymbol{i}\in\otimes_{s'=0}^{s}[n_{s'}]}} \sum_{i=1}^{m} \log \mu_s(\boldsymbol{h}_s|\mathscr{O}_{s-1}), \tag{33}$$

where $m$ is the size of the sample. And note that the problems given in definition 10 correspond to a hierarchy of maximum-likelihood problems. Those two problems are called dual problems of each other.

### 7. *Learning of Umwelt*

In this subsection, we present an algorithm that estimate the laws of the object random variables of an Umwelt such that the marginal $\mu_S(\boldsymbol{h}_S|\boldsymbol{x})$ is an estimation of the conditional probability measure $\mu(y|\boldsymbol{x})$ of a dataset/environment (cf. supp. B B 3). Meanwhile, we only describe the algorithm at a high level; in the next section, we shall give a particular implementation of the algorithm that is the forward and backward propagation of DNNs. The algorithm is given as algorithm 2.

**Algorithm 2** Learning algorithm of Umwelt.

**Input:** A sample $S_m = \{z_i = (\boldsymbol{x}^{(i)}, y^{(i)})\}_{i=1,\dots,m}$ whose examples are independent realizations of a random variable $Z := (X,Y)$ with an unknown law $\mu$; a loss function $\mathscr{L}$; the maximal scale $S$.
**Output:** A set of probability measures $\{\mu_s\}_{s\in[S]}$, where $\mu_S(\boldsymbol{h}_s|\boldsymbol{x})$ is a parametric estimation of $\mu(y|\boldsymbol{x})$.

Initialization: $(P, \mathscr{P}, \mu) \leftarrow$ Umwelt$((\mathbb{R}^n, \mathscr{R}^n, \mu), X)$, where the probability kernels are $\{\mu_s\}_{s\in[S]}$ given in lemma 1, and the parameters $\lambda_{\boldsymbol{i}}^s$ in $\mu_s$ are randomly initialized (e.g., sampled from Gaussian distributions).
**while** not converge **do**
  Compute the loglikelihood of $\mu_S(\boldsymbol{h}_S|\boldsymbol{x})$.
  Maximize the loglikelihood of $\mu_S(\boldsymbol{h}_S|\boldsymbol{x})$.
**end while**

The algorithm also puts together the pieces developed in previous subsections to describe the emergence of an Umwelt, which we summarize as follows. An Umwelt emerges by learning, or technically, estimating a conditional probability measure $\mu(y|\boldsymbol{x})$ from the sample $S_m$ of random variable $Z := (X,Y)$ (summary of supp. B B 3). More concretely, it first extends the probability space of sensor random variable $X$ to support a set of object random variables $\{H_s\}_{s\in[S]}$ that coarse-grain measures from events represented by $X$, through algorithm 1 given in supp. B B 4. Then, the laws of the object random variables are estimated through a hierarchy of enclosed maximum entropy problem described at definition 10 in supp. B B 5. The hierarchy of maximum entropy problems are solved by solving their dual problems, which maximize the loglikelihood of the laws of the object random variables. More specifically, at initialization, for each scale $s$, object random variables in $H_s$ randomly coarse-grain events from the previous scales, which is implemented by randomly initializing the parameters (i.e., Lagrange multipliers) $\lambda_{\boldsymbol{i}}^s$ of the exponential-family distributions given in lemma 1 in supp. B B 6. Then, because the goal is only to compute a $\mu_S(\boldsymbol{h}_S|\boldsymbol{x})$ that estimates $\mu(y|\boldsymbol{x})$, only loglikelihood of $\mu_S(\boldsymbol{h}_S|\boldsymbol{x})$ is maximized; that is, a probability measure is estimated such that it would give maximal likelihood to the sample $S_m$. Correspondingly, the $\{\lambda_{\boldsymbol{i}}^s\}_{s<S}$ of lower scales are modified to maximize $\mu_S(\boldsymbol{h}_S|\boldsymbol{x})$ instead of being modified to maximize $\mu_s(\boldsymbol{h}_s|\mathscr{O}_{s-1})$. Actually, there is no such $\mu_s(\boldsymbol{h}_s|\mathscr{O}_{s-1})$ to maximize because no ground truth on $\{H_s\}_{s<S}$ is available, and the optimization of $\{\lambda_{\boldsymbol{i}}^s\}_{s<S}$ to maximize $\mu_S(\boldsymbol{h}_S|\boldsymbol{x})$ should be understood as a statistical inference that infers hierarchical event coupling that best maximizes the likelihood of the observed coarse-grained random variables $H_S$—any values of the $\{\lambda_{\boldsymbol{i}}^s\}_{\boldsymbol{i}\in\otimes_{s'=0}^{s-1}[n_{s'}]}$ parameterize an exponential-family distribution that satisfies a set of hierarchical-coupled constraints. At a high level, the maximization is implemented as an iterative algorithm: first, the marginal $\mu_S(\boldsymbol{h}_S|\boldsymbol{x})$ (i.e., likelihood estimated from the current parameters) is computed, and maximized; then another iteration repeats, if the optimization has not converged. However, the computation of $\mu_S(\boldsymbol{h}_S|\boldsymbol{x})$ is intractable, and thus approximation is needed. A particular approximation scheme is implemented by DNNs, which is the subject of supp. B C.

## C. Stochastic, or Bayesian-probabilistic-graphical, definition of DNNs

In supp. B C, we show that the training of a DNN with ReLU activation function [95], the most widely used activation function, could be interpreted as an expectation-maximization algorithm that implements the probability-estimation/learning algorithm of Umwelt given in supp. B B.

More specifically, in supp. B C 1, we review the conventional functional definition of DNNs in the supervised learning setting. In supp. B C 2, we show that a DNN with ReLU activation function is a Umwelt with a hierarchical parameterization that estimates probability measures through dynamical programming. In supp. B C 3, we show that the forward propagation of a DNN does approximate inference that computes marginals of random variables in a Umwelt through (degenerate) Monte Carlo sampling. In supp. B C 4, we show that the back-propagation of a DNN maximizes the approximate loglikelihood obtained by forward propagation: the loglikelihood maximization is the dual problem of the maximum entropy problem of a Umwelt and the optimal solutions to these two problems are of the same objective value (risk). In supp. B C 5, we explain that the forward and backward propagation is an expectation-maximization algorithm that maximizes a parametric estimation of $\mu(y|\boldsymbol{x})$—the parametric estimation characterizes a hierarchical coupling between $Y$ and $X$, and this aspect has been introduced in section II A 2. After identifying the mapping between a DNN and a Umwelt, we give the stochastic definition of DNNs in supp. B C 6 that defines a DNN as a multi-layer probabilistic graphical model, which more specifically is a hybrid of Markov random field and Bayesian network. This definition characterizes the statistical aspects of DNNs, in addition to the functional aspects in the conventional definition. In supp. B C 7, we discuss the relationship between

the hierarchical maximum entropy problem that derives DNNs, and the DNNs trained with arbitrary risk functions. Lastly, in supp. B C 8, we present the class of loss functions that shall be studied in this work.

### 1. Conventional functional definition of supervised DNNs

The conventional definition of DNNs is a functional definition—the "functional" here refers to the mathematical denotation as in functional analysis. In this section, we present the conventional definition of DNNs under the setting of supervised learning with the simplest DNN, Multiple Layer Perceptron (MLP), to contrast with stochastic definition given in this section.

*a. Functional definition of DNNs.* A MLP conventionally is defined as a map that takes an input, and computes its output by recursively applying a linear map followed by a pointwise non-linear function; the map is formally given as follows. Suppose that the recursion has been taken $L$ times and $L \in \mathbb{N}^+$. We index each recursion by an integer $l$ and $l \in \mathbb{L}, \mathbb{L} := \{0, \ldots, L\}$. Each recursion is referred as a *layer*. The output of layer $l-1$ is fed to layer $l$ as the input, which is formally given as the equation

$$\boldsymbol{x}_l := g(\boldsymbol{W}_l^T \boldsymbol{x}_{l-1}), \quad (34)$$

where $\boldsymbol{x}_{l-1}$ denotes the input (which is also the output of layer $l-1$), $\boldsymbol{W}_l \in \mathbb{R}^{n_{l-1} \times n_l}$ the linear map, $g : \mathbb{R} \to \mathbb{R}$ the point-wise nonlinear function, and $\boldsymbol{x}_l \in \mathbb{R}^{n_l}, n_l \in \mathbb{N}^+$ the output of layer $l$; $\boldsymbol{x}_0$ is also denoted as $\boldsymbol{x}$, which denotes the input to the network. The recursion process composes a MLP, and we compactly write it as

$$T(\boldsymbol{x}; \theta) = \boldsymbol{W}_L^T g(\boldsymbol{W}_{L-1}^T \ldots g(\boldsymbol{W}_1^T \boldsymbol{x})), \quad (35)$$

where $\theta := \{\boldsymbol{W}_i\}_{i \in [L]}$, or simply

$$T\boldsymbol{x},$$

when we do not emphasize the parameters of $T$.

*b. Terminologies.* The preceding notations each has its colloquial names. Layer 0 is referred as the *bottom* layer, layer $L$ as the *top* layer, and the layers whose indexes are between 0 and $L$ as the *intermediate* layers. The number of layer $L$ is called the *depth* of the DNN, and the number of neurons at a layer is called the *width* of that layer. The parameters of linear maps are referred as *weights*. The nonlinear function $g$ is referred as the *activation* function. And the input $\boldsymbol{W}_l^T g(\boldsymbol{W}_{l-1}^T \ldots g(\boldsymbol{W}_1^T \boldsymbol{x}))$ to the activation function $g$ is referred as the *pre-activation* at layer $l$. A component $x_{li}$ of $\boldsymbol{x}_l$ is referred as a *neuron*—this is the conventional definition of neurons, and this definition shall be overridden later when we present a stochastic definition of neuron at definition 12 in supp. B C 6; $\boldsymbol{x}$ at the bottom layer is referred as *input* neurons; and $\boldsymbol{x}_L$ at the top layer as *output* neurons. $\{\boldsymbol{W}_l\}_{l \in [L]}$ are referred as *weight matrices*.

*c. Supervised learning of DNNs.* We shall study DNNs in the supervised setting, and in such a setting, a DNN is trained to approximate a function (or technically a mapping when the DNN has more than one output neurons) implicitly given in a dataset by the back-propagation algorithm [285] that adjusts the weights of the DNN by computing and back-propagating the discrepancy between the output neurons and the labels of data measured by a certain loss function; the process is formally presented as follows. The function is given implicitly in the form of a set of examples $\{(\boldsymbol{x}^{(i)}, y^{(i)})\}_{i=1,\ldots,m}$, where $\boldsymbol{x}^{(i)}$ is referred as an instance/example, $y^{(i)}$ as a label, and $m \in \mathbb{R}$ is the number of the examples, or the size of the dataset. Suppose that $\mathscr{L}$ is a loss function, the discrepancy is computed as

$$\mathscr{L}(T\boldsymbol{x}, y); \quad (36)$$

for example, suppose that $\mathscr{L}$ is the hinge loss, we have

$$\mathscr{L}(T\boldsymbol{x}, y) = \max(0, 1 - yT\boldsymbol{x}), \quad (37)$$

where both $T\boldsymbol{x}$ and $y$ are scalars—in this case, $\boldsymbol{W}_L$ degenerates into a vector. The training process minimizes the empirical expectation of the loss computed on each example, which is formally given as

$$\min_{\theta} R_m(T) \quad (38)$$

where

$$R_m(T) := \sum_{i=1}^{m} \mathscr{L}\left(T\boldsymbol{x}^{(i)}, y^{(i)}\right).$$

### 2. Hierarchical parameterization of Umwelt

The definition of Umwelt allows a large parameter space where probability kernels could parameterize probability measures. Nonetheless, we aim to study DNNs in this work, and thus in this section, we present a particular parameterization that would derive DNNs later.

Recall that in algorithm 2, at each scale, the parameters $\lambda_{\boldsymbol{i}}^s$ of the probability kernels $\mu_s(\boldsymbol{h}_s|\mathscr{O}_{s-1})$ are tensors. We reparameterize the tensors into products of scalars as follows.

$$\lambda_{\boldsymbol{i}}^s = \prod_{s=1}^{s} w_{i_{s-1}i_s}^s, \quad (39)$$

where $w_{i_{s-1}i_s}^s \in \mathbb{R}, i_{s-1} \in [n_{s-1}], i_s \in [n_s]$. Note that parameters are reused in the reparameterization given in eq. (39). For example,

$$\lambda_{\boldsymbol{i}}^{s+1} = w_{i_s i_{s+1}} \lambda_{\boldsymbol{i}_{:s+1}}^s.$$

Thus, $\lambda_{\boldsymbol{i}}^{s+1}$ are parameterized in reference to $\lambda_{\boldsymbol{i}}^s$. We refer the parameterization as *hierarchical* parameterization.

As a result, $\mu_s(\boldsymbol{h}_s|\mathscr{O}_{s-1})$ in eq. (31) is reparameterized as

$$\mu_s(\boldsymbol{h}_s|\mathscr{O}_{s-1}) = \frac{1}{Z} e^{\sum_{\boldsymbol{i} \in \otimes_{s'=0}^{s}[n_{s'}]} \prod_{s'=1}^{s} h_{i_{s'}}^{s'} w_{i_{s'-1}i_{s'}}^s x_{i_0}}. \quad (40)$$

Collecting the scalars into matrices, we have

$$\mu_s(\boldsymbol{h}_s|\mathcal{O}_{s-1}) = \frac{1}{Z}e^{\boldsymbol{x}^T \overrightarrow{\Pi}_{s'=1}^{s} \boldsymbol{W}_{s'}\mathrm{dg}(\boldsymbol{h}_{s'})}. \tag{41}$$

The reparameterization restricts the parameter space to a particular subset of $\mathbb{R}^{\times_{s=0}^{s} n_s}$. As a result, we might speculate that it restricts $\mu_s$ to a particular submanifold immersed in the manifold that corresponds to the exponential family parameterized by the unrestricted $\lambda_{\boldsymbol{i}}^s$. However, we would not study this informational-geometrical aspects of $\mu_s$, and the restriction is motivated by the fact that it would derive DNNs.

### 3. *Forward propagation as approximation inference*

In this section, we show that ReLU activation function [95] of DNNs could be understood as approximate inference in the Umwelt parameterized by the hierarchical parameterization given in supp. B C 2. More specifically, the forward propagation of DNNs could be understood as approximate inference of the marginal of object random variables of Umwelt, given an observed signal/datum; and thus is an implementation the step that computes loglikelihood in algorithm 2.

To begin with, we note that we have used $s$ to denote the scale of object random variables of Umwelt, and $l$ to denote the layer of a DNN. Formally, they are both simply integers. The different notations have been to emphasize that after each recursion of measure coarse-graining in algorithm 1, the object random variable $H_s$ represents object of a higher scale than the ones represented by $H_{s-1}$ before the recursion. Because in the rest of supp. B C, we shall show that DNNs are Umwelts, we shall use $l$ to denote different scales to relate to the conventional definition of DNNs, and when we say object random variables of layer $l$, it means the same with object random variable of scale $l$.

Recall that in the conventional definition of DNNs in supp. B C 1, an activation function is a nonlinear function that transforms input of a layer nonlinearly. Particularly, the most widely used activation function, ReLU, transforms input of layer $l$ as follows.

$$\mathrm{ReLU}(\boldsymbol{W}_l^T \boldsymbol{x}_{l-1})_i := \begin{cases} (\boldsymbol{W}_l^T \boldsymbol{x}_{l-1})_i, & \text{if } (\boldsymbol{W}_l^T \boldsymbol{x}_{l-1})_i > 0 \\ 0, & \text{otherwise.} \end{cases} \tag{42}$$

In the following, we show that eq. (42) could be understood as an entangled transformation that combines two operations into one that computes an approximation of the $\mu_l(\boldsymbol{h}_l|\mathcal{O}_{l-1})$: first, a Monte Carlo sample of $H_l$ is made; then the logit (i.e., $\boldsymbol{x}^T \overrightarrow{\Pi}_{l'=1}^{l} \boldsymbol{W}_{l'}\mathrm{dg}(\boldsymbol{h}_{l'})$ in eq. (41)) of $\mu_l(\boldsymbol{h}_l|\mathcal{O}_{l-1})$ is computed.

First, we motivate the approximate inference of the marginal of $H_l$ given a datum $\boldsymbol{x}$. Note that $\mu_l(\boldsymbol{h}_l|\mathcal{O}_{l-1})$ is a measure conditioned on $\mathcal{O}_{l-1}$. To compute $\mu_l$, random variables in $\mathcal{O}_{l-1}$ need to be observed. Recall that $\mathcal{O}_{l-1} := \{H_{l'}\}_{l' \in [l-1]} \cup \{X\}$. Let us assume that $\{H_{l'}\}_{l' \in [l-2]} \cup \{X\}$ are observed. As a consequence, $\mu_{l-1}(\boldsymbol{h}_{l-1}|\mathcal{O}_{l-2})$ is known. Ideally, we would like to compute the marginal of $H_l$ by the following weighted average

$$\mu_l(\boldsymbol{h}_l|\boldsymbol{x}) = \sum_{\boldsymbol{h}_{l-1} \in \mathbb{B}^{n_{l-1}}} \mu_l(\boldsymbol{h}_l|\boldsymbol{h}_{l-1}, \mathcal{O}_{l-2}) \mu_{l-1}(\boldsymbol{h}_{l-1}|\mathcal{O}_{l-2}).$$

However, the computation involves $2^{n_{l-1}}$ terms, and is intractable. To approximate the weighted average, we sample a sample of $H_{l-1}$ from $\mu_{l-1}$. When the weight matrices $\boldsymbol{W}_{l-1}$ are large in absolute value, the sampling would degenerate into a deterministic behavior. More specifically, let $\boldsymbol{W}_{l-1} := \frac{1}{T}\hat{\boldsymbol{W}}_{l-1}$, where $T \in \mathbb{R}$, and $\hat{\boldsymbol{W}}_{l-1}$ is a matrix whose norm (e.g., Frobenius norm) is 1. When $T \to 0$, the sampled $H_i^l$ would simply be determined by the sign of $\boldsymbol{x}^T \overrightarrow{\Pi}_{l'=1}^{l-1} \boldsymbol{W}_{l'}\mathrm{dg}(\boldsymbol{h}_{l'})\boldsymbol{W}_l$—$T$ could be appreciated as a temperature parameter that characterizes the noise of the inference. Let $\boldsymbol{x}_{l-1} := \boldsymbol{x}^T \overrightarrow{\Pi}_{l'=1}^{l-1} \boldsymbol{W}_{l'}\mathrm{dg}(\boldsymbol{h}_{l'})$, then we have

$$\boldsymbol{h}_i^l := \begin{cases} 1, & \text{if } (\boldsymbol{W}_l^T \boldsymbol{x}_{l-1})_i > 0 \\ 0, & \text{otherwise.} \end{cases} \tag{43}$$

Correspondingly, $\mu_{l-1}(\boldsymbol{h}_{l-1}|\mathcal{O}_{l-2})$ becomes a Dirac delta function on a certain $\hat{\boldsymbol{h}}_{l-1}$ given by eq. (43). Correspondingly, marginal $\mu(\boldsymbol{h}_l|\boldsymbol{x})$ of $H_l$ given $\boldsymbol{x}$ degenerated into $\mu(\boldsymbol{h}_l|\hat{\boldsymbol{h}}_{l-1}, \mathcal{O}_{l-2})$, which is

$$\frac{1}{Z}e^{\boldsymbol{x}^T \overrightarrow{\Pi}_{l'=1}^{l} \boldsymbol{W}_{l'}\mathrm{dg}(\boldsymbol{h}_{l'})}. \tag{44}$$

The previous computation is exactly what ReLU does. To see it more clearly, we rewrite ReLU as the product of the realization of object random variable $H_l$ and $\boldsymbol{W}_l^T \boldsymbol{x}_{l-1}$,

$$\mathrm{ReLU}(\boldsymbol{W}_l^T \boldsymbol{x}_{l-1}) := \mathrm{dg}(\boldsymbol{h}_l)\boldsymbol{W}_l^T \boldsymbol{x}_{l-1}.$$

ReLU first computes a Monte Carlo sample of $H_l$, and then computes the logit of eq. (44). Therefore, ReLU first computes an approximate inference of $\mu_l(\boldsymbol{h}_l|\mathcal{O}_{l-1})$, and then computes to prepare for the inference of $\mu_{l+1}(\boldsymbol{h}_{l+1}|\mathcal{O}_l)$ at next layer.

To conclude, the approximate inference is executed recursively from the first layer to the last layer. Therefore, the forward propagation of a DNN with ReLU activation function computes an approximate inference of the marginal $\mu_L(\boldsymbol{h}_L|\boldsymbol{x})$ of the top layer object random variable $H_L$ of a Umwelt, by estimating the realizations of $\{\boldsymbol{h}_l\}_{l<L}$, and approximating $\mu_L(\boldsymbol{h}_L|\boldsymbol{x})$ with $\mu_L(\boldsymbol{h}_L|\mathcal{O}_{L-1})$.

### 4. *Back propagation maximizes approximate loglikelihood*

The back-propagation of DNNs maximizes the approximated likelihood computed by the forward propagation as follows. The approximate inference described in supp. B C 3 approximates the marginal $\mu_l(\boldsymbol{h}_l|\boldsymbol{x}), l \in [L]$ with $\mu_l(\boldsymbol{h}_l|\mathcal{O}_{l-1})$. Recall that the goal is to maximize the loglikelihood of $\mu_L(\boldsymbol{h}_L|\boldsymbol{x})$. Therefore, we want to achieve maximally possible $\mu_L(\boldsymbol{h}_L|\mathcal{O}_{L-1})$ by not only changing the weight $\boldsymbol{W}_L$ at layer $L$, but also changing the hierarchical coupling parameterized

by $\{\boldsymbol{W}_l\}_{l\in[L-1]}$. That is, the optimization of the following objective function,

$$\max_{\theta} \sum_{i\in[m]} \log \mu_L(\boldsymbol{h}_L^{(i)}|\mathscr{O}_{L-1}^{(i)}). \tag{45}$$

For clarity, suppose that $n_L = 1$—that is, we are solving a binary classification problem—then eq. (45) is exactly the optimization problem where a DNN minimizes a logistic risk function. The optimization decreases the KL divergence between $\mu_L(\boldsymbol{h}_L|\mathscr{O}_{L-1})$ and $\mu(y|\boldsymbol{x})$—recall that $H_L$ is $Y$.

### 5. *Forward and backward propagation is expectation-maximization algorithm*

Therefore, the optimization of DNNs implements a classic *generalized expectation maximization* algorithm [96, section 9.4] that maximizes the loglikelihood that involves latent variables and is intractable to compute exactly. More specifically, first, the approximation inference discussed in supp. B C 3, implemented by forward propagation, maximizes $\mu_l(\boldsymbol{h}_l|\mathscr{O}_{l-1})$ by estimating realizations of $H_l$ while keeping the parameters $\boldsymbol{W}_l$ fixed. And in the degenerated low temperature setting, the Monte Carlo sample is the expectation of $H_l$. The forward propagation maximizes a lower bound of $\mu_L(\boldsymbol{h}_L|\boldsymbol{x})$[5]. Then, the approximated loglikelihood of $\mu_L(\boldsymbol{h}_L|\mathscr{O}_{L-1})$ is increased by modifying all weights $\{\boldsymbol{W}_l\}_{l\in[L]}$ through gradient descent, while keeping $\{\boldsymbol{h}_l\}_{l\in[L]}$ fixed, which is the back-propagation and is discussed in supp. B C 4. This step decreases the KL divergence between $\mu_L(\boldsymbol{h}_L|\mathscr{O}_{L-1})$ and $\mu(y|\boldsymbol{x})$. Afterwards, the iteration starts again until a local minimum is reached. As explained in supp. B B 7, this optimization optimizes for hierarchical coupling of events represented by $\{H_l\}_{l\in[L]}$ that maximizes the loglikelihood of $\mu_S$ upon the sample $S_m$.

### 6. *Stochastic definition of DNNs*

The development so far has characterized a DNN as a statistical inference system, or, to emphasize the intricate mechanism, as an Umwelt. To appreciate the development, we compare the characterization with the conventional functional characterization of DNNs given in supp. B C 1. The functional definition characterize a DNN as a functional approximator that approximates a decision function (for example, a sigmoid function with decision threshold 0.5). The statistical inference aspect of DNN is implicit: for example, when sigmoid decision function is used and the network is trained with logistic risk, the network approximates a probability distribution. However, in the interpretation that a DNN implement an Umwelt, a DNN is not a function approximator but a statistical inference system by definition. Therefore, we give a stochastic definition of DNNs in this section, to summarize the characterization of the computation in DNNs developed so far. The definition defines a DNN as a multi-layer probabilistic graphical model that is a hybrid of Markov random field and Bayesian network.

To begin with, some clarifications are needed. We shall use MLP as an example to deliver the definition, and the definition can be generalized to other architectures straightforwardly. Also, we shall work with the widely used activation function ReLU, and similarly to the generalization to other architectures, the derivation in this paper can be generalized to activation functions like Swish [144], or variants of ReLU [12, 286]. However, to keep the narrative succinct, such generalizations are not discussed in this work. In doing so, we only claim that the theoretical results in this work hold for MLP with ReLU as its activation function; the applicability to the generalized cases is not discussed and considered future works.

We first give a stochastic, measure-theoretical definition of layer $l$ of a $L$-layer DNN to replace the functional definition of a layer in supp. B C 1 as follows.

**Definition 11** (Neural Layer)**.** *Let $X_{l-1}$ denote a random variable supported on a measurable space $\mathscr{M}_{l-1} := (\mathbb{R}^{n_{l-1}}, \mathscr{R}_{l-1}, \mu_{l-1})$, and $\boldsymbol{W}_l$ denote a random matrix supported on $\mathscr{W}_l := (\mathbb{R}^{n_{l-1}\times n_l}, \mathscr{R}_l^{\mathscr{W}}, \mu_l^{\mathscr{W}})$, where $\mathscr{R}_{l-1}, \mathscr{R}_l^{\mathscr{W}}$ are the $\sigma$-algebra on $\mathbb{R}^{n_{l-1}}, \mathbb{R}^{n_{l-1}\times n_l}$, respectively, and $\mu_{l-1}, \mu_l^{\mathscr{W}}$ are probability measure of $X_{l-1}$ and $\boldsymbol{W}_l$, respectively. A* **neural layer** *of a DNN is a multiplication of random elements given as*

$$X_l := dg(H_l)\boldsymbol{W}_l^T X_{l-1}, \tag{46}$$

*where $H_l$ is a random vector whose conditional probability measure (conditioning on $X_{l-1}$) is given by*

$$\mu_l(\boldsymbol{h}_l|\boldsymbol{W}_l, \boldsymbol{x}_{l-1}) = \frac{1}{Z} e^{\boldsymbol{x}_{l-1}^T \boldsymbol{W}_l dg(\boldsymbol{h}_l)}, \tag{47}$$

*where*

$$Z = \sum_{\boldsymbol{h}_l \in \mathbb{B}^{n_l}} e^{\boldsymbol{x}_{l-1}^T \boldsymbol{W}_l dg(\boldsymbol{h}_l)};$$

*and $dg(H)$ is the diagonal matrix whose diagonal is $H$. When there is no risk of confusions, we shall use $\mu$ to denote the measure of all random variables involved: for example, $\mu(X_l), \mu(X_{l-1})$ denote the probability measure of $X_l, X_{l-1}$, respectively.*

Compared with the conventional definition given in supp. B C 1, the above definition gives a stochastic DNN that is a hybrid of Bayesian network and Markov random field, as explained in the following. From supp. B B to this subsection, we have explained that, in the supervised learning setting, a DNN is a statistical inference system that learns a hypothesis that infers/predicts $X_l$ at the top layer. The hypothesis is parameterized by $\theta$, and by defining the weight matrices as random matrices, probabilities are assigned to hypotheses. In

[5] The lower bound maximization is also a well known property of the expectation-maximization algorithm, whose discussion could be found in Bishop [96, section 9.4]. We do not digress to elaborate the lower bound because we shall study the optimization behaviors of the algorithm in a way that is not related to the lower bound—that is, the global minima and the plasticity phase discussed in this work.

this sense, the definition is Bayesian. Meanwhile, it is also an untypical Bayesian definition, which we shall clarify after presenting the stochastic definition of DNNs. At the same time, the law of the neuronal gates is a higher-order Boltzmann machine—recall that $X_{l-1} := \prod_{i=1}^{l-1} \text{dg}H_i \boldsymbol{W}_i^T X$, and thus the energy $\boldsymbol{x}_{l-1}^T \boldsymbol{W}_l \text{dg}(\boldsymbol{h}_l)$ characterizes $l$-order statistical coupling among all random variables below (and including) layer $l$. A Boltzmann machine is an undirected graphical model that is more generally known Markov random fields. Therefore, the stochastic definition is a Bayesian Markov random field.

The stochastic definition induces another set of definitions as follows.

**Definition 12** (Neuron; Neuronal Gate; Neuron Activation)**.** *We name the random variables involved in a neural layer as follows.*

1. *We refer the a component of the random vector $X_l$, as a* **neuron***; the random vector $X_l$ as* **neurons at layer** $l$.
2. *We refer a component of the random vector $H$ as a* **neuronal gate***, and similarly $H_l$ as* **neuronal gates at layer** $l$.
3. *We refer a realization $\boldsymbol{x}_l$ of $X_l$ as* **neuron activation** *at layer $l$, and* **activation** *in short; if a realization of neuronal gate $H_i^l$ is non-zero, where $H_i^l$ here refers to the $i^{th}$ component of $H_l$ (and so similarly does $X_i^l$ next), we refer the neuron $X_i^l$ as* **activated***; similarly, we also refer the neuronal gate $H_i^l$ as activated.*

The stochastic definition of a neural layer induces a stochastic definition of a DNN as follows.

**Definition 13** (Multi-Layer Perceptron (MLP), macroscopic definition)**.** *A* **multi-layer perceptron** *$T$ is a tuple $T := (T, \theta, \mathcal{G})$, where $\theta := \{\boldsymbol{W}_i\}_{i\in[L]}$ is the set of weights and $\mathcal{G} := \{H_j\}_{j\in[L]}$ is the set of neuronal gates, and with an abuse of notation that shall not cause confusions, $T$ denotes both the MLP and the map $T$ defined as follows. $T$ is composed by $L$ recursively cascaded layers defined in definition 11; at layer $l$, its input neurons are the output neurons $X_{l-1}$ of layer $l-1$. And compactly, we write an MLP with a single output neuron as the following multiplication of random variables*

$$T(X;\theta) = X^T \overrightarrow{\Pi}_{i=1}^{L-1} \boldsymbol{W}_i dg(H_i)\boldsymbol{\alpha} \tag{48}$$

*where the weight matrix $\boldsymbol{W}_L$ of the last layer is written as a vector $\boldsymbol{\alpha}$ since we are to study the binary-classification problem; $i$ denotes the layer index; $\theta$ denotes the parameters of $T$ (i.e., $\{\boldsymbol{W}_i\}_{i=1,\ldots,L-1} \cup \{\boldsymbol{\alpha}\}$); $L$ is the layer number; $\overrightarrow{\Pi}_{i=1}^{L-1} \boldsymbol{W}_i dg(H_i)$ denotes $\boldsymbol{W}_1 dg(H_1) \ldots \boldsymbol{W}_n dg(H_n)$. We refer this definition as the* **macroscopic** *definition of MLP.*

**Remark 2** (Graph-theoretic aspects of DNNs)**.** *$(T, \theta, \mathcal{G})$ is also a multilayer network [287], which is a concept in network science studying complex networks: note that a network is a graph, and thus the weights in $\theta$ are edges that join nodes in $\mathcal{G}$ (i.e., neuronal gates) across layers, and the complex interaction among the nodes are specified as a map $T(X;\theta)$. Correspondingly, we also refer to weights as edges, and neuronal gates as nodes when the emphasis on the graph-theoretical aspect of the definition is needed. We remark this graph-theoretical aspect because it helps appreciate the definition of circuits in DNNs later in supp. B D 3. A graphical illustration of DNNs is given in fig. 2.*

**Remark 3.** *As the name suggests, in addition to the definition of MLP here, there would also be another microscopic definition of DNNs, which would be given at definition 20 in supp. B D 5. There, we shall explain the denotation of micro and macro.*

The stochastic definitions given in this subsection is untypical compared with the commonly used Bayesian models because it misses some commonly components that associated with Bayesian models. First, Bayesian inference typically associates with a parametric prior, such as Gaussian distributions, while we shall endow a functional constraint on the parametric distribution as the weight matrices—a prior on $\mu(\boldsymbol{W})$ referred as *weight symmetry* in supp. B E 2. Second, the definition is decoupled with Bayesian inference—as explained previously, it is the fact that the hypothesis space are endowed with a probability measure that makes the definition Bayesian. Unlike typical Bayesian models, which bind with Bayesian inference that maximizes the posterior probability (i.e., $\mu(\boldsymbol{W}_l|X_l) = \frac{\mu(X_l|\boldsymbol{W}_l)\mu(\boldsymbol{W}_l)}{\mu(X_l)}$ in this case), the learning of DNNs still maximize likelihood (cf. algorithm 2). But this is not say this is the best choice: we aim to characterize the current practice in this work instead of exploring the best practice.

Lastly, to clarify that a network in experiments is a realization of the MLP defined at definition 13, we define the realization of MLP as follows.

**Definition 14** (A realization of MLP)**.** *A realization of Multiple Layer Perceptron is a realization of the MLP defined at definition 13, where $\{\boldsymbol{W}_l\}_{l\in[L]}$ are not random matrices, but a sample of the random matrices. When there is no confusion, we would refer a realization of MLP as an MLP as well.*

To conclude, by reconceptualizing a DNN as a statistical inference system that implements a Umwelt defined in supp. B B, we have reached a stochastic definition of DNNs, and an expectation-maximization algorithm (or more accurately, an interpretation of forward and backward propagation of DNNs as an expectation-maximization algorithm) to learn DNNs. We have moved rather fast when reaching such a new conceptualization and left many issues not sufficiently discussed (e.g., the informational-geometrical problem mentioned in supp. B C 2). In doing so, we aim to investigate a fundamental problem of DNNs: that is, why risk minimization of DNNs always reaches almost zero risk? This is the problem we shall investigate in the rest of this paper.

### 7. *Loglikelihood and surrogate risks*

The derivation of DNNs from Umwelt relies on using the loglikelihood as the risk function, while DNNs could be optimized with various of risk functions instead of just the logistic risk that maximizes loglikelihood. In this subsection,

we explain the relationship between general risks and the loglikelihood: in short, both loglikelihood and surrogate risk are convex surrogates of the $0-1$ risk function, and thus the solutions reached by other risks are also qualitatively close to the solutions reached by loglikelihood.

To begin with, we present the formulation of risk minimization in statistical learning theory. For binary classification, the labels are given as integer $0,1$. However, it is intractable to directly optimize for a $0-1$ risk, given as

$$\mathbb{E}_{\mu(z)}[\mathbf{1}_{h_L \neq y}].$$

Therefore, convex loss functions that are surrogates to the $0-1$ risk is used instead. Given a loss function $\mathscr{L}$, the objective is to identify a function $T: \mathscr{X} \to \mathscr{Y}$ in a hypothesis space (a class $\mathscr{T}$ of functions) that minimizes the *expected risk*

$$R(\mathscr{L} \circ T) = \mathbb{E}_{Z\sim\mu}\left[\mathscr{L}(TX,Y)\right], \tag{49}$$

Because $\mu$ is unknown, the observable quantity serving as an approximation to the expected risk $R(T)$ is the *empirical risk*, given as

$$R_m(\mathscr{L} \circ T) = \frac{1}{m}\sum_{i=1}^{m} \mathscr{L}\left(T\boldsymbol{x}^{(i)}, y^{(i)}\right). \tag{50}$$

And in practice of DNN training, the empirical risk risk is minimized through batch/stochastic gradient descent that bootstraps batches from the whole dataset repeatedly—samples of a smaller size $b \in \mathbb{N}^+$ are repeatedly uniformly sampled from the training set—until the training convergence. Both bootstrap sample and the dataset are a sample of $Z$. And thus we shall use $b$ or $m$ depending on the context, and both of the average compute an empirical risk.

Both the loglikelihood and other risk function are metrics that measure the closeness between an inferred label of an instance and the ground-truth label, and different metrics have different properties. Nonetheless, for well designed loss functions, the end results of optimization with these measures are qualitatively similar (in a rather rough sense), though the quantification of similarity needs careful case-by-case study, for example, see Bartlett *et al.* [288]. And thus, DNNs optimized with other risk functions would also have a qualitatively similar level of loglikelihood, and generally could also be understood as solving surrogate problems of the hierarchical maximum entropy problem of Umwelt.

#### 8. *The restricted class of loss function analyzed in this work*

In this section, we shall study a class of loss functions that are relatively simple compared with the manifold of functions used in practice today. The class of functions is obtained as the first sub-problem of two interdependent sub-problems that composes the general problem. For interested readers, the problem decomposition is given in supp. G A, and furthermore, how the results in this work could potentially generalize to all kinds of loss functions is also given in supp. G A 2. We take the sub-problem as the first beachhead problem to study the general problem—this class of functions include practical loss functions, such as the hinge loss.

To begin with, we formally present the class of loss functions, denotes as $\mathscr{L}_0$.

**Definition 15** (Function class $\mathscr{L}_0$)**.** *We study the class $\mathscr{L}_0$ of loss functions, such that for $l \in \mathscr{L}_0$, when the label $y$ is considered as given, it satisfies:*

1. $l(x): \mathbb{R} \to \mathbb{R}^+$*;*
2. *$l$ is convex;*
3. *the second order (sub)derivatives $\frac{d^2}{dx^2} l$ is zero;*
4. $\min_x l(x,y) = 0$.

We explain why the class is defined as such. Generally, the Hessian of a DNN's risk is decomposed into two random matrices: a Wigner-type matrix and a Wishart-type matrix—details could be found in supp. G A 1. In the class of functions $\mathscr{L}_0$, as a restult of property 3, the Wishart-type matrix is a zero matrix, and thus only the Wigner-type matrix is left. The restriction simplifies the problem whereas still allows us to study the the optimization of supervised DNNs in real problems. The class of $\mathscr{L}_0$ includes important loss functions like the hinge loss $\max(0, 1-\hat{H}_L Y)$, and the absolute loss $|\hat{H}_L - Y|$, which were first studied in Choromanska *et al.* [146]. Correspondingly, we have to restrict DNNs to only have a single output neuron, which has reflected in the definition of DNNs presented at eq. (48). The other properties are typically properties of well designed loss functions. Property 1 and 2 are commonly used characterizations of loss functions in optimization. Property 4 characterizes that the loss function should assign a zero value for a correctly classified example.

### D. DNN self-organization through a feedback-control loop composed of coarse-grained variable and hierarchical circuits

In supp. B D 1, we characterize the risk minimization of DNNs as a variational free energy (or, more colloquially, uncertainty) minimization process where a DNN approximates the entropy of the environment/dataset (here entropy might better be understood as a measure of organization instead of disorder). In supp. B D 2, we characterize the predictions of a DNN as a coarse-grained random variable. In supp. B D 3, we develop a circuit formalism to characterize the hierarchical coupling among neurons in DNNs that computes the coarse-grained variable. The circuits are composed by neurons and the weights that connect neurons, where the input neurons at the bottom layer intake signals (datasets are digitalized signals), the hidden neurons in the intermediate layers perform computation, and the output neuron at the top layer effect action (e.g., pattern recognition). The circuit formalism reveals that the computation done in a DNN is simply the composition of **basis circuits** through addition and multiplication. And to compactly denote the computation done by a set of circuits, in supp. B D 4, we define a concept of **assemblies**, which formalizes the concept used by D. Hebb to denote functional units

of neurons in his *Organization of Behaviors* [289] that intakes input, computes, and emits outputs; that is, " an 'assembly' of association-area cells which can act briefly as a closed system after stimulation has ceased" [289, p. 60]. In supp. B D 5, with the circuit formalism, we characterize the self-organizing process as a dynamical process that executes a feedback-control loop composed by the circuits and the coarse-grained variable that the circuits compute: in each loop, the discrepancy between coarse-grained variable and feedback signals (labels) from the environment (dataset) is computed, propagated back to (self-)organize microscopic units (i.e., neurons) and induces system/macroscopic behavior change that minimizes the variational free energy.

### 1. *Variational free energy minimization in informational self-organization of DNNs*

In this section, we interpret the objective function of DNNs as a quantity known as *variational free energy*, such that the optimizing of DNNs could be interpreted as approximating the entropy/organization of the environment/dataset.

*a. Supervised DNNs maximize a Boltzmann distribution.* We begin with an example where a DNN does binary classification and minimizes the logistics risk. Supervised DNNs with logistics risk maximizes a Boltzmann probability distribution, as explained in the following. This is tautology given that we have shown that DNNs could be derived from maximum entropy estimation of probability distributions in supp. B C. We explicitly point out the connection here. In the risk function $R(\mathscr{L} \circ T)$ given at eq. (49), if we use the logistics loss function as the loss function $\mathscr{L}$, the risk function is instantiated to minimize (that is, maximize the negative of) the following risk

$$S_{\mu,\nu} := -\mathbb{E}_{(\boldsymbol{x},y)\sim\mu}\left[\log \nu(h_L, \boldsymbol{x})\right], \tag{51}$$

where

$$\nu(h_L, \boldsymbol{x}) := \frac{1}{Z} e^{-E(\boldsymbol{x}, h_L)} \mu(\boldsymbol{x}), \tag{52}$$

$$E(h_L, \boldsymbol{x}) := -\boldsymbol{x}^T \overrightarrow{\Pi}_{i=1}^{L-1} \boldsymbol{W}_i \mathrm{dg}(\boldsymbol{h}_i) \boldsymbol{\alpha}_L h_L \tag{53}$$

$$Z := \sum_{h_L \in \{0,1\}} e^{\boldsymbol{x}^T \overrightarrow{\Pi}_{i=1}^{L-1} \boldsymbol{W}_i \mathrm{dg}(\boldsymbol{h}_i) \boldsymbol{\alpha}_L h_L} \mu(\boldsymbol{x}), \tag{54}$$

$\mu(\boldsymbol{x})$ is the base measure on data $X$, and $Z$ is referred as the partition function. Note that eq. (52) is the law of the joint distribution of $H_L, X$. Further recall that in supp. B B 7, we have explained that $Y$ is the top layer neuronal gate (or, object random variable) $H_L$. Therefore, eq. (51) computes the loglikelihood of the estimated probability of the data $X, Y$. Thus, the risk of this DNN is a Boltzmann distribution with a complex *energy function*—energy function refers to $E(\boldsymbol{x}, y)$ in eq. (52), and in statistical physics it characterizes the energy of a state of the system. The minimization of the risk is the maximization of the Boltzmann probability distribution because of the minus sign. This family of models is also known as *energy DNN* models in the literature.

*b. Maximization of Boltzmann distribution as log-likelihood maximization of a Bayesian model.* The maximization of a Boltzmann distribution maximizes the log-likelihood part of a posterior probability, and thus we digress slightly to clarify the Bayes in the Bayesian definition given in definition 11. Suppose that we would like to maximize the posterior probability, we would have the risk given as

$$\begin{aligned} S_{\mu,\nu} &:= -\mathbb{E}_{(\boldsymbol{x},y)\sim\mu}\left[\log \nu(h_L, \boldsymbol{x})\nu(\theta)\right] \\ &:= -\mathbb{E}_{(\boldsymbol{x},y)\sim\mu}\left[\log \nu(h_L, \boldsymbol{x})\right] - \mathbb{E}_{(\boldsymbol{x},y)\sim\mu}\left[\log \nu(\theta)\right], \end{aligned}$$

where $\nu(\theta)$ denotes the prior distribution on weights. Therefore, despite being a Bayesian model, as defined in definition 11, the learning process does not maximize the posterior probability, but maximizes the log-likelihood. In this work, we shall not study the influence of such a design choice; we only aim to clarify the Bayes in the log-likelihood estimation.

*c. DNNs approximate the entropy of the environment.* The maximization of a Boltzmann distribution previously approximates the entropy of the environment (dataset), as explained in the following. As the notation suggests, that logistics risk is also the cross entropy between the true probability measure $\mu$ (cf. supp. B B 3) and the *variational* approximation $\nu$ (eq. (52)) of $\mu$ by a DNN. And cross entropy could be decomposed into the summation of the KL divergence $D_{\mathrm{KL}}(\mu||\nu)$ and entropy $S_\mu$ as

$$S_{\mu,\nu} = S_\mu + D_{\mathrm{KL}}(\mu||\nu).$$

It is known that $D_{\mathrm{KL}}$ is non-negative, and thus given a fixed $\mu$, the minima of $S_{\mu,\nu}$ is achieved when $\nu$ approximates $\mu$ exactly; in this case, the entropy of the DNN (i.e., $\nu$) is the same with the entropy of the environment—that is, the niche where the system embodies, or the dataset $S_m$ particularly in this work. Also, the entropy here might be better understood as a characterization of organization instead of disorder.

*d. DNNs minimize variational free energy.* To relate the entropy approximation to self-organization of physical systems, the previous entropy-approximating process has been referred as minimizing **variational free energy** [113–119]. Recall that for physical systems, without energy intake, any processes minimize free energy, and free energy could be decomposed into the summation of averaged energy and negative entropy as

$$F = \mathbb{E}_\mu[E(\boldsymbol{x})] - TS_\mu, \tag{55}$$

where with an abuse of notation, $T$ here denotes temperature instead of a DNN. And specifically for the self-organizing process of a physical system, the process dissipates energy and reduces entropy [120]. Thus, by minimizing the uncertainty in predicting the environment (dataset) (i.e., $S_{\mu,\nu}$), a DNN approximates $S_\mu$ in eq. (55), and thus could be understood as variationally approximating the free energy of the environment. Therefore, $S_{\mu,\nu}$ is also referred as *variational free energy*, and the self-organizing process is said to follow the *free energy principle* by Friston et al. [113–119].

Recall that a loss function in statistical learning [121] is a surrogate function that characterizes the discrepancy between the true measure ($\mu$ in eq. (51)) and the approximating measure

($\nu$ in eq. (51))—cf. supp. B C 7. A different loss function is only a different way to approximate the discrepancy. Therefore, regardless of the loss functions, a risk minimizes the variational free energy. Consequently, we could characterize the risk minimization of a DNN as an informational self-organizing process as follows.

*e. Informational self-organization of DNNs.* The risk minimization of a DNN is a self-organizing process where the system dissipates energy and approximate the entropy/order of the environment (i.e., the data-label mapping given in the dataset $S_m$) by minimizing the discrepancy between the predictions of the system and the feedback signals received from the environment.

The self-organizing process couples neurons hierarchically. Thus, we study the feedback-control loop between the coarse-grained random variables computed by the hierarchical coupling among neurons and the hierarchical coupling next.

### 2. *Coarse-grained variables computed by DNNs*

In this subection, we describe the coarse-grained random variable in DNNs. Actually, it has already been mentioned in supp. B D 1: the variable is simply the random variable

$$H_L,$$

and when a logistic risk is used, the law of $H_L$ is the Boltzmann distribution given at eq. (52). In supp. B D 1, we emphasize the connection between the risk minimization of DNNs and free energy minimization in physics; here, we explain the coarse-graining done by $H_L$, which has also been explained with a simple example in supp. B B 4.

The coarse-grained random variable $H_L$ represents whether a certain macroscopic pattern occurs in a signal $X$. As explained in supp. B B, coarse-graining in a Umwelt is to the construction of a random variable whose single state (i.e., $H_L = 1$) represents multiple states (e.g., multiple instances of $X$ are mapped to the same state $H_L = 1$) of random variables that are being coarse-grained, and formally, the probability measure of a state of $H_L$ is an integration of multiple states of $X$ as

$$\nu(H_L = 1) = \int_{\boldsymbol{x}\in\mathbb{R}^n} \frac{1}{Z} e^{\boldsymbol{x}^T \overrightarrow{\prod}_{i=1}^{L-1} \boldsymbol{W}_i \mathrm{dg}(\boldsymbol{h}_i)\boldsymbol{\alpha}_L} \mu(\boldsymbol{x}) d\boldsymbol{x}. \tag{56}$$

This is a designed feature of Umwelt. Thus, a macroscopic pattern is a pattern that integrates over many degrees of freedom that represent certain collective behaviors of the neurons; for example, the macroscopic pattern could be the existence of a cat in an image.

The coarse-grained random variable $H_L$ converts the complicated task of detecting macroscopic patterns into a computable problem. The probability the macroscopic pattern is considered existed in a signal is given as

$$\nu(H_L = h_L | X = \boldsymbol{x}) = \frac{\frac{1}{Z} e^{\boldsymbol{x}^T \overrightarrow{\prod}_{i=1}^{L-1} \boldsymbol{W}_i \mathrm{dg}(\boldsymbol{h}_i)\boldsymbol{\alpha}_L h_L} \mu(\boldsymbol{x})}{\frac{1}{Z} e^{\boldsymbol{x}^T \overrightarrow{\prod}_{i=1}^{L-1} \boldsymbol{W}_i \mathrm{dg}(\boldsymbol{h}_i)\boldsymbol{\alpha}_L \cdot 1} \mu(\boldsymbol{x}) + \frac{1}{Z} e^{\boldsymbol{x}^T \overrightarrow{\prod}_{i=1}^{L-1} \boldsymbol{W}_i \mathrm{dg}(\boldsymbol{h}_i)\boldsymbol{\alpha}_L \cdot 0} \mu(\boldsymbol{x})},$$

where $\nu(h_L = 1|\boldsymbol{x}) > 0.5$ when the exponent $\boldsymbol{x}^T \overrightarrow{\prod}_{i=1}^{L-1} \boldsymbol{W}_i \mathrm{dg}(\boldsymbol{h}_i)\boldsymbol{\alpha}_L \cdot 1$ (the case $h_L = 1$) is larger than 0 (the case $h_L = 0$, i.e., $\boldsymbol{x}^T \overrightarrow{\prod}_{i=1}^{L-1} \boldsymbol{W}_i \mathrm{dg}(\boldsymbol{h}_i)\boldsymbol{\alpha}_L \cdot 0$). Thus, if we take 0.5 as the decision threshold, the pattern recognition problem is converted to an arithmetical problem. The complexity exists in the energy function.

### 3. *Hierarchical circuits in DNNs*

To analyze the energy function, we develop a formalism of circuit in this subsection that characterizes the hierarchical coupling among neurons.

The stochastic definition of DNNs abstracts the complex coupling among neurons statistically into probability measures of random variables, and the abstraction enables us to decouple the complex activation patterns of DNNs into *basis circuits* that could be analyzed, as defined next.

**Definition 16** (Basis Circuit)**.** *Let $T = (T, \theta, \mathscr{G})$ be an MLP. Let $s, e \in \mathbb{L}, s < e$ and $i_l \in [n_l], s \le l \le e$. Let*

$$(W^s_{i_s i_{s+1}}, W^{s+1}_{i_{s+1} i_{s+2}} \ldots, W^{e-1}_{i_{e-2} i_{e-1}}, W^e_{i_{e-1} i_e}) \tag{57}$$

*be a sequence (i.e., an ordered set) of edges in $\theta$ that each is an entry of the weight matrix of a layer, sequentially from layer $s$ continuously to layer $e$. Meanwhile, each edge $W^l_{i_{l-1} i_l}$ in the sequence joins two nodes $H^{l-1}_{i_{l-1}}, H^l_{i_l}$ in a sequence of nodes*

$$(H^s_{i_s}, \ldots, H^e_{i_e}). \tag{58}$$

*The random variable induced by the sequential interlacing multiplication of edges and nodes is called a* **basis circuit***, defined as,*

$$\Psi^{s\ldots e}_{i_s \ldots i_e} := H^{s-1}_{i_{s-1}} \prod_{l=s}^{e} W^l_{i_{l-1} i_l} H^l_{i_l}. \tag{59}$$

*Optionally, a basis circuit could miss a node/neuron at the beginning or/and the end of the circuit, and is denoted as*

$$\Psi^{\wedge s\ldots e}_{i_s \ldots i_e} := \prod_{l=s}^{e} W^l_{i_{l-1} i_l} H^l_{i_l}, \tag{60}$$

*which misses the input neuron, or*

$$\Psi^{\wedge s\ldots e \wedge}_{i_s \ldots i_e} := H^{s-1}_{i_{s-1}} \left( \prod_{l=s}^{e-1} W^l_{i_{l-1} i_l} H^l_{i_l} \right) W^e_{i_{e-1} i_e}, \tag{61}$$

*which misses both the input neuron and output neuron. The vector consists of the sequences of weights in $\Psi^{\wedge s\ldots e \wedge}_{i_s \ldots i_e}$ is denoted as $\boldsymbol{w}^{s\ldots e}_{i_s \ldots i_e}$, and is referred as the* **circuit weights***. To emphasize the $s\ldots e$ is a continuous sequence, we write $s\ldots e$ as $s \sim e$. The sequence $(s, \ldots, e)$ is called the* **circuit layer index***, and the vector $(i_s, \ldots, i_e)$ is called the* **circuit weight index***. Let $\bar{l} := (s, \ldots, e), \boldsymbol{i} := (i_s, \ldots, i_e)$. The pair $(\bar{l}, \boldsymbol{i})$ is called the* **circuit index***. A basis circuit is compactly noted as*

$$\Psi^{\bar{l}}_{\boldsymbol{i}};$$

*and its weight as* $\boldsymbol{w}_{\boldsymbol{i}}^{\bar{l}}$. *Given a basis circuit, if all the neuronal gates are activated, the basis circuit is called* **activated.** *We also refer* $|\bar{l}| - 1 = e - s$ *as the* **length** *of the basis circuit, and* $\Psi_{i_{s'}\ldots i_{e'}}^{s'\ldots e'}$ *(where* $s' > s, e' < e$*) a* **subcircuit** *of* $\Psi_{i_s\ldots i_e}^{s\ldots e}$. *In addition, let* $I := \{\boldsymbol{i}\}$, *the notation is also used to denote a set of basis circuits: we denote the set of basis circuits* $\{\Psi_{\boldsymbol{i}}^{\bar{l}}\}_{\boldsymbol{i}\in I}$ *as*

$$\Psi_I^{\bar{l}}.$$

*The pair* $(\bar{l}, I)$ *is referred as* **circuit index set.**

A neuron circuit is recursively composed by basis circuits as follows.

**Definition 17** (Neuron Circuit)**.** *Let* $\bar{l}$ *be a sequence, and* $\bar{l} \subseteq \mathbb{L}$. *Let* $I$ *be a set whose elements* $\boldsymbol{i}$ *are vectors satisfy* $\boldsymbol{i} \in \overrightarrow{\bigotimes}_{l\in\bar{l}}[n_l]$, *where* $\otimes$ *denotes Cartesian product, and* $\overrightarrow{\bigotimes}$ *denotes the products are performed sequentially according to the order of* $\bar{l}$. *Then* $(\bar{l}, I)$ *is a circuit index set. A* **neuron circuit** $\Omega_I^{\bar{l}}$ *is a random variable recursively composed of circuits by the following two rules: Let* $(\bar{l}_1, I_1)$ *and* $(\bar{l}_1, I_2)$ *be two circuit index sets; assume two circuits* $\Omega_{I_1}^{\bar{l}_1}, \Omega_{I_2}^{\bar{l}_2}$,

1. *a new circuit could be formed by multiplication*

$$\Omega_{I_1\otimes I_2}^{\bar{l}_1\cup\bar{l}_2} = \Omega_{I_1}^{\bar{l}_1} \times \Omega_{I_2}^{\bar{l}_2},$$

*or compactly* $\Omega_{I_1}^{\bar{l}_1}\Omega_{I_2}^{\bar{l}_2}$, *where the circuit layer index needs to satisfy* $\bar{l}_1 < \bar{l}_2$ *or* $\bar{l}_1 > \bar{l}_2$ *(cf. the partial order in supp. B A);*

2. *or by addition*

$$\Omega_{I_1\cup I_2}^{\bar{l}_1} = \Omega_{I_1}^{\bar{l}_1} + \Omega_{I_2}^{\bar{l}_2},$$

*where the circuit layer index needs to satisfy* $\bar{l}_1 = \bar{l}_2$ *(i.e., elementwise equality).*

*A basis circuit is also a circuit. The set of all possible circuit* $\mathscr{C}$ *of* $T$ *is referred as the* **circuit space**, *and the* **dimension** *of the space is the number of the basis circuits of* $T$, *i.e.,* $\prod_{l=0}^{l} n_l$, *and is denoted* $|\mathscr{C}|$. *The realization of a circuit is call the* **output** *of the circuit.*

We illustrate the definition with a six-layer DNN as example. We expand the matrix form of the energy function in eq. (53), $\boldsymbol{x}^T\boldsymbol{W}_1\mathrm{dg}(\boldsymbol{h}_1)\boldsymbol{W}_2\mathrm{dg}(\boldsymbol{h}_2)\boldsymbol{W}_3\mathrm{dg}(\boldsymbol{h}_3)\boldsymbol{W}_4\mathrm{dg}(\boldsymbol{h}_4)\boldsymbol{\alpha}_5$, of the DNN into addition. The addition form is given as

$$\begin{aligned}&\boldsymbol{x}^T\boldsymbol{W}_1\mathrm{dg}(\boldsymbol{h}_1)\boldsymbol{W}_2\mathrm{dg}(\boldsymbol{h}_2)\boldsymbol{W}_3\mathrm{dg}(\boldsymbol{h}_3)\boldsymbol{W}_4\mathrm{dg}(\boldsymbol{h}_4)\boldsymbol{\alpha}_5 \\ =&\sum_r \alpha_r^5 H_q^4 \sum_{p,q} W_{pq}^4 H_p^3 \sum_{k,p} W_{kp}^3 H_k^2 \sum_{k,j} W_{jk}^2 H_j^1 \sum_{j,i} W_{ij}^1 X_i \\ =&\sum_{i,j,k,p,q,r} \alpha_r^5 H_q^4 W_{pq}^4 H_p^3 W_{kp}^3 H_k^2 W_{jk}^2 H_j^1 W_{ij}^1 X_i,\end{aligned} \tag{62}$$

Each term in the addition eq. (62) is a basis circuit, i.e., $X_i\Psi_{ijkpqr}^{\wedge 12345\wedge}$. The positiveness of the energy function is the addition of many basis circuits whose contributions are activated and deactivated by the neuronal gates $\{H_{i_l}^l\}_{l\in[6], i_l\in[n_l]}$.

Using the circuit formalism, eq. (62) could written compactly as

$$\Omega_I^{\wedge 12345\wedge} = \sum_{(i,j,k,p,q,r)\in I} X_i \Psi_{ijkpqr}^{\wedge 12345\wedge} = \sum_{\boldsymbol{i}\in I} \Psi_{\boldsymbol{i}}^{1\sim 5\wedge}, \tag{63}$$

where $I = \{\boldsymbol{i} | \boldsymbol{i} \in \prod_{l=0}^{5} \overrightarrow{\bigotimes}[n_l]\}$. Notice that $\{H_{i_l}^l\}_{l\in[6], i_l\in[n_l]}$ are binary random variables, i.e., valued in $\{0,1\}$, and they value 1 only if $\sum_{\boldsymbol{i}\in I_l} \Psi_{\boldsymbol{i}}^{1\sim 5\wedge}$, where $I_l = \prod_{l'=0}^{l} \overrightarrow{\bigotimes}[n_{l'}]$, are realized positive, respectively.

The basis circuit $\Psi_{\boldsymbol{i}}^{1\sim 5\wedge}$ is illustrated graphically in fig. 2. The sequence $(w_{i_s i_{s+1}}^s, \ldots, w_{i_{e-1} i_e}^e)$ in definition 16 is a *path* in graph theory [290, p. 162] whose vertices are the sequence $(H_{i_s}^s, \ldots, H_{i_e}^e)$ of neuronal gates, and is illustrated as the thick green path in fig. 2. A basis circuit $\Psi_{\boldsymbol{i}}^{1\sim 5\wedge}$ is a path that connects the input neurons on the left to the output neurons on the right (neurons that make decisions). When all the neuronal gates of a basis circuit are activated, the basis circuit is activated and contributes to the addition in $\Omega_I^{1\sim 5\wedge}$. Each activated basis circuit might be interpreted as a feature that contributes to the circuit $\Omega_I^{1\sim 5\wedge}$ that detects the class of macroscopic patterns represented by $H_L$.

The preceding example is the simplest case of circuit composition, where a circuit is composed by addition of basis circuits. Later in supp. B G 1, when we analyze the circuit in the Hessian of risk, we shall deal more complex composition where multiplication of circuits is involved. Generally, the multiplication rule is the reuse of sequential computation. The addition rule is the synthesis of parallel computation, where the outputs of different parallel circuits are added. The composition of circuits are recursive, in another word, hierarchical.

## 4. *Neuron assemblies, perturbations of basis circuits and derivatives of assemblies in DNNs*

The computation done in a DNN is simply the composition of basis circuits through addition and multiplication. And to compactly denote the computation done by a set of basis circuits, we refer it as an *assembly*, a concept used by D. Hebb to denote functional units of neurons in his *Organization of Behaviors* [289] that intakes input, computes, and emits outputs. We shall also show that derivatives of an assembly are still an assembly, which would reveal the order and phases of DNNs in supp. B F and supp. B G, respectively.

**Definition 18** (Neuron Assembly)**.** *An* **assembly** *of a basis circuits is a neuron circuit composed by the rules given in definition 17, formally given as,*

$$\sum_{\boldsymbol{i}\in I} \Omega_{\boldsymbol{i}}^{\bar{l}}, \tag{64}$$

*where* $\Omega_{\boldsymbol{i}}^{\bar{l}}$ *denotes a circuit composed by the multiplication of basis circuits, and* $I$ *is a set of circuit indices (defined in definition 16). We refer eq. (64) as a* **neuron assembly**, *or a* **circuit assembly**.

To give an example, the output of a DNN is a neuron assembly, given as follows.

$$\begin{aligned} T(X;\theta) &= X^T \overrightarrow{\Pi}_{i=1}^{L-1} \boldsymbol{W}_i \mathrm{dg}(H_i)\boldsymbol{\alpha} \\ &= \prod_{l=1}^{L} (\sum_{i_{l-1},i_l} H^{l-1}_{i_{l-1}} W^l_{i_{l-1}i_l}) \\ &= \sum_{i_0,\ldots,i_L} \prod_{l=1}^{L} H^{l-1}_{i_{l-1}} W^l_{i_{l-1}i_l} \\ &= \sum_{\boldsymbol{i}\in I} X_{i_0} \Psi_{\boldsymbol{i}}^{\wedge 1\sim L\wedge}, \end{aligned} \quad (65)$$

where $I = \overrightarrow{\otimes}_{l\in\mathbb{L}}[n_l]$, $H^0_{i_0} := X_{i_0}$, and the weight $\boldsymbol{\alpha}$ the last layer is written as a matrix for consistence. Recall that Hebb characterizes an assembly as " an 'assembly' of association-area cells which can act briefly as a closed system after stimulation has ceased" [289, p. 60], and further recall that each circuit is a random variable whose realizations are referred as activation of the circuit. Thus, an activation of eq. (64) formalizes the transience of Hebb's assembly. And the assembly given by eq. (65) detects a specific pattern—recall that in supp. B C 8 we restrict the DNNs studied to do binary classification—through activation of its basis circuits.

The circuit formalism reveals that the derivatives of circuits are still circuits, and the derivatives of assemblies are still assemblies. This observation shall later reveal the order and phases of DNNs in supp. B F and supp. B G, respectively. We present the results on the derivatives of circuits and assemblies in the following. The derivatives of circuits reduce to the addition and multiplication rules, as given in the following—the proofs are given in supp. E A.

**Lemma 2.** *Let $\Psi_{\boldsymbol{i}}^{s\sim e}$ be a basis circuit, then its partial derivative w.r.t. an edge/weight $w^l_{i_{l-1}i_l}$ in layer $l$, where $s \le l \le e$, is given as*

$$\frac{\partial \Psi_{\boldsymbol{i}}^{\wedge s\sim e\wedge}}{\partial w^l_{i_{l-1}i_l}} = \Psi_{\boldsymbol{i}_{:l}}^{\wedge s\sim l-1\wedge} H^{l-1}_{i_{l-1}} H^l_{i_l} \Psi_{\boldsymbol{i}_{l+1:}}^{\wedge l+1\sim e\wedge}. \quad (66)$$

**Remark 4.** *Note that although $\Psi_{\boldsymbol{i}}^{\wedge s\sim e\wedge}$ is the multiplication of random variables, here the derivatives are taken w.r.t. realizations of neuron weight variables. This is because the interested quantities are derivatives of realizations of MLP (cf. definition 14).*

The lemma implies the derivative of an assembly in turn is another assembly as follows.

**Corollary 1.** *Let $\Omega_I^{\wedge\bar{l}\wedge}$ denote the circuit given as*

$$\Omega_I^{\wedge\bar{l}\wedge} = \sum_{\boldsymbol{i}\in I} \Psi_{\boldsymbol{i}}^{\wedge s\sim e\wedge}$$

*where $\bar{l} := \{s,\ldots,e\} \subseteq \mathbb{L}$ is a sequence, and $I = \overrightarrow{\otimes}_{l\in\bar{l}}[n_l]$. Then, its partial derivative w.r.t. an edge/weight in layer $l$ is given as*

$$\frac{\partial \Omega_I^{\wedge\bar{l}\wedge}}{\partial w^l_{i_{l-1}i_l}} = \sum_{\boldsymbol{i}\in I^{\backslash\{l-1,l\}}_{i_{l-1}i_l}} \Psi_{\boldsymbol{i}_{:l}}^{\wedge s\sim l-1\wedge} H^{l-1}_{i_{l-1}} H^l_{i_l} \Psi_{\boldsymbol{i}_{l:}}^{\wedge l+1\sim e\wedge}. \quad (67)$$

*Compactly, it could be denoted as*

$$\Omega^{\wedge\bar{l}_{\backslash\{l\}}\wedge}_{I^{\backslash\{l-1,l\}}_{i_{l-1}i_l}},$$

*where $\bar{l}_{\backslash\{l\}}$ denotes*

$$\bar{l}_{\backslash\{l\}} := \{s,\ldots,l-1,l+1,\ldots,e\},$$

*and $I^{\backslash\{l-1,l\}}_{i_{l-1}i_l}$ denotes*

$$\overrightarrow{\otimes}_{\{p\in\bar{l}|p<l-1\}}[n_p] \otimes \{i_{l-1}\} \otimes \{i_l\} \overrightarrow{\otimes}_{\{q\in\bar{l}|q>l\}}[n_q];$$

*that is, $[n_{l-1}], [n_l]$ are substituted by single element sets $\{i_{l-1}\}, \{i_l\}$, respectively, in the consecutive Cartesian products that previously composes $I$.*

*Furthermore, we have*

$$\frac{\partial \mathscr{L}(T(X;\theta),Y)}{\partial w^l_{i_{l-1}i_l}} = \frac{\partial \mathscr{L}\left(\sum_{\boldsymbol{i}\in I} X_{i_0}\Psi_{\boldsymbol{i}}^{\wedge 1\sim L\wedge}, Y\right)}{\partial w^l_{i_{l-1}i_l}}$$

*is given as*

$$\begin{aligned} \Omega^{\bar{l}_{\backslash\{l\}}}_{I^{\backslash\{l-1,l\}}_{i_{l-1}i_l}} &= \sum_{\boldsymbol{i}\in I^{\backslash\{l-1,l\}}_{i_{l-1}i_l}} \Omega_{\boldsymbol{i}}^{\bar{l}_{\backslash\{l\}}} \\ &= \sum_{\boldsymbol{i}\in I^{\backslash\{l-1,l\}}_{i_{l-1}i_l}} \Psi_{\boldsymbol{i}_{:l}}^{\wedge s\sim l-1\wedge} H^{l-1}_{i_{l-1}} H^l_{i_l} \Psi_{\boldsymbol{i}_{l:}}^{\wedge l+1\sim e\wedge} \mathscr{L}'(\cdot), \end{aligned} \quad (68)$$

*where $\mathscr{L}'(\cdot)$ denotes the derivative of the loss function $\mathscr{L}$ w.r.t. the output of circuit $\Omega_I^{\bar{l}}$.*

The derivative could be performed recursively, and particularly, the second derivatives (i.e., Hessian entries) are given as

**Corollary 2.** *The second partial derivative of the circuit form eq. (65) of DNNs,*

$$\frac{\partial^2 \mathscr{L}(T(X;\theta),Y)}{\partial w^l_{i_{l-1}i_l} \partial w^{l'}_{i_{l'-1}i'_l}} = \frac{\partial^2 \mathscr{L}\left(\sum_{\boldsymbol{i}\in I} X_{i_0}\Psi_{\boldsymbol{i}}^{\wedge 1\sim L\wedge}, Y\right)}{\partial w^l_{i_{l-1}i_l} \partial w^{l'}_{i_{l'-1}i'_l}}$$

*is given as*

$$\sum_{\boldsymbol{i}\in I^{\backslash\{l-1,l,l'-1,l'\}}_{i_{l-1}i_l i_{l'-1}i_{l'}}} X_{i_0} \Psi_{\boldsymbol{i}_{:l}}^{\wedge 1\sim l-1\wedge} H^{l-1}_{i_{l-1}} H^l_{i_l} \Psi_{\boldsymbol{i}_{l:l'}}^{\wedge l+1\sim l'-1\wedge} H^{l'-1}_{i_{l'-1}} H^{l'}_{i'_l} \Psi_{\boldsymbol{i}_{l':}}^{\wedge l'+1\sim L\wedge} \mathscr{L}'(\cdot), \quad (69)$$

*where $l < l', l, l' \in [L]$—when $l = l'$, the derivatives are zero—and we have assumed that $\mathscr{L}''(\cdot)$ is zero because we study a class of loss functions whose second derivative is zero (this is formally given in supp. B C 8), e.g., hinge loss.*

*Or compactly, by absorbing the nodes and dropping wedge symbols, let*

$$\Omega_{\boldsymbol{i}}^{\bar{l}_{\backslash\{l,l'\}}} := \Psi_{\boldsymbol{i}_{:l}}^{1\sim l-1} \Psi_{\boldsymbol{i}_{l:l'}}^{l+1\sim l'-1} \Psi_{\boldsymbol{i}_{l':}}^{l'+1\sim L}, \quad (70)$$

*where* $\bar{l}_{\backslash\{l,l'\}} := \{1,\ldots,l-1,l+1,\ldots,l'-1,l'+1,\ldots,L\}$*; we have*

$$\frac{\partial^2 \mathscr{L}(T(X;\theta),Y)}{\partial w^{l}_{i_{l-1}i_l}\partial w^{l'}_{i_{l'-1}i'_l}} = \sum_{\boldsymbol{i}\in I^{\backslash\{l-1,l,l'-1,l'\}}_{i_{l-1}i_l i_{l'-1}i_{l'}}} \Omega_{\boldsymbol{i}}^{\bar{l}_{\backslash\{l,l'\}}}, \quad (71)$$

*where* $I^{\backslash\{l-1,l,l'-1,l'\}}_{i_{l-1}i_l i_{l'-1}i_{l'}}$ *denotes*

$$\overrightarrow{\otimes}_{\{p\in\bar{l}|p<l-1\}}[n_p]\otimes\{i_{l-1}\}\otimes\{i_l\}\overrightarrow{\otimes}_{\{p\in\bar{l}|l<p<l'-1\}}[n_p]$$
$$\otimes\{i_{l'-1}\}\otimes\{i_{l'}\}\overrightarrow{\otimes}_{\{p\in\bar{l}|p>l\}}[n_p].$$

The corollary shows that a Hessian entry is an addition of many circuits of the same type that is a multiplication of three basis circuits, which computes the second-order perturbations induced by $\partial w^{l}_{i_{l-1}i_l}$ and $\partial w^{l'}_{i_{l'-1}i'_l}$. We shall give an illustration of the perturbation of basis circuits of order two in supp. B G 1, where we discuss the circuits that compute Hessian in details.

The derivatives could be performed recursively up to $L$ times, and beyond $L$ times, the derivatives would be zero. To refer to the circuits that compute the perturbations of weights (against the risk), we refer them as the *perturbations of basis circuits*, and formally define them as follows.

**Definition 19** (Perturbations of basis circuits)**.** *Let*

$$\delta^k\Psi^{\bar{l}}_{\boldsymbol{i}} := \frac{\partial^k\Psi^{\bar{l}}_{\boldsymbol{i}}}{\prod_{w_j\in\boldsymbol{w}^{\bar{l}}_{\boldsymbol{i}},j\in[n]}\partial w_j}, \quad (72)$$

*where* $k\in\mathbb{N}$. $\delta^k\Psi^{\bar{l}}_{\boldsymbol{i}}$ *are referred as* **perturbations of basis circuits** *induced by weight perturbations of order k, or simply perturbations of basis circuits of order k.* $\delta^k\Psi^{\bar{l}}_{\boldsymbol{i}}, k=0,1,2$ *denote previous* $\Psi^{\bar{l}}_{\boldsymbol{i}}, \Omega_{\boldsymbol{i}}^{\bar{l}_{\backslash\{l\}}}$ *and* $\Omega_{\boldsymbol{i}}^{\bar{l}_{\backslash\{l,l'\}}}$ *in a unified way. Furthermore, for convenience, we let* $\mathscr{B}_k$ *denote the set consists of all the perturbations of basis circuits of order k (*$k\in\mathbb{N}$*), and* $I_k$ *denote the corresponding set of circuit weight indices:for example,*

1. $\mathscr{B}_0$ *denotes* $\{\delta\Psi^{\bar{l}}_{\boldsymbol{i}}\}_{\boldsymbol{i}\in I}$*, and* $I_0$ *refers to the I in eq.* (65)*;*
2. *similarly,* $\mathscr{B}^1_{i_{l-1}i_l}$ *denotes* $\{\delta^1\Psi^{\bar{l}}_{\boldsymbol{i}}\}_{\boldsymbol{i}\in I^{\backslash\{l-1,l\}}_{i_{l-1}i_l}}$*, and* $I^1_{i_{l-1}i_l}$ *denotes* $I^{\backslash\{l-1,l\}}_{i_{l-1}i_l}$ *in eq.* (67)*, or simply* $\mathscr{B}_1, I_1$*, respectively when the weight being differentiated is not important;*
3. *and* $\mathscr{B}^2_{i_{l-1}i_l i_{l'-1}i_{l'}}$ *denotes* $\{\delta^2\Psi^{\bar{l}}_{\boldsymbol{i}}\}_{\boldsymbol{i}\in I^{\backslash\{l-1,l,l'-1,l'\}}_{i_{l-1}i_l i_{l'-1}i_{l'}}}$*, and* $I^2_{i_{l-1}i_l i_{l'-1}i_{l'}}$ *denotes* $I^{\backslash\{l-1,l,l'-1,l'\}}_{i_{l-1}i_l i_{l'-1}i_{l'}}$ *in eq.* (71)*, or simply* $\mathscr{B}_2$*,* $I_2$*, respectively.*

To conclude with some clarifications, the definition is given just enough to present the results in this work, and many further aspects are not discussed: for example, the addition rule does not accommodate skip-layer edges as in ResNet [282]; and the characterization is set-theoretical algebraic operations yet the stochastic structure of circuits has not been characterized—the circuit space is an ambient space of certain manifold structure and the cumulants among assmeblies discussed later in supp. B G 7 are measures of "dissimilarity".

### *5. Adaptive feedback-control loop between coarse-grained variables and hierarchical circuits in DNNs*

The coarse-grained variable, neuron circuits and neuron assemblies constituent of formalism to characterize the self-organizing process of a DNN as a dynamical process that executes a feedback-control loop, as given in the following.

To begin with, we summarize the circuit definition of DNNs. Recall that we have given a definition of DNNs previously in definition 13, which we have referred as the macroscopic definition of DNNs. The definition in the matrix form is referred as the macroscopic definition because that form takes a system-wide view on the system, and is conducive to analyzing system-wide behavior. With the characterization of microscopic interaction among neurons as circuits, we also have given a definition of DNNs that based on the circuit formalism at eq. (65) in supp. B D 3, which characterizes the coarse-graining of computation of basis circuits. For clarity, we summarize it as the definition in the following.

**Definition 20** (Multiple layer perceptron, microscopic definition)**.** *A Multiple Layer Perceptron* $T(X,\theta)$ *is an assembly (defined at definition 18) composed by a set of basis circuits* $\{\Psi^{1\sim L\wedge}_{\boldsymbol{i}}\}_{\boldsymbol{i}\in I}$ *(defined at definition 16) as follows,*

$$T(X;\theta) = \sum_{\boldsymbol{i}\in I} X_{i_0}\Psi^{\wedge 1\sim L\wedge}_{\boldsymbol{i}}, \quad (73)$$

*where* $I = \overrightarrow{\otimes}_{l\in\mathbb{L}}[n_l]$*, and we have written the input neuron* $X_{i_0}$ *explicitly to emphasize that the circuit take inputs and compute. We refer this definition as the* **microscopic** *definition of MLP.*

The microscopic definition shall help us decompose the complex circuits in DNNs into simple basis circuits, and the behavior of the system could be analyzed by analyzing these basis circuits.

Formally, the self-organizing process of a DNN could be characterized as a differential equation, which is given as a definition for clarity as follows.

**Definition 21** (Feedback-control loop)**.** *Let* $R_m$ *denote the empirical risk defined in eq.* (50)*; for example, in the problem setting of this work, the empirical surrogate risk is given as*

$$R_m = \sum_{i=1}^{m}\max(0, 1-y^{(i)}T\boldsymbol{x}^i).$$

*Then, the dynamics of the self-organizing process of a DNN is a* **feedback-control loop** *given as the iterative process*

$$\frac{d\boldsymbol{\theta}}{dt} = -\eta\nabla_{\boldsymbol{\theta}}R_m, \quad (74)$$

*where* $\eta$ *is a scalars that scale the gradient* $\nabla_{\boldsymbol{\theta}}R_m$ *and is called as* **step size***, or* **learning rate** *in the literature.*

**Remark 5.** *Usually, this feedback-control loop would simply be referred as a feedback loop. And we append a "control" to the qualifier to indicate an action of the system upon receiving the feedback signals. This resembles the concept of sensorimotor loop [90] in embodied intelligence. However, the action*

*of a system does not necessarily involves a motor; in the case of DNNs, it is the modification of the neuronal weights, which is implemented as, for example, modification of memory registers, and could be understood as morphological computation. Therefore, we use a more general term of feedback-control loop.*

The definition characterizes a dynamical process that executes a loop described as follows: first, the circuit composed by neurons represents a hypothesis that computes a prediction of a coarse-grained random variable; second, a surrogate risk that measures the discrepancy between the prediction and the observed valued of the variable (feedback signals) from the environment/dataset; third, the circuit self-organizes according to gradient/feedback back-propagated from the feedback signals (the derivative of risk w.r.t. $T$) at the top-layer neuron; lastly, the process goes back to the first step. Note that currently, the goal is to define concepts formally, and thus we do not introduce complications by expanding the gradient into a neuron assembly; this would be done in supp. B F.

The differential equation is highly nonlinear, and unlikely accepts an analytic solution. To study the behavior of such an equation, we again look for ideas in theoretical biology. For a given evolving biotic system, it only has local information within spatial and temporal vicinity of its current state; and the system utilizes the local information to search for the local maxima on the fitness landscape that encode the hypotheses that are of high reproduction probability. Furthermore, in biotic systems, random fluctuations at the initial condition could result in critically different forms of organization of the system [45]—the phenomenon known as *chaos* in science. Such local exploitative behaviors of biotic systems are characterized as evolution by exploring *adjacent possible* states [7, p. 263] of the system by increasing *diversity* [137]. Therefore, to study the self-organizing process characterized by the equation, we do not aim to solve the equation, but to study the adjacent possible states of the system of sufficient diversity. In doing so, we identify a symmetry in DNNs, and study its effect on the adjacent possible states.

### E. Adaptive symmetries in the feedback-control loop

First, in supp. B E 1, We review the formalism of symmetry group in the self-organization of physical systems with the spin glass model as an example. In supp. B E 2, we define a stochastic adaptive symmetry of DNNs. Weight symmetries induce a *composite symmetry* that are the circuit symmetry mentioned previously and is defined and presented from supp. B E 3 to B E 4. This phenomenon is referred as *circuit symmetry* and is characterized as a theorem in supp. B E 5. In supp. B E 6, we motivate the hypothesis of such a coarse-grained adaptive symmetry. The hypothesis is later validated from supp. B F to B G through a high-dimensional probability bound obtained by analyzing the many-body statistical interaction among assemblies, and experiments.

#### 1. *Self-organization in physics: conservative symmetries and their breaking*

The self-organizing of a physical system is a process where the symmetries of energy—that is, symmetric states conserve the energy of the system—are broken, and the system transits to a state of a different level of energy. In this subsection, we review the formalism of symmetry group in the self-organization of physical systems with the spin glass model, in a rather simplistic way, as an example.

To begin with, we introduce some preliminaries.

1. First, we introduce the concept of symmetry groups. A *transformation group* of a set of objects is a group of transformation/map that applies on the objects. A transformation group $G$ is called a *symmetry group* when the transformation $g \in G$ leaves the object invariant by a certain criterion.

2. Second, we give the definitions of the groups that characterize the spins in a spin glass system in the following.

**Definition 22** (Translation group)**.** *Let $G_t$ be a group $\mathbb{Z}$ mod $n$, where $n \in \mathbb{N}$ and $\mathbb{Z}$ is the set of integers equipped the usual addition group action $+ : G_t \times G_t \to G_t$; that is, given a $x, y \in \mathbb{Z}$ mod $n, g_x \in G_t, g_y \in G_t$, we have*

$$g_x + g_y = g_{(x+y) \bmod n}.$$

*Then, the group $G_t$ is called a* **translation group**.

**Definition 23** (Rotation group)**.** *Let $G_r$ be a group $\{1, -1\}$ with the usual multiplication group action $\cdot : G_r \times G_r \to G_r$: that is, given a $x, y \in \{1, -1\}, g_x \in G_r, g_y \in G_r$, we have*

$$g_x \cdot g_y = g_{x \cdot y}.$$

*Then, the group $G_r$ is called a* **rotation group**.

At the beginning of the self-organizing process of a spin glass, the translation group and the rotation group are symmetry groups of free energy, and thus probability measure of the spins. More specifically, Let $\boldsymbol{\sigma}$ denotes the a random vector whose entries characterize the spins of a spin glass. The law of $\boldsymbol{\sigma}$ is a Boltzmann distribution $\rho$, whose exact form could be found at eq. (110) in supp. D C. The preceding symmetry could be formalized as follows.

1. First, the transformation group $G_t$ is a symmetry group on $\boldsymbol{\sigma}$ in the sense that, for example, the margin probability distribution $\rho(\sigma_i), \sigma_i \in \{\sigma_i\}_{i \in [n]}$ ($n$ is the number of spins) of each spin in the system is translational invariant: given a one-dimensional spin glass model where the spins are a function defined on a translational group (i.e., $\sigma_i : [n] \to \{1, -1\}$), we have

$$\forall g_x \in G_t, \rho(g_x.\sigma_i) = \rho(\sigma_{(i+x) \bmod n}) = \rho(\sigma_i). \tag{75}$$

This is the symmetry that makes reasonable the mean-field assumptions (cf. supp. D D) of the spin glass model.

2. Second, the system also satisfies rotational symmetry. Let $G_r$ be a rotational symmetry group, then we have

$$\forall g_x \in G_r, \rho(g_x.\sigma_i) = \rho(x \cdot \sigma_i) = \rho(\sigma_i). \tag{76}$$

*2. Weight symmetries: stochastic, heterogeneous symmetries in DNNs*

We characterize a symmetry of the probability measures in DNNs with the formalism of symmetry group, referred as *weight symmetry*, in the following.

Weight symmetry is defined as follows.

**Definition 24** (Weight symmetry)**.** *Given a MLP $T$, the weight matrix $\boldsymbol{W}_l$ at each layer $l$ is a sample of a random matrix whose law $\mu$ satisfies*

$$\forall i_l \in [n_l], i_{l-1} \in [n_{l-1}], \mu(w^l_{i_{l-1}i_l}) = \mu(-w^l_{i_{l-1}i_l}); \tag{77}$$

*that is, for any weights in layer $l$, it is realized from a random variable whose law is symmetrically distributed w.r.t. the y-axis.*

*Furthermore, for weights $w^l_{i_{l-1}i_l}, l \in [l], i_{l-1} \in [n_{l-1}], i_l \in [n_l]$ and $w^{l'}_{i_{l'-1}i_{l'}}, l' \in [l], i_{l'-1} \in [n_{l'-1}], i_{l'} \in [n_{l'}]$, they are realizations of random variables $W^l_{i_{l-1}i_l}, W^{l'}_{i'_{l'-1}i'_{l'}}$ that satisfy*

$$W^l_{i_{l-1}i_l} \perp W^{l'}_{i_{l'-1}i'_l}; \tag{78}$$

*that is, for each weight, it is independent with the rest of the weights. We refer the properties of weights given at eq. (77) and eq. (78) as* **weight symmetry***, and refer eq. (77) as the* **adaptive symmetry** *of weight symmetry, and eq. (78) as the* **diversity** *of the weight symmetry.*

Experimentally, we compute weights' distributions of neurons throughout training, and the results are shown in fig. 3a. As could be seen, at initialization, the weights' distributions at all layers are symmetric w.r.t. the $y$-axis at initialization. This results from the initialization scheme that initializes the weights with symmetric (normal) distributions. More importantly, although the symmetries break and distributions skew as training progresses, the symmetric shape of the distributions still stays in a non-trivial way.

The composition, or cooperation of the weight symmetries would induce a symmetry of basis circuits, which we turn to next.

*3. Symmetry and scale: stability of circuits*

The definition of weight symmetry given in supp. B E 2 is qualitative. Yet, we are studying a nonlinear system, which for this particular DNN system implies that the law of neuronal gates are of an exponential family, and is influenced by the scale, or magnitude of the neural weights and the neuron activation input (from the previous layer). Therefore, the outputs of circuits defined at definition 17 are influenced by the magnitude of the weights. To analyze the effect of weight symmetry on circuits, we characterize the magnitude of weights in this subsection.

Given the importance of the magnitude's influence on symmetry of circuits, we emphasize such magnitude as a definition as follows.

**Definition 25** (Circuit stability)**.** *Let $(T, \theta, \mathscr{G})$ be an MLP, where $\theta := \{\boldsymbol{W}_l\}_{l \in \mathbb{L}^+}$. We refer $T$ as an MLP that satisfies* **circuit stability** *when the following two conditions are satisfied: a $c \in \mathbb{R}$ exists, such that*

1. *$\forall l \in [L], i_l, i_{l-1} \in [n]$, $\mu(|w^l_{i_{l-1}i_l}| \geq c/\sqrt{n}) = 0$;*
2. *$\forall l \in [L]$, $\mu(|x^l_{i_l}| \geq c) = 0$,*

*where simplicity and clarity, we assume $\forall l \in \mathbb{L}, n_l = n \in \mathbb{N}^+$.*

The definition characterizes both the global and the local behaviors of DNNs, as explained in the following. Recall that

$$X^l_{i_l} = \sum_{i_{l-1}=1}^{n} W^l_{i_{l-1}i_l} X^{l-1}_{i_{l-1}} \tag{79}$$

$$= \sum_{\boldsymbol{i} \in \otimes^l [n]} \Psi^{1\sim l}_{\boldsymbol{i}}, \tag{80}$$

where the first is the recursive characterization of neurons from neurons the previous layer, and the second is the circuit characterization—$\otimes^l[n]$ denotes $l$ times Cartesian product of $[n]$. From eq. (79), we could see that the circuit is computed by the addition of $n$ terms $w^l_{i_{l-1}i_l} x^{l-1}_{i_{l-1}}$. The first condition of circuit stability characterizes that, for each the weights in the circuits, it makes a democratic contribution that does not overwhelm the rest of the neurons. Meanwhile, from eq. (80), we could see that the activation $x^l_{i_l}$ of a neuron is the coarse-grained effect of exponential number of circuits composed by weights and neuronal gates. The second condition of circuit stability characterizes that the magnitude of such coarse-graining maintains within a constant unrelated to the number of neurons; that is, no exponential amplification or attention in the process of coarse-graining. To acute readers, this looks related to criticality in physics: the phenomenon is referred as the *extended criticality* phenomenon, which we shall discuss further in supp. C B. The two conditions combined characterize the system behavior of DNNs, from which we shall analyze the computation of DNNs that solves non-trivial tasks, e.g., detection of macroscopic patterns, through collective computation of neurons.

In experiments, such stability is carefully maintained by initialization schemes, and normalization during training, and this practice is discussed further in supp. C B. Also, as a final clarification, in addition to the formal assumptions given at definition 25, in informally discussion, we shall assume $x^l_{i_l} = \Theta(1)$.

*4. Circuit symmetry: composite adaptive symmetry from weight symmetry*

Weight symmetry and circuit stability would induce a symmetry of circuits that we refer as *circuit symmetry*, and is the *microscopic* adaptive symmetry of DNNs. We present circuit symmetry in this section. As in supp. B E 1, we first define the mathematical groups, and then characterize the symmetries of basis circuits with such groups.

Two mathematical groups exist in DNNs at the circuit level. To characterize the symmetry, we first need to define a mathematical group referred as *circuit-translation group*.

**Definition 26** (Circuit-translation group)**.** *Let $G_l$ be a group $\mathbb{Z} \bmod n_l$, where $\mathbb{Z}$ is the set of integers equipped the usual addition group action. Let $G_t$ be the set that is composed by Cartesian product of groups $\overrightarrow{\otimes}_{l=0}^{L} G_l$, and is equipped with the group action $a : G_t \otimes G_t \to G_t$ defined as*

$$a\left((g_0,\ldots,g_L),(g'_0,\ldots,g'_L)\right) = \left((g_0+g'_0) \bmod n_0,\ldots,(g_L+g'_L) \bmod n_L\right),$$

*where $(g_0,\ldots,g_L),(g'_0,\ldots,g'_L) \in G_t$. Then $G_t$ is also a group whose action is a, which can be straightforwardly verified. The group $G_t$ gives a transformation group on the set of basic circuits $\{\Psi_{\boldsymbol{i}}^{1\sim L\wedge}\}_{\boldsymbol{i}\in I}$ as follows*

$$\forall g \in G_t, g.\Psi_{\boldsymbol{i}}^{1\sim L\wedge} = \Psi_{g.\boldsymbol{i}}^{1\sim L\wedge},$$

*where*

$$g.\boldsymbol{i} = a(g,\boldsymbol{i}).$$

Notice that we use the same symbol $a$ to denote the transformation that $g \in G_t$ applies on basis circuit $\Psi_{\boldsymbol{i}}^{1\sim L\wedge}$; this is because the action of the group $G_t$ is the same map with the transformation that $g$ applied on $\boldsymbol{i}$. A transformation $g$ in the group $G$ could be intuitively understood as the action that picks another basis circuit indexed by $g.\boldsymbol{i}$. Also note that, the index set $I := \overrightarrow{\otimes}_{l\in\mathbb{L}}[n_l]$ used in indexing circuits in supp. B D 3 is simply the circuit-translation group without the group action. Thus, from now on, we shall use $I$ and $G_t$ to denote the index set of basis circuits interchangeably.

The circuit-translation group and the rotation group defined at definition 26 are symmetry groups of basis circuits, as characterized in the following informal proposition.

**Informal Proposition 1** (Circuit symmetry)**.** *Let $T$ be a MLP, and $\Psi_{\boldsymbol{i}}^{s\sim e}$ be an basis circuits of $T$, where $\boldsymbol{i} \in \otimes_{l=s}^{e}[n_l]$, and the weights $w_{i_{l-1}i_l}^{l}$ satisfy weight symmetry defined at definition 24 and circuit stability defined at definition 25. Let $G_t$ be a circuit-translation group defined at definition 26, and $G_r$ a rotation group defined at definition 23. Then, we have*

$$\forall g_t \in G_t, g_r \in G_r, \mu(g_r.\psi_{g_t.\boldsymbol{i}}^{s\sim e\wedge}) \approx \mu(\psi_{g_t.\boldsymbol{i}}^{s\sim e\wedge}). \tag{81}$$

We shall give the formal characterization of the circuit symmetry where the approximate equality $\approx$ is characterized, after explaining the phenomenon characterized by the symmetry. The symmetry of $\mu(\Psi_{\boldsymbol{i}}^{s\sim e})$ implies that a basis circuit, statistically, would compute an output that is be of equal probability to be positive, or negative—that is, a symmetric output—in response to an observation $X_{i_0}$. In addition, the mean of $\Psi_{\boldsymbol{i}}^{1\sim L}$ is close to zero (characterized by lemma 3 later). Thus, each basis circuit statistically fluctuates around zero, and poses in a state to adapt and break the circuit symmetry in response to the feedback signals. The circuit symmetry is experimentally observed as well, as shown in fig. 3b.

In the following, we present the circuit symmetry formally. The proof is given in supp. E B 1.

**Proposition 1** (Circuit symmetry)**.** *Let $T$ be a MLP, and $\Psi_{\boldsymbol{i}}^{s\sim e}$ (also denoted as $\Psi_{\boldsymbol{i}}^{\bar{l}}$) be an basis circuits of $T$, where $\boldsymbol{i} \in \otimes_{l=s}^{e}[n_l]$, and the weights $w_{i_{l-1}i_l}^{l}$ satisfy weight symmetry defined at definition 24 and circuit stability defined at definition 25. Let $G_t$ be a circuit-translation group defined at definition 26, and $G_r$ a rotation group defined at definition 23. Let $m_k, k = 1\ldots+\infty$, be the moments of $\Psi_{\boldsymbol{i}}^{\bar{l}}$, where $m_k$ denotes the kth order moment. For each $\Psi_{\boldsymbol{i}}^{\bar{l}}$, let $\hat{\Psi}_{\boldsymbol{i}}^{\bar{l}}$ be a corresponding random variable whose characteristic function's Taylor series expansion is*

$$\sum_{k=0}^{+\infty} \frac{m_{2k}}{2k!}(it)^{2k};$$

*that is, $\hat{\Psi}_{\boldsymbol{i}}^{\bar{l}}$ is a random variable whose even-order moments are the same with $\Psi_{\boldsymbol{i}}^{\bar{l}}$, and whose odd-order moments are zero. Or, in other words,*

$$\forall g_r \in G_r, \mu(\hat{\psi}_{\boldsymbol{i}}^{\bar{l}}) = \mu(g_r.\hat{\psi}_{\boldsymbol{i}}^{\bar{l}}). \tag{82}$$

*Then, asymptotically, the circuit satisfies*

$$\forall g_t \in G_t, \left|\mathbb{E}\left[e^{i(\frac{\sqrt{n}}{c})^{e-s}\Psi_{g_t.\boldsymbol{i}}^{\bar{l}}t}\right] - \mathbb{E}\left[e^{i(\frac{\sqrt{n}}{c})^{e-s}\hat{\Psi}_{g_t.\boldsymbol{i}}^{\bar{l}}t}\right]\right| \leq \left|O\left((\frac{1}{2\sqrt{n}})^{e-s}\sin(t)\right)\right|, \tag{83}$$

*where we normalize $\Psi_{\boldsymbol{i}}^{\bar{l}}$ with $(\frac{\sqrt{n}}{c})^{e-s}$ to make $\Psi_{\boldsymbol{i}}^{\bar{l}}$ supported on $(-1,1)$.*

**Remark 6.** *We emphasize that the asymptotic notation $O$ is taken w.r.t. $n^{e-s}$ (i.e., $e-s$th power of the number of neurons at each layer). Thus, though the circuit length $e-s$ is also a variable, the inequality does not need the length to asymptotically goes to infinity. Instead, it should be understood as an exponentially compounding of $\sqrt{n}$ that creates very large number to measure up to the asymptotic bound.*

We explain the proposition by pointing out the connection to its informal version. It is well known that if the characteristic function of a probability measure $\mu$ is real, then the measure is symmetric w.r.t. the $y$-axis—the measure $\mu$ and $-\mu$ are of the same characteristic function. And as a random variable whose odd moments are zero, the characteristic function of $\hat{\Psi}_{\boldsymbol{i}}^{\bar{l}}$ is real and thus $\mu(\hat{\psi}_{\boldsymbol{i}}^{\bar{l}})$ is symmetric w.r.t. the $y$-axis, that is, satisfying eq. (82). Equation (83) characterizes that the closeness of the characteristic function of $\Psi_{\boldsymbol{i}}^{\bar{l}}$ and that of $\hat{\Psi}_{\boldsymbol{i}}^{\bar{l}}$: an decay factor $\left|O\left((\frac{1}{2\sqrt{n}})^{e-s}\sin(t)\right)\right|$ is induced by weight symmetry that makes the difference between $\Psi_{\boldsymbol{i}}^{\bar{l}}$ and $\hat{\Psi}_{\boldsymbol{i}}^{\bar{l}}$ (i.e., asymmetry of $\Psi_{\boldsymbol{i}}^{\bar{l}}$) decays exponentially w.r.t. the length $e-s$ of the circuit. Therefore, the longer the circuit (that is, the deeper the network), the more symmetry $\mu(\psi_{\boldsymbol{i}}^{\bar{l}})$ is.

Proposition 1 results from the exponential decay of odd moments of $\Psi_{\boldsymbol{i}}^{\bar{l}}$ against the length of the circuit. We present the lemma that characterizes such a decay in the following, which would later motivate the analysis the Hessian of DNNs.

**Lemma 3.** *Let $\{\Psi_{\boldsymbol{i}}^{\bar{l}}\}_{\boldsymbol{i}\in\underline{G}\subset G_t}$ be a set of basis circuits, where $\bar{l} := (s,\ldots,e)$, and $G_t$ is the circuit-translation group defined*

*at definition 26. Then, we have*

$$\left|\mathbb{E}\left[\prod_{\boldsymbol{i}\in\underline{G}\subset G_t}\Psi_{\boldsymbol{i}}^{\bar{l}}\right]\right| \leq O\left((\frac{c}{\sqrt{n}})^{|\underline{G}|(e-s)}(\frac{c}{2\sqrt{n}})^{\Sigma_{l=s}^{e}p_l}\right), \quad (84)$$

*where $p_l$ denotes the number of neuronal gates (of the set of circuits $\{\Psi_{\boldsymbol{i}}^{\bar{l}}\}_{\boldsymbol{i}\in\underline{G}\subset G_t}$) at each layer $l$ that satisfy the following condition: at least one of the corresponding circuit weights (i.e., $W_{i_{l-1}i_l}^{l}$) of the gate (i.e., $H_{i_l}^{l}$) is of odd power.*

The proof is given in supp. E B 1. We explain the phenomenon characterized by the lemma in the following by giving a proof sketch.

*Proof sketch of lemma 3.* In addition being a stochastic, heterogeneous symmetry, circuit symmetry is further a *composite symmetry* [125, Chp 7] that is composed from more elementary symmetries of weights. More concretely, each basis circuit is composed by weights, which each is realized from a random variable, and neuronal gates, which each depends on a great number of other neurons. More specifically, let $s = 1, e = L$, and recall that a basis circuit is of the form

$$\Psi_{i_1\dots i_L}^{1\sim L} = H_{i_L}^{L}W_{i_{L-1}i_L}^{L}H_{i_{L-1}}^{L-1}W_{i_{L-2}i_{L-1}}^{L-1}\dots W_{i_1i_2}^{2}H_{i_1}^{1}W_{i_0i_1}^{1}X_{i_0}. \quad (85)$$

Because $\{W_{i_{l-1}i_l}^{l}\}_{i_{l-1}\in[n_{l-1}]}, l \in [L], i_l \in [n_l]$ are of weight symmetry, each $W_{i_{l-1}i_l}^{l}$ is of equal probability to be positive and negative. Meanwhile, the activation of $H_{i_L}^{L}$ depends on a great number of neurons, and thus is only weakly correlated with the incoming weights (e.g., $W_{i_{L-1}i_L}^{L-1}$) when the number of weights involved in the calculation of higher moments are small. As a result, when calculating the odd moments of $H_{i_L}^{L}W_{i_{l-1}i_l}^{l}\Psi_{i_1\dots i_{L-1}}^{1\sim L-1}$, the integration against $W_{i_{l-1}i_l}^{L}$ over $[-\infty, 0]$ and $[0, +\infty]$ would almost cancel out, and only leaves a residual. To appreciate the cancellation, we might visit the odd moments of the product

$$\prod_{l=1}^{L}W_{i_{l-1}i_l}^{l}.$$

As a result of weight symmetry, the first order moment is given as

$$\mathbb{E}[\prod_{l=1}^{L}W_{i_{l-1}i_l}^{l}] = \prod_{l=1}^{L}\mathbb{E}[W_{i_{l-1}i_l}^{l}] = 0^L = 0.$$

Unlike the simple case here where weight symmetry induces exact zero, in the case of a basis circuit, weight symmetries induce an exponential decay because the switch of the sign of $W_{i_{l-1}i_l}^{l}$ does weakly influence the probability of $H_{i_l}^{l}$ being activated. The situation for higher order moments are similar. Note that the symmetry holds for each layer (i.e., self-similarity). Thus, the residual from layer $L$ would further be reduced by the weight symmetry in the lower layers. As a result, we obtain an exponential decay of moments characterized in the lemma. □

5. *Circuit-symmetry breaking in the feedback-control loop*

Recall that in supp. B D, we have characterized that the self-organizing process of a DNN where the system adapts to the environment (or, minimized uncertainty over a dataset) by back-propagating the discrepancy between a coarse-grained variable and the feedback signal (label) given from the environment (dataset). As a result, though at initialization, all basis circuits of a DNN satisfy the circuit symmetry, the self-organizing process breaks circuit symmetries. We characterize the broken circuit symmetries during training in this subsection.

More specifically, although each gradient update during the risk minimization might break the circuit symmetry of a subsets of basis circuits $I_b$, the symmetry might still hold in the circuits in the set $I \setminus I_b$—that is, the original set $I$ with basis circuits with $I_b$ removed. Thus, so long as a sufficient reservoir of basis circuits satisfy circuit symmetry, the system could keep adapting to the environment by breaking the circuit symmetry of circuits in the reservoir. As such, the system is in a state where broken symmetries and symmetries *stably coexist*: the broken symmetries encode information that processes past examples, whereas the symmetries maintains the ability to process novel examples. By maintaining such a coexistence, the system maintains stability to interact with the environment/datasets, and ability to adapt according to novel situations. In the following, we characterize the broken circuit symmetry where weight symmetries and broken weight symmetries coexist.

First, we present the theorem that characterizes the mixed of symmetries and broken symmetries in a circuit as follows.

**Theorem 1** (Broken circuit symmetry)**.** *Let $T$ be a MLP, and $\Psi_{\boldsymbol{i}}^{s\sim e}$ (also denoted as $\Psi_{\boldsymbol{i}}^{\bar{l}}$) be a basis circuits of $T$, where $\boldsymbol{i} \in \otimes_{l=s}^{e}[n_l]$, and the weights $w_{i_{l-1}i_l}^{l}$ satisfy circuit stability defined at definition 25. Furthermore, $e-s-b_{\boldsymbol{i}}$ number of circuit weights of $\Psi_{\boldsymbol{i}}^{\bar{l}}$ satisfy weight symmetry defined at definition 24—that is, $b_{\boldsymbol{i}}$ number of weights are of broken weight symmetry. Then, asymptotically, the circuit satisfies*

$$\forall g_t \in G_t, \left|\mathbb{E}\left[e^{i(\frac{\sqrt{n}}{c})^{e-s}\Psi_{g_t,\boldsymbol{i}}^{\bar{l}}t}\right] - \mathbb{E}\left[e^{i(\frac{\sqrt{n}}{c})^{e-s}\hat{\Psi}_{g_t,\boldsymbol{i}}^{\bar{l}}t}\right]\right| \quad (86)$$
$$\leq \left|O\left((\frac{1}{2\sqrt{n}})^{e-s-b_{\boldsymbol{i}}}\sin(t)\right)\right|,$$

*where the notations are same with proposition 1 .*

The theorem is a straightforward corollary of proposition 1 and corollary 4 (given shortly short), and the proof is given in supp. E B 2. The theorem characterizes a hierarchical "resilience" that the maintains the symmetry of $\mu(\psi_{\boldsymbol{i}}^{\bar{l}})$: as long as there is one circuit weight left that satisfies weight symmetry, a decay factor exists to make $\mu(\psi_{\boldsymbol{i}}^{\bar{l}})$ an approximately symmetric distribution—refer to supp. B E 4 for explanation why eq. (86) results in $\mu(\psi_{\boldsymbol{i}}^{\bar{l}})$ being a symmetric distribution. Consequently, to break the symmetry of the probability measure $\mu(\psi_{\boldsymbol{i}}^{\bar{l}})$, all the weight symmetries in the circuit need to be broken.

Furthermore, recall in supp. B D 4 we have shown that derivatives of basis circuits are also circuits, which we refer as perturbation of basis circuits. Such hierarchical decay also

exists in these circuits as well, which we characterize in the following corollary. The proof is given in supp. E B 2.

**Corollary 3.** *Let $T$ be a MLP trained with logistic loss function, and as in corollary 6, let $\delta^k \Psi_{\boldsymbol{i}}^{\bar{l}}, k = 1,2$ be a perturbation basis circuits (of order $k$) of $T$, where $\boldsymbol{i} \in \mathscr{B}_k$, and the weights $w_{i_{l-1}i_l}^{l}$ satisfy circuit stability defined at definition 25. Furthermore, and $L-k-b_{\boldsymbol{i}}$ number of circuit weights of $\Psi_{\boldsymbol{i}}^{\bar{l}}$ satisfy weight symmetry defined at definition 24—that is, $b_{\boldsymbol{i}}$ number of weights are of broken weight symmetry, and note $k$ layers that have been differentiated out. Then, asymptotically, the circuit satisfies*

$$\forall g_t \in G_t, \left| \mathbb{E}\left[ e^{i(\frac{\sqrt{n}}{c})^{L-k}\delta^k \Psi_{g_t.\boldsymbol{i}}^{\bar{l}} t} \right] - \mathbb{E}\left[ e^{i(\frac{\sqrt{n}}{c})^{L-k}\delta^k \hat{\Psi}_{g_t.\boldsymbol{i}}^{\bar{l}} t} \right] \right| \quad (87)$$
$$\leq \left| O\left( (\frac{1}{2\sqrt{n}})^{L-k-b_{\boldsymbol{i}}} \sin(t) \right) \right|,$$

*where the notations are same proposition 1 .*

**Remark 7.** *Unlike in the case of proposition 1, $\delta^k \Psi_{\boldsymbol{i}}^{\bar{l}}$ is normalized by $(\frac{\sqrt{n}}{c})^{L-k}$ to make the $\delta^k \Psi_{\boldsymbol{i}}^{\bar{l}}$ supported on $(-1,1)$ because the scale of perturbation of basis circuits differs from that of basis circuits in proposition 1: $k$ weights are differentiated out in the perturbation of basis circuits, and to normalize its support to $(-1,1)$, $k$ factors of $\frac{\sqrt{n}}{c}$ are removed.*

Compared with theorem 1 (let $s = 0, e = L$), we have an missed a decay factor $(c/2\sqrt{n})^k$ because the weights of layers that have be differentiated out (and thus it does not contribute the decay). Therefore, perturbation of basis circuits (of order one) also satisfy circuit symmetry.

As in the case of proposition that characterizes circuit symmetry, the broken symmetry theorem results from a similar moment decay phenomenon, which we characterize in the following corollaries, whose proofs are also given in supp. E B 2. These corollaries shall motivate the analysis of Hessian of DNNs as well.

**Corollary 4.** *Let $\{\Psi_{\boldsymbol{i}}^{\bar{l}}\}_{\boldsymbol{i} \in \underline{G} \subset G_t}$ be a set of basis circuits, where $\bar{l} := (s, \ldots, e)$, and $G_t$ is the circuit-translation group defined at definition 26. Then, we have*

$$\left| \mathbb{E}\left[ \prod_{\boldsymbol{i} \in \underline{G} \subset G_t} \Psi_{\boldsymbol{i}}^{\bar{l}} \right] \right| \leq O\left( (\frac{c}{\sqrt{n}})^{|\underline{G}|(e-s)} (\frac{c}{2\sqrt{n}})^{\Sigma_{l=s}^{e} p_l - b_l} \right), \quad (88)$$

*where $p_l$ denotes the number of neuronal gates (of the set of circuits $\{\Psi_{\boldsymbol{i}}^{\bar{l}}\}_{\boldsymbol{i} \in \underline{G} \subset G_t}$) at each layer $l$ that satisfy the following condition: at initialization, at least one of the corresponding circuit weights (i.e., $W_{i_{l-1}i_l}^{l}$) of the gate (i.e., $H_{i_l}^{l}$) is of odd power; and $b_l$ denotes the number of “broken” neuronal gates: for gates that at initialization have at least one weight of an odd power, and no long does so at the current state of training.*

**Corollary 5.** *Let $\{\delta^k \Psi_{\boldsymbol{i}}^{\bar{l}}\}_{\boldsymbol{i} \in \mathscr{B}_k}$ be a set of perturbation of basis circuits of order $k = 1,2$ (defined at definition 19), from a MLP trained with logistic loss function. Then, we have*

$$\left| \mathbb{E}\left[ \prod_{\boldsymbol{i} \in \underline{G} \subset \mathscr{B}_k} \delta^k \Psi_{\boldsymbol{i}}^{\bar{l}} \right] \right| \leq O\left( (\frac{c}{\sqrt{n}})^{|\underline{G}|(L-k)} (\frac{c}{2\sqrt{n}})^{\Sigma_{l=s}^{e} p_l - b_l} \right), \quad (89)$$

*where $p_l$ and $b_l$ have the same denotation with those in corollary 4.*

**Remark 8.** *Corollary 4 and corollary 5 actually could be written as one corollary by denote $\delta^0 \Psi_{\boldsymbol{i}}^{1\sim L}$ as $\Psi_{\boldsymbol{i}}^{1\sim L}$, however, corollary 4 also include subcircuit $\Psi_{\boldsymbol{i}}^{s\sim e}$ of basis circuits $\Psi_{\boldsymbol{i}}^{1\sim L}$, while corollary 5 requires $s = 1, e = L$. Therefore, we write them as two separate corollaries.*

### 6. Hypothesis: self-organizing of DNNs as an extended symmetry-breaking process with stable macroscopic adaptive symmetries

Recall at eq. (73), the output of a DNN is the addition of basis circuits over the circuit-translation group $I := \overrightarrow{\bigotimes}_{l \in \mathbb{L}} [n_l]$. The addition computes exactly the kind of coarse-graining variables in statistical physics: the addition of aligned spins in spin glasses over a translation group, calculated by techniques such as renormalization group, manifests as magnetic force—we refer to supp. D B for a review of coarse-graining variables in physics. As the coarse-graining effect of translation symmetry in a spin glass system might manifest as macroscopic magnetization, we hypothesize that the coarse-graining effect of circuit symmetry over $I$ might manifest as a certain macroscopic adaptive symmetry. More specifically, in this section, we motivate the hypothesis that the self-organizing process of a DNN is an extended symmetry-breaking process where intact and broken circuit symmetries coexist and manifests as an adaptive symmetry at the coarse-granularity of assemblies.

To begin with, we note that each neuron (i.e., $X_{i_l}^{l}$ defined at definition 12) is an assembly, more specifically,

$$X_{i_l}^{l} = \sum_{\boldsymbol{i} \in I_l} \Psi_{\boldsymbol{i}}^{1\sim l},$$

where $I_l := \otimes_{l'=0}^{l'-1} [n_{l'}] \otimes \{i_l\}$. With the access to easy visualization through Tensorboard [291], for any practitioner who has plotted the histograms of the pre-activation of DNNs at intermediate layers, the symmetry of histogram w.r.t. the $y$-axis would not be unfamiliar. Though not exactly the histograms of pre-activation, we would present experimental evidence of such symmetries later in supp. B F 2. Therefore, we proceed to study the self-similarity between adaptive symmetry of basis circuits and that of the assemblies; and more specifically, a self-similarity between the moments of basis circuits, and the moment of assemblies exists, as presented in the following.

First, we calculate the upper bound of the first and second moment of eq. (73), at initialization, according to corollary 4, which is given as the following lemma.

**Lemma 4.** *Let $\{\delta^k \Psi_{\boldsymbol{i}}^{1\sim L}\}_{\boldsymbol{i} \in \mathscr{B}_k}$ be perturbation of basis circuits defined at definition 19 of a MLP $T$. Then, at initialization, we have*

$$\mathbb{E}[\sum_{\boldsymbol{i} \in \mathscr{B}_k} \delta^k \Psi_{\boldsymbol{i}}^{1\sim L}] \leq O\left( (\frac{c^2}{2})^{L-k} \right), \quad (90)$$
$$\mathbb{E}[(\sum_{\boldsymbol{i} \in \mathscr{B}_k} \delta^k \Psi_{\boldsymbol{i}}^{1\sim L})^2] \leq O\left( c^{2(L-k)} + (\frac{c^2}{2})^{2(L-k)} \right).$$

**Remark 9.** *We note that the asymptotic notation is taken against* $1/\sqrt{n}^L$*, as in the case of lemma 3; no* $\sqrt{n}$ *appears in eq. (90) because a cancellation occurs, which would be clear in the proof we would shortly present.*

**Remark 10.** *Note that when* $k=0$*,* $\sum_{\mathbf{i}\in\mathscr{B}_k}\delta^k\Psi_{\mathbf{i}}^{1\sim L}$ *computes the output of the DNN; that is* $TX$*; when* $k=1$*, it computes an entry of the gradient (cf. corollary 1); when* $k=2$*, it computes an entry of the Hessian (cf. corollary 2).*

Recall that the symmetry of basis circuits results from the decay of odd moments relative to the even moments. From the lemma, we can see the decay of first moment relative to the second moment of the assemblies is self-similar to the decay of the basis circuits. More specifically, the ratio between $\mathbb{E}[\sum_{\mathbf{i}\in\mathscr{B}_k}\delta^k\Psi_{\mathbf{i}}^{1\sim L}]$ and $\mathbb{E}[(\sum_{\mathbf{i}\in\mathscr{B}_k}\delta^k\Psi_{\mathbf{i}}^{1\sim L})^2]$ is approximately self-similar to the ratio between $\mathbb{E}[\delta^k\Psi_{\mathbf{i}}^{\bar{l}}]$ and $\mathbb{E}[(\delta^k\Psi_{\mathbf{i}}^{\bar{l}})^2]$, of a given basis circuit—the $(\frac{c^2}{2})^{2L}$ term in the second moment is minor compared with the dominant term $c^{2L}$—by lemma 3, we have

$$\mathbb{E}\left[\Psi_{\mathbf{i}}^{\bar{l}}\right]\le O\left((\frac{1}{2})^L(\frac{c}{\sqrt{n}})^{2L}\right),\mathbb{E}\left[(\Psi_{\mathbf{i}}^{\bar{l}})^2\right]\le O\left((\frac{c}{\sqrt{n}})^{2L}\right).$$

Similar to the case of basis circuits, the depth has an exponential effect in reducing the first moment (i.e., the $1/2^L$ fractor), in comparison with the second moment.

Because the proof of lemma 4 is very simple, and informative, we give the proof in the following, where we could see that the coarse-graining effect of circuit symmetry concretely.

*Proof of lemma 4.* We first compute the moments of the addition of perturbation of basis circuits of order zero; that is, the set of basis circuits that compose the MLP circuit. At initialization, using lemma 3, we would have the first moment satisfies,

$$\mathbb{E}\left[\sum_{\mathbf{i}\in\mathscr{B}}\Psi_{\mathbf{i}}^{\bar{l}\wedge}\right]=\sum_{\mathbf{i}\in\mathscr{B}}\mathbb{E}\left[\Psi_{\mathbf{i}}^{\bar{l}\wedge}\right]\le n^L(\frac{c}{\sqrt{n}})^{L^2}\frac{1}{2^L}=(\frac{c^2}{2})^L.$$

Furthermore, the second moment is given as

$$\begin{aligned}\mathbb{E}[(TX)^2]=&\mathbb{E}\left[(\sum_{\mathbf{i}\in\mathscr{B}}\Psi_{\mathbf{i}}^{\bar{l}\wedge})^2\right]\\=&\sum_{\mathbf{i}\in\mathscr{B}}\mathbb{E}\left[\left(\Psi_{\mathbf{i}}^{\bar{l}}\right)^2\right]+\sum_{\mathbf{i}\in\mathscr{B},\mathbf{j}\in\mathscr{B},\mathbf{i}\neq\mathbf{j}}\mathbb{E}\left[\Psi_{\mathbf{i}}^{\bar{l}}\Psi_{\mathbf{j}}^{\bar{l}}\right]\\\le&n^L(\frac{c}{\sqrt{n}})^{2L}+(n(n-1))^L(\frac{c}{\sqrt{n}})^{4L}\frac{1}{2^{2L}}\\\le&c^{2L}+(\frac{c^2}{2})^{2L}.\end{aligned}$$

The proof of perturbation of basis circuit of order $k=1,2$ is almost the same: each differentiated weight would remove a decay factor $\frac{1}{2}(c/\sqrt{n})^2$, and meanwhile, it also removes $n$ number of weights in the addition because except the basis circuits that include the weight being differentiated, the rest of the basis circuits that do not have the weight would be differentiated to zero. And thus we would not repeat the calculation. □

Second, such decay of the moments of assemblies persists when circuit symmetries are only partially broken as a result of training/self-organization: that is, the coexistence of symmetries and broken symmetries characterized in supp. B E 5 manifests at the coarse-granularity of assemblies as decaying of odd moments of assemblies, when the a sufficient reservoir of weights of circuit symmetry exists. Formally, it is characterized as the following lemma.

**Lemma 5.** *Let* $\{\delta^k\Psi_{\mathbf{i}}^{1\sim L}\}_{\mathbf{i}\in\mathscr{B}_k}$ *be perturbation of basis circuits defined at definition 19 of a MLP* $T$*. Suppose that there exists* $\mu>0,\mu\in\mathbb{R}$*, such that* $\sqrt{n}^{1-\mu}$ *weights are of broken weight symmetry at each layer, then we have*

$$\begin{aligned}\mathbb{E}[\sum_{\mathbf{i}\in\mathscr{B}_k}\delta^k\Psi_{\mathbf{i}}^{1\sim L}]\le O\left((\frac{c^2}{2})^L+\frac{1}{\sqrt{n}^{L\mu}}c^L\right),\\\mathbb{E}[(\sum_{\mathbf{i}\in\mathscr{B}_k}\delta^k\Psi_{\mathbf{i}}^{1\sim L})^2]\le O\left(c^{2L}+(\frac{c^2}{2})^{2L}+\frac{1}{\sqrt{n}^{2L\mu}}c^{2L}\right).\end{aligned}\tag{91}$$

From the lemma we could see that until the number weights of broken symmetry at each layer exceed $\sqrt{n}$, the decay of the first moment compared with the second moment manifesting at initialization (i.e. the beginning of the self-organizing process) still persists. Furthermore, we note that we obtain here is an upper bound, and in experiments, the threshold is likely higher: this is because upper bound analyzes the worst case behaviors. We also observe such a phenomenon in experiments, which we shall discuss in supp. B G 6 later.

The proof of lemma 5 is also very simple, and informative, and thus we present it here.

*Proof of lemma 5.* Similar to in the proof of lemma 4, we first prove the upper bound for perturbation of basis circuit of order zero. By corollary 4, we have

$$\mathbb{E}\left[\sum_{\mathbf{i}\in\mathscr{B}}\Psi_{\mathbf{i}}^{\bar{l}\wedge}\right]=\sum_{\mathbf{i}\in\mathscr{B}}\mathbb{E}\left[\Psi_{\mathbf{i}}^{\bar{l}\wedge}\right]\le\sum_{\mathbf{i}\in\mathscr{B}}(\frac{c}{\sqrt{n}})^{L^2-b_i}\frac{1}{2^{L-b_i}},\tag{92}$$

where $b_i$ denotes the number of circuit weights of $\Psi_{\mathbf{i}}^{\bar{l}\wedge}$ are of broken weight symmetry. Then, the upper bound of the first moment is given as,

$$\begin{aligned}&\mathbb{E}\left[\sum_{\mathbf{i}\in\mathscr{B}}\Psi_{\mathbf{i}}^{\bar{l}\wedge}\right]\\\le&(n-\sqrt{n}^{1-\mu})^L(\frac{c}{\sqrt{n}})^{L^2}\frac{1}{2^L}+\sqrt{n}^{L(1-\mu)}(\frac{c}{\sqrt{n}})^L\\\le&(\frac{c^2}{2})^L+\frac{1}{\sqrt{n}^{L\mu}}c^L.\end{aligned}$$

And the upper bound of the second moment is given as

$$
\begin{aligned}
&\mathbb{E}\left[(\sum_{\boldsymbol{i}\in\mathscr{B}}\Psi_{\boldsymbol{i}}^{\bar{l}\wedge})^2\right]\\
=&\sum_{\boldsymbol{i}\in\mathscr{B}}\mathbb{E}\left[\left(\Psi_{\boldsymbol{i}}^{\bar{l}}\right)^2\right]+\sum_{\boldsymbol{i}\in\mathscr{B},\boldsymbol{j}\in\mathscr{B},\boldsymbol{i}\neq\boldsymbol{j}}\mathbb{E}\left[\Psi_{\boldsymbol{i}}^{\bar{l}}\Psi_{\boldsymbol{j}}^{\bar{l}}\right]\\
\leq& n^L(\frac{c}{\sqrt{n}})^{2L}+\left((n-\sqrt{n}^{1-\mu})((n-\sqrt{n}^{1-\mu})-1)\right)^L(\frac{c}{\sqrt{n}})^{4L}\frac{1}{2^{2L}}\\
&+\left(\sqrt{n}^{L(1-\mu)}(\sqrt{n}^{L(1-\mu)}-1)(\frac{c}{\sqrt{n}})^{2L}\right)\\
\leq& c^{2L}+(\frac{c^2}{2})^{2L}+\frac{1}{\sqrt{n}^{2L\mu}}c^{2L}.
\end{aligned}
$$

Similar to the generalization from order zero to order one and two in the proof of lemma 4, the differentiated weight simply removes a layer from the addition, and thus we would not repeat it. □

Therefore, unlike the symmetry breaking in physics, which is a power-law singularity where the symmetry of all units breaks simultaneously, the breaking of circuit symmetries might be an extended process where the broken and intact symmetries coexist, and when a sufficient intact symmetries exist, the coarse-grained effect of the symmetries at initialization persists during the self-organizing process even overall the symmetries are partially broken. This is also a qualitative difference between the symmetry breaking of physical systems and that biotic systems, which we refer to supp. D F for a review. If the self-similar decay of moments hold for moments of all order, then the assemblies would also be of a symmetric distribution, as that of the individual basis circuits. However, to study the adaptive symmetry of assemblies, we shall approach slightly differently, which is motivated next.

To begin with, we present the Taylor series expansion of the characteristic function of a DNN as follows,

$$
\mathbb{E}[e^{it\sum_{j=1}^{b}TX^{(j)}/b}]=\sum_{k=0}^{+\infty}\frac{1}{k!b^{k-1}}m_k(it)^k, \quad (93)
$$

where $b$ is the batch size used in practice during stochastic gradient descent, and $m_k$ denotes the $k$th moments of $TX$. From it, we could observe two types of possible decay:

- the first is the decay of odd moments, as discussed in this section previously;
- the second is the decay of the higher moments (i.e., the factor $1/b^{k-1}$) as a result of averaging over batches during training.

Although the analysis of the coarse-graining of the first and second moments suggests that the decay of the odd moments of assemblies is self-similar to the decay of the odd moments of the basis circuits, the calculation gets rather unwieldy for higher moments. Furthermore, we are manipulating upper bounds when calculating the moments of assemblies, and although the upper bound estimation characterizes the adaptive symmetry of individual basis circuits well enough, it likely overestimates the moments of coarse-grained circuits: we only make rather generic assumptions, i.e., circuit stability, and ignore the fact that the majority of the cross-moment of basis circuits could be simply very close zero, because when one circuit is activated, another one involved in the cross-moment might be not.

Therefore, in the rest of this work, we shall study the adaptive symmetries of assemblies by assuming on worst-case behaviors of the statistics of the assemblies that characterize these two type of decays. This approach might be appreciated by comparing it with the mean-field methods in statistical physics in its early days: in physics, the translation and rotation symmetry of spins presented earlier in supp. B E 1 has motivated the coarse-grained approximation of statistical behaviors of a collective of spins through its mean (i.e., the mean-field assumption) that, though with some discrepancy with the experimental results as a result of the approximation, qualitatively characterizes the behaviors of the physical systems (e.g., critical temperatures of phase transitions)—such epistemology of physics is reviewed in supp. D D. And we also note that rigorous characterization of such self-similarity in physics is very hard, and has not been reached even today [292].

To conclude, in the rest of this work, we shall study the adaptive symmetries of the assemblies, more specifically, the phase transitions of self-organizing process of DNNs, by analyzing the moment decay of the assemblies, which we next turn to.

### F. Order from fluctuations, or order from adaptive symmetry

In supp. B F 1, we present an *order parameter* of DNNs. In supp. B F 2, we experimentally study the coarse-grained effect of circuit symmetries on the order parameter.

#### 1. Order and plasticity order parameter of DNNs

In this subsection, we present an order parameter of DNNs by examining the elementary excitation of DNNs. Interestingly, the order parameter is symbolically equivalent (and only symbolically because the underlying mechanism are different) to the spin glass order parameter. We refer it as the *plasticity order parameter*.

To begin with, we briefly describe the elementary excitation in spin glasses. At equilibrium states, the spins in a spin glass satisfy certain symmetries that correspond to low energy (relatively to its neighboring states on the energy landscape). An *elementary excitation* of a system is the behaviors of the units of the system induced by perturbations: when the system dissipates energy as a result of the perturbations, the symmetries in the system are perturbed and the system is excited to a lower energy state and result in a coarse-grained/macroscopic behavior, or order of the system. For spin glasses at the ferromagnet phase, an approaching external magnetic field would excite it to repulse or attract the source of the magnetic field. The excitation is referred as the magnetization order parameter. Interested readers could find more background details in

supp. D C.

The self-organizing of DNNs could be conceptualized as the process where perturbations continually excite the system and break symmetries, characterized by a differential equation: in response to novel examples—in the sense that their errors measured by the surrogate risk are not zero—the system is continually being excited to decrease the risk by breaking circuit symmetries according to the feedback signals (gradients) from the risk. Each excitation/loop would modify the weights, and approximately reduce the risk (i.e., potential function) $R$ by

$$\eta \mathbb{E}_{Z\sim\mu}\left[||\nabla_\theta R||_2^2\right]. \tag{94}$$

Therefore, whether the variational free energy could be further decreased is characterized by the 2-norm of the first-order derivative of risk (variational free energy); that is, the first-order excitation induced by external perturbations. The circuit form of the excitation is given as follows. Taking the first-order derivative of the risk given at eq. (49) with the circuit form of DNN given at eq. (73), the circuit form of the eq. (94) is given by the following corollary—the proof is given in supp. E A.

**Corollary 6.** *Let $R_m$ be the empirical risk of a DNN $T(X;\theta)$. Then, the square of the 2-norm of the gradient is given as*

$$||\nabla_\theta R_m||_2^2 = \sum_{l=1}^{L} \sum_{i_{l-1}=1,i_l=1}^{n_{l-1},n_l} \sum_{\boldsymbol{i},\boldsymbol{i}'\in I_{i_{l-1}i_l}^{\backslash\{l-1,l\}}} \Omega_{\boldsymbol{i}}^{\bar{l}\backslash\{l\}} \Omega_{\boldsymbol{i}'}^{\bar{l}\backslash\{l\}}, \tag{95}$$

*where $\Omega_{\boldsymbol{i}}^{\bar{l}\backslash\{l\}}$ denotes*

$$X_{i_0}\Psi_{\boldsymbol{i}_{:l}}^{\wedge 1\sim l-1\wedge} H_{i_{l-1}}^{l-1} H_{i_l}^{l} \Psi_{\boldsymbol{i}_{l:}}^{\wedge l+1\sim L\wedge} \mathscr{L}'(\cdot), \tag{96}$$

*which is the first derivative of basis circuit $\Psi_{\boldsymbol{i}}^{\bar{l}}$ given at lemma 2 that intakes a datum $X_{i_0}$ at the bottom layer, and a derivative $\mathscr{L}(\cdot)$ at the top layer; and $I_{i_{l-1}i_l}^{\backslash\{l-1,l\}}$ is given in corollary 1.*

Despite the horrendous notation system, the expectation of the gradient norm symbolically resembles the spin glass order parameter. Recall that the spin order parameter of spin glasses is given as

$$\mathbb{E}_{\rho(\boldsymbol{\sigma})}[\sum_{ij} J_{ij}\sigma_i\sigma_j], \tag{97}$$

where $J_{ij}$ are constants, $\sigma_i, i\in[n]$ denotes spins, and $\rho$ denotes the law of the spins $\boldsymbol{\sigma}$—it could be derived by taking the first order derivative of free energy (i.e., the elementary excitation), and the derivation is given in supp. D C for interested readers. Equation (95) resembles symbolically to eq. (97) if we merge the three summation symbols into one big symbol. The symbolic resemblance results from the phenomena that the elementary excitation of both systems are the coarse-grained effects of the synchronized symmetries, and thus at the symbol level, they are equivalent: $\mathbb{E}_{Z\sim\mu}\left[||\nabla_\theta R||_2^2\right]$ coarse-grains (i.e., averages) the outputs of the circuits $\Omega_{\boldsymbol{i}}^{\bar{l}\backslash\{l\}}$, while $\mathbb{E}_{\rho(\boldsymbol{\sigma})}[\sum_{ij} J_{ij}\sigma_i\sigma_j]$ coarse-grains the spin direction of the spins.

Therefore, the expected squared gradient norm quantitatively characterizes the order of DNNs: whether the DNN system still possesses circuit symmetries to continually decrease risk in response to novel examples; in other words, whether the circuit symmetries have been completely broken. And we refer it as the *plasticity order parameter*. And we emphasize it as a definition in the following.

**Definition 27** (Plasticity order parameter)**.** *The order parameter of a DNN, which characterizes whether a DNN could still decrease uncertainty of specific novel examples processed by the DNN, is given as*

$$\mathbb{E}\left[||\nabla_\theta R_m||_2^2\right]. \tag{98}$$

We discuss the coarse-grain effect of circuit symmetry on the plasticity order parameter next.

### 2. *Experimental study on the order of DNNs: nonzero order parameter and symmetry of gradients*

Recall that by corollary 1, an entry of the gradient is an assembly of perturbation of basis circuits, and we have hypothesized in supp. B E 6 that assemblies of perturbation of basis circuits are self-similar to perturbations of basis circuits, in the sense of symmetry of law. Therefore, in this subsection, we perform an experimental study on the coarse-grained effect of the symmetry on the order of DNNs. The study shows throughout training of a DNN, the entries of the gradient are distributed symmetrically w.r.t. $y$-axis, the order parameter is nonzero, and both converge to zero when risk converges to zero.

To begin with, recall that by corollary 1, an entry of the gradient is the addition of perturbation of basis circuits, and for readers' convenience, we reproduce it as

$$\frac{\partial \mathscr{L}(T(X;\theta),Y)}{\partial w_{i_{l-1}i_l}^{l}} = \sum_{\boldsymbol{i}\in I_{i_{l-1}i_l}^{\backslash\{l-1,l\}}} \Omega_{\boldsymbol{i}}^{\bar{l}\backslash\{l\}}.$$

An illustration of perturbations of assembly of order one is given in fig. 2 as well. Corollary 1 characterizes the perturbation of the risk of order one induced the perturbation of a weight; it is simply the addition of $\Omega_{\boldsymbol{i}}^{\bar{l}\backslash\{l\}}$, the perturbation of basis circuits of order one induced by perturbation of weight. $\Omega_{\boldsymbol{i}}^{\bar{l}\backslash\{l\}}$ is illustrated as the think red line in fig. 2, where the weight perturbation is illustrated as a curvy line between two neuronal gates. Intuitively, when a basis circuit is activated, the first-order perturbation of a weight induced on risk is proportionally to the multiplication of the rest of the weights (i.e., the rest of the straight lines in the path). Therefore, the hypothesis given in supp. B E 6—that the at a coarse granularity, an adaptive symmetry, that is self-similar to the adaptive symmetry of basis circuits, holds as well—applies to the elements of gradient.

We validate the hypothesis experimentally: we compute and plot the (step-size normalized) order parameter and the distribution of gradients throughout training in fig. 4, which has been given earlier in section II E 2. In physics, the order parameters are more well known as a quantity that transits from

zero to nonzero (or, vice versa), than elementary excitation in response to external perturbations. From fig. 4a, we could see that the gradients have been distributed symmetrically w.r.t. $y$-axis until the last epochs during training where the gradients are close to zero. From fig. 4b, we could see that the order parameter starts from nonzero and gradually decreases to a value that is almost zero (the fluctuations are statistical fluctuations).

Therefore, a self-similar adaptive symmetry manifests at the coarse-granularity of gradients. More specifically, each entry of the gradient, or simply each gradient of a weight is a random variable. And thus, the histogram of all the gradients are a sample of $N$ random variables ($N$ is the number of parameters/weights of DNNs). By hypothesis, these random variables are of a symmetric law, and thus such a sample would be symmetrically distributed against $y$-axis, and the experiment validates that. Furthermore, the nonzero of order parameter is a simple consequence of such adaptive symmetry: note that gradient norm (i.e., order parameter) is the sum of the square of the gradients, and thus a symmetric and nonzero distribution of gradients imply nonzero of the order parameter.

Further recall that in supp. B F 1, the order parameter is proposed to characterize the phenomenon that whether a DNN could still decrease the uncertainty of novel examples; that is, examples with nonzero errors. The experiment results also corroborate the characterization: when there are still examples of nonzero errors, the order parameter is nonzero, and thus characterizes further reduction the uncertainty; the order parameter is only zero when all examples are of (almost) errors.

To conclude, this subsection experimentally shows that the coarse-grained of circuit symmetry manifests as an adaptive symmetry at the coarse-granularity of gradients, and thus results in nonzero of plasticity order parameter that quantifies the order of DNNs; that is, whether uncertainty/risk could be reduced in response to novel examples until zero risk is reached. However, there are many underlying issues that have not been discussed. Recall that in supp. B E 5 and B E 6, we have discussed that the self-organizing/training process of DNNs is a symmetry breaking-process where the intact and broken symmetries coexist, and a sufficient reservoir of circuit symmetries shall maintain the adaptive symmetry of circuits at a coarse-granularity. Therefore, As a symmetry breaking process, at least we have not studied the criticality in the process. Actually, because the qualitative difference between physical systems and biotic systems, there are much more unknown: for example, we have not studied the coexistence of intact and broken symmetries (how many symmetries have been broken), or the information encoded in the network as a result of such symmetry breaking. As the readers might be also aware the symmetry breaking of DNNs is a representative of a new class of systems that would take more efforts to understand, and could not be thoroughly investigated in a single work. Though to clarify the difference between the symmetry breaking process of DNNs and that in physics, we shall discuss the criticality during the self-organizing process in supp. C B, in this work, we mainly focus on understanding a phase of DNNs, which we turn to next.

### G. Plasticity phase and benign pathways on the risk landscape

We theoretically study the coarse-grained effect of partially broken circuit symmetries on the Hessian entries from supp. B G 1 to supp. B G 3. In supp. B G 1, we present the assemblies that compute the Hessian. In supp. B G 2 and B G 3, we characterize the coarse-grained effect of partially broken circuit symmetries in neuron assemblies hypothesized in supp. B E 6 as assumptions on Hessian entries (i.e., statistics of neuron assemblies), and quantities in the assumptions are interpreted as control parameters of DNNs. Under the assumptions, we present a theorem and a corollary from supp. B G 4 to B G 5 that characterizes the plasticity phase of DNNs. In supp. B G 4, the assumptions and the theorem are presented informally to prevent distractions from complicated technical details—their formal versions are given in supp. B H. The corollary are experimentally validated in supp. B G 5, where the phenomena characterized by the corollary are qualitatively observed throughout training. These assumptions are experimentally validated from supp. B G 6 to B G 7.

#### 1. *Perturbations of basis circuits of order two that compute Hessian*

Recall that in corollary 2, we have shown that an entry of Hessian is the addition of perturbation of basis circuits of second order. To begin with, in this subsection, we give a concrete example to help appreciate the process where a circuit computes a Hessian entry.

We give the Hessian entry of a six-layer DNN as an example, where $L = 5$ and $l = 2, l' = 4$, as follows

$$\begin{aligned}
&\frac{\partial^2 \mathscr{L}\left(\sum_{\boldsymbol{i}} X_{i_0} \Psi^{\wedge 12345\wedge}_{\boldsymbol{i}\in I}, Y\right)}{\partial w^2_{i_1 i_2} \partial w^4_{i_3 i_4}} \\
&= \sum_{i_0, i_5} X_{i_0} \Psi^{\wedge 1\sim 1}_{i_0, i_1} H^2_{i_2} \Psi^{\wedge 3\sim 3}_{i_3} H^4_{i_4} \Psi^{\wedge 5\sim 5\wedge}_{i_5} \mathscr{L}'(\cdot) \\
&= \sum_{i_0, i_5} X_{i_0} w^1_{i_0 i_1} H^1_{i_1} \times H^2_{i_2} w^3_{i_2 i_3} H^3_{i_3} \times H^4_{i_4} \alpha^5_{i_5} \mathscr{L}'(\cdot).
\end{aligned}$$

Similar to yet more complicated than the circuit that computes the output coarse-grained variable of a DNN given at eq. (63), the circuit that computes a Hessian entry is the addition of perturbation of basis circuits of order two (i.e., $\Omega^{\bar{l}\setminus\{l,l'\}}_{\boldsymbol{i}}$ in corollary 2), that each is a multiplication of three basis circuits $\Psi^{\wedge 1\sim 1}_{i_0,i_1}, \Psi^{\wedge 3\sim 3}_{i_3}, \Psi^{\wedge 5\sim 5\wedge}_{i_5}$. Also, note that the basis circuit $\Psi^{\wedge 5\sim 5\wedge}_{i_5}$ intakes the derivative of the loss $\mathscr{L}(\cdot)$ w.r.t. the output of the $\sum_{\boldsymbol{i}} X_{i_0} \Psi^{\wedge 12345\wedge}_{\boldsymbol{i}\in I}$, and computes the feedback (gradient back-propagated to layer 5 from $\mathscr{L}'(\cdot)$). Each basis circuit is a path in the network (cf. the graphic-theoretical interpretation of DNNs in B C 6), and if joined together, is a basis circuit defined at definition 16 with $w^l_{i_{l-1} i_l}, w^{l'}_{i_{l'-1} i'_l}$ differentiated out. $\Omega^{\bar{l}\setminus\{l,l'\}}_{\boldsymbol{i}}$ characterizes the infinitely small change of risk that would be induced by infinitely small change of the both edges $w^l_{i_{l-1} i_l}$ and $w^{l'}_{i_{l'-1} i'_l}$. $\Omega^{\bar{l}\setminus\{l,l'\}}_{\boldsymbol{i}}$ is illustrated in fig. 2 as the three

thick orange straight lines connected by two curvy lines (which represent the perturbed weights).

### 2. *Coarse-grained effect of circuit symmetry on Hessian entries*

Recall that earlier in supp. B E 6, we have explained that we shall analyzes the coarse-grained effect of the circuit symmetries on assemblies to study the adaptive symmetry of neuron assemblies. Therefore, in a way not unsimilar to the way that mean-field assumptions characterize translation symmetry in physics systems, we shall characterize the coarse-graining effect of partially broken circuit symmetries in DNNs as assumptions on statistics of assemblies in supp. B G 3. In this subsection, we motivate those assumptions.

To begin with, we recap the relationship between Hessian and the coarse-grained effect of perturbations of basis circuits of order two. Recall that in corollary 2, a Hessian entry (i.e., the perturbations of the risk $R_m$ induced by two weights) is the summation of perturbations of basis circuits of order two. And note that the second-order perturbation of risk $R_m$ induced by perturbations of all weights is given by $\delta\boldsymbol{\theta}^T\boldsymbol{H}\delta\boldsymbol{\theta}$, where $\delta\boldsymbol{\theta} \in \mathbb{R}^N$ are perturbations of weights and $\boldsymbol{H}$ denotes the Hessian. Therefore, the second-order perturbation of risk in the circuit form is given as

$$\delta\boldsymbol{\theta}^T\boldsymbol{H}\delta\boldsymbol{\theta} = \sum_{l=1}^{L}\sum_{l'=1}^{L}\sum_{i_{l-1}=1}^{n_{l-1}}\sum_{i_l=1}^{n_l}\sum_{i_{l'-1}=1}^{n_{l'-1}}\sum_{i_{l'}=1}^{n_{l'}} \sum_{\boldsymbol{i}\in\mathscr{B}^2_{i_l i_{l-1} i_{l'} i_{l'-1}}} \mathbb{E}[\Omega_{\boldsymbol{i}}^{\bar{l}\setminus\{l,l'\}}]\delta w^l_{i_{l-1}i_l}\delta w^{l'}_{i_{l'-1}i'_l}, \tag{99}$$

where $\Omega_{\boldsymbol{i}}^{\bar{l}\setminus\{l,l'\}}$ is defined in corollary 2 and is the perturbation of basic circuit $\Psi_{\boldsymbol{i}}^{\bar{l}}$ (of order two) induced by the perturbations of circuit weight $\boldsymbol{w}_{\boldsymbol{i}}^{\bar{l}}$ at layer $l, l'$, i.e., $\delta w^l_{i_{l-1}i_l}\delta w^{l'}_{i_{l'-1}i'_l}$—it is also explained with an illustration previously in supp. B G 1. That is, from eq. (99), $\delta\boldsymbol{\theta}^T\boldsymbol{H}\delta\boldsymbol{\theta}$ is the summation/coarse-graining of $(n^2L)^2n^{L-2}$ (assuming $\forall l \in [L], n_l = n$) perturbations of basis circuits.

In the following, we analyze the effect of circuit symmetry on such coarse-graining to motivate the assumptions next in supp. B G 3 that characterize the behaviors of neuron assemblies.

First, unlike the first order perturbation $\nabla_\theta R^T\delta\boldsymbol{\theta}$, where the perturbations induced by each weight are simply squared and summed together, the output of the circuits $\Omega_{\boldsymbol{i}}^{\bar{l}\setminus\{l,l'\}}, l, l' \in [L], \boldsymbol{i} \in \mathscr{B}^2_{i_l i_{l-1} i_{l'} i_{l'-1}}$ is structured as a matrix. Through matrix calculus, the Hessian matrix is given by the following lemma. The proof is given in supp. G B 1.

**Lemma 6.** *Let $\boldsymbol{H}$ denote the Hessian of the empirical risk eq. (50) w.r.t. weights of a DNN. Then, we have*

$$\boldsymbol{H} = \begin{bmatrix} \boldsymbol{0} & \boldsymbol{H}_{12}^T & \dots & \boldsymbol{H}_{1L}^T \\ \boldsymbol{H}_{12} & \boldsymbol{0} & \dots & \boldsymbol{H}_{2L}^T \\ \vdots & \ddots & \ddots & \vdots \\ \boldsymbol{H}_{1L} & \boldsymbol{H}_{2L} & \dots & \boldsymbol{0} \end{bmatrix}, \tag{100}$$

*where $\boldsymbol{H}_{pq}, p, q \in \mathbb{L}$ are the block matrices $\boldsymbol{H}_{pq} = \frac{\partial^2 R_m}{\partial \boldsymbol{W}_p \partial \boldsymbol{W}_q}$ and are given as,*

$$\begin{aligned}\boldsymbol{H}_{pq} = \frac{1}{b}\sum_{o=1}^{b}\Big[&\mathscr{L}'(T\boldsymbol{x}^{(o)}, y^{(o)})dg(\boldsymbol{h}^o_q)\overrightarrow{\Pi}_{k=q+1}^{L-1}(\boldsymbol{W}_k dg(\boldsymbol{h}^{(o)}_k))\boldsymbol{\alpha} \\ &\otimes \overleftarrow{\Pi}_{j=p+1}^{q-1}(dg(\boldsymbol{h}^o_j)\boldsymbol{W}^T_j)dg(\boldsymbol{h}^o_p) \\ &\otimes (\boldsymbol{x}^{(o)})^T\overrightarrow{\Pi}_{i=1}^{p-1}(\boldsymbol{W}_i dg(\boldsymbol{h}^o_i))\Big].\end{aligned} \tag{101}$$

*where $\otimes$ denotes Kronecker product and $\mathscr{L}'$ denotes the derivative of the loss function $\mathscr{L}$, and b denote the sample size—it is denoted by b to remark that empirical Hessian is computed batch-wise.*

That is, the object to study is the coarse-grained effects of the circuit symmetry on the the Hessian matrix $\boldsymbol{H}$.

Second, the coarse-grained effect of circuit symmetries hypothesized in supp. B E 6 suggests that the matrix $\boldsymbol{H}$ is a matrix with close to zero mean, and sparse correlation among its entries, as explained in the following. First, recall that in supp. B E 6, we have discussed that the first moments of assemblies of perturbation of basis circuits are orders of magnitude smaller than the second moments. Considering that the second moments are at the scale of $\Theta(1)$ (cf. supp. B E 3), the decay of the first moment implies that the first moment is close to zero. Further recall that by corollary 2, an entry of Hessian is an assembly of perturbation of basis circuit (of order two). And thus, the mean of $\boldsymbol{H}$ is close to zero. Second, observe that the cross-moments among Hessian entries are the cross-moments of assemblies of perturbation of basis circuits. For example, the second moment between two Hessian entries are given as

$$\begin{aligned}&\sum_{j=1}^{b}\mathbb{E}\left[\frac{1}{b^2}\sum_{\boldsymbol{i}\in\mathbb{B}^2_{i_l i_{l-1} i_{l'} i_{l'-1}}}\delta^2 X^{(j)}_{i_0}\Psi^{\wedge\bar{l}}_{\boldsymbol{i}}\sum_{\boldsymbol{j}\in\mathbb{B}^2_{j_l j_{l-1} j_{l'} j_{l'-1}}}\delta^2 X^{(j)}_{i_0}\Psi^{\wedge\bar{l}}_{\boldsymbol{j}}\right] \\ =&\frac{1}{b}\sum_{\boldsymbol{i}\in\mathbb{B}^2_{i_l i_{l-1} i_{l'} i_{l'-1}}}\sum_{\boldsymbol{j}\in\mathbb{B}^2_{j_l j_{l-1} j_{l'} j_{l'-1}}}\mathbb{E}\left[\delta^2\Psi^{\bar{l}}_{\boldsymbol{i}}\delta^2\Psi^{\bar{l}}_{\boldsymbol{j}}\right].\end{aligned}$$

And thus the decay of odd moments (as a result of weight symmetry), and higher moments (as a result of averaging over a batch) discussed in section II D 3 hold for cross-moments among Hessian entries as well. Therefore, the cross-moments among Hessian entries also have such decay. Because cross-moments are measures of correlation, we might hypothesize that the Hessian is a matrix with sparse correlation among its entries.

To conclude, for a hierarchically large DNN with sufficient reservoir of weights with circuit symmetries, a stable coexistence of intact and broken circuit symmetries might induce a Hessian that is a real symmetric matrix with zero-mean and sparse statistical dependence among its entries. This is formulated as assumptions next.

### 3. *Control parameters, and assembly assumptions of DNNs*

The phase space in physics is essentially a model that adequately characterizes a physical system in a way that explains

the system's behaviors (of interests). Therefore, the quantification of the coarse-grained variables (identified through symmetries) is essentially an approximation, and thus are usually referred as assumptions that are self-consistent with the phenomena being modeled. And the parameters of the coarse-grained variables (or as the coarse-grained variables themselves) that control the phase transitions are referred as *control parameters*. This epistemology of physics is reviewed in supp. D D. Therefore, to study the phases of DNNs, we identify assumptions and control parameters of DNNs that let the coarse-grained perturbation of basis circuit of order two (characterized by eq. (99)) manifest a stable adaptive symmetry. In this subsection, we present the assumptions and the control parameters [6], which have been motivated in supp. B G 2, and we shall also compare them with mean-field assumptions and control parameters of spin glasses.

To begin with, we introduce the *assembly-symmetry control parameter*, which comes from the following assumption.

**Assumption 1** (Assembly Symmetry). $\mathbb{E}[\boldsymbol{H}] = \boldsymbol{0}$.

The assumption characterizes the coarse-grained effect of circuit symmetries on the first moment of assemblies, as motivated in supp. B G 2. Intuitively, it characterizes the phenomenon that the second-order perturbations of assemblies fluctuate around zero and thus maintain an adaptive symmetry that can adapt to both positive and negative feedback signals to reduce the risk of a novel example. The zero–mean of the Hessian would ensure the eigenspectrum of Hessian to be symmetric w.r.t. the $y$-axis—this is discussed next in supp. B G 4—which provides an equal number of positive eigenvalues and negative eigenvalues to decrease the risk (more background discussion on the role of Hessian in optimization could be found in supp. D E). Thus, the mean of the Hessian is interpreted as the **assembly-symmetry control parameter**, or simply **symmetry control parameter**.

As discussed in supp. D D, control parameters characterize a system's behaviors that control phase transitions, and the behaviors could have multi-facet characterization: for a water-molecule system, both pressure and temperature are control parameters that control the phase transitions. In this case, in addition to the symmetry control parameter, we need another control parameter that characterizes the correlation among Hessian entries as follows.

To characterize the sparse dependence speculated in supp. B G 2, we formally define the coupling among Hessian entries as follows.

**Definition 28** (Coupling set). *Let $\boldsymbol{H} \in \mathbb{R}^{N\times N}$ be the Hessian of a DNN's risk. Given $\alpha := (i, j), \alpha \in \mathbb{I}$, where $\mathbb{I} := [N] \times [N]$, denote $h_\alpha$ the $i^{th}$ row, $j^{th}$ column of $\boldsymbol{H}$, and $\mathcal{N}(\alpha)$ the set consisting of entries (of $\boldsymbol{H}$) that $h_\alpha$ is statistically dependent with. We call $\mathcal{N}(\alpha)$ the* **coupling set** *of $h_\alpha$.*[7]

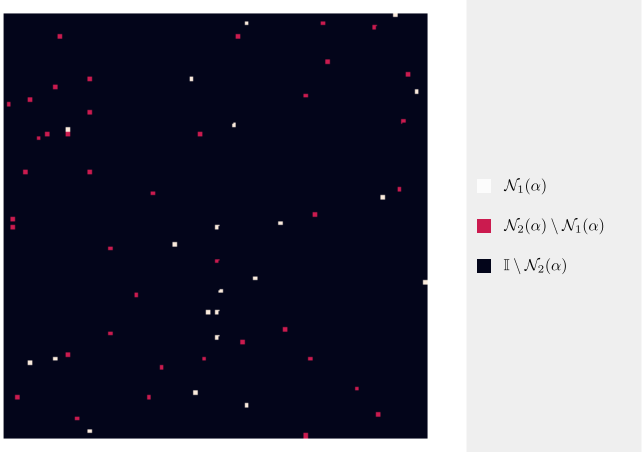


FIG. 9. The illustration of the size of the coupling set defined in simplified Assumption 2.B. The image represents the square matrix $\boldsymbol{U}$ defined in eq. (102), which is normalized Hessian matrix, with its index set $\mathbb{I}$ color coded. The assumption roughly states that for the two set $\mathcal{N}_1$ (color coded by white pixels) and $\mathbb{I} \setminus \mathcal{N}_2$ (color coded by black pixels) of entries of $\boldsymbol{U}$, the correlations between $\boldsymbol{U}_{\mathcal{N}_1}$ and $\boldsymbol{U}_{\mathbb{I}\setminus\mathcal{N}_2}$ varnish. Meanwhile, strong correlations are allowed in $\mathcal{N}_2$ (same as $\mathcal{N}$). Informally, each coupling set is a set of entries where the patterns encoded are correlated, e.g., legs, and arms of persons. Quantitatively, suppose that we have a 10-layer NN with 100 neurons in each layer, then the Hessian $\boldsymbol{H}$ would be of dimension $N = 10^5$, then $N^{1/2}$ is $10^{2.5}$. That is, the coupling set could have almost $10^{2.5}$ entries. That means for each entry, it could have almost $10^{2.5}$ number of correlated entries among only $10^3$ neurons.

The sizes of the coupling sets of all Hessian entries characterize the sparsity of the statistical dependency among Hessian entries, and are a characterization of the hierarchical coupling among neurons—or in other words, assembly diversity—in DNNs. And thus the *coupling set sizes* (i.e., $|\mathcal{N}(\alpha)|, \alpha \in \mathbb{I}$) are interpreted as the control parameters, and referred as **assembly-diversity control parameters**, or simply **diversity control parameter** in this work[8].

The diversity control parameter comes from the diversity assumption given in asm. 2 in supp. B H 2. We give simplified version here in the following.

**Simplified Assumption 2.A** (Assembly Diversity). *For each $\alpha \in \mathbb{I}$, the size of the coupling set satisfies $|\mathcal{N}(\alpha)| < \sqrt{N}$; that is, $h_\alpha$ is at most statistically dependent with $\sqrt{N}$ entries of $\boldsymbol{H}_{\mathbb{I}\setminus\{\alpha\}}$.*

**Remark 11.** *The assumption is formally given in asm. 2 as correlation (i.e., cumulant) decay between each Hessian entry $h_\alpha$ and the entries outside its coupling set $\mathcal{N}(\alpha)$. However,*

[6] We remark that control parameters given here may not be the only control parameters of DNNs. However, they are the control parameters relevant to the landscape analysis in this work.

[7] Technically, the statistical dependence is characterized through cumulant decay in asm. 2. The characterization is not given here because here we aim to give a simplified presentation to convey the ideas..

[8] It is not referred as the sparsity control parameter because the naming is misleading in the sense it gives the impression that the sparser the interaction, the better a DNN optimizes, and de-emphasizes the cooperation among neurons.

*considering the correlation decay formulation is more complicated, and the core idea is conveyed by the simpler statistical dependency here to help understanding.*

An illustration of the diversity assumption is given in fig. 9—this illustration is intended for the more complicated formal version of the diversity assumption given in supp. B H 2. As can be seen, under the assumption, the coupling among neurons is sparse: note that overall there are $N^2 - 1$ possible pairs between each $(i, j)$ and the rest of $\mathbb{I}$, and thus for an upper bound of $\sqrt{N}$ on the coupling set size, the statistically dependency among entries in $\boldsymbol{H}$ is considered sparse.

*a. Comparison between control parameters of DNNs and those of spin glasses.* To help appreciate the control parameters, we compare the control parameters here with the control parameters of spin glasses. First, both the control parameters of DNNs are characterized by coarse-grained observables, as are the temperature and average coupling constant $J_0$ of spin glasses. Though both being coarse-grained observables, as a result of the heterogeneity in DNNs, the control parameters of DNNs are not global scalars that characterize the average behavior of all units uniformly, as in spin glasses, but a matrix of control parameters that each characterizes the statistics of an assembly that computes the induced perturbation on the risk by the second order perturbations of two weights. Second, both the symmetry control parameter and $J_0$ characterize the average of two polarized behaviors of units: the increase and decrease of uncertainty of basis circuits, and the up and down directions of spins, respectively. Third, both the diversity control parameter and temperature characterize the coupling among units: the correlation among circuits (hierarchical coupling among neurons) and correlation among spins (at high temperature spins are of high kinetic energy and would correlate with other spins less), respectively.

When the preceding control parameters of a DNN satisfy the preceding assumptions, and furthermore, the regularity assumptions introduced later in supp. B H 3 are satisfied, the coarse-grained perturbation of basis circuits of order two given by eq. (99) would manifest an adaptive symmetry, which we turn to next.

#### 4. *Symmetry of Hessian eigenspectrum, or plasticity phase theorem of DNNs*

Under the assumptions given in supp. B G 3, which characterizes the coarse-grained effect of circuit symmetry on Hessian entries, we prove a theorem that characterizes the adaptive symmetry of eq. (99) in supp. B G 2—that is, the coarse-grained effect of circuit symmetry on the second order perturbation of risk induced by an arbitrary weight perturbation $\delta\boldsymbol{\theta}$. More specifically, the adaptive symmetry is the phenomenon that the eigenspectrum (i.e., probability density distribution of eigenvalues) of Hessian is distributed symmetrically against $y$-axis—that is, given any $\delta\boldsymbol{\theta} \in \mathbb{R}^N$, $\delta\boldsymbol{\theta}'$ exists such that $\delta\boldsymbol{\theta}'^T \boldsymbol{H} \delta\boldsymbol{\theta}' = -\delta\boldsymbol{\theta}^T \boldsymbol{H} \delta\boldsymbol{\theta}$. In this subsection, we present the theorem informally.

To begin with, we clarify the problem setting. Recall that in supp. B C 8, we have explained that this work studies a class of functions that is defined at definition 15, which could roughly be understood as the surrogate loss functions that are designed to work with binary classification, e.g., the hinge loss. The class does not include multi-class classification loss functions such as the cross entropy loss, or the quadratic loss for regression. The rationale behind such a restriction, and generality of the proof to any loss functions are discussed supp. G A, where we also discuss the speculation that the concept of circuit symmetry might suffice to prove similar results for all loss functions, and the hinge loss is the first part of two interdependent problems that consist of the general setting.

In addition to the diversity assumption, the proof of the theorem requires further regularity assumptions that assume finiteness in some quantities involved, a nondegenerate assumption that includes the case, for example, that requires the Hessian not to be a zero matrix. The regularity and nondegeneration assumptions are commonly used in high dimensional probabilistic analysis to rule out singularities, e.g., infinite moments. As discussed in section II D 3, the quantitative bounds are to qualitatively characterize DNNs, because the regularity assumptions are more technical—in the sense that they qualitatively correspond to the characterization that some quantities should be finite—instead of conceptual as the assumptions previously. Thus, we defer the description of these assumptions to supp. B H 3, and their implications to supp. B H 5.

The theorem that characterizes the local geometry of risk landscape of DNNs is informally given as follows; it is formally a probability upper bound, and is given later in supp. B H 5.

**Informal Theorem 1** (Plasticity Phase). *Let $R_m(T)$ be the empirical risk function (defined at eq. (50)) of a DNN $T$ with $n_L = 1$ (defined at definition 13) with a loss function $\mathscr{L}$ of class $\mathscr{L}_0$ (defined at definition 15). Let $\boldsymbol{H} \in \mathbb{R}^{N\times N}$ (c.f. eq. (100)) denotes the Hessian of $R_m(T)$, and $\mu_{\boldsymbol{H}}$ denotes the eigenspectrum (i.e., probability density distribution of eigenvalues) of $\boldsymbol{H}$. For a DNN that is hierarchically large, if $\boldsymbol{H}$ satisfies the assembly-diversity, assembly-symmetry and two further regularity assumptions, then with a high probability, $\mu_{\boldsymbol{H}}$ satisfies that,*

$$\forall \lambda \in \mathbb{R}, \mu_{\boldsymbol{H}}(\lambda) \approx \mu_{\boldsymbol{H}}(-\lambda).$$

Recall that an eigenvalue $\lambda$ is associated with a eigenvector, and thus for any eigenvector $\boldsymbol{\theta} \in \mathbb{R}^N$, $\boldsymbol{\theta}'$ could be found that satisfies $\boldsymbol{\theta}'^T \boldsymbol{H} \boldsymbol{\theta}' = -\boldsymbol{\theta}^T \boldsymbol{H} \boldsymbol{\theta}$; $\boldsymbol{\theta}$ can be infinitely small because the scale of an eigenvector does not change its eigenvalue. Therefore, the coarse-grained effect of circuit symmetry provides adequate negative eigenvalues such that the self-organizing of a DNN would not be trapped by local minima where no negative eigenvalues exist. This effect shall lead to benign pathways on the risk landscape that lead to zero risk, which we shall discuss next in supp. B G 5. Also, we shall explain why the theorem is referred as the plasticity phase theorem in supp. B G 8.

As an ending note, recall that in section II D 3, we explain that a DNN is studied via upper bounds that not exactly, but qualitatively characterize the behaviors of the DNN. In this particular theorem here, the theorem is intended to qualitatively characterizes the behaviors of DNNs in the sense that

zero mean of and sparse correlation among Hessian entries would induce symmetrically distributed eigenvalues; but not to exactly characterize the behaviors of DNNs in a quantitative sense. In supp. B G 5, B G 6 and supp. B G 7, we shall present the experimental results that qualitatively support the theorem.

### 5. *Benign pathways to zero-risk attractors on the risk landscape of DNNs*

The theorem implies that for a DNN with sufficient circuit symmetries, its risk could be continually decreased until the lower bound of the risk is reached. We investigate such an implication in this section, which is given as a corollary that characterizes a region of DNNs' state/weight space, or risk landscape (because risk is a function defined in the state space) where pathways to zero risk could be found by following gradients. The corollary is explained and supported by the experiments. We refer the pathways as the *benign pathways* on the risk landscape.

**Corollary 7.** *Given a DNN under the assumptions and setting of theorem 2, the states in the region of the DNN's risk landscape demarcated by the assumptions satisfies the following properties:*

*(a) all local minima are global minima with zero risk;*

*(b) half of the non-zero eigenvalues of any states in the region are negative;*

*(c) A constant* $\lambda_0 \in \mathbb{R}$ *exists, such that* $||\boldsymbol{H}||_2$ *is upper bounded by* $\mathbb{E}_m[\mathscr{L}'(T(X),Y)]\lambda_0$, *where* $\mathbb{E}_m[\mathscr{L}'(T(X),Y)]$ *is the empirical expectation of derivative* $\mathscr{L}'$ *of loss function* $\mathscr{L}$ *w.r.t.* $TX$. *This implies as the risk of states in the region decreases, the spectral norm* $||\boldsymbol{H}||_2$ *of Hessian* $\boldsymbol{H}$ *(of the states) is increasingly close to zero.*

The proof is given in supp. G B 3. We give a proof sketch in the following.

*Proof sketch of corollary 7.* We break down the analysis of Hessian $\boldsymbol{H}$ into two cases: (a) for all training examples, at least one example $(x,y)$ has non-zero loss value; (b) and all training examples are classified properly with zero loss. In case (a), by theorem 2, $\boldsymbol{H}$ is always indefinite, has half of its eigenvalues negative, and thus corresponds to a saddle point. In case (b), we are at global optima, where all losses are zero. Further recall that in eq. (101), the Hessian is scaled by $\mathscr{L}'$. Thus, the spectral norm is scaled by the $\mathscr{L}'$, which leads to part (c). □

We explain the corollary with the experiments that support it. The part (b) of the corollary states that half of the non-zero eigenvalues of the Hessian are negative. Such symmetry is found in experiments and shown in fig. 8a, which has been given earlier in section II F 5. It implies that throughout the risk minimization, every state with non-zero risk on the risk landscape could be decreased in the sense that if these states are saddle points, descending directions exist to move away from them. Yet, if each state has negative eigenvalues in its non-zero eigenvalues, how could minima be found? For a well-designed loss function, when the loss $\mathscr{L}(\boldsymbol{x},y)$ of an example is zero (property 4 of the loss function class $\mathscr{L}_0$), its derivative at $\boldsymbol{x}$ is zero, i.e., $\mathscr{L}'(\boldsymbol{x},y) = 0$. As more examples have been mapped to the zero loss (classified correctly in term of the surrogate loss), $\mathbb{E}_m[\mathscr{L}'(T(X),Y)]\lambda_0$ is increasingly close to zero. Because $||\boldsymbol{H}||_2$ is upper bounded by $\mathbb{E}_m[\mathscr{L}'(T(X),Y)]\lambda_0$, eigenspectrum of $\boldsymbol{H}$ is increasingly concentrated around zero. Therefore, the part (c) of the theorem states that as the risk decreases, and the Hessian eigenspectrum would increasingly concentrate towards zero, as supported by experimental evidence presented in fig. 8a. The minima are reached when all example $\boldsymbol{x}$ are classified correctly—that is, the risk is zero; in this case, the Hessian becomes a zero matrix, and all eigenvalues are zero—though we note that in the experiments the zero is only approximately reached because stochasticity in the stochastic gradient descent, which introduces statistical fluctuations. As a result, we have the part (a) of the theorem that states all local minima are global minima with zero risk[9]. Therefore, in the state space demarcated by assumptions of theorem 2, benign pathways could be found by following gradients of risk. The training loss and accuracy curves of the training are shown in fig. 8b.

To conclude, the corollary and the experiments characterize the local geometry of a region of DNNs' risk landscape where benign pathways could be found by following gradients and lead to zero risk. Such local geometry results from the assumptions given in supp. B G 3 that are motivated from circuit symmetries. Next, we experimentally validate the assumptions.

### 6. *Experimental validation of the assembly-symmetry assumption, and symmetric distributions of Hessian entries*

In this subsection, we present experiment support for the assembly-symmetry assumption given in supp. B G 3. More specifically, the experiments show that during the training, the Hessian entries' means concentrate on zero, and furthermore, the distributions of Hessian entries are also self-similar to the those of perturbation of basis circuits, in the sense that the distributions of the Hessian entries are approximately symmetric, as in the case of gradient entries.

To begin with, we recall the intention of the experiments presented in supp. B G 6 and also supp. B G 7. As explained previously in section II D 3, the assumptions are part of an upper bound that are intended to qualitatively characterize the coarse-grained effect of circuit symmetries, and not to give exact quantitative characterization. Therefore, the experiment

[9] We note that some subtlety exists because of the stochastic gradient descent. During training, each batch is a bootstrap sample of the dataset, and thus the Hessian is also the average of Hessian of examples in this sample. The plasticity phase implies all loss of these bootstrap samples could be decreased to zero. And because the samples are bootstrap samples—that is they are repeatedly randomly sampled from the dataset—at the end of the training, empirical risk would reach zero as well.

results here also do not aim to exactly, but to qualitatively validate the assumptions.

*a. Zero mean of the Hessian entries.* First, we plot the probability density distribution of means of Hessian entries normalized by standard deviations in fig. 7. We also plot the fraction of normalized means that are less than 0.15 in fig. 7b. Figure 7 shows that throughout the training, the means concentrate on zero in the sense that most of the means do not fluctuate further than 0.15 standard deviation from zero, which is clearly a concentration of measure on zero, as explained in the following. Suppose that the standard deviation is $\sigma$ for a Hessian entry. Then, the deviation averaged over the dataset is $\sigma/\sqrt{\lceil m/b \rceil}$, where $m$ is the size of the dataset, and $b$ is the batch size. First, from fig. 7b we can see that throughout training, the fraction of the means that are less than 0.15 is at least 95%, and as the training progresses, the percentage gradually increases up to around 98%. To help appreciate the zero-mean characterized by the assumption, we might compare it with the concentration of measure on zero phenomenon induced by a normal distribution with zero mean. In the practice of statistics, to estimate the mean of random variable of a normal distribution, a sample would be sampled, and empirical mean of the sample computed. For empirical mean computed from a sample of size $s$, the standard deviation of the sample is $\sigma/\sqrt{s}$, where $\sigma$ is the standard deviation of the variable: that is, the larger the sample size, the closer the samples are to the mean. And for an empirical mean computed from the sample, it has approximately 95% probability to be within the interval $(-2\sigma/\sqrt{s}, 2\sigma/\sqrt{s})$. Thus, for a sample of size $\lceil m/b \rceil = \lceil 10000/64 \rceil = 157$, for a probability of 95%, the empirical mean of a sample from a zero-mean normal distribution would be in the interval of $0.16\sigma$. Therefore, the experiment validates the assumption that the means of Hessian entries are almost zero.

Nevertheless, despite the closeness to zero, we also observe a phenomenon that probably results from the coarse-grained effect of broken circuit symmetries. As could be seen from fig. 7a, a double peak gradually emerges as the training progresses. This phenomenon probably results from the broken circuit symmetries, which moves the mean away from zero: recall that as characterized by corollary 5, the decay of odd moments results from the weight symmetries, and broken weight symmetries weaken the decay. We shall further discuss circuit-symmetry breaking later in supp. B G 8 and supp. C.

*b. Symmetric distributions of Hessian entries.* Although the symmetry of Hessian entries is not part of the assumptions that lead to the plasticity phase theorem, it is informative to corroborate the self-similarity between the basis circuits and eigenspectrum. Thus, we further plot in fig. 6a the probability density distributions of three randomly sampled Hessian entries throughout training, which has been given in section II F 4—we also have sampled dozens more entries and the entries here reflect the population's behaviors. From fig. 6a, we can see that the distributions are also approximately symmetric against the $y$-axis.

To conclude, the preceding phenomena quantitatively validate the assembly-symmetry assumption presented in supp. B G 3 and the coarse-grained effect of circuit symmetry on Hessian entries (i.e., neuron assemblies of perturbation of basis circuits of order two) hypothesized in supp. B E 6.

### 7. *Experimental validation of the assembly-diversity assumption*

In this subsection, we present experiment support for the assembly-diversity assumption. More specifically, as discussed in section II D 3, the experiments in this subsection is also intended to qualitatively validate the assembly-diversity assumption. And we show that during the training, each Hessian entry has a *very large absolute* coupling set size (i.e., the diversity control parameter) and a *very small relative* coupling set size compared with all the possible entries, and therefore, validate qualitatively the sparse dependency among Hessian entries.

To begin with, we describe the methods to validate the assumption. Recall that in section II D 3, we hypothesize the decay of moments of neuron assemblies, which motivates the sparse correlation assumption given in supp. B G 3. The decay is actually characterized as decay of cumulants, a well known alternative to moments to characterize the statistical behaviors of random variables, in the formal version of the diversity assumption given in asm. 2. To see the relationship between cumulants and moments, recall that the first-order moment is the same with first order cumulant, the second, third, fourth order cumulants are second, third, fourth order mean-normalized moments, respectively. Cumulants also have the appealing property that when random variables are mutually statistically independent, the cumulants of all orders among them varnish are zero. We review the definition of cumulants in supp. F A 1.

We compute the cumulants of Hessian entries to study the dependency between Hessian entries, which estimates coupling set sizes as explained in the following. As visualized in fig. 9 previously, for each Hessian entry $\alpha$, it has a coupling set $\mathscr{N}(\alpha)$, and for each entry $u_\beta, \beta \in \mathscr{N}$, $u_\beta$ is weakly correlated with entries outside the coupling set (i.e., $u_\gamma, \gamma \in \mathbb{I} \setminus \mathscr{N}(\alpha)$). In experiments, we interpret the weak correlation as statistical independence—as in the simplified diversity assumption given in simplified Assumption 2.A. We translate the relation into properties of cumulants that is computable as follows.

- **Covariance and coupling set size.** Given $u_\alpha, \alpha \in \mathbb{I}$, the number of non-zero covariances (i.e., the second order cumulants) among Hessian entries is the coupling set size $|\mathscr{N}(\alpha)|$ of $u_\alpha$: the statistical independence implies that $\kappa(\beta, \gamma), \beta \in \mathscr{N}_1, \gamma \in \mathbb{I} \setminus \mathscr{N}(\alpha)$ between $u_\beta$ and entries $u_\gamma$ outside the coupling set is zero, which implies that the number of non-zero normalized $\kappa(\beta, \gamma), \beta, \gamma \in \mathscr{N}(\alpha)$ would be the coupling set size $|\mathscr{N}|$.

- **Higher order cumulants and coupling set size.** Given $u_\alpha, \alpha \in \mathbb{I}$, the number of non-zero skewnesses, i.e., third order cumulants, and excess kurtoses, i.e., fourth order cumulants, would be $|\mathscr{N}|^2, |\mathscr{N}|^3$ respectively—we collect the definition of multivariate skewness and kurtosis in supp. I B 1—as explained in the following. In this case, the statistics involve $k = 3, 4$ sets. Suppose that $k$ Hessian entries are picked. If one of them is outside the coupling

sets of the rest, then the $k$-way cumulant is zero. More specifically, for skewness, the assumption corresponds to the phenomenon that for any Hessian entry $\alpha, \beta$, given three Hessian entries $\alpha_1, \beta_1, \gamma_1$, if at least one entry, e.g., $\gamma_1 \in \mathbb{I} \setminus (\mathcal{N}(\alpha) \cup \mathcal{N}(\beta)), \alpha_1 \in \mathcal{N}(\alpha), \beta_1 \in \mathcal{N}(\beta)$, does not come from the coupling set $\mathcal{N}(\alpha), \mathcal{N}(\beta)$ of $\alpha, \beta$, then the skewness $\kappa(\alpha_1, \beta_1, \gamma_1) = 0$. That implies that given a specific $\alpha$, $|\mathcal{N}|^2$ non-zero skewness are allowed. The same logic applies to kurtoses, and we could have $|\mathcal{N}|^3$ non-zero kurtoses.

We note that zero cumulants among Hessian entries here do no imply that the sample cumulants are zero in experiments. This is because of statistical fluctuations. More specifically, the cumulants are estimated through sample cumulants. For example, given two random variables $X, Y$, even if they are statistical independent, and thus $\mathbb{E}[XY] = 0$, the sample covariance $\frac{1}{m}\sum_{i=1}^{m} X_i Y_i$ is a random variable that fluctuates around zero—the zero cumulant only implies mean of the sample cumulant is 0. And thus to test whether cumulants among Hessian entries are zero (or in other words, whether they are statistical independent), we need to perform hypothesis test. The details are given in supp. I B.

We compute the non-zero cumulants of the DNN in the experiments (i.e., the VGGNet on CIFAR10 modified for binary classification) throughout training as well. For each entry, we compute the number of non-zero normalized covariances, i.e., Pearson correlation coefficients (CC), and compute their average. In addition, we also compute higher order cumulants, i.e., the skewness and excess kurtosis. The results are summarized in fig. 6 in section II F 4 and fig. 7c. [10]

*a. Sparse dependency in DNNs in practice, qualitative observations.* We draw the correlation coefficient matrices of Hessian entries at the beginning and end of training respectively of the VGG net, as shown in fig. 6. We can see at the start of the training (fig. 6b), the correlation coefficient matrix is very sparse in the sense that a vast majority of the entries are close to zero. At the end of the training (fig. 6c), more strong correlations emerge after the statistical information in data is learned, but the matrix is still sparse in the sense that most of the entries are still close to zero.

*b. Sparse dependency in DNNs in practice, quantitative estimations.* As explained previously, we quantitatively estimate the coupling set sizes by computing the averages (over all Hessian entries) of the number of non-zero covariances, skewnesses, and excess kurtoses respectively throughout training, and the result is given in fig. 7c. As shown by the light red line in fig. 7c at the end of the training, for a given Hessian entry $u_\alpha$, of overall $8.68 \cdot 10^{12}$ possible coefficients between $u_\alpha$ and $\boldsymbol{U}_{\mathbb{I}\setminus\{\alpha\}}$—the network contains $N = 8.68 \cdot 10^{12}$ number of parameters—$u_\alpha$ only correlates $3.39 \cdot 10^{-4}$ of them.

*c. Growth ratio of high order non-zero correlations.* The diversity assumption also predicts that the number of non-zero cumulants of all order would grow at a geometric sequence, as discussed earlier in this subsection. Figure 7c shows that the number of non-zero CCs, skewness, kurtoses roughly make up a geometric sequence throughout training. For example, at the end of the training, the sequence is $N^{3/2}, N^3, N^{9/2}$ with a common ratio of $N^{3/2}$. It shows that the average number of non-zero covariances, skewnesses and excess kurtoses, i.e, $|\mathcal{N}|$, $|\mathcal{N}|^2$ and $|\mathcal{N}|^3$, supports the diversity assumption. However, it also shows that the coupling set size $|\mathcal{N}|$ could be as large as roughly $N^{3/2}$ instead of $N^{1/2}$ in simplified Assumption 2.A. This is expected because the upper bound characterizes worst-case behaviors (cf. section II D 3), though it does not rule out the possibility that the upper bound of the diversity control parameter in the diversity assumption for theorem 2 could be improved to allow more dependency—however, this is considered as future works: rigorous results on the Wigner-type matrix with correlations are difficult and are an ongoing effort in the random matrix community in the past 60 years since Wigner [141] (1957) initialized the field, and we have built on the state-of-the-art results [55] (2019) of this type of random matrices.

To conclude, experimental results qualitatively validate the assembly-diversity assumption. Though the quantitative values of the diversity control parameters are only meaningful in a qualitative sense, and may vary as different hypothesis test methods are used to decide whether a non-zero cumulant is caused by statistical fluctuations, or by correlation among entries, it is evident that the DNN contains a very large absolute coupling set size and a very small relative coupling set size compared with all the possible entries. It qualitatively validates the sparse correlation among Hessian entries (and thus the cross-moment decay of neuron assemblies). We shall discuss the results from the perspective of a phase next in supp. B G 8.

### 8. *Plasticity phase of DNNs*

The presentation of this section largely follows the standard practice of mathematical results, where definitions, assumptions, theorems, and experimental validations are presented in sequel. Yet, in the narrative of this paper, as narrated in the introductory section I, this section is to study the symmetry-breaking (self-organizing) process of DNNs, and thus in subsection, we describe the symmetry-breaking process by synthesizing the results in this work, and the process suggests that the assumptions might demarcate a region of the state space that should be considered as a phase of DNNs, which we refer as the *plasticity* phase. We describe the process in the following.

*a. Initial state.* At the start of the self-organization, the neurons of a DNN constituent hierarchical circuits of circuit symmetries that compute a coarse-grained random variable whose uncertainty is to be minimized through a feedback-control loop (cf. supp. B D and B E). At this state, the coarse-grained effect of circuit symmetries manifest as the phenomena that the examples (from the dataset) are classified ran-

[10] Because some randomness exists in DNN training, e.g., the random initialization of weights and the sequence to process training examples, the experiments are run for three trials. Though the numbers reported in the figures fluctuates slightly from trial to trial, the reported phenomena, i.e. sparse dependency and a growth rate of $|\mathcal{N}|$ for the higher order correlations, are consistently observed.

domly with approximately fifty-fifty chance of being right (cf. fig. 8), the gradients (cf. supp. B F 2), the Hessian entries (cf. supp. B G 6) and the eigenvalues of Hessian (cf. supp. B G 5) are all distributed symmetrically against $y$-axis, respectively; and the means of Hessian entries are close to zero, and correlation among Hessian entries are sparse (cf. supp. B G 7).

*b. Symmetry breaking.* For each execution of the feedback-control loop, even with a fixed dataset, each batch of examples are novel examples that are an external perturbation of the DNN self-organizing system. The coarse-grained variable computed to predict the label of the examples is measured against the feedback signal/labels. In response to the perturbation—that is, the discrepancy between the coarse-grained output variable and the feedback signal—the perturbations/errors are back propagated to all neurons, and the system is excited to reduce the perturbation (cf. supp. B F). Correspondingly, the neurons of the DNN self-organize to encode information in the form of circuits, the circuit symmetries of a subset of the basis circuits break, and the perturbations/uncertainty/risk is reduced (cf. supp. B E). The broken weight symmetries would weaken the decay of the moments (cf. supp. B E 6), and more specifically, the means of and the moments/cumulants among Hessian entries. Experimentally, this decay manifests as the gradually emerging double peak of the distributions of Hessian entries' means (i.e., the symmetry control parameters) observed in supp. B G 6, and the gradually increasing correlation among Hessian entries measured in cumulants (i.e., the diversity control parameters) observed in supp. B G 7.

*c. Stable coarse-grained adaptive symmetry.* For a DNN that is hierarchically large and of sufficient circuit symmetries (relatively to the dataset)—which is formulated as assumptions in supp. B G 3—the broken circuit symmetries are a minority compared with the intact circuit symmetries. And thus the coarse-grained effect of the coexistence of intact and broken circuit symmetries manifests as the phenomena that the means of Hessian entries still fluctuate very close to zero, the correlation among Hessian entries is still sparse, and the distributions of weights, gradients, Hessian entries and eigenvalues of Hessian are all approximately symmetric throughout training, respectively. Therefore, the risk could be continually decreased.

*d. Uncertainty minimized.* Each batch is a bootstrap sample of the dataset, and as the training examples are repeatedly sampled to the system, statistically, the excitation of the system induced by the perturbations gradually becomes smaller, and eventually reaches zero because the dataset stops being novel perturbations to the system. Experimentally, this reflects as the phenomena that the empirical risk, and the support of the distributions of gradients, Hessian entries and Hessian eigenspectrum, respectively, gradually converge to zero. As a result, the risk of the dataset is zero and the self-organizing process finishes—however, the system still possesses many weights that are of weight symmetry, and if novel examples are fed to the system, non-zero eigenvalues would emerge and half of them would be negative again (cf. corollary 7).

Recall that in section II F, we have explained that a collection of states with stable symmetries is referred as a phase in physics. Thus, to refer to the behaviors of DNNs in the preceding self-organizing process in a conceptually compact way, we interpret the collection of states, where circuit symmetries stably exist (along with broken circuit symmetries) to manifest adaptive symmetry at the level of assemblies (i.e., symmetry of the gradient distribution, and the eigenspectrum of Hessian), as a phase of DNNs, which we refer as the **plasticity phase**.

### H. Formal version of the plasticity phase theorem

In this section, we present the formal version of theorem 2 that previously has been given informally in supp. B G 4. We begin by introducing the key ideas behind the proof in supp. B H 1. Then, we proceed to formally present the results.

First, we present the assumptions of the theorem. In supp. B H 2, we shall formally present the assembly-diversity assumption that has been previously presented in a simplified version in supp. B G 3. In addition to the assumptions that have been previously given in supp. B G 3, in supp. B H 3, we shall further present two more assumptions on regularities—here regularity refers to non-existence of singularities, e.g., having finite moments—of statistics of Hessian, which are referred as the *boundedness* assumption and the *stability* assumption, respectively. Overall, though also characterizing cumulant decay among Hessian entries, they could roughly be understood as formal technicalities to avoid infinity. And recall that in section II D 3, we have discussed that the assumptions are to qualitatively, not exactly, characterize the behaviors of DNNs. Therefore, these more technical aspects are not included in the narrative in supp. B G.

Then, we formally present the plasticity theorem. In supp. B H 4, we present preliminary definitions needed to formally present the theorem. In supp. B H 5, the formal version of theorem 2 is presented, and the relationship between the theorem and the experiments is discussed in more depth. Also, we present the proof sketch of the theorem. The full proof is given at supp. G.

To begin with, we introduce some new notations. Let

$$\boldsymbol{A} := \mathbb{E}[\boldsymbol{H}], \frac{1}{\sqrt{N}}\boldsymbol{U} := \boldsymbol{H} - \boldsymbol{A}, \mathscr{S}[\boldsymbol{R}] := \frac{1}{N}\mathbb{E}_{\boldsymbol{U}}[\boldsymbol{URU}] \quad (102)$$

where $\mathscr{S}[\boldsymbol{R}]$ is a linear operator on the space of matrices, and the expectation in $\mathscr{S}$ is taken w.r.t. $\boldsymbol{U}$ while keeping $\boldsymbol{R}$ fixed. $\boldsymbol{U}$ is the Hessian normalized by mean subtraction, and rescaling.

#### 1. *High-dimensional-probability analysis of the random Hessian matrix with correlations*

We give a high level introduction to the idea underlying the theorem in this section.

The phenomenon characterized by the theorem is broadly known as the *concentration-of-measure* phenomenon. The simplest example would be the well-known normal distribution. Given an ensemble of i.i.d. random variables with zero mean, because the random variables are independent with each other, and have an equal probability being positive, or negative, they tend to cancel each other out when averaged, symmetrically

spread against $y$-axis, and converge to a normal distribution. Thus, sampling many samples from the average of the ensemble, 95% of them would concentrate in the range between $[+2\sigma, 2\sigma]$, where $\sigma$ is the standard deviation of the ensemble.

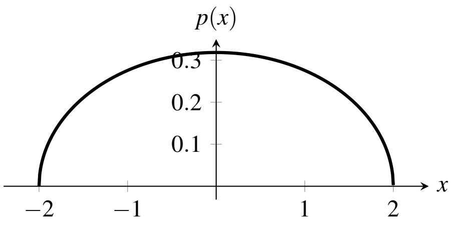


FIG. 10. Eigenspectrum of Wigner matrix. The $x$-axis is the numerical value of eigenvalues, and the $y$-axis is the probability of obtaining an eigenvalue of a specific numeric value if we randomly sample an eigenvalue of all the eigenvalues of $\boldsymbol{A}_N$.

What we need is the concentration of measure in the space of matrices. The phenomena manifests clearest in the simplest kind of Wigner-type matrix, i.e., the *Wigner matrix*. A Wigner matrix is a matrix whose entries are independent identically distributed univariate Gaussian random variables. Its *eigenspectrum*—the probability density distribution of eigenvalues—is probabilistically close to a function that is a closed-form solution to a scalar equation; the function is illustrated in fig. 10. The eigenspectrum of Wigner matrix is symmetric w.r.t. the $y$-axis, which implies half of its non-zero eigenvalues are negative. More verbosely, for $1 \leq i < j < \infty$, let $a_{ij}$ be i.i.d. random variables with zero mean and unit variance, and $a_{ij} = a_{ji}$. Then $\boldsymbol{A}_N = [a_{ij}]_{i,j=1}^N$ is a matrix with random entries. It is the classic random matrix named Wigner matrix. Given an eigenvector $\boldsymbol{t}$ of $\boldsymbol{A}_N$, we know that when we multiply it with $\boldsymbol{A}$, we have $(\boldsymbol{At})_i = \sum_k a_{ik}t_k$. Note that when $\{a_{ik}t_k\}_{k=1,\ldots,N}$ are i.i.d. random variables, $a_{ik}t_k$ also tend to cancel each other out and spread symmetrically around 0, resulting that eigenvalues behave similarly. Thus, when the dimension of the matrix $N$ is large enough, we would have the eigenspectrum of the distribution shown in fig. 10. It is termed *semi-circle law*. The eigenspectrum is obtained by solving a *self-consistent* equation as following

$$1 + (z + m)m = 0, \Im m > 0, \Im z > 0$$

where $z$ is a constant complex number, $m$ is the unknown complex number to solve. Then, we apply *inverse stieltjes transform* (c.f. lemma 7) to get the spectrum.

Note that Wigner matrix has very strong requirements on its entries: independent identically distributed. However, notice that the key phenomenon we need is just the concentration of measure; that is, $\{a_{ik}t_k\}_{k=1,\ldots,N}$ tend to cancel out and spread around 0 with similar chances of being positive or negative, resulting in a close-to-zero symmetric eigenvalue distribution. Thus, the required assumptions are just that the Hessian entries are of zero mean, and of sparse correlations with one another to obtain a semi-circle-law-like eigenspectrum. Erdos *et al.* [55] proves a more sophisticated phenomenon of Wigner-type matrices with correlations than that of Wigner matrix: stating in an over-simplifying way, given a matrix $\boldsymbol{H} \in \mathbb{R}^{N\times N}$, for each given entries $h_\alpha$, if it does not couple with more than $\sqrt{N}$ of all the $N^2$ entries, then by a high-probability bound, the eigenspectrum of $\boldsymbol{H}$ are close to the solution to a matrix equation known as *Matrix Dyson Equation*, a matrix version of the preceding self-consistent equation—a high-level, more detailed description of the sparse correlation that leads to the equation is further given in supp. F A 2. Such sparse correlation has been illustrated in fig. 9. By such assumptions, the eigenspectrum of Hessian can be obtained from $\boldsymbol{G}$, given as the solution to the equation

$$\boldsymbol{I} + (z - \boldsymbol{A} + \mathscr{S}[\boldsymbol{G}])\boldsymbol{G} = \boldsymbol{0}, \Im \boldsymbol{G} \succ \boldsymbol{0}, \Im z > 0, \tag{103}$$

where $z$ is still a complex number, $\boldsymbol{G}$ is the unknown complex matrix to solve, $\Im \boldsymbol{G}$ denotes the imaginary part of $\boldsymbol{G}$, $\Im \boldsymbol{G} \succ 0$ means $\Im \boldsymbol{G}$ is positive definite, $\boldsymbol{A}$ and $\mathscr{S}[\boldsymbol{G}]$ are defined previously at eq. (102). And if the mean of the matrix $\boldsymbol{A}$ is a zero matrix, we further prove that the eigenspectrum obtained from such an equation is symmetric w.r.t. $y$-axis, which is the plasticity phase theorem.

### 2. *Assembly-diversity assumption*

In this subsection, we present the full version of the simplified assembly-diversity assumption given in supp. B G 3.

To convey the core idea, we still first present a simplified assumption as an example before giving the assumption in the full form.

**Simplified Assumption 2.B.** *There exists $\mu > 0$ such that the following holds: for every $\alpha \in \mathbb{I}$, there exists two sets $\mathscr{N}_k = \mathscr{N}_k(\alpha), k = 1,2$ such that $\alpha \in \mathscr{N}_1 \subset \mathscr{N}_2 = \mathscr{N} \subset \mathbb{I}, |\mathscr{N}| \leq N^{1/2-\mu}$ and*

$$\kappa(f(\boldsymbol{U}_{\mathbb{I}\setminus\mathscr{N}}), g(\boldsymbol{U}_{\mathscr{N}_1})) \leq N^{-3}||f||_3||g||_3,$$

*for any functions $f, g$, where $||||_3$ is the $L^3$ norm on function space.*

The assumption characterizes the a sparse statistical dependence among Hessian entries as explained in the following. The assumption states that for each Hessian entry, it has a set $\boldsymbol{U}_{\mathscr{N}_1}$ of Hessian entries that it could potentially strongly correlate, and for entries outside this set (i.e., $\boldsymbol{U}_{\mathbb{I}\setminus\mathscr{N}}$), it only very weakly correlate with them. More specifically, because the assumption holds for any function $f, g$, $\forall \beta \in \mathscr{N}_1$ and $\forall \gamma \in \mathbb{I}\setminus\mathscr{N}$, let $f(\boldsymbol{U}_{\mathbb{I}\setminus\mathscr{N}}) = u_\gamma$ and $g(\boldsymbol{U}_{\mathscr{N}_1}) = u_\beta$, and we have

$$\kappa(u_\beta, u_\gamma) \leq N^{-3}\left(\kappa(u_\beta^3)\kappa(u_\gamma^3)\right)^{-3},$$

where $\kappa(u_\beta, u_\gamma)$ denotes the covariance of entries $u_\beta, u_\gamma$ of $\boldsymbol{U}$, and $\kappa(u_\beta^3), \kappa(u_\gamma^3)$ denotes the mean of $u_\beta^3, u_\gamma^3$, respectively. Thus, cumulants across sets decay with an extra decay factor $N^{-3}$ compared with the cumulants within sets. Recall that the varnishing of cross-cumulants implies statistical independence between random variables. Therefore, suppose higher cumulants varnish, then the decay of $\kappa(u_\beta, u_\gamma)$ implies the

diminishing statistical independence between $u_\beta, u_\gamma$. The decay that holds for any function $f, g$ characterizes a statistical independence between the two sets $\boldsymbol{U}_{\mathbb{I}\backslash\mathcal{N}}, \boldsymbol{U}_{\mathcal{N}_1}$ of random variables. To help understand the sparsity, or, the size of $\mathcal{N}$ intuitively, we have illustrated it with fig. 9 earlier. The coupling set size $|\mathcal{N}|$ provides a parameter to summarize the interaction among Hessian entries.

Simplified Assumption 2.B characterizes the statistical dependence of one Hessian entry against the rest of entries, and we need to characterize the statistical dependence among arbitrary combination of Hessian entries, which is the assembly-diversity assumption given in the following.

**Assumption 2** (Assembly Diversity)**.** *There exists $\mu > 0$ such that the following holds: for every $\alpha \in \mathbb{I}$ and $q, R \in \mathbb{N}$, there exists a sequence of nested sets $\mathcal{N}_k = \mathcal{N}_k(\alpha)$ such that $\alpha \in \mathcal{N}_1 \subset \mathcal{N}_2 \subset \cdots \subset \mathcal{N}_R = \mathcal{N} \subset \mathbb{I}, |\mathcal{N}| \leq N^{1/2-\mu}$ and*

$$\kappa\Big(f(\boldsymbol{U}_{\mathbb{I}\backslash\cup_j\mathcal{N}_{n_j+1}(\alpha_j)}), g_1(\boldsymbol{U}_{\mathcal{N}_{n_1}(\alpha_1)\backslash\cup_{j\neq 1}\mathcal{N}(\alpha_j)}), \ldots, g_q(\boldsymbol{U}_{\mathcal{N}_{n_q}(\alpha_q)\backslash\cup_{j\neq q}\mathcal{N}(\alpha_j)})\Big) \leq N^{-3q}||f||_{q+1}\prod_{j=1}^{q}||g_j||_{q+1}, \tag{104}$$

*for any $n_1, \ldots, n_q < R$, $\alpha_1, \ldots, \alpha_q \in \mathbb{I}$ and functions $f, g_1, \ldots, g_q$, where $||||_p, p \in \mathbb{N}$ is the $L^p$ norm on function space.*

**Remark 12.** *The sparse dependency between entries are referred as correlation decay in Erdos* et al. *[55], which refers to the phenomenon that the correlation between entries are decayed slowly w.r.t. a certain distance metric between entries. This characterization is largely historical and context-dependent: in physical systems, the correlation normally decays w.r.t. the distance between units, a setting that is studied by many previous works on random matrices with correlations. However, a novelty in Erdos* et al. *[55] is to use a neighborhood criterion that do not have such a distance metric. Meanwhile, the neighborhood is denoted as coupling set in this work because the physical distance among circuits is not meaningful. Correspondingly, it is more descriptive to refer the phenomenon as sparse dependency. And thus, we have referred the random matrix with slow correlation decay as the random matrix with sparse dependency.*

Instead of just characterizing the cross-cumulants between two sets, the assumption here characterize the higher order cumulants among $q$ sets, each of which is a coupling set of a Hessian entry, and thus characterizes the statistical dependency among Hessian entries through the higher order cumulants of arbitrary combination of Hessian entries. To generalize the example from the two-set case, let $\{u_{\alpha_i}\}_{i=1,\ldots,q}$ be $q$ Hessian entries, and thus each of them has a coupling set $\mathcal{N}(\alpha_i)$. Let $\beta_i \in \mathcal{N}_{n_i}(\alpha_i), i = 1, \ldots, q$, and $\gamma \in \mathbb{I}\backslash\cup_{i=1}^{q}\mathcal{N}_{n_i}(\alpha_i)$, then for any $(q+1)$-way cumulant $\kappa(\beta_1, \ldots, \beta_q, \gamma)$, it satisfies $\kappa(\beta_1, \ldots, \beta_q, \gamma) \leq N^{-3q}\left(\prod_{i=1}^{q}\kappa(u_{\beta_i}^3)\right)^{-3}$. Therefore, the assumption also characterizes the decay of cumulants that cross sets. Note that the order of $\beta_i, \gamma$ is exchangeable, thus the ordering in the indices is arbitrary. Here cumulants are referred with the same symbol $\kappa$ because covariance is second-order cumulant. For regular probability distributions as that in DNNs, the cumulants uniquely determines the probability distribution, and thus the cumulants uniquely characterize the statistical dependency between Hessian entries.

### 3. *Regularity assumptions*

As explained in supp. B H 2, the assembly-diversity assumption characterizes the cumulant decay across coupling sets of Hessian entries, however, it does not characterize the strength of the correlation within a coupling set of a Hessian entry. In this subsection, we present regularity assumptions that characterize the overall strength of correlation among Hessian entries, which roughly states that the correlation should be less than infinity; that is, bounded.

We first present a boundedness assumption. As previously, we first state the assumption that only involves second-order statistics to convey the intuition of the assumption.

**Simplified Assumption 3.A** (Boundedness Simplified)**.** *The statistics of $\boldsymbol{U}$ satisfy the following:*

1. *$\exists\mu, \sigma \in \mathbb{R}, \forall\alpha \in \mathbb{I}, \mathbb{E}[|u_\alpha|] \leq \mu, \mathbb{E}[|u_\alpha|^2] \leq \sigma$;*
2. *For any $\varepsilon > 0, \exists C_1, C_2(\varepsilon) \in \mathbb{R}$, where $C_2(\varepsilon)$ depends on $\varepsilon$, $|||\kappa|||_2^{iso} \leq C_1, |||\kappa|||_2 := |||\kappa|||_2^{av} + |||\kappa|||_2^{iso}, |||\kappa|||_2 \leq C_2(\varepsilon)N^\varepsilon$.*

The first part of the assumption is straightforward. It states that the mean and variance of $u_\alpha$ are bounded. The second part is more complicated. It asks certain averages of all covariance between entries of $\boldsymbol{U}$ are bounded, measured by certain norms. In any DNNs of a finite size, the mean, covariance, and the norms are finite, and thus the assumptions hold. We explain the technicalities of the second part of the assumption as follows.

First, we explain the non-uniform bound. The bound $|||\kappa|||_2 \leq C_2(\varepsilon)N^\varepsilon$ asks for a non-uniform bound w.r.t. $N$: since $|||\kappa|||_2$ is required to be smaller than $C(\varepsilon)N^\varepsilon$, its upper bound can grow with $N$.

Second, we explain the norms. $||\cdot||^{\mathrm{av}}$ and $||\cdot||^{\mathrm{iso}}$ are norms that characterize the largest of certain weighted averages of all the covariances. They are norms defined in Erdos *et al.* [55], whose exact forms are of minor interests here: recall that theorem 2 aims to qualitatively characterize the behaviors of DNNs, and in this work although the bounds characterize that in certain quantitative ways the correlations are bounded, the bounds are only meaningful is the way that it qualitatively characterizes correlations are not infinite. Therefore, we shall collect the definitions in supp. F A 3, and illustrate the intuition of the norm using $|||\kappa|||_2^{\mathrm{av}}$ as an example, where av stands for average. $\forall\alpha, \beta \in \mathbb{I}$, denote $\alpha := (a_1, a_2), \beta := (b_1, b_2)$, and let $\boldsymbol{K}^{\mathrm{av}}$ be the matrix, of which

$$\boldsymbol{K}^{\mathrm{av}}_{a_1N+a_2, b_1N+b_2} := |\kappa(\alpha, \beta)|;$$

note that $\boldsymbol{K}^{\mathrm{av}}$ is a $N^2 \times N^2$ matrix, and each row of $\boldsymbol{K}^{\mathrm{av}}$ is the covariances of $u_\alpha$ with all entries (including $u_\alpha$ itself) of

$\boldsymbol{U}$. Let $||\boldsymbol{K}^{\text{av}}||$ denote $|||\kappa|||_2^{\text{av}}$, the 2-norm of $\boldsymbol{K}^{\text{av}}$. $||\boldsymbol{K}^{\text{av}}||$ characterizes a collective behavior of all the covariances. To understand the characterization, recall the definition of $||\cdot||$ on matrix as follows.

$$||\boldsymbol{K}^{\text{av}}|| = \max_{||\boldsymbol{x}||\leq 1} \boldsymbol{x}^T \boldsymbol{K}^{\text{av}} \boldsymbol{x}$$
$$= \max_{||\boldsymbol{x}||\leq 1} \sum_{a_1=1,b_1=1,a_2=1,b_2=1}^{a_1=N,b_1=N,a_2=N,b_2=N} x_{a_1N+b1} |\kappa(a_1b_1,a_2b_2)| x_{a_2N+b2}.$$

Thus, it is the largest possible weighted average of all the absolute covariances. Simplified Assumption 3.A asks the largest weighted average to be finite. $|||\kappa|||_2^{\text{iso}}$ defines a similar quantity with $|||\kappa|||_2^{\text{av}}$, and interested readers may refer its definition to definition 35 in supp. F A 3.

The full version of the boundedness assumption is presented as follows.

**Assumption 3** (Boundedness)**.** *The statistics of* $\boldsymbol{U}$ *satisfy the following:*

1. $\forall q \in \mathbb{N}, \exists \mu_q \in \mathbb{R}, \forall \alpha \in \mathbb{I}, \mathbb{E}[|\boldsymbol{U}_\alpha|^q] \leq \mu_q$.
2. $\forall R \in \mathbb{N}, \varepsilon > 0, \exists C_1, C_2(\varepsilon) \in \mathbb{R}$*, where* $C_2(\varepsilon)$ *depends on* $\varepsilon$*, we have* $|||\kappa|||_2^{iso} \leq C_1, |||\kappa||| \leq C_2(\varepsilon)N^\varepsilon$.

The first part of the assumption similarly asks that the mean, covariance, and all higher order moments to be finite. The second part replaces the $|||\kappa|||_2$ with a norm $|||\kappa|||$ that involves the cumulant of all orders. And similarly for reasons given in the explanation of simplified Assumption 3.A, we do not elaborate the technicalities of the norm. Interested readers may refer to supp. F A 3.

In addition to the boundedness assumption, an assumption that characterizes the regularity of the operator $\mathscr{S}$ (defined at eq. (102)) is needed.

**Assumption 4** (Stability)**.** $\exists 0 < c < C, \forall \boldsymbol{T} \succeq \boldsymbol{0}, c\, N^{-1} tr\, \boldsymbol{T} \preceq \mathscr{S}[\boldsymbol{T}] \preceq CN^{-1} tr\, \boldsymbol{T}$.

This is also an assumption similar to asm. 3, that ensures $\mathscr{S}[G]$ in eq. (103) is bounded in reference to the trace of its argument $\boldsymbol{T}$: $\mathscr{S}[\boldsymbol{G}]$ needs to stay in an interval that is comparable to tr $\boldsymbol{G}$—neither explodes ($\preceq CN^{-1}\text{tr}\, \boldsymbol{T}$), nor degenerates ($c\, N^{-1}\text{tr}\, \boldsymbol{T} \preceq$). The assumption ensures the stability of eq. (103). More specifically, to appreciate the assumption, we could expand $\mathscr{S}[\boldsymbol{T}]$ as

$$\mathscr{S}[\boldsymbol{T}] = \int \boldsymbol{U}\boldsymbol{T}\boldsymbol{U}\rho(\boldsymbol{U})d\boldsymbol{U},$$

where $\rho(U)$ is the law of the matrix $\boldsymbol{U}$. $\mathscr{S}[\boldsymbol{T}]$ is also a symmetric matrix. And given that $\boldsymbol{T} \succeq \boldsymbol{0}$, for any vector $\boldsymbol{x} \in \mathbb{R}^N$, we have

$$\boldsymbol{x}^T\mathscr{S}[\boldsymbol{T}]\boldsymbol{x} = \int \boldsymbol{x}^T\boldsymbol{U}\boldsymbol{T}\boldsymbol{U}\boldsymbol{x}\rho(\boldsymbol{U})d\boldsymbol{U} = \int (\boldsymbol{U}\boldsymbol{x})^T\boldsymbol{T}\boldsymbol{U}\boldsymbol{x}\rho(\boldsymbol{U})d\boldsymbol{U},$$

which is a weighted sum of positive semi-definite matrices. The lower bound in the assumption asks that such sum of positive semi-definite matrices to be positive definite, i.e., not degenerating to contain zero eigenvalues, whereas the upper bound asks its eigenvalues to be finite. The lower bound essentially requires that for any $\boldsymbol{x}, \boldsymbol{T}$, $(\boldsymbol{U}\boldsymbol{x})^T\boldsymbol{T}\boldsymbol{U}\boldsymbol{x} > 0$ is of nonzero probability. We provide examples in the following to help appreciate the bound.

- Consider a more extreme case, where $\boldsymbol{U}$ becomes a zero matrix. In this case, the lower bound is violated, and the eigenspectrum becomes a singular point at zero. Though the eigenspectrum could still be considered as symmetric, but the benign risk landscape does not exist. The lower bound requires some safe margin away from degeneration.

- Let $\boldsymbol{T}$ be a diagonal matrix with a single non-zero entry at $(i,i)$, we have $\mathscr{S}[\boldsymbol{T}]_{pq} = (1/N)t_{ii}\mathbb{E}[u_{pi}u_{iq}]$. Further letting $\mathbb{E}[u_{pi}u_{iq}] = 0, p \neq q$, $\mathscr{S}[\boldsymbol{T}]$ is thus a diagonal matrix with diagonal elements $s_{pp} = (t_{ii}/N)\mathbb{E}[u_{pi}^2]$ (recall $\boldsymbol{U}$ is symmetric). The assumption asks the variance $\mathbb{E}[u_{pi}^2], p = 1\ldots N$ to be within the interval $[c, C]$.

## 4. *Preliminary definitions*

To present the theorem formally, we need some further definitions. The following definitions can be found in Tao [293] unless otherwise noted.

The theorem is about the relationship between the sparse dependency and the eigenspectrum of the Hessian. The eigenspectrum is studied as empirical spectral distribution (ESD) in random matrix theory [293].

**Definition 29** (Empirical Spectral Distribution)**.** *Given a* $N \times N$ *random matrix* $\boldsymbol{H}$*, its empirical spectral distribution* $\mu_{\boldsymbol{H}}$ *is*

$$\mu_{\boldsymbol{H}} = \frac{1}{N}\sum_{i=1}^{N} \delta_{\lambda_i}$$

*where* $\{\lambda_i\}_{i=1,\ldots,N}$ *are all eigenvalues of* $\boldsymbol{H}$ *and* $\delta_{\lambda_i}$ *is the delta function* $\delta(x-\lambda_i)$.

Given a hermitian matrix $\boldsymbol{H}$, its ESD $\mu_{\boldsymbol{H}}(\lambda)$ can be studied via its resolvent $\boldsymbol{G}$.

**Definition 30** (Resolvent)**.** *Let* $\boldsymbol{H}$ *be a normal matrix, and* $z \in \mathbb{H}$ *a spectral parameter. The* **resolvent** $\boldsymbol{G}$ *of* $\boldsymbol{H}$ *at* $z$ *is defined as*

$$\boldsymbol{G} = \boldsymbol{G}(z) = \frac{1}{\boldsymbol{H}-z}$$

*where*

$$\mathbb{H} := \{z \in \mathbb{C} : \Im z > 0\}$$

$\mathbb{C}$ *denotes the complex field, and* $\Im$ *is the function returns imaginary part of a complex number* $z$.

Resolvent $\boldsymbol{G}$ is related to eigenspectrum of $\boldsymbol{H}$ through stieltjes transform of $\mu_{\boldsymbol{H}}(\lambda)$.

**Definition 31** (Stieltjes Transform)**.** *Let $\mu$ be a Borel probability measure on $\mathbb{R}$. Its Stieltjes transform at a spectral parameter $z \in \mathbb{H}$ is defined as*

$$m_\mu(z) = \int_{\mathbb{R}} \frac{d\mu(x)}{x-z}$$

The normalized trace of $\boldsymbol{G}$ is stieltjes transform of eigenspectrum of $\boldsymbol{H}$

$$m_{\mu_{\boldsymbol{H}}}(z) = \frac{1}{N}\text{tr } G$$

For a proof, the reader may refer to proposition 2.1 in Alt *et al.* [56].

$\mu_{\boldsymbol{H}}$ can be recovered from $m_{\mu_{\boldsymbol{H}}}$ through the inverse formula of Stieltjes-Perron.

**Lemma 7** (Inverse Stieljies Transform)**.** *Suppose that $\mu$ is a probability measure on $\mathbb{R}$ and let $m_\mu$ be its Stieltjes transform. Then for any $a < b$, we have*

$$\mu((a,b)) + \frac{1}{2}[\mu(\{a\}) + \mu(\{b\})] = \lim_{\Im z \to 0} \frac{1}{\pi}\int_b^a \Im m_\mu(z) d\Re z$$

*where $\Re$ is a function that returns the real part of $z$.*

**Remark 13.** *We give a short and rather informal explanation on the intuition behind the inverse Stieltjes transform, and more details can be found at Tao [293, p. 144]. Given $z = a + ib$, the imaginary part of the Stieltjes transform $m_\mu$ of $\mu$ can be written as*

$$\Im m_\mu(a+ib) = \pi\mu * P_b(a),$$

*where $*$ denotes convolution and*

$$P_b(x) := \frac{1}{\pi}\frac{b}{x^2+b^2}.$$

*$P_b(x)$ is known as the Poisson kernel and forms a family of approximations to identity. Thus, $\mu * P_b$ converges in the vague topology to $\mu$ as $b \to 0$.*

## 5. *The plasticity phase theorem*

If the assumptions asm. 1 2 3 4 hold, we would have the following theorem.

**Theorem 2.** *Let $R_m(T)$ be the empirical risk function (defined at eq. (50)) of a DNN $T$ with $n_L = 1$ (defined at eq. (48)) with a loss function $\mathscr{L}$ of class $\mathscr{L}_0$ (given at definition 15). If the Hessian $\boldsymbol{H} \in \mathbb{R}^{N\times N}$ (c.f. eq. (100)) of $R_m(T)$ satisfies assumptions 1 2 3 4, and let $\boldsymbol{M}$ be the solution to the Matrix Dyson Equation given at eq. (102). Then the resolvent $\boldsymbol{G}$ of $\boldsymbol{H}$ satisfies the following.*

1. *$\boldsymbol{G}$ is close to $\boldsymbol{M}$ in the sense of the following probability bound. For any $\gamma, \varepsilon > 0$, there exists $\delta > 0$, such that for all $D > 0$, give any $z \in \mathbb{D}_\gamma^\delta$, we have*

$$P\left(|tr\ (\boldsymbol{BG}(z) - \boldsymbol{M}(z))| \le ||\boldsymbol{B}||\frac{N^\varepsilon}{N\Im z}\right) \ge 1 - CN^{-D}, \quad (105)$$

*where $\boldsymbol{B}$ is an arbitrary deterministic matrix, $N$ is the dimension of $\boldsymbol{H}$, $C > 0$ is a constant depending on $D, \varepsilon, \gamma$ and constants in assumption 2 3. $\varepsilon$ can be chosen small, so $||\boldsymbol{B}||\frac{N^\varepsilon}{N\Im z}$ approaches zero as N grows. The region $\mathbb{D}_\gamma^\delta$ is roughly the region in the complex plane around the intervals that are inside the support of $\mu_{\boldsymbol{H}}$, where $\mu_{\boldsymbol{H}}$ is the empirical spectral distribution of $\boldsymbol{H}$. Formally, it is defined as*

$$\mathbb{D}_\gamma^\delta := \{z \in \mathbb{H} \mid |z| \le N^{C_0}, \Im z \ge N^{-1+\gamma},$$
$$\mu_{\boldsymbol{H}}(x) + dist(x, supp\mu_{\boldsymbol{H}}) \ge N^{-\delta}\},$$

*where $\mathbb{H}$ is the complex domain, and $C_0$ is a constant larger than 100.*

2. *The eigenvalue probability density distribution $\mu_{\boldsymbol{M}}$ recovered from $\boldsymbol{M}$ through inverse Stieljies transform (lemma 7) is symmetric w.r.t. y-axis, i.e., $\mu_{\boldsymbol{M}}(-x) = \mu_{\boldsymbol{M}}(x), x \in \mathbb{R}$, and $supp\mu_{\boldsymbol{M}}$ is a finite union of closed intervals with nonempty interior, where $supp\mu_{\boldsymbol{M}}$ denotes the support of $\mu_{\boldsymbol{H}}$.*

**Remark 14.** *A note on the generality of the theorem. First, though the network $T$ is restricted to be of an MLP defined in eq. (48), it is chosen for clarity of the presentation. Because the assumptions are on the Hessian entries, the theorem can be generalized to any networks with a feedforward architecture, (e.g., Convolutional Neural Network [11]) though the details of the Hessian entries, i.e., eq. (101), would be different. Nonetheless, the satisfaction of the assumptions in these networks in practice is another matter and does not necessarily comply with the theoretical assumptions, but should be studied in case-by-case fashion.*

**Remark 15.** *The region $\mathbb{D}_\gamma^\delta$ might need some explanations. Recall in remark 13, $\Im m_{\mu_{\boldsymbol{H}}}$ converges to $\mu_{\boldsymbol{H}}$ as $\Im z$ approaches 0. When N is large, the lower bound of $\Im z$, i.e., $N^{-1+\gamma}$, which is attainable, converges to 0, and thus the probability density function recovered from $m_{\mu_{\boldsymbol{M}}}$ also converges to $\mu_{\boldsymbol{M}}$, i.e., the eigenspectrum of $\boldsymbol{M}$. Therefore, the closeness, in the sense of the probability bound, between $\boldsymbol{G}$ and $\boldsymbol{H}$ in the domain $\mathbb{D}_\gamma^\delta$ also leads to the closeness between the eigenspectrum of them. The probability bound is discussed in the main thread below.*

As previously discussed in supp. B G 4, the theorem is intended to qualitatively, not exactly, characterize the behaviors of DNNs in the sense that close-to-zero mean of and sparse correlation among Hessian entries would induce symmetrically distributed eigenvalues. Now, with the technical details available here, we discus the relationship between the theorem and the experiments in more depth.

We elaborate the relationship between the probability bound and the experiments in the following. The non-asymptotic probability bound eq. (105) characterizes that the probability that the eigenspectrum of the Hessian $\boldsymbol{H}$ of DNNs is symmetric grows at a rate of $1 - CN^{-D}$ w.r.t. $N$ (note that $C > 0, D > 0$ are constants). Such characterization identifies a relationship between the control parameters (i.e. mean of Hessian and coupling set size) and the symmetry of the eigenspectrum (that

characterizes the coarse-grained effect of circuit symmetry on Hessian eigenspectrum); in other words, the relationship between the coarse-grained effect of circuit symmetries on Hessian entries, and the coarse-grained effect of circuit symmetries on Hessian spectrum. As discussed in section II D 3, such non-asymptotic high probability bounds frequently appear in statistical learning theory, where the generalization upper bounds characterize the generalization errors of hypotheses. As in the cases there, the probability bound here characterizes experiments qualitatively: despite being quantitative characterization, its exact value is not very informative because it characterizes the worst-case behaviors, achieved through a series of inequalities that enlarge the left hand side whose accumulative effects usually result in a loose bound compared with the statistical behavior in experiments. However, the bounds are relevant in the sense that they identify relevant quantities/parameters that parameterize the hypothesis space, and by studying the quantities or controlling the parameters, qualitative predictions can be made on the behaviors of the hypotheses[11]. For example, in addition to the margin of support vector machine mentioned in section II D 3, for Wigner matrix (cf. supp. B H 1), where $N$ is required to be large, but the semi-circle manifests at $N \sim 100$. And thus, the phenomenon predicted by the probability bound is validated by observing the behaviors of the samples at reasonably large $N$. In our case, as the experiments from supp. B G 5 to supp. B G 7 show, the behaviors characterized by the assumptions and the bound manifest at finite $N$ of DNNs (i.e., VGGNet) in practice that are considered small (compared with billion-parameters models nowadays, e.g., GPT-3 [294])—actually such a network still has $\sim 10^7$ number of parameters (cf. the experiment details in supp. H B), and implies a Hessian matrix of $\sim 10^{14}$ number of entries, and is still very large.

[11] This is also why we refer the asm. 3 and asm. 4 as regularity assumptions: the regularity assumptions are about regularity of the Hessian that rules out infinity and degeneration and are artifacts/technicalities resulting from mathematization. Rigorously speaking, the regularity assumptions contribute to the constants in the probability bound in theorem 2: constants $C_1, C_2$ and $N^{\varepsilon}$ in asm. 3 contribute to the constant $C$ and to the constant $D$, respectively, in the probability bound given at eq. (105); that is, the rate of convergence of $\boldsymbol{G}$ to $\boldsymbol{M}$, i.e., the resolvent matrix with a symmetric eigenspectrum. And thus, to mathematically guarantee the left hand side of eq. (105) is close to 1, the rate $C$ is needed to be small enough to make the probability bound on the resolvent hold. Thus, when the cumulant norms grow in a rate comparable to $N$, $N^{-D}$ may not be able to compensate the large $C$, and the bound might be vacuous. In Erdos *et al.* [55], to theoretically guarantee the left hand side of eq. (105) is close to 1, constant $C_1, C_2$ needs to exist uniformly w.r.t. $N$, so that when $N$ is large enough, the high probability bound is close to 1. However, as discussed in this paragraph, the exact value (which the constants contribute to) is of a minor concern in this work, and is the qualitative behavior characterized by the bound that is relevant. Thus, the probability bound's characterization of the resolvent matrix is experimentally verified by observing the qualitative behavior characterized by the bound, i.e., the sparse dependency and the symmetry of eigenspectrum. Consequently, though the boundedness and stability assumptions are different from the conventional regularity assumptions in the sense that the Dirac function is not a regular function, we still refer the assumptions as regularity assumptions because what is being characterized by the assumptions is simply certain qualitatively finiteness—though this issue does call for future works that investigate tighter bound in the sense that it could lead to controllable conditions that guarantee the plasticity phase.

Lastly, we present the proof sketch of theorem 2—the proof is given in supp. G B 3.

*Proof sketch of theorem 2.* As motivated in II D 3, we analyze the statistical dependence among Hessian entries (neuron assemblies of second-order perturbation of basis circuits) of DNNs with the class of loss function defined at definition 15, which reveals that the Hessian is a real symmetric random matrix with zero mena and sparse correlation among entries. This has been discussed in supp. B G 2.

Then, we undertake a non-parametric statistical analysis on the Hessian entries and show that when asm. 1 2 3 4 are satisfied, the eigenspectrum of Hessian can be analyzed with the MDE—this is a concentration of measure phenomenon introduced in supp. B H 1. The analysis is built on recent results on the random matrices, which we review in supp. F. To briefly summarize them, the results in Erdos *et al.* [55] is the major result that we build on, which show that if a random matrix satisfies asm. 2, asm. 3 and asm. 4, and furthermore the mean of the matrix is bounded, then, the resolvent of the matrix is probabilistically close to the solution to the MDE (cf. eq. (103)). Theorem 2.1 of Helton *et al.* [53] ensures the uniqueness of the solution to the MDE. The eigenspectrum of $\boldsymbol{H}$ can be obtained from the resolvent of matrix (cf. lemma 7). And theorem 2.5 of Alt *et al.* [56] ensures eigenspectrum to have support that is the union of close intervals with nonempty interior.

Equipped with the analytic technique, we prove in lemma 11 by assuming the zero mean (i.e., asm. 1), that the eigenspectrum of the matrix solved from the MDE studied is symmetric w.r.t. y-axis; that is, given any positive eigenvalue $\lambda$, $-\lambda$ is also an eigenvalue. The technical results are summarized as lemma 10 and lemma 11, and the proof is given in supp. G B 2. The idea is that though the eigenspectrum cannot be obtained in closed-form as the semi-circle law in the case of Wigner matrix, we still can analyze its qualitative behaviors through the MDE. □

## C. EXTENDED DISCUSSION: COMPLEXITY FROM ADAPTIVE-SYMMETRIES BREAKING

### A. From spin glasses to DNNs by increasing potential complexity

By this stage, it might be confusing that during training, a DNN both breaks symmetries and stays in a phase with stable symmetries. And thus to help appreciate this phase of DNNs, we further compare it with the spin glass phase of spin glasses, and show that this paradox could be resolved by putting spin glasses and DNNs in a spectrum of models with increasing *potential complexity*: it is the vastly increased potential complexity—which we mean by a hierarchically large DNNs with an abundant reservoir of circuits with circuit symmetries—enables a diachronic "frustration" process where circuit symmetries continually break, and makes the self-organizing of DNNs both a symmetry-breaking process and a phase with stable symmetries.

### 1. Symmetry breaking and spin glass phase of spin glasses

To being with, we describe the symmetry-breaking process of spin glasses, from the paramagnetic phase to the spin glass phase, in a similar way in which that of DNNs is described in supp. B G 8.

*a. Initial state.* Upon the decrease of temperature to a value below the critical temperature (i.e., quenching), the spins in the system would dissipate energy to the environment through kinetic collisions with one another. However, at the instant in the beginning, all spins are still of rotation and translation symmetry, and spin directions of all spins are disorganized, and thus magnetic moments of all spins cancel out with one another. As a result, at the coarse-grained/macroscopic level, no magnetization manifests by the spin system.

*b. Symmetry breaking.* As the temperature decreases, the spin system would take a phase transition into a *spin-glass* phase, where a symmetry known as *replica symmetry* is broken [123, Chp 3]; that is, the rotation symmetry and translation symmetry break, however, unevenly in different locations (i.e., different replicas) of the system. As a result, within a replica, translation symmetry holds, while across replicas, it breaks. And different regions/replicas of the system manifest different magnetic behaviors, and are characterized by different nonzero spin glass order parameters $q$, in which case, $q$ is indexed by replica indices in replica methods, e.g., $q_{\alpha\beta}$ where $\alpha \in [n], \beta \in [n]$. Overall, the system manifests magnetization.

*c. Metastable coarse-grained conservative symmetry at thermodynamic timescale.* After the symmetry breaking process after quenching, the system would start a frustration process, where utilizing the internal and external energy fluctuations, the spins in the system would be excited to cross small energy barriers to decrease the free energy. However, at the thermodynamic timescale, the system looks as if in equilibrium, only transits among symmetric states that conserve the free energy, and thus the coarse-grained effect of the system's symmetries manifests as magnetization. These states which are referred as *metastable* states of the system.

*d. Free energy minimized.* At a timescale (e.g., over days) that is orders of magnitude longer than the thermodynamic timescale, the alignment of spins resulted from the quenching gradually disappears, the magnetization (i.e., $q_{\alpha\beta}$) would gradually decay from nonzero to (almost) zero, and the system would reach a local minimum (with zero magnetization, or some fraction of the original $q_{\alpha\beta}$) with high energy barriers, and macroscopically manifests as the eventual (almost) de-magnetization.

*e. Similarities between the frustration process of spin glasses and training process of DNNs.* As suggested by the organization and naming of previous paragraph titles, the frustration process of spin glasses strikingly resembles the training process of DNNs.

- First, in spin glasses, spins of translation symmetry within replicas and of broken translation symmetry across replicas coexist, while in DNNs, basis circuits of intact circuit symmetries and of broken symmetries coexist;
- Second, in spin glasses, the translation symmetries are broken by energy perturbations, while in DNNs, the circuit symmetries are broken by informational perturbations;
- Third, in spin glasses, the spin glass order parameter characterizes the coarse-grained effect of translation symmetries in response to energy fluctuations (which could be obtained by taking derivative of free energy against spin variables, cf. supp. D C), and converges towards almost zero as the frustration process progresses, while the plasticity order parameter characterizes the coarse-grained effect of circuit symmetries in response to information perturbations (recall that the two parameters are symbolically equivalent, cf. supp. B F 1), and converges towards almost zero as the training process progresses.
- Lastly, both these two systems undertake a temporally extended self-organizing process.

However, despite the similarity, fundamental difference exist between these two systems. The frustration of spin glasses is caused by spins' competing configurations that are of different symmetries, but also are of almost the same free energy. And thus the replicas in the system would choose one configurations, or another in a statistically random way, and the system hops from a local minimum of a particular configuration of symmetries to another given the energy fluctuations, and slowly drifts to the lowest possible free energy. In contrast, the circuit symmetries of DNNs do not compete with one another, at least not in the way of symmetries of spin glasses, but break cooperatively to reduce information perturbations of novel examples.

### 2. Spin glasses to DNNs by increasing potential complexity

Yet, this is not the end of the story; the connection between the two systems reveals not by direct comparison, but by putting them in a spectrum of phenomenological models that are of increasing information capacity and are perceived of increasing complexity (perhaps because more information is encoded after self-organization finishes)—therefore, we also have use information capacity interchangeably with potential complexity in this work.

To begin with, increasingly complex competing symmetries similar to the ones in spin glasses have been speculated to be the foundation of evolution. The pioneer of complex science, P. Anderson, prefigured in the seminal essay *More is Different* [3, p. 396]: "... at some point we harre to stop talking about decreasing symmetry and start calling it increasing complication ..." in "... functional structure in a teleological sense ..."—teleology refers to goal-directed behaviors controlled by feedback [8], and in modern terminology, complication is referred as complexity. In the paper, DNA molecules are referred as systems that are more complex than relatively well understood systems such as glasses. And for such more complex systems, a frustration phenomenon of DNA molecules at the

*evolutionary timescale* has been speculated as the physical foundations of evolution [50]. As in a frustrated system, the differences in free energies of DNA molecules with different nucleotide sequences are orders of magnitude smaller than the total energy of covalent bonds in these molecules. These different metastable states separated by these low energy barriers among DNA molecules are gnomes of different organisms. The drifting among the metastable states creates a population of organisms with diverse survival hypotheses, and the competition among these hypotheses manifests as evolution by natural selection.

Correspondingly, a series of phenomenological models with increasing complex design in evolutionary biology qualitatively reproduces the phenomena in evolutionary history. For example, the NK model [295] of evolution, which is equivalent [7, p. 257] to a model of spin glass known as Sherrington–Kirkpatrick model [123, p. 14], manifests the *ruggedness* (which is another name for frustration) of the fitness landscape where genotypes tend to stay in a locally maximal fitness for some time before moving out of it; the NKCS model in evolution [42], which uses many spin glass models that each models a species and overall model an ecosystem, manifest the *punctuated equilibrium* phenomenon (a sudden burst of new species after a long period where few new species emerge) observed in archaeological records.

When a system is very large and is adjacent to a large number of almost symmetric states with similar free energy, we might speculate that statistically there is no preference to transit to any of the adjacent states as a result of fluctuations, and consequently, the system poses in a state that would be of equal probability to transit to a large number of adjacent possible states, and the evolution could be understood as natural selection on the random talk on these adjacent possible states. That is, an adaptive symmetry whose breaking is selected by the feedback signals from the environment. Unlike the symmetries in physics, which formalizes a conservative law that conserves the free energy of different states related by certain transformations and thus characterizes the invariant of free energy, the adaptive symmetry is the conservation of change of free energy; or in other words, *the invariant of change that emerges as a result of the increased sophistication and amount of symmetries*.

The plasticity of nervous systems has been considered as a major innovation in the evolutionary history [296] that improves over the gnome-based exploration of alternative hypotheses by differential mortality, and is able to explore alternative hypotheses within the lifespan of individuals [46]. From this perspective, if we trace the history of ideas backward, DNNs are also developed from the spin glass model. The Hopfield Network [123, p. 133] models the memory mechanism of nervous systems with the spin glass model in physics. Hopfield Network inspires the Boltzmann Machine [297], which could be understood as a system that implements a plastic way of encoding information compared with the NK model: the genes (i.e., the spin in a spin glass) in the NK model could only change its value through random mutation to increase the fitness and can only interact with neighboring genes through fixed coupling constants—the competing configurations of different symmetries but almost the same free energy—while the neurons in DNNs activate, or deactivate in response to the incoming signals, and the coupling parameters (i.e., weights) among neurons could be change in a hierarchically cooperative way to minimize uncertainty. And Restricted Boltzmann Machine (RBM) [298] was developed from the Boltzmann Machine by restricting neurons to only have inter-layer connections. Hierarchically stacked RBMs compose Deep Belief Network (DBN) [161], which showed that DNNs are powerful and DNNs' early poor performance might result from improper technical design. Further studies showed that even without the pre-training by DBN, DNNs with ReLU activation function can reach their best performance [95]. Then, supervised DNNs became the Zeitgeist, and set off the Deep Learning revolution [10]. And the Umwelt in this work is developed by synthesizing DBN and supervised DNNs.

Therefore, a DNN is a phenomenological model of nervous systems whose hierarchically large size and plastic hierarchical coupling among units—formalized as hierarchically large DNNs with abundance of reservoir of circuits with circuit symmetries in this work—enable the system to indefinitely process informational perturbations, and to encode information up to the maximal complexity possible. In other words, compared with spin glasses, the vastly increasing potential complexity enables a diachronic "frustration" process where circuit symmetries continually break. Large potential complexity transforms the metastability of spin glasses to the stability of DNNs, and makes the self-organizing of DNNs both a symmetry-breaking process and a phase with stable symmetries.

### B. Extended criticality of DNNs

Because the self-organizing of DNNs is a continual symmetry-breaking process, it might also be confusing that criticality is not mentioned in this work: macroscopic symmetry breaking needs the microscopic fluctuations to synchronize at a scale-free/macroscopic scale, and this phenomenon is referred as *criticality* in physics. As in the identification of the plasticity phase of DNNs, where the concept shifts from symmetry of invariants to symmetry of variants, the criticality of the symmetry breaking needs a similar conceptual shift. In the extended circuit-symmetries breaking process of a DNN, the DNN stays in an *extended critical regime* where a power-law criticality exists between microscopic change of weights and the macroscopic reduction of uncertainty, i.e., the plasticity order parameter. In this subsection, we clarify the concept of criticality of DNNs, by again putting DNNs in the spectrum of models of increasing potential complexity from physics to biology.

#### *1. From criticality in physics to extended criticality in biology*

To begin with, we briefly review criticality in physics. Phase transitions of a statistical-physical system occur when microscopic symmetry breaking is synchronized macroscopically throughout the system. The synchronization is possible be-

cause at the critical control parameter (e.g., temperature), the correlation among units is scale-free (macroscopic, or more precisely, of a power-law); microscopically, the symmetry breaking of a unit (e.g., the flipping of a spin in the spin glass) would cause a domino effect over the system. And because the process happens at thermodynamic timescale, it occurs so fast that the process is mathematically formalized as a singularity.

However, unlike the homogeneity of a physical system, the heterogeneity of biotic systems causes that such domino effects of symmetry breaking of units could only happen within subsets of the system, and the self-organizing process shifts from a singular process to a symmetry-breaking process extended over space and time. Recall that we have discussed in supp. C A that the symmetry-breaking of spin glasses happens over a timescale much higher than the thermodynamic timescale because the competing configurations of symmetries are of almost the same free energy. Furthermore, the number of symmetric states of a biotic systems is orders of magnitude larger than the symmetric states of physical systems, and the evolution process continually breaks symmetries. Thus, the singular process of symmetry-breaking in physical becomes an extended process in biotic systems where adaptive symmetries are continually being broken. This phenomenon is referred as *extended criticality* [36, 37] in theoretical biology. And this conceptual shift is reviewed in more details in supp. D F.

### 2. *Edge of chaos and extended criticality of DNNs*

Further recall that in supp. C A, we have discussed that DNNs could be positioned in a spectrum phenomenological models of increasing potential complexity, where the phenomenological models of DNA molecules are in the middle of the spectrum. Therefore, the criticality of DNNs could also be understood through the concept of extended criticality, which we mostly discuss informally in the following.

The circuit stability assumption made at definition 25 actually is a rather simplistic characterization of a phenomenon known as computation on the *edge of chaos* [42, 147, 148]. As a straightforward consequence of lemma 5, the square norm of gradient, i.e., the plasticity order parameter, is the sum of the square norm of individual gradient entry, and is given as

$$||\nabla_\theta R_m||_2^2 \leq O(Ln^2 c^{2(L-1)}), \tag{106}$$

where $L$ and $n$ are the depth and width of a DNN, respectively, $c$ is a constant that depends on the constants in the circuit stability assumption given at definition 25, and we have omitted an decay exponentially against depth. Qualitatively, eq. (106) characterizes a phenomenon known as computation on the edge of chaos, as explained in the following.

1. As discussed in supp. B F, the self-organization of DNNs is an "order from fluctuations" phenomenon where the system utilizes weight perturbations to decrease the errors computed from feedback signals. For the current practice of DNNs and well-designed loss functions, the feedback signals (i.e., losses) is at the order of magnitude $\Theta(1)$.

2. Thus, the perturbations induced by weights need to be at the order of magnitude of the signals: otherwise, for perturbations whose order of magnitude is larger than that of the feedback signals, the information encoded in the signals would be drown in the noise of the perturbations—this is referred as the **chaotic** regime in Kauffman and Johnsen [42]; for perturbations whose order of magnitude is smaller than that of the feedback signals, the system-wide change induced by the weight perturbations would be inconsequential to the signals, and thus be ineffective to decrease the errors—this is referred as the **frozen** regime in Kauffman and Johnsen [42].

3. The phenomenon, that the perturbations induced by weights are of the same order of magnitude with the feedback signals, could be mathematically stated as a manifold exists inside an ambient state space where power-law criticality exists; and generally such a phenomenon is referred as **edge of chaos**. Such a phenomenon is characterized simplistically by eq. (106), which characterizes the collective behaviors of neurons as follows. Recall that $c$ in eq. (106) comes from the circuit stability assumption given at definition 25, and characterizes the largest value of individual weight or neuron activation; therefore, eq. (106) characterize the worst-case synchronized/collective perturbation induced by all weights and neurons in the system. Underlying such a uniform worst-case characterization of microscopic weight changes, a vast heterogeneity actually exists: each weight is a degree of freedom, yet they cooperate to adapt to the direction in the weight space that maximizes the uncertainty reduction in the current iteration of the feedback-control loop.

4. Meanwhile, and unlike statistical-physical systems, where the number of units are so large that they could be mathematically treated as infinite, for DNNs, even though the number of parameter is large (i.e., $Ln$ weights), the loss (i.e., feedback signals) and the order parameter (i.e., eq. (106)) is carefully maintained at roughly the same order of magnitude by techniques such as step-size tuning, initialization schemes, and online normalization, such that the exponential effect of $c^{2(L-1)}$ and the accumulated effect of perturbations induced by $Ln^2$ weights are counteracted by step size, and a computation-at-the-edge-of-chaos phenomenon manifests—we would expand on the details along with empirical results next in supp. C B 3.

5. Consequently, eq. (106) is a power-law when DNNs are properly tuned; that is, a power-law criticality. This is also experimentally observed in fig. 4b, where we could see that statistically, the order parameter is roughly a faction of the loss (i.e., the feedback signals), and approaches to zero as the loss itself approaches to zero.

By self-organizing on the edge of chaos, the system encodes the information in the feedback signals by selectively keeping the weight fluctuations that decrease the errors computed through feedback signals. And this manifold of edge of chaos is an extended, instead of singular, regimen of the state space where power-law criticality exists, and thus an **extended criticality**.

### 3. *Experimental support for the extended criticality and edge-of-chaos phenomenon of DNNs*

We provide further empirical results on the extended criticality phenomena of DNNs. In the following, we shall show that the practice of DNN training could be interpreted as tuning the system to be in the extended critical regimen; that is, the risk of DNNs could only be decreased when the order parameter is roughly at a fraction of the order of magnitude of the signals/labels.

More specifically, during the execution of the feedback-control loop (defined in supp. B D 5), $c$ and the step size $\eta$ are tuned to keep the plasticity order parameter at a fraction of the order magnitude of the risk—here $c$ strictly speaking denotes the parameter that parameterizes the variance of the Gaussian distribution (i.e., $\mathcal{N}(0, c/\sqrt{n})$) that initializes the weights[12]. We demonstrate the phenomenon through the the conventional varnishing ($c = 1/2$), stable ($c = 1$), and exploded ($c = 2$) gradient initialization schemes respectively—the latter two corresponds to well known Xavier [19] and MSRA [12] initialization schemes, respectively. The experiment settings are the same with the setting introduced in section I A 3, except that the initialization schemes are different and the momentum is not used in the gradient descent training.

*a. A DNN in the chaotic regimen.* First, we demonstrate the behaviors of DNNs in the chaotic regime through the initialization scheme that induces exploding gradients. From fig. 11a, we could see that when $c = 2$, the order parameter is of value $\sim 10^4$. According to eq. (106), the magnitude of (the expected squared norm of) an entry of the gradient is $\sim 10^{-3}$ (recall that the net has $\sim 10^7$ parameters). Further note that the variance of weight are $\sim c/10^{-3}$. If we do not carefully select $\eta$, and by default, a typical choice of $\eta$ could be 0.1, we would observe a chaotic phenomenon in fig. 11b: in the bottom panel, the risk of the initialization scheme with $c = 2$ rapidly grows to be larger than $10^{16}$ in two steps, and diverges afterwards. The phenomenon makes sense because the DNN is supposed to learn regularities in the dataset, and in this case, the system overreacts in the sense it adapts to a very noisy signal prematurely: in this case, the perturbations induced by a single batch is $\sim 10^{-3}$, and is at the same magnitude of the weights; as a result, the system falls in a positive reinforcing loop that amplifies the weights at each iteration, and the risk grows exponentially.

The chaotic behaviors could be mitigated by scaling down the order parameter by decreasing the step size $\eta$: at each gradient descent step, we choose $\eta$ as $0.01/||\nabla_{\boldsymbol{\theta}} R_m||_2^2$, and the training proceeds as shown in the top panel in fig. 11b, where risk (the $c = 2$ line) gradually decreases from 1 to 0.5 at the first 200 steps. In this case, the square norm of a gradient entry is $\sim 10^{-7}$ ($\eta$ at each step is shown as the $c = 2$ line in fig. 11c). As a result, each gradient update only infinitesimally changes the weights, and given enough steps—for example, the experiments shown in section II use $300 \times 157 =\sim 5 \times 10^4$ steps—the risk could be minimized to zero.

*b. A DNN in the frozen regimen.* Second, we demonstrate the behaviors of DNNs in the frozen regime through the initialization scheme that induces varnishing gradients. From fig. 11a, we could see that when $c = 1/2$, the order parameter is of value $\sim 10^{-8}$, and thus the squared norm of a gradient entry is $\sim 10^{-15}$, which would be too small compared with the magnitude of the weights ($\sim c/10^{-3}$). A naive $\eta \sim 0.1$ could not meaningfully affect the risk. And furthermore, the results in supp. B G inform us this is not because of the system is trapped in local minima: from supp. B G, we know that eigenspectrum is symmetric, and the change in $c$ alone simply induces a scaling of the eigenspectrum, because DNNs with ReLU activation function are piece-wise linear. More specifically, multiplying $c$ by a factor $d$ would scale all Hessian eigenvalues exponentially by $d^{(L-2)/2}$ [13]. The symmetry of eigenspectrum in the varnishing regimen is also experimentally observed in fig. 12. As a result, the training would not be trapped in local minima solely because of different initialization schemes discussed here.

Even with the dynamical step size scheme that works with the chaotic regime (the step sizes at each step is given as the $c = 1/2$ line in the bottom panel of fig. 11c), as shown in bottom panel in fig. 11b, the risk does not change much at the beginning for 20 steps, and increases exponentially afterwards. This is because the order parameter is only a first-order approximation of the coarse-grained effect of the perturbation of weights on the risk, and an exponentially large $\eta$ invalidates the local linear approximation: the higher order perturbations would be nontrivial—for example, the second order perturbations would be enlarged by $\eta^2$. As a result, the change of risk at each gradient descent is influenced by the higher order stochastic fluctuations—we plot the difference between the expected/approximated risk and the actual risk after a gradient descent step in fig. 13b. From fig. 13b we can see that at the initially 20 steps, the over-amplification does not change the risk noticeably, because the higher order fluctuations are small. However, stochastically, a large fluctuation eventually occurs at around 20th step, where the difference between the expected

[12] This $c$ and the $c$ discussed in supp. C B 2 are conceptually similar: because in previous theoretical characterization, the value of $c$ is a constant in asymptotic bounds, and thus it is understood at the granularity of orders of magnitude instead of precise values; and both these two $c$ characterizes the magnitude of order parameters. Therefore, in this non-rigorous empirical discussion, we regard the two concepts as the same, and reuse the symbol in this subsection.

[13] Formally, let $\boldsymbol{H}$ denote the Hessian of a DNN whose parameters are initialized with $\mathcal{N}(0, c/\sqrt{n})$. And let $\boldsymbol{H}(d)$ denote another Hessian of a DNN whose parameters are initialized with $\mathcal{N}(0, cd/\sqrt{n})$. Then, we have the block matrices of $\boldsymbol{H}_(d)$ given as

$$\begin{aligned}\boldsymbol{H}(d)_{pq} = {} & \mathcal{L}'(T\boldsymbol{x}, y)\mathrm{dg}(\boldsymbol{h}_q)\overrightarrow{\prod}_{k=q+1}^{L-1}(\sqrt{d}\boldsymbol{W}_k\mathrm{dg}(\boldsymbol{h}_k))\sqrt{d}\boldsymbol{\alpha} \\ & \otimes \overleftarrow{\prod}_{j=p+1}^{q-1}(\mathrm{dg}(\boldsymbol{h}_j)\sqrt{d}\boldsymbol{W}_j^T)\mathrm{dg}(\boldsymbol{h}_p) \\ & \otimes \boldsymbol{x}^T\overrightarrow{\prod}_{i=1}^{p-1}(\sqrt{d}\boldsymbol{W}_i\mathrm{dg}(\boldsymbol{h}_i)),\end{aligned}$$

where the neuronal gates and weight matrices are those of $\boldsymbol{H}$. Factoring the $\sqrt{d}$ out, we have

$$\boldsymbol{H}(d)_{pq} = d^{(L-2)/2}\boldsymbol{H}_{pq}.$$

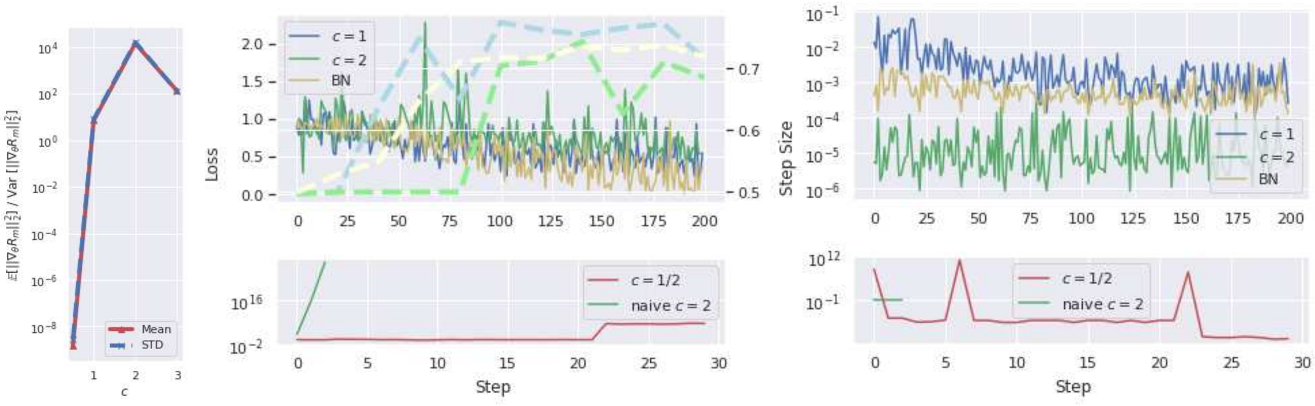


(a) (b) (c)

FIG. 11. Empirical study of DNNs with different initialization schemes. **(a)** We initialize the weights of a DNN with $c = 1/2, 1, 2$ and compute the plasticity order parameter and its standard deviations (STDs). The last datum at $c = 3$ is the datum for the network with Batch Normalization. Note that the two lines are almost identical, and the standard deviation line overlays on the mean line. We do not plot the STDs as error bars since we have used a logarithmic scale, and error bars in this case are not intuitive. **(b)** Top panel: the training loss curve for 200 steps of NNs whose risk can be minimized. The dashed lines are the test accuracy curves, and the right y-axis shows the accuracy. Bottom panel: the training loss curves for 2 steps of $c = 2$ case with constant step size 0.1, and for 30 steps of $c = 1/2$ case with dynamic step sizes, respectively. **(c)** The corresponding step size curves of fig. 11b during training.

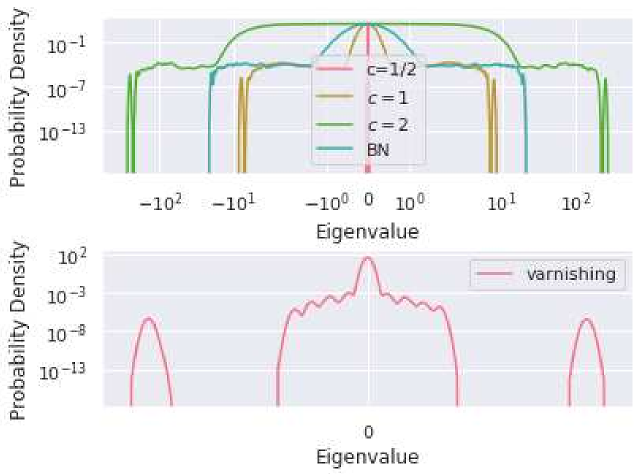


FIG. 12. The eigenspectrum of a VGG net with the same configuration as that in fig. 8 but with Batch Normalization removed and the initialization scheme changed. The bottom panel is a zoom-in of the eigenspectrum of the network in the varnishing regime; it is plotted separately because it has degenerated into a line in the panel above.

and actual risk is $\sim 10^5$, and the weights would be changed to that direction. As a result, the risk would increase exponentially because a single batch is not the dataset—over-adaptation in a single batch does not perform well in the whole dataset—and outside the local region, the change induced by the large weight change is unknown and probably leads to pathological behaviors. This phenomenon could not be mitigated in first-order algorithms.

*c. A DNN in the extended critical regimen.* Lastly, to avoid the pesky tuning of the step size $\eta$ in the chaotic regime and the pathology resulting from higher order stochastic fluctuations in the frozen regime, an approach is to tune $c$ such that the order parameter is roughly of the order of magnitude of the risk. This corresponds to the $c = 1$ initialization scheme that induces stable gradients. In this case, the risk and step size dynamics are shown as the $c = 1$ in fig. 11b and fig. 11c, respectively. From fig. 11c, we could see that $\eta \sim 10^{-2}$ at the first 200 steps, which is close to the constant step size scheme typically used in DNN training, and from fig. 11b, we could see the risk decreases gradually. Meanwhile, from fig. 13a, we can see that the first-order approximation of the risk also has manageable errors.

A logic extension of the previous approach is to normalize the scale of the circuits during training, and an implementation is Batch Normalization (BN) [214]—this is also the technique we use in experiments: it is equivalent to multiplying a weight matrix $\boldsymbol{W}_l$ with a diagonal matrix $\boldsymbol{\Sigma}_l$, i.e., $\boldsymbol{x}_{l-1}^T \boldsymbol{W}_l \boldsymbol{\Sigma}_l$, where $1/\Sigma_{ii}^l$ is the standard deviations of $\boldsymbol{x}_{l-1}^T \boldsymbol{W}_l$; at initialization, it amounts to initialize $w_{ij}^l, i, j \in [n]$ with $\mathcal{N}(0, \Sigma_{jj}^l c/n)$, respectively. As a result, a DNN with BN has gradients as follows (the calculation of gradient can be found in supp. G B 1):

$$
\begin{aligned}
&\partial l(T\boldsymbol{x}, y)/\partial \mathrm{vec}\boldsymbol{W}_p \\
=&\mathcal{L}'(T\boldsymbol{x}, y)\boldsymbol{\alpha}^T \overleftarrow{\prod}_{j=p+1}^{L-1}(\mathrm{dg}(\boldsymbol{h}_j)\boldsymbol{\Sigma}_j \boldsymbol{W}_j^T)\mathrm{dg}(\boldsymbol{h}_p) \\
&\otimes \boldsymbol{x}^T \overrightarrow{\prod}_{i=1}^{p-1}(\boldsymbol{W}_i \boldsymbol{\Sigma}_i \mathrm{dg}(\boldsymbol{h}_i)),
\end{aligned}
$$

where $\overleftarrow{\prod}_{j=p+1}^{L-1}(\mathrm{dg}(\boldsymbol{h}_j)\boldsymbol{\Sigma}_j \boldsymbol{W}_j^T)$ denotes $\mathrm{dg}(\boldsymbol{h}_{L-1})\boldsymbol{\Sigma}_{L-1}\boldsymbol{W}_{L-1}^T \ldots \mathrm{dg}(\boldsymbol{h}_{p+1})\boldsymbol{\Sigma}_{p+1}\boldsymbol{W}_{p+1}$. It prevents explosion by maintaining the rightmost term to have unit variance in each dimension, and alleviate the exponential behavior of the order parameter. By applying BN to the $c = 2$ case previously, the order parameter is scaled down from

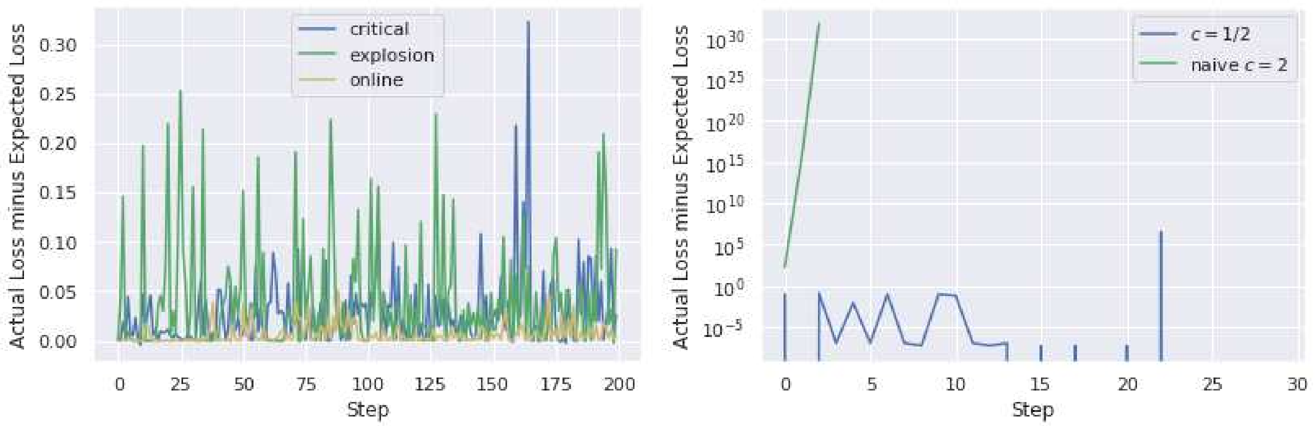


(a) (b)

FIG. 13. The difference between expected loss esimated by first-order approximation, and the actual loss computed after gradient update, under various regimens. **(a)** The difference of losses in regimens that can be successfully optimized. "explosion" denotes the regimen where $c = 2$, and "critical" denotes the regime where $c = 1$. "online" denotes the regimen where batch normalization is used. **(b)** The difference of losses in regimens that cannot be optimized.

$\sim 10^4$ to $\sim 10^2$, and it enables DNNs to be trained in $\sim 100$ times larger step sizes, as shown in the yellow lines in fig. 11b and fig. 11c.

### C. Extended phase transition of DNNs

Therefore, not only the self-organizing of DNNs is both a symmetry-breaking process and a phase, it is also both a phase and a phase transition. This characterization is a straightforward extension of the extended criticality discussed in supp. C B: a sufficient proportion of the the large number of circuit symmetries in DNNs need to break before the stability of the macroscopic/assembly adaptive symmetries of DNNs could break; and thus the phase transition of DNNs also shifts from singular phase transitions process (in physics) to an *extended phase transition* process where circuit symmetries are continually being broken in extended critical states.

We briefly discuss the extended phase transition in this subsection, mostly aiming to clarify confusions and corroborate the plasticity phase. First, in supp. C C 1, we discuss a phase of DNNs with a toy DNN with homogeneous neurons where a paucity of adaptive symmetries exist and the DNN could easily be unable to decrease the errors of novel examples, which we refer as the *frustration* phase—note that the frustration here does not necessarily mean the system is trapped in local minima that are not global minima, but simply be of nonzero risk, and this denotation of frustration phase is more because the phase is understudied than it is carefully designed this way; and then in supp. C C 2, we discuss the extended phase transition between the frustration phase and the plasticity phase.

#### *1. Frustration phase of DNNs*

Although the increase of potential complexity stabilizes the adaptive symmetries of DNNs, as the complexity of the dataset increases while the reservoir of circuit symmetry in the DNN does not increase, eventually, the circuit symmetries could be completely broken, and the stable symmetries described in supp. B G 8 could disappear. The plasticity phase where circuit symmetry is stable is the focus of this work, yet to help appreciate the plasticity phase, in this subsection, we preliminarily discuss the rest of phase space: we describe a toy case of a phase, which we refer as the **frustration phase** where a paucity of adaptive symmetries exist, to contrast it with the plasticity phase.

Recall that the circuit symmetry is a heterogeneous symmetry that characterizes the adaptive symmetry and diversity of basis circuits. Thus, to construct a case where a paucity of adaptive symmetries exist, we design a DNN with homogeneous neurons. In this toy case, as a result of lacking adaptive symmetries, the DNN could only decrease the error of examples from a specific half-subspace of the instance space, and would frustrate easily in response to examples from other regions.

The DNN with homogeneous neurons is given as follows. During training, let $T$ be a DNN where all the weight matrices $\{\boldsymbol{W}_i\}_{i\in[L-1]}$ are constrained to the space of rank 1 matrix $\boldsymbol{u}\boldsymbol{u}^T$, where $\boldsymbol{u} \in \mathbb{R}^n, n \in \mathbb{N}^+, \boldsymbol{u} > 0, \boldsymbol{u}^T\boldsymbol{u} = 1$, and the last layer weight is a vector $\boldsymbol{\alpha}$ given as $\boldsymbol{u}$. The DNN $T$ has a simple behavior,

$$T\boldsymbol{x} = \begin{cases} x^T \overrightarrow{\Pi}_{i=1}^{L-1}(\boldsymbol{u}\boldsymbol{u}^T)\boldsymbol{u} = x^T\boldsymbol{u} & \boldsymbol{x}^T\boldsymbol{u} > 0 \\ 0 & \boldsymbol{x}^T\boldsymbol{u} \leq 0 \end{cases}, \tag{107}$$

because when $\boldsymbol{x}^T\boldsymbol{u} \neq 0$, then all neuronal gates $\{\boldsymbol{h}_i\}_{i=1,\dots,L-1}$ are activated (i.e., are of value 1), and thus $T$ behaves as a linear DNN; otherwise, all gates are deactivated, and $T$ outputs zero.

Suppose that the DNN is trained with hinge loss, then we can simplify the block Hessian of $T$ given at eq. (101) as

$$\boldsymbol{H}_{pq} = \begin{cases} -\boldsymbol{x}^T\boldsymbol{u}\mathbf{1}_{y^T\boldsymbol{x}<1}\boldsymbol{u}^T \otimes \boldsymbol{u}\boldsymbol{u}^T \otimes \boldsymbol{u} & \boldsymbol{x}^T\boldsymbol{u} > 0 \\ 0 & \boldsymbol{x}^T\boldsymbol{u} \leq 0 \end{cases},$$

Notice that the block matrix does not depend on $p,q$; denote it as $\boldsymbol{H}_{\text{homo}}$ and thus the Hessian matrix of $T$ is of the following form

$$\begin{bmatrix} \mathbf{0} & \boldsymbol{H}_{\text{homo}} & \cdots & \boldsymbol{H}_{\text{homo}} \\ \boldsymbol{H}_{\text{homo}} & \mathbf{0} & \cdots & \boldsymbol{H}_{\text{homo}} \\ \vdots & & \ddots & \vdots \\ \boldsymbol{H}_{\text{homo}} & \boldsymbol{H}_{\text{homo}} & \cdots & \mathbf{0} \end{bmatrix}, \tag{108}$$

where with an abuse of notation, we denote the block Hessian matrix between weights of layer from 1 to $L-1$ and the weight of the last layer $\boldsymbol{\alpha}$ as $\boldsymbol{H}_{\text{homo}}$ as well (and it has not been explicitly calculated because it would not be used later and we only aim to illustrate the homogeneity of Hessian here).

The Hessian given at eq. (108) is a matrix with homogeneous entries with a large coupling set size. More specifically, first, from eq. (108), we can see that the Hessian consists of identical matrix $\boldsymbol{H}_{\text{homo}}$; furthermore, for each $\boldsymbol{H}_{\text{homo}}$, when it does not degenerate into a zero matrix, its entries are constrained within the quartic functions of elements of $\boldsymbol{u}$, i.e., $u_iu_ju_ku_l, i,j,k,l \in [n]$. Consequently, in each $\boldsymbol{H}_{\text{homo}}$, given an entry $u_{i'}u_{j'}u_{k'}u_{l'}, i',j',k',l' \in [n]$, it correlates with all entries of the form $u_{i'}u_ju_ku_l, j,k,l \in [n]$, $u_iu_{j'}u_ku_l, i,k,l \in [n]$, and so on. Thus, even if we only count the correlation of the form $u_{i'}u_ju_ku_l, j,k,l \in [n]$, it at least correlates with $n^3 \cdot (L-1)^2$ entries among overall $n^4 \cdot L^2$ entries, where the minus 1 in $(L-1)^2$ is to exclude the zero block matrices at the diagonal. To compare with the threshold $\sqrt{N}$ in the diversity assumption (where $N \times N$ is the dimension of the Hessian), in this case $\sqrt{N} = n\sqrt{L}$. Thus, for the homogeneous DNNs, each entry of $\boldsymbol{H}_{\text{homo}}$ at least correlates with $o(N^{\frac{3}{2}}L^{\frac{1}{2}})$ number of entries.

The Hessian looks complicated, however, as a result of the homogeneity of the weights, despite the large number of weights, the DNN degenerates into a linear classifier as follows. Compose eq. (107) with the hinge loss, we have

$$\mathscr{L}(T\boldsymbol{x},y) = \begin{cases} \max\{0, 1-y(x^T\boldsymbol{u})\} & \boldsymbol{x}^T\boldsymbol{u} > 0 \\ 1 & \boldsymbol{x}^T\boldsymbol{u} \leq 0 \end{cases}. \tag{109}$$

In this case, the DNN has degenerated into a piece-wise linear classifier, and only responds to the examples with in the one-dimensional subspace $\boldsymbol{u}$. And it is well known that a linear classifier cannot solve the XOR problem [299].

Therefore, when the homogeneous DNN trained with eq. (109) converges, the plasticity order parameter would be zero, and the DNN would frustrate in nonzero risk minima that perform poorly on examples that outside the half-subspace of $\boldsymbol{u}$.

To conclude, we could see that despite being symbolically the same (but the symbols bind to different values), the homogeneity of weights of DNNs results in a completely different macroscopic behaviors, as broken down in the following. To begin with, suppose that $\boldsymbol{u}$ is randomly initialized from a random variable of symmetric law, zero mean and unit variance. Then, the optimization of eq. (109) is also a symmetry-breaking process: at initialization, $x^T\boldsymbol{u}$ would be realized around zero, and in response to the feedback signal $y$, it could be either decreased or increased until frustration. However, microscopically, all the weights $w^l_{i_{l-1}i_l}$ in of the homogeneous DNN are constrained in the set $\{u_i\}_{i\in[n]}$. As a result, no concentration-of-measure phenomenon as that of the plasticity phase exists, and the coarse-grained behavior of the homogeneous neurons degenerates into a piece-wise linear classifier that can only decrease the errors of examples in the a specific subspace, and does not respond to examples from other subspaces. Consequently, if the DNN encounters novel examples come from the other subspaces, it would frustrate in minima with nonzero risk. In contrast, DNNs in the plasticity phase discussed in supp. B G could be understood to contain a large number of half-subspaces—recall that a DNN with ReLU activation function is piece-wise linear—that each could process many examples.

### 2. *Extended phase transitions between plasticty phase and frustraion phase*

The difference in diversity control parameter between the heterogeneous DNN discussed throughout this work and the homogeneous DNN in supp. C C 1 seems to suggest that as the diversity of neural circuits decreases, a DNN might transit from the plasticity phase to the frustration phase. We discuss the transition speculatively in this subsection. The discussion is to clarify the concept that the extended symmetry-breaking should also be understood as an extended phase transition, not to give any definite conclusion on the extended phase transition, which is out of scope of this work.

To begin with, we briefly summarized the two phases. Recall that in section II D 3, we have explained that to characterize the heterogeneity in DNNs, we make a trade-off between analyticality and verisimilitude, and the theoretical characterization characterizes extreme behaviors that bound statistical behaviors of the system. These two phases are two extreme macroscopic behaviors of DNNs identified by this method: in the plasticity phase, a DNN could always decrease risk, or in the frustration phase, a DNN would easily frustrate. The plasticity phase is a practically important phase in the sense that it suggests an explanation of the optimization power of DNNs, and might potentiate scientific methods to minimize risks (e.g. optimizable conditions that ensure DNNs to stay in the plasticity phase), while the frustration phase is a toy example to demonstrate that when the control parameters change, a DNN would not necessarily stay in the plasticity phase.

The difference in diversity control parameter between the heterogeneous DNN discussed in this work and the homogeneous DNN in supp. C C 1 seems to suggest that as the diversity of neural circuits decreases (perhaps as a result of a large amount of circuit-symmetries breaking), a DNN might transit from the plasticity phase to the frustration phase. We elaborate this speculation in the following.

1. First, we review the results so far. In supp. B G 8, we show that theoretically if the diversity control parameter of a DNN is smaller than $\sqrt{N}$ (where $N$ is the number of parameters), the DNN is in the plasticity phase; and the theoretical characterization is qualitatively validated through experiments from supp. B G 5–B G 7. These results characterize benign pathways of DNNs that suggests an explanation of the optimization power of DNNs. The $\sqrt{N}$ threshold given in asm. 2 is a worst-case estimation of the diversity of circuit symmetries in DNNs, and frustration should occur at a threshold higher than $\sqrt{N}$. Meanwhile, Supplement C C 1 shows that when the diversity control parameter is high, in that case larger than $\sqrt{N}^{3/2}L^{1/2}$ (where $L$ is the number of layers), a specific DNN is equivalent to a linear classifier and could easily frustrate.

2. The plasticity order parameter of DNNs is nonzero in the plasticity phase, when novel examples with nonzero loss still exist. Meanwhile, in the toy network given in supp. C C 1, the order parameter would be stably zero at the end of the training with nonzero risk.

3. From these results, we might speculate that the gradual change of control parameters might lead to the transition between these two phases; more concretely, as the symmetry breaking of a DNN continues, if the training dataset exceeds the upper bound of the information that could be encoded by the broken circuit symmetry of the DNN, we might expect the system would frustrate at nonzero risks during training.

4. Some empirical observations [21, 300, 301] have shown that by increasing the complexity of the dataset, or decreasing the size of the DNN (which correspond to the decrease of circuit symmetries, relative to the dataset), the DNN would manifest phase-transition like behaviors agreeing with the extended phase-transition speculation that transit from being able to minimize the risk to zero to being unable to do so. Some further discussion on the empirical observations is given in supp. A D 6, where we discuss the related works on phases of DNNs.

Overall, the study of such a speculation would be interesting future works.

### D. Complexity from adaptive-symmetries breaking

This section has discussed many concurrences of previously orthogonal phenomena, and such paradoxical concurrence of previously orthogonal properties of a system/object has repeatedly happened in the history of physics, e.g., the wave-particle duality in quantum physics, and the mass-energy equivalence in special relativity. The resolving of such paradoxes is referred as the paradigm shift by Thomas S. Kuhn [33], where anomalies in the previous paradigm are reconciled by the new paradigm. Compared with most systems in physics, in addition to energy and matter, biotic systems are informational systems in a fundamental way [49]; and as physical forces could be unified by pushing the dimensionality higher, in this new dimension of information, a new category referred as invariance of change emerges upon the invariance of energy, and is formalized through a new category of symmetries (i.e., adaptive symmetries) in this work. From this perspective, the fact that, the self-organizing process of DNNs is both a phase transition and a phase, might not be so paradoxical: after all, “nothing in biology makes sense except in the light of evolution” [302], and biotic systems are in the diachronic process of evolving. Meanwhile, as the increasing of speed leads to mass-energy equivalence that opens the door to the world of subatoms, speculatively, the increasing of complexity might open a door to the world of complexity. Therefore, in the following, we discuss this work from the perspective of complexity.

In this work, though we try to reach the complex world by leveraging on existing biology and complexity theories, the backbone is still extended from the theory of physics: the self-organizing process of DNNs is characterized as a symmetry-breaking process. To extrapolate the speculation of P. Anderson given in supp. C A 2 that speculates the increase of sophistication of symmetries breaking correlates with the increase of complexity, symmetry breaking and complexity suggested by this work is like a duality: the accumulation of a large number of adaptive symmetries breaking manifests as the complex behaviors of a system.

More specifically, the formalism in this work formalizes a series of informally description of the behaviors of complex systems under the context of DNNs. First, the circuit-symmetry breaking process encodes information of the environment/dataset by breaking the adaptive-symmetrical random fluctuations of basis circuits, which is a formalism of phenomena (of DNNs) described by phrases given as “order from fluctuations” [120], “order from noise” [100], or “order from chaos” [136] (cf. section II E 1). Second, at the end of the training, the complex patterns in natural images that could be classified by a DNN are what would be referred as complexity, and this training process is a process where random perturbations produce a change in organization by reducing the redundancy (i.e., a reservoir of basis circuits with circuit symmetry) and increasing the complexity of a system—at least, up to a certain point, as long as there is enough redundancy (i.e., the plasticity phase) to keep the system going—which is a formalism of the phenomena “complexity from noise” [303, p. 154], or complexity from diversity [137] under the context of DNNs. Third, the complexity of a DNN arises from its interaction with the environment through a feedback-control loop composed by a coarse-grained variable and hierarchical circuits, which is also a formalism of developments (applied to DNNs) propose that complexity emerges from signals from environment [46] through coarse-grained variables computed by hierarchical circuits [49].

Therefore, although this discussion section mostly aims to clarify understudied concepts in the extended symmetry-breaking process of DNNs, we conclude with a statement that summarizes the plasticity phase from the perspective of complexity. In doing so, we point out the connection between adaptive-symmetries breaking and complexity. Similar to the phenomenon that complexity in biotic systems arises as biotic diversity selected by fitness maximization, the complexity in DNNs arises through adaptive symmetries breaking where

neural-circuit diversity is selected by risk minimization. Therefore, adaptive-symmetry breaking process could summarized as **complexity from adaptive-symmetries breaking**, which characterizes the phenomenon that:

> DNNs are able to increase the potential complexity of the system plastically, and when the potential complexity of a system is larger than the complexity of a dataset, a DNN could absorb informational perturbations from the environment and self-organize into a functional structure that reaches a goal with zero training errors measured by a certain surrogate risk.

Through such a summary, we point to the uninvestigated behaviors of DNNs in vast uncharted area in the brave new world of complexity.

## D. EPISTEMOLOGY AND METHODOLOGY, FROM DISORGANIZED COMPLEXITY TO ORGANIZED COMPLEXITY

From glassy systems, biotic systems to DNNs, in a highly abstract level, the self-organization of the systems are all goal-directed behaviors: glassy systems minimize free energy; biotic systems maximize fittness; and DNNs minimize risk. However, as the interactions among units become increasingly complex, the emergent system behaviors gradually morph from macroscopic broken symmetries to sophisticated teleological behaviors. The complexity in physical systems is known as *disorganized complexity*, whereas the complexity in biotic systems is known as *organized complexity* [1]. Underlying these emergent phenomena, there lies incremental changes that accumulate into qualitative evolution of the way that the units in the systems are self-organized. In this section, we review such morphism of the preceding self-organization systems and the methodologies that study them, which provides the context of our method.

More specifically, in supp. D A, we review that to study organized complexity, we need to study a fundamentally different type of biological symmetries that characterize invariant of adaptation instead of the physical symmetries that characterize the invariant of free energy. In supp. D B, we review that the coarse-graining of the symmetric behaviors of microscopic units needs to shift from the level of individual units, to circuits composed by the units in a feedback-control loop. In supp. D C, we review the epistemological role of phase, phase space, and how order parameters are identified in physics. In supp. D D, we review the epistemological role of control parameters, and the formulation of assumptions in physics. In supp. D E, we review how a phase of a physical system is identified. In supp. D F, we review the shift of the concept of criticality in biotic systems: it shifts from singular criticality in physics to criticality that extends over space and time.

### A. From conservative-symmetry breaking to adaptive-symmetry breaking

In this section, we discuss the epistemological role played by symmetry in physics, and from such an epistemological analysis of the concept of symmetry, we discuss possible symmetries in biotic systems; the discussion suggests a different type of symmetry-breaking which we referred as *adaptive symmetries*, in contrast to the symmetry-breaking in physics, which is referred as *conservative symmetries*. An adaptive symmetry of DNNs referred as *circuit symmetry* is defined formally in this work, and is introduced in section II D 2.

Symmetry has been the foundational concept of physics that formalizes invariants of the physics systems under study that constitutes the fundamentals of the science of the systems [36, 37], as briefly reviewed in the following. All fundamental laws of physics are the implementations of a geodesic principle (minimization of certain *potential functions*) under an appropriate mathematical space. The understanding of systems' behaviors lies in the identification of a mathematical space and the metric in the space that measures the behaviors of the system. The construction of such a mathematical space requires stable (i.e., invariant) behaviors over time that could be observed by spatial or/and time scale of human perception; that is, a *conservation law*. Such stable behaviors are ergodic states of the system that are related by symmetric transformations that conserve the potential. And thus, the study of the behaviors of a physical system converts to the study of symmetries of the system: that is, symmetries construct objectivity by identifying observables that are stable such that they could be measured by instruments; furthermore, the breaking of symmetries is associated with the change of a system's stable behaviors, and thus characterizes the dynamics of the system; and the hypotheses posed by these mathematical structure and the experimentally validation of the hypotheses through measurements on the observables constitute the fundamentals of the science of the system. Further discussion can be found in Bailly and Longo [36]. We further give an example under our context. A spin glass is a complicated system where the interaction of spins are governed by quantum physics. However, the behaviors of the system can be understood by idealizing the spins and analyzing only the symmetries of the system in a mathematical space under the geodesic principle; for example, the spin glass model. The spins in the spin glass model are binary random variables in a probability measure space (i.e., the mathematical space), whose law is a Boltzmann distribution. The system minimizes (i.e., the geodesic principle) the free energy (i.e., the metric in the space). At a high temperature the rotation symmetry of the spins are the stable invariant that characterizes the behaviors of the system—rotation of the spins conserves the free energy. Energy dissipation of the system decreases free energy, and thus breaks the rotation symmetry. The breaking of the rotational symmetry characterizes the dynamics (phase diagram) of the system. The dynamical process can be experimentally observed by measuring the magnetization, and the spin glass order parameters, which are coarse-grained behaviors of symmetric units in the system.

Therefore, symmetries formalizes the conserved behaviors

(e.g. free energy in a spin glass) of a physical system when no external factors (e.g., energy) are influencing the system; and the breaking of symmetries characterizes the breaking of the conserved behaviors, and thus the dynamics of the process. In this regards, symmetries in physical are **symmetries of conservation**, or **conservative symmetries**.

However, in biotic systems, no conserved behaviors exist because a biotic system is in a non-equilibrium state that continually intakes energy, and thus the conserved behaviors are continually being broken [37]. This can be concretely seen in the frustration phenomenon in DNA molecules. As a macromolecule consists of orders of magnitude more atoms than a molecule in a typical glassy system, it contains many symmetric states of similar free energy separated by small energy barriers. At the evolutionary timescale, the systems are continually adapting by transiting from one state to another state; that is, continually breaking symmetries, and in a diachronic process of becoming [38].

Although that symmetries are invariants of systems under study that constitute the fundamental of the science of the systems, under such an epistemology, invariants do not necessarily need to be the invariants of conservation. In this regard, it has been proposed that the *trajectories (dynamics)* of biotic systems are *generic* whereas *static states* of the systems are *specific* Longo and Montévil [37], Montévil *et al.* [47], and biotic systems regulate and control the process, but not the content of the process [52], in contrast to the case of physical systems where the static states of the systems are generic whereas the dynamics is specific. We come back to the example of spin glasses to illustrate the statement. Given a spin glass, we perceive the identity of the system as a static system without or without magnetization (despite the aging phenomenon), whereas the dynamics of the system is understood as a transient process (trajectories in the phase space) through which the system is magnetized or demagnetized. However, given a biotic system, for example, the genes, its static state is not perceived as the identity of the system because it is the history (polygenesis) and the dynamics (ontogenesis) of the system that has regularities that holds explanatory or predictive power: the diversity of the beak of *Darwin's finches* is explained by the diachronic process of adapting to different but similar environments, i.e., evolution; and the information encoded in genes of sea urchin is understood by studying the dynamic process driven by the feedback-control loop implemented in the gene regulatory network (more on this in supp. D B).

Therefore, invariants still exist in biotic systems, but not in the form of symmetries of conservation, but as the invariant of change/variants. And in this work, we shall formalize such invariants in DNNs, which we refer as the **symmetry of adaptation**, or **adaptive symmetry**, as introduced in the following. The symmetries of adaptation is not symmetries of conservation, for example, induced by simple symmetric configurations of molecule structure that conserve free energy, but the symmetries of possible directions to adapt, induced by the complex cooperative interaction among the heterogeneous units in a biotic system. Such adaptive symmetries have been studied in biology for some time [45], though their physical mechanism and connection to the conservative symmetries in physics is still not fully understood, and a formalism comparable to the Noether's theorem in physics is yet to be formulated [37, 61]. The breaking of such symmetries results in functional diversification on every scale, from molecular assemblers, to subcellular structure, to cell types themselves, tissue architecture, and embryonic body axes [45]. The symmetry breaking process is also a typical self-organizing process triggered by random fluctuations and feedback signals [45]. For example, the cell specification in the embryonic differentiation could be conceptualized as a symmetry breaking process: from a symmetric state where an embryonic cell has multiple ways to adapt, in response to the feedback signals regulated temporally and spatially by *gene regulatory networks* [43, 44], the cell breaks the symmetry, and specifies into more specialized types of cells; therefore, to study biotic systems, not only the concept of symmetries from physics is needed, so is the concept of feedback and control [41]. In the lifespan of a biotic system, the symmetries and broken symmetries *coexist*, and might be a way to characterize structural stability and adaptability of life [37]: for example, despite an organism was developed by breaking a sequence of symmetries since the embryonic stage, immune cells could still break symmetries and differentiate into specialized immune cells in response to specific pathgens.

### B. From coarse-graining of conservative-symmetry to coarse-graining of adaptive-symmetries in feedback-control loop composed by hierarchical circuits

The macroscopic behaviors—that is, the order at a higher scale—of a self-organizing system is induced by the symmetries of microscopic units in the system; for example, for glassy systems, it is the macroscopically synchronized symmetries of microscopic spins that are perceived as magnetic force. Thus, the system could be studied through interaction between the symmetries and the macroscopic behaviors of the system, by typically formulating variables that *coarse-grain* over the symmetric behaviors of constituent units. Meanwhile, as discussed in supp. D A, the symmetries in biotic systems are not symmetries of conservation, but symmetries of adaptation; and thus the methodology correspondingly shifts: different from the study in physical systems that coarse-grains over symmetries of conservation through representative techniques like renormalization group [58–60, 122], the study of biotic systems analyzes the symmetries (and symmetry breaking) in the feedback-control loop between *hierarchical circuits* (or simply *circuits*) in the system and the coarse-grained variables computed by the circuits. We formalize such a feedback-control loop of DNNs in this work. Intuitively, the formalism formalizes hierarchically coupling among neurons where the weights among units adapt cooperative according to the gradients recursively computed from the coarse-grained variable at the top layer. This loop is introduced in section II C under the context of biological feedback-control loop.[14]. We introduce

[14] There might be confusions: given the observation that hierarchical circuits seem to manifest clearer in neural networks than in biotic systems, so why

the biological feedback-control loop in the following.

In physics, as a result of symmetries, the coarse-grained variable that characterizes physical systems could be computed by integrating over activities of constituent units. In simpler self-organizing physical systems, the symmetries enable the system to be characterized by coarse-grained variables that are the simple average of activities of units; for example, the well known variables such as volume and pressure of a water molecule system. Similar ideas apply to complex physical systems, where symmetries enable a coarse-grained characterization of the system that could be recursively, or hierarchically, computed through iterative renormalization over the symmetrical groups that integrates out short-range interaction among units, and summarizes the macroscopic behaviors [122]. Perhaps the most widely studied example is the study of spin glasses based on renormalization group [58–60].

However, in biotic systems, as discussed in supp. D A, symmetries are continually being broken; and thus the stable/invariant behaviors of the system shifts from conservation (of the potential function) to adaptation. In the context of complex systems, they are referred as *complex adaptive systems* [3, 311–314]: a complex adaptive system consists of a vast number of *heterogeneous* microscopic agents that interact locally in a *hierarchically coupled* way against teleological feedback signals and induce an emergent macroscopic phenomenon. The lack of stable conservative symmetries makes solutions that relies on such symmetries (e.g., the renormalization group technique previously) nonapplicable and the distinction between scales obscure. The challenges become how to analyze the spatially and temporally heterogeneous units, and the coupled interaction among units that a microscopic change at one scale has implications that ramify across scales throughout the system [69, 70].

Our study could be appreciated under the efforts to theorize biology through the concept of symmetry breaking, which has been introduced in supp. D A, and through the concept of computational circuits, as introduced in the following.

The adaptive-symmetry breaking could be systematically studied through analyzing the **feedback-control loop** between **hierarchical circuits** (or simply **circuits**) in the system and the coarse-grained variables computed by the circuits; the circuits are networks composed by the coupled heterogeneous units that intake feedback (signals from the environment and other units in the system), perform internal computation, and effect actions, and meanwhile compute the coarse-grained variables in the process [48, 49]. For example, in the genotype of an organism, the hypothesis of the organism is encoded as the coupling of heterogeneous genes, and could temporally and spatially regulate the development of the organism. The regulatory process could be studied by analyzing the hierarchical circuits (e.g., gene regulatory networks) that implement feedback-control loops with hierarchically coupled regulatory logic operation and gene expression (which for example, could generate regulatory signals) [43, 44]—hierarchy here refers to, for example, the animal body development determined by gene regulatory networks, where each phase of the development encoded by the genes has beginning, middle and terminal stages, and later events recursively refine the body parts developed in early events [43]. To give a concrete example, the mechanism of the cell specification of sea-urchin embryo was discovered by studying the feedback-control loop between the hierarchical circuits and the differentiation of cells at different regions of the embryo: in this case, the cells' relative positions could be interpreted as the coarse-grained variables that are computed from circuits composed by the constituent units; the computed coarse-grained variable in turn controls the symmetry breaking of constituent units, i.e., specification of cells in the embryo, which specifies according to the feedback signals dispersed by the regulatory network according to the relative position [49, 315]—that is, a feedback-control loop.

### C. Definition of phase and order parameter through symmetries

Coarse-graining variables introduced in supp. D B compose the *phase space* of a physical system, where the coarse-grained variables are further categorized as *control parameters* and *order parameters*, and the distinctive macroscopic behaviors (i.e., order) of the system are referred as the *phases* of the system. In this section, we clarify the concepts of phase and order parameter—control parameter is clarified next in supp. D D. According to the epistemology reviewed here, we define the order parameter (which is introduced in section II E), and a phase (which is introduced in section II F) of DNNs in this work.

To begin with, we summarize the concepts. In physics,

1. a phase referrs to a collection of a system's states with *stable symmetries* [38];

bother borrowing conceptual aids from biotic systems to explain our study of DNNs? A short answer is that both the study of biotic systems and DNNs were influenced by the same origin, and the more theoretical works were developed in the former perhaps because they are relatively simpler. The long answer is given as follows. In the colloquial language, "circuit" normally denotes the electronic circuits, which a cultural import to other disciplines from electronic and computer science. In the formative years of computer science, it was importantly influenced by a logic model of the brain [304], which we may refer as the McCulloch-Pitts model [305], or the MP model. The algorithmic thinking developed since then provided a mental framework to study natural and social phenomena as computational phenomena, and under such a framework, theories and methodologies were developed for biotic systems that evolved earlier, which are simpler and more observable than the brain. Meanwhile, DNNs are phenomenological models of the brain whose intellectual forbears, e.g., Perceptron [306], were also further developed from the MP model to handle uncertainty. This line of works developed mostly by pushing benchmarks that solved increasingly difficult engineering problems, and was relatively deficient in building theories. And now, sensibly though not without a sense of awe of the century-long efforts, the concepts developed from the early study of the brain come back to become the concepts to help study the phenomenological model of the brain, i.e., DNNs. The connection between DNNs and complex systems could go even deeper: MP-model was developed within the school of Cybernetics ([5, Chp 2], [307–309]), which also exerted intellectual influence on complex systems [71]; and we would not expand on this vast topic. In addition, we note that neural circuitry is also an explicitly discussed concept in neuroscience [310, p. 521], however, perhaps the biotic nervous system is more a mystery than DNNs, and we would not expand on this vast topic as well.

2. and an order parameter quantitatively characterizes the macroscopic order (i.e., coarse-grained effect of the symmetries) of a system, and is the *elementary excitation* [35, Chp 9.3] of the system in response to perturbations—that is, the behaviors of the system in response to (external or internal) perturbations as a result of the coarse-grained effect of the system's symmetries.

It is in the sense of phase and order parameter explained here that we shall discuss the phases and order parameter of DNNs. We elaborate these two concepts in the following.

### 1. *Phase and phase space*

First, we clarify the concept of phase space. Recall that in supp. D A, we have discussed that (pertinent/interesting) invariants/symmetries identify stable observables that could be measured, and from these observables, hypotheses could be formulated and verified, which constitute the fundamentals of the science of a system. These observables are organized under the concept of phase space [38]. More specifically, in physics, a **phase space** is the space of *observables* (and parameters) that uniquely determines the trajectories of a system [38]; that is, along with the potential function, they compose a formal and quantitative characterization of the geodesic principle of a specific physics law—the geodesic principle is discussed in supp. D A. Thus, given the potential function and the phase space, the system's behaviors (of interest) are determined. And, each **phase** in the phase space refers to a collection of states (or in the degenerate cases, e.g., classic mechanics, a single state) of a system that is of certain stable symmetries, and corresponds to a coordinate or region in the phase space.

We illustrate the concepts with the phase space in statistical mechanics. A statistical physical system, e.g., a spin glass, consists of a great number of molecules, and it is impossible to measure the position and velocity of each molecule in the system. However, as a result of the ergodicity and symmetries in the system, the macroscopic behaviors of the system are stable and are measured in observables such as temperature and the spin glass order parameters (cf. the discussion of relationship between symmetries and physical laws in supp. D A). Thus, despite the great number units in the system, the pertinent trajectories of the spin glass system can be uniquely determined by the parameters (i.e., temperature $T$ and the average coupling constant $J_0$) and the order parameters: the phase space of a spin glass model could be drawn on a coordinate system where the $x$-axis is $J_0$ and the $y$-axis is $T$, and phase transitions are trajectories on the coordinate system (cf. figure 2.1 in Nishimori [123])—in this case, the magnetization and spin glass order parameter are not drawn as separated axes but as labels on the regions of the phase space. The phases of the magnetic system are regions in the phase space: for example, the ferromagnet phase (which is of translation symmetry, but of broken rotation symmetry), or the spin glass phase (which is of broken replica symmetry).

### 2. *Elementary excitation and order parameter*

A phase of a system in statistical mechanics is quantitatively characterized by **order parameters** that are obtained by identifying the symmetries of the system and examining the elementary excitation of the system in response to perturbations [35, Chp 9.3]. We elaborate with the derivation of the spin glass order parameter of the spin glass model in this subsection.

An elementary excitation of a system is the behaviors of the units of the system induced by perturbations. A statistical-physical system poses to minimize the free energy of the system, and the preferred symmetries of units in the system are also of relatively lower free energy. When the system dissipates energy, the symmetries in the system are perturbed and the system is excited to a lower energy state—if the energy dissipation is sufficient large or the system is at critical regimens, the symmetries would be broken, and the system would undertake a phase transition—and manifests a coarse-grained/macroscopic behavior, or an order, of the system. We demonstrate the derivation of the spin glass order parameter of the spin glass model through examining elementary excitation to motivate the definition of order parameter of DNNs.

The simplest spin glass model is given as the following Boltzmann distribution,

$$\rho(\boldsymbol{\sigma}) = \frac{1}{Z} e^{\frac{1}{n}\sum_{i=1}^{n}\sigma_i \sum_{j=1, j\neq i}^{n} \frac{1}{T} J_{ij}\sigma_j}, \qquad (110)$$

where $\boldsymbol{\sigma}$ is of length $n$, whose components $\sigma_i$ is a binary random variable supported on $\{-1,1\}$ and represents a spin; $T$ is a parameter characterizes the uncertainty of the environment, and originally represents temperature in the Boltzmann distribution; $J_{ij}$ is the coupling constants that characterize the interaction among spins, which is normally randomly sampled from a probability distribution, e.g., the Gaussian distribution of mean $J_0$; $Z$ is the partition function.

The phases of spin glasses are characterized by order parameters as follows. An order parameter $q$ of spin glasses of the spin glass model is known as the *spin glass order parameter* [123, p. 17], and was originally derived from replica methods as

$$q = \frac{1}{n}\sum_{i=1}^{n} \mathbb{E}^2_{\rho(\sigma_i)}[\sigma_i]. \qquad (111)$$

$q$ characterizes the frustration phenomenon in a glassy magnet as follows. A glassy magnet frustrates as a result of the disordered interaction among spins, which is characterized as the random coupling constants $J_{ij}$ in eq. (110). The disordered interaction among spin variables induces metastable states where even in low temperature, the spins would not uniformly align with each other, which creates *local* environments in the materials where the average of spin directions is not zero, despite that the *global* average is zero; that is, the magnetization $m_n$

$$m_n = \frac{1}{n}\sum_{i=1}^{n} \mathbb{E}_{\rho(\sigma_i)}[\sigma_i], \qquad (112)$$

where the suffix $n$ is to distinguish it from the sample number $m$ in supp. B B 3, is zero, whereas $q$ is non-zero. This local

frustration does not exist in ferromagnets, because the local environments are uniformly the same. Together with $m_n$, $q$ characterizes different phases of the system, e.g., paramagnet ($m_n = 0, q = 0$), spin glass ($m_n = 0, q > 0$), or ferromagnet ($m_n > 0, q > 0$) phase. Similar to the phase transition in magnets at the critical temperature, the transition between these phases of the spin glasses occurs at critical temperatures (cf. fig. 2.1 in Nishimori [123]).

The spin glass order parameter could also be obtained by examining the elementary excitation of the spin glass model in response to temperature perturbations. Recall that the spin glass order parameter characterizes the drifting phenomenon that energy fluctuations in a spin glass could enable the system to cross energy barriers. Such energy fluctuations are typically heat fluctuations. Thus, the drifting is an elementary excitation of the system in response to heat fluctuations. Taking the first-order derivative free energy against temperature, the spin glass order parameter could be obtained as follows.

$$-\frac{\partial F}{\partial T} = -\frac{\partial - T \ln Z(\boldsymbol{x})}{\partial T} \tag{113}$$

$$= T \sum_{\boldsymbol{\sigma} \in \{1,-1\}^n} \left( \frac{1}{Z} e^{\frac{1}{T}\sum_{ij} J_{ij}\sigma_i\sigma_j} \sum_i -\frac{1}{T^2} J_{ij}\sigma_i\sigma_j \right)$$

$$= -\frac{1}{T}\mathbb{E}_{\rho(\boldsymbol{\sigma})}[\sum_{ij} J_{ij}\sigma_i\sigma_j]. \tag{114}$$

Equation (111) is proportional to eq. (114) by taking the mean-field assumption that $\sigma_i, \sigma_j$ are independent random variables. The magnetization order parameter $m_n$ can be derived similarly by taking derivative w.r.t. an external magnetic field, which is omitted in our discussion. The frustration phenomenon can also be characterized with eq. (114): at high temperature, eq. (114) is zero, and thus the system is in a disordered phase and its free energy roughly stays stable; at low temperature, eq. (114) is small yet nonzero, and thus the system gradually decreases its free energy but in a slow pace, i.e., drifting.

To clarify, despite the seemingly formal and systematical derivation of the spin glass order parameter, the identification of order parameters of a statistical-physical system is still an art [35, p. 274]—the hard parts are to identify the right Boltzmann distribution and the proper assumptions (e.g., mean-field assumptions) on the units. The preceding derivation is clean only in retrospect.

If a system is continually being perturbed, the derivative would become part of a differential equation that characterizes the dynamics of the system. And thus order parameters also characterize the macroscopic dynamics of the system—it is in this sense that Synergetics [102, p. 25] generalizes the definition of order parameter. So is our generalization of order parameter to DNNs.

### D. From symmetries to assumptions and control parameters

The phase space introduced in supp. D C is essentially a model that adequately characterizes a physical system in a way that explains the system's behaviors. Therefore, the quantification of the coarse-grained variables (identified through symmetries) is essentially an approximation, and thus are usually referred as assumptions that are self-consistent with the phenomena being modeled. And the parameters of the coarse-grained variables (or as the coarse-grained variables themselves) that control the phase transitions are referred as *control parameters*.

In this section, we first elaborate the assumptions and control parameters the through formulation of the classical mean-field assumption and the control parameters of spin glasses. Then, we suggests that unlike uniform control parameters (e.g., temperature) of physical systems, to study DNNs, we might need fine-grained control parameters over the coupling among neurons. The control parameters in this work (introduced in section II F 4) is formulated according to the epistemological role of control parameters reviewed here.

The mean-field assumptions are not physical reality, but they are formulated to approximately characterize the coarse-grained behaviors of the system as a result of symmetry and disorganized interaction, as explained in the following. As a result of translational symmetry, the behaviors of spins are homogeneous. Furthermore, the homogeneous behaviors are disorganized and cancel each other out: in the neighborhood of a spin, the disorganized force between the spin and the neighboring spins makes the higher order interaction among these spins cancel out, and the first order statistics of the spin direction statistically approximate the behaviors of the spin—this is also why mean-field methods only accurately describe Ising models (of magnets) of infinite range, or of dimension larger than or equal to four [122, p. 226], where the neighborhood of a spin contains enough spins for the force to cancel out one another. Therefore, the behaviors of microscopic spins could be characterized by the average/coarse-grained behavior, which is formulated as assumptions in the mean-field theory.

The assumptions are parameterized by a set of control parameters that characterize the symmetric behaviors of spins, and provide a way to control the behaviors (microscopic and macroscopic) in the system; this can be seen in the example of temperature of a spin glass. As discussed previously, as a result of the translational symmetry, a spin glass system behaves like a macroscopic spin, or as a field, whose behavior is the average of all spins. Thus, temperature—that is, the average kinetic energy—characterizes both the kinetic energy of the field, and the microscopic kinetic energy of individual spins. When the system dissipates heat/energy at specific parts of the system, the energy of the whole system tends to dissipate as a result of the disorganized interaction. Over a timescale meaningful for observation, The kinetic energy of all spins would fall uniformly/symmetrically and the temperature would fall accordingly. When the temperature falls to the extent that the inter-spin interaction dominates over the kinetic energy of spins, the macroscopic behavior of the system changes by undertaking a phase transition.

The mean-field assumption, and the control parameters together bridges the microscopic to the macroscopic in the methods known as mean-field methods—perhaps the simplest statistical field methods— where the phases and phase transitions of spin glasses are studied [123].

For DNNs, the mean-field assumption does not apply to

neurons because the interaction of neurons is *organized*. Unlike the coarse-grained variables in the spin glass (e.g., the magnetization and the spin glass order parameter), which is a construction of scientists that characterizes the collective behaviors of the spins in the system, the coarse-grained variable in a complex adaptive system is computed by the system itself (cf. the discussion of coarse-grained variables in supp. D B). For a DNN, the coarse-grained variable is computed by hierarchical coupling among neurons. Thus, the value of the coarse-grained variable is directly computed by incoming synapses/edges that are different from one another because they are supposed to coarse-grain different mesoscopic or macroscopic patterns. A mean-field assumption ignores such hierarchical coupling, and no patterns could be recognized because the circuit simply would output random values independently with the input examples. Thus, the mean-field assumption, at least in this naive form at the level of neurons, stops to characterize DNNs.

Therefore, to study such organized complexity, we investigate DNNs as follows. We characterize the self-organizing process as an adaptive-symmetry breaking process driven by a feedback-control loop between hierarchical circuits and a coarse-grained variables in a DNN (cf. supp. D B). To understand the symmetry-breaking process, instead of analyzing at the granularity of neurons, we look at the *granularity of circuits* and formulate assumptions on the coupling among circuits through adaptive symmetries. Meanwhile, a set of control parameters parameterizes the assumptions, which are fine-grained quantitative characterization of the coupling among circuits. The assumptions, the control parameters and together with a theorem proved from the assumptions characterize a phase of DNNs.

### E. Hessian analysis on stability of symmetries and on local geometry of potential function landscape

In supp. D C, we have recalled that in physics, a phase is defined as a collection of states with stable symmetries. The stability of symmetries in physics systems is studied by analyzing effect of second order perturbations, which for high dimension problems, is the Hessian. Meanwhile, the analysis stability of symmetries is also the analysis of the local geometry of the potential function's landscape, where stable local minima are phases, and unstable states are transient states in phase transitions. We shall study the coarse-grained effect of the adaptive symmetry on the Hessian of a DNN's risk, which would suggest a phase of DNNs with stable symmetries. We introduce landscape analysis generally in this section.

Though the order of a phase is characterized by the order parameter (i.e. coarse-grained effect of symmetries, or in other words, elementary excitation) of the system, the stability of the order (and thus the symmetries) is characterized by derivatives of order parameter, i.e., the second order interaction among units. This can be seen in the analysis of phase transitions in physics. Phase transitions in spin glasses are characterized by the singular changes of order parameters, and such singularities are studied by analyzing the second order interaction among spins, for example, magnetic susceptibility (the second order derivative of the free energy w.r.t. the external magnetic field): in the paramagnetic phase, the magnetic susceptibility is zero, and becomes infinite at critical regime. Thus, second order quantities characterize the stability of the symmetries that induces the order characterized by the order parameters.

Formally, for a system whose state $\boldsymbol{x}$ is high dimensional, the local geometry (i.e. stability) of a state is characterized by the *Hessian*, $d^2\phi(\boldsymbol{x})/d\boldsymbol{x}^2$, of the system's potential function $\phi(\boldsymbol{x})$, which characterizes the second-order interaction among constituent units; it informs the directions that could further decrease $\phi(\boldsymbol{x})$, as explained in the following. A self-organizing system starts from a disordered state and ends at an attractor where $d\boldsymbol{x}/dt = 0$. When the system is driven to minimize a function $\phi(\boldsymbol{x};\boldsymbol{c})$, $d\boldsymbol{x}/dt$ is given as $\nabla_{\boldsymbol{x}}\phi$ (or quantities that derived from $\nabla_{\boldsymbol{x}}\phi$ in more sophisticated algorithms), and an attractor is a *stationary point* of $\phi_{\boldsymbol{x}}$ where $\nabla_{\boldsymbol{x}}\phi = 0$. At the stationary points of $\phi(\boldsymbol{x})$, the *eigenspectrum* (the distribution of eigenvalues) of its Hessian informs the types of the stationary points: all-positive eigenvalues corresponds to a local minimum (black dots in fig. 5); all-negative eigenvalues corresponds to a local maximum; otherwise, $\phi(\boldsymbol{x})$ is a saddle point, implying that the state is unstable and extra directions exist to further minimize $\phi(\boldsymbol{x})$ (the white dot in fig. 5).

Therefore, the local geometry of all states of a system, which is referred as the *landscape* of the system's potential function, characterizes the phases and phase transitions of this system. Formally, the landscape of a function $\phi(\boldsymbol{x})$ denotes the graph, i.e., the ordered pair $(\boldsymbol{x}, \phi(\boldsymbol{x}))$, of $\phi(\boldsymbol{x})$. In low dimensional space (two, or three dimension), the graph of $\phi(\boldsymbol{x})$ resembles a mountain, and thus is referred as the landscape. The self-organizing process is a process where the system moves from stationary points to stationary points on the landscape. The dynamics and the properties of self-organization are characterized by transition trajectories between stationary points, and stationary points of the landscape.

Such landscape analysis is a practiced technique that study the evolution of complex systems. For example, researchers have studied the potential energy landscape of the system, e.g., that of protein, glasses [316], evolution (Gros [317] Chapter 6, Nicolis and Nicolis [6] Chapter 3.8), where emergent properties are predicted from local minima and the transition states that connect them [318]. In these problems, a full characterization of the landscape could inform researchers the system is structure-seeking that equilibrates rapidly, or has competing structures or morphologies, which may be manifested as phase transitions and even glassy phenomenology [318]. To give an example, the frustration phenomenon of spin glasses is studied by analyzing the energy landscape: a landscape analysis of a spin glass model through Hessian informs that local minima are increasingly numerous as the free energy deceases Auffinger *et al.* [319].

### F. From singular criticality to extended criticality

To transit from a phase of a type of stable symmetries to another, the system needs to be in state of *criticality*. Unlike the power-law singularities at a specific control parameter (e.g.,

the Curie temperature) in physics, the criticality of biotic systems exists in an interval of control parameters, and is referred as *extended criticality* [36, 37, 42], which characterizes the phenomenon that a biotic system is in a continual symmetry breaking process where the system is in critical states extended throughout space and time. We introduce the concepts of extended criticality in this subsection, which sets the background of the criticality of DNNs discussed in supp. C B.

### 1. Criticality and timescale of symmetry breaking

To begin with, we describe the criticality in the singular phase transitions in physics. A phase transition of a statistical physical system is a process where the free energy (i.e., potential function) of the system undertakes singular change as a control parameter (e.g., the temperature) crosses a critical threshold, and the system transits from one phase (of one type of stable symmetries) to another. We describe the process with the concepts introduced so far. Properties of units (e.g. molecular structure of spin glasses) induce forces in physical systems that prefer a certain *low-energy* structure of *broken symmetries*—i.e., a structure that is less symmetric than the structure of the system in a disordered state. At high temperatures, the forces that prefer broken symmetries are disrupted by the thermal fluctuations, and thus are uncoordinated and tends to decay without an influence beyond the immediately microscopic neighborhood; and the system is at an *equilibrium*. As the control parameter changes (e.g., rapid decrease of temperature), at a *critical* temperature, the forces would triumph over thermal fluctuations, and broken symmetries at a microscopic scale would be synchronized macroscopically. Then, the system would undertake a *phase transition* from a disordered equilibrium to macroscopically manifest the broken symmetric structure (e.g., alignment of spin directions of spins to manifest magnetization)—another equilibrium—and transits from one local minimum of free energy to another. The singular change is characterized by the discontinuous singularities in the first-order derivatives (e.g., entropy and volume of water), or a *power-law singularities* in the first-order derivatives (e.g., magnetization of ferromagnets) at critical control parameters (c.f. [35, Chp 11,12]): that is, at critical control parameters, the perturbations of a microscopic unit would be synchronized macroscopically and cause a singular change of free energy. In the case of spin glasses, the spin glass order parameter is of a **power-law**[15] against *perturbations of spins* at critical temperature [320, p. 237], in addition to other quantities with a power law [321].

However, these singularities in physics are mathematical abstraction, and the complexity of the symmetries increases, the timescale of phase transitions increase. Though the magnetization of ferromagnet is mathematical characterized as a singularity, in practice, the synchronization of broken symmetries of a system is like percolation: a microscopic broken symmetry is synchronized over a local area of the system whose scale is macroscopic, not necessarily over the whole system; and the domino effect that the broken symmetries are synchronized over the whole system takes some time to propagate. The frustrating of spin glasses is an extended process of such domino effect, which is caused by spins' competing configurations that are of different symmetries, but also are of almost the same free energy. And thus the replicas (i.e., different spatial regions) in the system would choose one configurations, or another in a statistically random way, and the system hops from a local minimum of a particular configuration of symmetries to another as a result of the domino effect induced by energy fluctuations, and slowly drifts to the lowest possible free energy.

Biotic systems (e.g., DNA molecules) are much more complex macromolecules with manifold of competing symmetries; and for such more complex systems, a frustration phenomenon of DNA molecules at the *evolutionary timescale* has been hypothesized as the physical foundations of evolution [50]. As in a frustrated system, the differences in free energies of DNA molecules with different nucleotide sequences are orders of magnitude smaller than the total energy of covalent bonds in these molecules. These different metastable states separated by these low energy barriers among DNA molecules are gnomes of different organisms. The drifting among the metastable states creates a population of organisms with diverse survival hypotheses, and the competition among these hypotheses manifests as evolution by natural selection.

### 2. Edge of chaos and extended criticality

The criticality over an extended timescale in evolution has been phenomenologically observed in a model known as NKCS model, This criticality is referred as evolution on the *edge of chaos* [42], and is further conceptualized as *extended criticality*. We introduce these concepts as follows.

The phenomenon of evolution at the edge of chaos is observed in a model known as the NKCS model of evolution [42]. NKCS model is an extension of the NK model [295], which is equivalent [7, p. 257] to the spin glass model introduced in supp. D C 2 that is known as Sherrington–Kirkpatrick model [123, p. 14]. NKCS phenomenologically models an ecosystem that consists of multiple competing NK models. More specifically, NKCS model characterizes an ecosystem of $S$ species by characterizing each species by a Boltzmann distribution, however, in addition to the intra-species coupling of genes characterized by the coupling constants $J_{ij}$ in the spin glass model given in supp. D C, inter-species coupling of genes is also characterized: each gene in a species is coupled with $C$ chosen genes from each of $S$ other species. In the computer simulations of the NKCS model, each species is assigned a random genotype and takes turns to mutate genes. A mutation

[15] Colloquially, a power-law criticality is an ordered macroscopic change of the system's behavior caused by microscopic perturbations of units of the system: "ordered" here refers to the phenomenon that a microscopic perturbation is not amplified, or attenuated exponentially as it propagates in the system, such that microscopic change would induce a stable system-wide (macroscopic) effect; otherwise, exponential amplification would result in chaotic behavior change, while exponential attenuation would result in no behavior change.

in a species would modify the fitness of the species, and the inter-species coupling would lead to mutations in other species to find another equilibrium where all species are at their local maxima, i.e., a Nash equilibrium. The phenomenon is called *avalanche*. The number of generations to reach another equilibrium is called the *avalanche size*, and a generation refers to the procedure where all species have taken turns to finish their mutation. The dynamics of the model is controlled by the relative size between $K$ and CS:

1. When $K > CS$, the system is in an **frozen** phase, where a mutation in a species would lead to a small avalanche size, and in the new equilibrium, the fitness of each species is close to the value before the avalanche.

2. When $K < CS$, the system is in a **chaotic** phase, where a mutation in a species would make the system keep mutating, and never reaches a new equilibrium. In this case, the avalanche size is infinite.

3. At the **critical** regimen $K_c := K = CS$, the avalanche size obtains its maximum. Meanwhile, the *mean fitness* of all species reaches the maximum as well. When $K$ diverges from $CS$, the mean fitness decreases: above (below) $K_c$, the average species fitness monotonously decreases with increasing (decreasing) $K$.

Therefore, at the critical ratio $(K/CS)_c$, a microscopic change (i.e., a mutation) can lead to the maximal macroscopic change (i.e., the avalanche size) of the system, without bringing chaos to the ecosystem, while at the same time, making the system reach the maximal mean fitness; more specifically, the avalanche size is of *a power-law* against *perturbations of genes*. The dynamics of the ecosystem at the critical ration is referred as **evolution at the edge of chaos**, and suggests an explanation to the punctuated equilibrium; that is, massive species extinction and creation events in the evolutionary history.

From the NKCS model, we could observe that phenomenological, the existence of power-law criticality—system-wide/macroscopic behavior change induced by unit/microscopic perturbations—exists in more than singular points (e.g., the region in the parameter space where $K$ and $CS$ are of a certain ratio), and the domino effect induced by microscopic perturbations takes more time to propagate. Furthermore, the edge of chaos hypothesis has been motivated by simulations of evolving agents [147], cell automata [148], and the phenomenological model of evolution [317, p. 136]. The hypothesis was originally proposed as a singular value of a parameter where computation could be performed best—though the vague concept of good performance is ill-defined [148]. However, such singular criticality has been found inaccurate because for evolving cellular automata to perform computation, a particular task is required to identify a particular range of the parameter for good performance, and more than one critical values of the parameter exists that have such edge-of-chaos phenomenon, which each corresponds to a way of breaking a symmetry, and a different fitness value [322].

Therefore, the concept of edge of chaos is further developed into a concept referred as **extended criticality** [36, 37]. Recall that in this subsection, we have discussed that DNA molecules are macromolecules that many metastable states that are of similar free energy separated by small energy barriers. Those metastable states could be appreciated as near-symmetric states of DNA. Because of the proliferation of the symmetries in biotic systems, criticality exists in a dense subset/interval of the multidimensional parameter space instead of a singular point. Through extended criticality, microscopic change of a unit can be amplified into a macroscopic change of the system, and thus penetrate scales; and the characteristics of such criticality is a power-law between a macroscopic variable and microscopic perturbations. And as a result of the proliferation of symmetries in biotic systems, evolution could be understood as being in an extended critical regimen of the state space, and in a continual symmetry-breaking process at the evolutionary timescale.

## E. PROOFS OF PROPERTIES OF CIRCUITS

### A. Proofs of properties of circuit calculus

The proofs given in this subsection are rather straightforward—the difficulty lies in the efforts to work out the definitions—and could be considered as exercises to get familiar with the circuit formalism.

*Proof of derivative rule of basis circuits, i.e., lemma 2.* We write out the $\Psi_{\boldsymbol{i}}^{s\ldots e}$ explicitly according to definition 16 as follows.

$$\Psi_{\boldsymbol{i}}^{s\ldots e} := H_{i_{s-1}}^{s-1} \prod_{l=s}^{e} w_{i_{l-1} i_l}^{l} H_{i_l}^{l},$$

where the neuron weights are written as lowercase scalars because they are realizations of neuron weight random variables. It is a simple multiplication of scalars and scalar random variables whose realizations are scalars. Therefore, taking the partial derivative w.r.t. $w_{i_{l-1} i_l}^{l}$ we have

$$\begin{aligned}\frac{\partial \Psi_{\boldsymbol{i}}^{s\sim e}}{\partial w_{i_{l-1} i_l}^{l}} &= H_{i_{s-1}}^{s-1} \prod_{l'=s}^{l'-1} w_{i_{l'-1} i_{l'}}^{l'} H_{i_{l'}}^{l'} H_{i_l}^{l} \prod_{l''=l''+1}^{e} w_{i_{l''-1} i_{l''}}^{l''} H_{i_{l''}}^{l''} \\ &= \Psi_{\boldsymbol{i}_{:l}}^{s\sim l-1} H_{i_l}^{l} \Psi_{\boldsymbol{i}_{l+1:}}^{\wedge l+1\sim e}.\end{aligned}$$

□

*Proof of derivatives of circuits, i.e., corollary 1.* To prove eq. (67), we apply lemma 2 to each of the terms in the summation. Note that for $\boldsymbol{i}$ that satisfies $w_{i_{l-1} i_l}^{l} \notin \boldsymbol{i}$, the derivative is zero.

Equation (68) is simply eq. (67) that takes an input at top layer. More verbosely, the first order (partial) derivatives of DNNs composed with a loss function in the circuit form are

calculated by applying lemma 2 as follows. □

$$\frac{\partial \mathscr{L}(T(X;\theta),Y)}{\partial w^l_{i_{l-1}i_l}} = \frac{\partial \mathscr{L}\left(\sum_{\boldsymbol{i}\in I} X_{i_0}\Psi^{\wedge 1\sim L\wedge}_{\boldsymbol{i}},Y\right)}{\partial w^l_{i_{l-1}i_l}}$$
$$= \partial \sum_{\boldsymbol{i}\in I^{\setminus\{l-1,l\}}_{i_{l-1}i_l}} X_{i_0}\Psi^{\wedge 1\sim l-1\wedge}_{\boldsymbol{i}:l} H^{l-1}_{i_{l-1}} w^l_{i_{l-1}i_l} H^l_{i_l}\Psi^{\wedge l+1\sim L\wedge}_{\boldsymbol{i}_l:}\mathscr{L}'(\cdot)/\partial w^l_{i_{l-1}i_l}$$
$$= \sum_{\boldsymbol{i}\in I^{\setminus\{l-1,l\}}_{i_{l-1}i_l}} X_{i_0}\Psi^{\wedge 1\sim l-1\wedge}_{\boldsymbol{i}:l} H^{l-1}_{i_{l-1}} H^l_{i_l}\Psi^{\wedge l+1\sim L\wedge}_{\boldsymbol{i}_l:}\mathscr{L}'(\cdot).$$

□

*Proof of the second derivatives of circuits, i.e., corollary 2.* The second order (partial) derivatives—that is, the Hessian entries—of a DNN composed with a loss function in the circuit form are calculated by applying corollary 1 twice as follows.

$$\frac{\partial^2 \mathscr{L}(T(X;\theta),Y)}{\partial w^l_{i_{l-1}i_l}\partial w^{l'}_{i'_{l'-1}i'_l}} = \frac{\partial^2 \mathscr{L}\left(\sum_{\boldsymbol{i}\in I} X_{i_0}\Psi^{\wedge 1\sim L\wedge}_{\boldsymbol{i}},Y\right)}{\partial w^l_{i_{l-1}i_l}\partial w^{l'}_{i'_{l'-1}i'_l}}$$
$$= \frac{\partial \sum_{\boldsymbol{i}\in I^{\setminus\{l-1,l\}}_{i_{l-1}i_l}} X_{i_0}\Psi^{\wedge 1\sim l-1\wedge}_{\boldsymbol{i}:l} H^{l-1}_{i_{l-1}} H^l_{i_l}\Psi^{\wedge l+1\sim L\wedge}_{\boldsymbol{i}_l:}\mathscr{L}'(\cdot)}{\partial w^{l'}_{i'_{l'-1}i'_l}}$$
$$= \sum_{\boldsymbol{i}\in I^{\setminus\{l-1,l,l'-1,l'\}}_{i_{l-1}i_l i_{l'-1}i_{l'}}} X_{i_0}\Psi^{\wedge 1\sim l-1\wedge}_{\boldsymbol{i}:l} H^{l-1}_{i_{l-1}} H^l_{i_l}\Psi^{\wedge l+1\sim l'-1\wedge}_{\boldsymbol{i}_{l:l'}} H^{l'-1}_{i_{l'-1}}$$
$$H^{l'}_{i'_l}\Psi^{\wedge l'+1\sim L\wedge}_{\boldsymbol{i}_{l'}:}\mathscr{L}'(\cdot)$$

where $l<l', l,l'\in[L]$—when $l=l'$, the derivatives are zero—and we have assumed that $\mathscr{L}''(\cdot)$ is zero because we study a class of loss functions whose second derivative is zero (this is formally given in supp. B C 8), e.g., hinge loss. □

*Proof of corollary 6.* Denote $X_{i_0}\Psi^{\wedge 1\sim l-1\wedge}_{\boldsymbol{i}:l} H^{l-1}_{i_{l-1}} H^l_{i_l}\Psi^{\wedge l+1\sim L\wedge}_{\boldsymbol{i}_l:}\mathscr{L}'(\cdot)$ as $\Omega^{\bar{l}\setminus\{l\}}_{\boldsymbol{i}}$, where $\bar{l}_{\setminus\{l\}}$ and $I^{\setminus\{l-1,l\}}_{i_{l-1}i_l}$ have the same denotation as in corollary 1. We can write the gradient of the risk as

$$\nabla_\theta R_m = \begin{bmatrix} \sum_{\boldsymbol{i}\in I^{\setminus\{0,1\}}_{00}} \Omega^{\bar{l}\setminus\{1\}}_{\boldsymbol{i}} \\ \vdots \\ \sum_{\boldsymbol{i}\in I^{\setminus\{l-1,l\}}_{i_{l-1}i_l}} \Omega^{\bar{l}\setminus\{l\}}_{\boldsymbol{i}} \\ \vdots \\ \sum_{\boldsymbol{i}\in I^{\setminus\{L-1,L\}}_{n_{L-1}n_L}} \Omega^{\bar{l}\setminus\{L\}}_{\boldsymbol{i}} \end{bmatrix},$$

which is a $N$-dimension vector, where $N=\sum_{l=1}^L n_{l-1}n_l$ is the number of weights. The square of the 2-norm of the vector is given as

$$||\nabla_\theta R_m||_2^2 = \sum_{l=1}^L \sum_{i_{l-1}=1,i_l=1}^{n_{l-1},n_l}\left(\sum_{\boldsymbol{i}\in I^{\setminus\{l-1,l\}}_{i_{l-1}i_l}} \Omega^{\bar{l}\setminus\{l\}}_{\boldsymbol{i}}\right)^2$$
$$= \sum_{l=1}^L \sum_{i_{l-1}=1,i_l=1}^{n_{l-1},n_l}\sum_{\boldsymbol{i},\boldsymbol{i}'\in I^{\setminus\{l-1,l\}}_{i_{l-1}i_l}} \Omega^{\bar{l}\setminus\{l\}}_{\boldsymbol{i}}\Omega^{\bar{l}\setminus\{l\}}_{\boldsymbol{i}'}$$

### B. Proofs of circuit symmetry and broken circuit symmetry of basis circuits

#### 1. *Proof of circuit symmetry*

We first present a lemma that characterizes the decay of the first moment to demonstrate the idea of the proof, and then present the proofs of results given in supp. B E 4.

**Lemma 8.** *Let $\Psi^{\bar{l}}_{\boldsymbol{i}}$ be a basis circuit of circuit symmetry, where $\bar{l}=(s,\ldots,e), s<e, s,e\in\mathbb{L}$, and $\boldsymbol{i}\in\otimes_{l\in\bar{l}}[n_l]$. Then, we have*

$$\left|\mathbb{E}\left[\Psi^{\bar{l}}_{\boldsymbol{i}}\right]\right| \le O\left(\left(\frac{c}{\sqrt{2n}}\right)^{2(e-s)}\right).$$

*Proof.* We calculate the mean of $\Psi^{\bar{l}}_{\boldsymbol{i}}$ as follows.

$$\mathbb{E}\left[\Psi^{\bar{l}}_{\boldsymbol{i}}\right]$$
$$= \int \psi^{s\sim e}_{\boldsymbol{i}} \prod_{l=s}^{e}\mu_l(\boldsymbol{h}_l|\mathscr{O}_{l-1})\mu(\boldsymbol{W}_l)\mu(\boldsymbol{x}_{s-1})d\mathscr{O}_l$$
$$= \int \prod_{l=s}^{e} h^l_{i_l} w^l_{i_{l-1}i_l}\frac{1}{Z_l}e^{\boldsymbol{x}^T_{l-1}\boldsymbol{W}_l\boldsymbol{h}_l}\mu(\boldsymbol{W}^l_{\mathbb{I}_l\setminus\{(i_{l-1},i_l)\}})\mu(w^l_{i_{l-1}i_l})\mu(\boldsymbol{x}_{s-1})d\mathscr{O}_l, \tag{115}$$

where

$$\mathbb{I}_l = [n_{l-1}]\otimes[n_l],$$

and

$$\boldsymbol{x}_l = \boldsymbol{x}^T_s \overrightarrow{\Pi}^l_{j=s}\boldsymbol{W}_j\mathrm{dg}(\boldsymbol{h}_j), Z_l = \sum_{\boldsymbol{h}_l\in\mathbb{B}^n} e^{\boldsymbol{x}^T_{l-1}\boldsymbol{W}^l\boldsymbol{h}_l}.$$

We give several remarks on the integral. First, because the neuronal gates $\boldsymbol{h}_l, l\in[L]$ are discrete random variables, the integral symbol should be a summation technically; but to avoid clutters, we denote them and the integration over weights and $\boldsymbol{x}_{s-1}$ with one integral symbol. Second, in the preceding probability factorization, despite the fact that $\Psi^{\bar{l}}_{\boldsymbol{i}}$ only involves $2|\bar{l}|-1$ number of random variables, the neuronal gates $H^l_{i_l}$ depend on the weights and neuronal gates of all previous layers. Third, we also clarify that in layer $e$, only the $i_l$th column $\boldsymbol{W}^l_{:,i_l}$ is actually necessary—the rest is integrated into one—the rest of $\boldsymbol{W}_l$ is included to enable us to write the measure in a single $\prod$ symbol compactly. Lastly, in the rest of the proof, for convenience and clarity, let $\boldsymbol{w}^l_{i_l}$ denote $\boldsymbol{W}^l_{:,i_l}$, and $G^l_{\neg i_l}$ denote $[n_l]\setminus\{i_l\}$.

The integral is a high dimension integral over $\mathscr{O}_l$. It could be calculated by first calculating the integral inside out. More

specifically,

$$\mathbb{E}\left[\Psi_{\boldsymbol{i}}^{\bar{l}}\right] = \int \dots \int_{-\infty}^{\infty} \sum_{h_{i_e}^e \in \mathbb{B}} h_{i_e}^e w_{i_{e-1}i_e}^e \mu(h_{i_e}^e | \mathscr{O}_{e-1}) \mu(\boldsymbol{W}_e) d\boldsymbol{W}_e \tag{116}$$

$$\prod_{l=s}^{e-1} \sum_{\boldsymbol{h}_l \in \mathbb{B}^{n_l}} h_{i_l}^l w_{i_{l-1}i_l}^l \mu_l(\boldsymbol{h}_l | \mathscr{O}_{l-1}) \mu(\boldsymbol{W}_l) \mu(\boldsymbol{x}_{s-1}) d\mathscr{O}_l, \tag{117}$$

and the integral could be calculated by first calculating eq. (116).

Therefore, to estimate an upper bound of $\left|\mathbb{E}\left[\psi_{\boldsymbol{i}}^{\bar{l}}\right]\right|$, we first calculate an upper bound of the innermost integral; that is,

$$\left|\mathbb{E}\left[\Psi_{\boldsymbol{i}}^{\bar{l}} | \mathscr{O}_{l-1}\right]\right|$$

where the integral is taken against $\boldsymbol{W}_l$ and $h_{i_l}^l$ ($l = e$), and more specifically,

$$\begin{aligned}
&\left|\mathbb{E}\left[\Psi_{\boldsymbol{i}}^{\bar{l}} | \mathscr{O}_{l-1}\right]\right| \\
=& \left| \int_{-\infty}^{+\infty} w_{i_{l-1}i_l}^l \frac{1}{Z_{i_l}^l} e^{\sum_{j_{l-1} \in G_{\neg i_{l-1}}^{l-1}} w_{j_{l-1}i_l}^l x_{j_{l-1}}^l} e^{w_{i_{l-1}i_l}^l x_{i_{l-1}}^l} \right. \\
& \left. \mu(\boldsymbol{W}_{\mathbb{I}_l \setminus \{(i_{l-1},i_l)\}}^l) \mu(w_{i_{l-1}i_l}) d\boldsymbol{W}_{\mathbb{I}_l \setminus \{(i_{l-1},i_l)\}}^l dw_{i_{l-1}i_l} \right|,
\end{aligned}$$

where

$$Z_{i_l}^l = \sum_{\boldsymbol{h}_l \in \mathbb{B}} e^{\boldsymbol{x}_{l-1}^T \boldsymbol{w}_{i_l}^l h_{i_l}}.$$

The integral inside $|\cdot|$ could decomposed into two parts as a result of weight symmetry, given as

$$\begin{aligned}
& \int_0^{+\infty} w_{i_{l-1}i_l}^l \frac{1}{Z_{i_l}^l} e^{\sum_{j_{l-1} \in G_{\neg i_{l-1}}^{l-1}} w_{j_{l-1}i_l}^l x_{j_{l-1}}^l} e^{w_{i_{l-1}i_l}^l x_{i_{l-1}}^l} \\
& \quad \mu(\boldsymbol{W}_{\mathbb{I}_l \setminus \{(i_{l-1},i_l)\}}^l) \mu(w_{i_{l-1}i_l}) d\boldsymbol{W}_{\mathbb{I}_l \setminus \{(i_{l-1},i_l)\}}^l dw_{i_{l-1}i_l} \\
+ & \int_0^{+\infty} - w_{i_{l-1}i_l}^l \frac{1}{Z_{-i_l}^l} e^{\sum_{j_{l-1} \in G_{\neg i_{l-1}}^{l-1}} w_{j_{l-1}i_l}^l x_{j_{l-1}}^l} e^{-w_{i_{l-1}i_l}^l x_{i_{l-1}}^l} \\
& \quad \mu(\boldsymbol{W}_{\mathbb{I}_l \setminus \{(i_{l-1},i_l)\}}^l) \mu(w_{i_{l-1}i_l}) d\boldsymbol{W}_{\mathbb{I}_l \setminus \{(i_{l-1},i_l)\}}^l dw_{i_{l-1}i_l}
\end{aligned}$$

where

$$Z_{-i_l}^l := 1 + e^{\sum_{j_{l-1} \in G_{\neg i_{l-1}}^{l-1}} w_{j_{l-1}i_l}^l x_{j_{l-1}}^l} e^{-w_{i_{l-1}i_l}^l x_{i_{l-1}}^l}.$$

We again note that although only one integral symbol $\int$ is used, and this integral is a high dimensional integral. And, we have

$$\begin{aligned}
& \left|\mathbb{E}\left[\Psi_{\boldsymbol{i}}^{\bar{l}} | \mathscr{O}_{l-1}\right]\right| \\
\leq & \int_0^{+\infty} w_{i_{l-1}i_l}^l \left| \frac{1}{Z_{i_l}^l} e^{\sum_{j_{l-1} \in G_{\neg i_{l-1}}^{l-1}} w_{j_{l-1}i_l}^l x_{j_{l-1}}^l} e^{w_{i_{l-1}i_l}^l x_{i_{l-1}}^l} \right. \quad (118) \\
& \left. - \frac{1}{Z_{-i_l}^l} e^{\sum_{j_{l-1} \in G_{\neg i_{l-1}}^{l-1}} w_{j_{l-1}i_l}^l x_{j_{l-1}}^l} e^{-w_{i_{l-1}i_l}^l x_{i_{l-1}}^l} \right| \quad (119) \\
& \mu(\boldsymbol{W}_{\mathbb{I}_l \setminus \{(i_{l-1},i_l)\}}^l) \mu(w_{i_{l-1}i_l}) d\boldsymbol{W}_{\mathbb{I}_l \setminus \{(i_{l-1},i_l)\}}^l dw_{i_{l-1}i_l}.
\end{aligned}$$

Note that

$$\begin{aligned}
& \left| \frac{1}{Z_{i_l}^l} e^{\sum_{j_{l-1} \in G_{\neg i_{l-1}}^{l-1}} w_{j_{l-1}i_l}^l x_{j_{l-1}}^l} e^{w_{i_{l-1}i_l}^l x_{i_{l-1}}^l} \right. \quad (120) \\
& \left. - \frac{1}{Z_{-i_l}^l} e^{\sum_{j_{l-1} \in G_{\neg i_{l-1}}^{l-1}} w_{j_{l-1}i_l}^l x_{j_{l-1}}^l} e^{-w_{i_{l-1}i_l}^l x_{i_{l-1}}^l} \right| \\
= & \left| e^{w_{i_{l-1}i_l}^l x_{i_{l-1}}^l} - e^{-w_{i_{l-1}i_l}^l x_{i_{l-1}}^l} \right| \\
& \bigg/ \left( e^{\sum_{j_{l-1} \in G_{\neg i_{l-1}}^{l-1}} w_{j_{l-1}i_l}^l x_{j_{l-1}}^l} + e^{w_{i_{l-1}i_l}^l x_{i_{l-1}}^l} \right. \\
& \left. + e^{-\sum_{j_{l-1} \in G_{\neg i_{l-1}}^{l-1}} w_{j_{l-1}i_l}^l x_{j_{l-1}}^l} + e^{-w_{i_{l-1}i_l}^l x_{i_{l-1}}^l} \right) \\
\leq & \frac{1}{2} \left| e^{w_{i_{l-1}i_l}^l x_{i_{l-1}}^l} - e^{-w_{i_{l-1}i_l}^l x_{i_{l-1}}^l} \right|.
\end{aligned}$$

And thus, we have

$$\begin{aligned}
& \left|\mathbb{E}\left[\Psi_{\boldsymbol{i}}^{\bar{l}} | \mathscr{O}_{l-1}\right]\right| \\
\leq & \left| \frac{1}{2} \int_0^{+\infty} w_{i_{l-1}i_l}^l \left| e^{w_{i_{l-1}i_l}^l x_{i_{l-1}}^l} - e^{-w_{i_{l-1}i_l}^l x_{i_{l-1}}^l} \right| \right. \\
& \left. \mu(\boldsymbol{W}_{\mathbb{I}_e \setminus \{(i_{e-1},i_e)\}}^e) \mu(w_{i_{e-1}i_e}) d\boldsymbol{W}_{\mathbb{I}_e \setminus \{(i_{e-1},i_e)\}}^e dw_{i_{e-1}i_e} \right| \\
= & \left| \int_0^{+\infty} \frac{1}{2} w_{i_{l-1}i_l}^l \left| e^{w_{i_{l-1}i_l}^l x_{i_{l-1}}^l} - e^{-w_{i_{l-1}i_l}^l x_{i_{l-1}}^l} \right| \mu(w_{i_{e-1}i_e}) dw_{i_{e-1}i_e} \right|,
\end{aligned}$$

where in the second step, $\mu(\boldsymbol{W}_{\mathbb{I}_e \setminus \{(i_{e-1},i_e)\}}^e)$ is integrated out as 1.

By the assumption that circuit stability holds; and $|e^{ax} - e^{-ax}|$ is a monotonously increasing function of $a$ regardless of $x \in \mathbb{R}$. Therefore, we further have that there exists $c \in \mathbb{R}$ such that

$$\begin{aligned}
\left|\mathbb{E}\left[\Psi_{\boldsymbol{i}}^{\bar{l}} | \mathscr{O}_{l-1}\right]\right| &\leq \int_0^{+\infty} \frac{c}{2\sqrt{n}} \left| e^{c/\sqrt{n}} - e^{-c/\sqrt{n}} \right| \mu(w_{i_{e-1}i_e}) dw_{i_{e-1}i_e} \\
&= \frac{c}{4\sqrt{n}} \left| e^{c/\sqrt{n}} - e^{-c/\sqrt{n}} \right|.
\end{aligned}$$

Then, by Taylor series expansion, we have

$$\left|\mathbb{E}\left[\Psi_{\boldsymbol{i}}^{\bar{l}} | \mathscr{O}_{l-1}\right]\right| \leq O\left(\frac{1}{2}\left(\frac{c}{\sqrt{n}}\right)^2\right). \tag{121}$$

Recall that $\mathbb{E}\left[\psi_{\boldsymbol{i}}^{\bar{l}} | \mathscr{O}_{l-1}\right]$ is the innermost integral of $\mathbb{E}\left[\psi_{\boldsymbol{i}}^{\bar{l}}\right]$. More verbosely, the relationship between the two could be captured by the following example: let $A, B$ be two random variables, and $f$ be a function, we have

$$\mathbb{E}_{\mu(A,B)}[f(A,B)] = \mathbb{E}_{\mu(B)}\left[\mathbb{E}_{\mu(A|B)}[f(A,B)|B]\right]$$

Given that the innermost integral has been enlarged as a constant, the second innermost integral becomes the innermost one, and the calculation could be performed exactly as previously done to the previous innermost integral. As a result, with

the bound given at eq. (121), we have the following recursive relationship

$$\left|\mathbb{E}\left[\Psi_{\boldsymbol{i}}^{\bar{l}}\right]\right| \leq O\left(\frac{1}{2}(\frac{c}{\sqrt{n}})^2\right)\left|\mathbb{E}\left[\psi_{\boldsymbol{i}:e}^{\bar{l}}\right]\right|.$$

That's why we intentionally refer $e$ as $l$ and let $l = e$ in the previous estimation. For integration at each layer, the cancellation induced by the weight symmetry would create a factor $O((\frac{c}{\sqrt{n}})^2)$. For a basis circuit of length $e-s$, we have

$$\left|\mathbb{E}\left[\Psi_{\boldsymbol{i}}^{\bar{l}}\right]\right| \leq O\left((\frac{c}{\sqrt{2n}})^{2(e-s)}\right).$$

□

*Proof of lemma 3.* The calculation of higher moments is similar to but slightly more sophistication than the calculation of the first moment (i.e., mean) given in the proof of lemma 8. To begin with, we write out the integral that computes the moments as in the proof of lemma 8.

$$\begin{aligned}
&\mathbb{E}\left[\prod_{\boldsymbol{i}\in G\subset G_t}\Psi_{\boldsymbol{i}}^{\bar{l}}\right] \quad (122)\\
&=\int\prod_{\boldsymbol{i}\in G\subset G_t}\psi_{\boldsymbol{i}}^{s\sim e}\prod_{l=s}^{e}\mu_l(\boldsymbol{h}_l|\mathscr{O}_{l-1})\mu(\boldsymbol{W}_l)\mu(\boldsymbol{x}_{s-1})d\mathscr{O}_l\\
&=\int\prod_{l=s}^{e}\prod_{i_l\in G_l\subset G_l^t}h_{i_l}^l w_{i_{l-1}i_l}^l\frac{1}{Z_l}e^{\boldsymbol{x}_{l-1}^T\boldsymbol{W}_l\boldsymbol{h}_l}\\
&\mu(\boldsymbol{W}_{\mathbb{I}_l\setminus\{(i_{l-1},i_l)\}}^l)\mu(w_{i_{l-1}i_l}^l)\mu(\boldsymbol{x}_{s-1})d\mathscr{O}_l,
\end{aligned}$$

where $G_t := \otimes_{l=s}^{e}[n_l]$ is a circuit-translational group, $\underline{G} \subset G_t$ is a multiset of basis circuits whose cross-moment are being computed—for example, $|G| = 2$ then eq. (122) computes the second order moment between two basis circuits—and $G_l^t$ represent the subgroup $[n_l]$.

Observe that different neuronal gates $H_{i_l}^l, i_l \in G_l$ at the same layer are conditional independent, conditioning on $\mathscr{O}_{l-1}$. Therefore, the cancellation induced by weight symmetry in the proof of lemma 8 still holds, but we need to deal with the case where basis circuits share the same neuronal gates: in this case, for example, two basis circuits could share $H_{i_l}^l$, and/or $H_{i_{l-1}}^{l-1}$; then we would have circuit weights that would not cancel out as strongly as the case where no gates are shared. More concretely, we compute the second order moments of two basis circuits to demonstrate the phenomenon in the following.

First, let $\Psi_{\boldsymbol{i}}^{\bar{l}}$ and $\Psi_{\boldsymbol{j}}^{\bar{l}}$ be two basis circuits where $i_e \neq j_e$. Then, we have the innermost integral of eq. (122) as

$$\begin{aligned}
&\mathbb{E}\left[\Psi_{\boldsymbol{i}}^{\bar{l}}\Psi_{\boldsymbol{j}}^{\bar{l}}|\mathscr{O}_{l-1}\right]\\
&=\int_{-\infty}^{-\infty} w_{i_{l-1}i_l}^l w_{j_{l-1}j_l}^l\frac{1}{Z_l}e^{\boldsymbol{x}_{l-1}^T\boldsymbol{W}_l\boldsymbol{h}_l}\\
&\mu(\boldsymbol{W}_{\mathbb{I}_l\setminus\{(i_{l-1},i_l),(j_{l-1}j_l)\}}^l)\mu(w_{i_{l-1}i_l}^l)\mu(w_{j_{l-1}j_l}^l)d\boldsymbol{W}_l\\
&=\int_{-\infty}^{-\infty} w_{i_{l-1}i_l}^l\frac{1}{Z_{i_l}^l}e^{\boldsymbol{x}_{l-1}^T\boldsymbol{w}_{i_l}^l h_{i_l}^l}\mu(\boldsymbol{w}_{i_l}^l)d\boldsymbol{w}_{i_l}^l\\
&w_{j_{l-1}j_l}^l\frac{1}{Z_{j_l}^l}e^{\boldsymbol{x}_{l-1}^T\boldsymbol{w}_{j_l}^l h_{j_l}^l}\mu(\boldsymbol{w}_{j_l}^l)d\boldsymbol{w}_{j_l}^l.
\end{aligned} \quad (123)$$

Notice that the integral factorized into two separate integrals as a result of conditional independence between $h_{i_l}^l$ and $h_{j_l}^l$. Therefore, the weight symmetry induced cancellation occurs, and we have

$$\left|\mathbb{E}\left[\Psi_{\boldsymbol{i}}^{\bar{l}}\Psi_{\boldsymbol{j}}^{\bar{l}}|\mathscr{O}_{l-1}\right]\right| \leq O\left((\frac{c}{\sqrt{2n}})^4\right).$$

That is, as a result of the weight symmetry, a decay of second order cross-moment occurs.

On the other hand, let $\Psi_{\boldsymbol{i}}^{\bar{l}}$ and $\Psi_{\boldsymbol{j}}^{\bar{l}}$ be two basis circuits where $i_e = j_e$. There are two possible subcases: $i_{e-1} = j_{e-1}$ and $i_{e-1} \neq j_{e-1}$. In the first case, we have the innermost integral of eq. (122) as

$$\begin{aligned}
&\mathbb{E}\left[\Psi_{\boldsymbol{i}}^{\bar{l}}\Psi_{\boldsymbol{j}}^{\bar{l}}|\mathscr{O}_{l-1}\right]\\
&=\int_{-\infty}^{-\infty}(w_{i_{l-1}i_l}^l)^2\frac{1}{Z_l}e^{\boldsymbol{x}_{l-1}^T\boldsymbol{W}_l\boldsymbol{h}_l}\mu(\boldsymbol{W}_{\mathbb{I}_l\setminus\{(i_{l-1},i_l)\}}^l)\mu(w_{i_{l-1}i_l}^l)d\boldsymbol{W}_l.
\end{aligned} \quad (124)$$

In this case, the cancellation from weight symmetry does not occur, and thus by the assumption of circuit stability, we would have

$$\mathbb{E}\left[\Psi_{\boldsymbol{i}}^{\bar{l}}\Psi_{\boldsymbol{j}}^{\bar{l}}|\mathscr{O}_{l-1}\right] \leq (\frac{c}{\sqrt{n}})^2.$$

In the second case, we have eq. (122) as

$$\begin{aligned}
&\mathbb{E}\left[\Psi_{\boldsymbol{i}}^{\bar{l}}\Psi_{\boldsymbol{j}}^{\bar{l}}|\mathscr{O}_{l-1}\right]\\
&=\int_{-\infty}^{-\infty} w_{i_{l-1}i_l}^l w_{j_{l-1}i_l}^l\frac{1}{Z_l}e^{\boldsymbol{x}_{l-1}^T\boldsymbol{W}_l\boldsymbol{h}_l}\\
&\mu(\boldsymbol{W}_{\mathbb{I}_l\setminus\{(i_{l-1},i_l),(j_{l-1},i_l)\}}^l)\mu(w_{i_{l-1}i_l}^l)\mu(w_{j_{l-1}i_l}^l)d\boldsymbol{W}_l.
\end{aligned} \quad (125)$$

The same as what has been done in eq. (120), the integral could

be enlarged as follows.

$$
\begin{aligned}
&\int_{-\infty}^{-\infty} w^l_{i_{l-1}i_l} w^l_{j_{l-1}i_l} \frac{1}{Z_l} e^{\boldsymbol{x}^T_{l-1}\boldsymbol{W}_l\boldsymbol{h}_l} \\
&\qquad \mu(\boldsymbol{W}^l_{\mathbb{I}_l\setminus\{(i_{l-1},i_l),(j_{l-1},i_l)\}})\mu(w^l_{i_{l-1}i_l})\mu(w^l_{j_{l-1}i_l})d\boldsymbol{W}_l \\
\leq &\int_{-\infty}^{+\infty}\int_0^{+\infty} w^l_{i_{l-1}i_l}\frac{c}{\sqrt{n}} \\
&\qquad \Bigg|\frac{1}{Z^l_{i_l}} e^{\sum_{j_{l-1}\in G^{l-1}_{\neg i_{l-1}}} w^l_{j_{l-1}i_l}x^l_{j_{l-1}}} e^{w^l_{i_{l-1}i_l}x^l_{i_{l-1}}} \\
&\qquad - \frac{1}{Z^l_{-i_l}} e^{\sum_{j_{l-1}\in G^{l-1}_{\neg i_{l-1}}} w^l_{j_{l-1}i_l}x^l_{j_{l-1}}} e^{-w^l_{i_{l-1}i_l}x^l_{i_{l-1}}}\Bigg| \\
&\qquad \mu(\boldsymbol{W}^l_{\mathbb{I}_l\setminus\{(i_{l-1},i_l),(j_{l-1},i_l)\}})\mu(w^l_{i_{l-1}i_l})d\boldsymbol{W}^l_{\mathbb{I}_l\setminus\{(i_{l-1},i_l),,(j_{l-1},i_l)\}}dw^l_{i_{l-1}i_l} \\
\leq &\int_0^{+\infty} w^l_{i_{l-1}i_l}\frac{c}{\sqrt{n}}\frac{1}{2}\left|e^{w^l_{i_{l-1}i_l}x^l_{i_{l-1}}} - e^{-w^l_{i_{l-1}i_l}x^l_{i_{l-1}}}\right| dw^l_{i_{l-1}i_l}.
\end{aligned}
$$

where in the first inequality, the integral whose range is $[0, +\infty)$ is taken against $w^l_{i_{l-1}i_l}$, and the rest of the integrals are taken over $(-\infty, +\infty)$; in the second inequality, all variables except $w^l_{i_{l-1}i_l}$ are integrated out because the measure integrates to 1. Compared with the $i_{e-1} = j_{e-1}$ case, we get one more decay factor, while compared with the $i_e \neq j_e$ case, in this case, we get one less decay factor, shown as follows.

$$
\begin{aligned}
&\int_0^{+\infty} w^l_{i_{l-1}i_l}\frac{c}{\sqrt{n}}\frac{1}{2}\left|e^{w^l_{i_{l-1}i_l}x^l_{i_{l-1}}} - e^{-w^l_{i_{l-1}i_l}x^l_{i_{l-1}}}\right| dw^l_{i_{l-1}i_l} \\
\leq &O\left(\frac{c}{\sqrt{n}}\frac{1}{2}(\frac{c}{\sqrt{n}})^2\right).
\end{aligned}
$$

Though the previous analysis is applied to the second order moment, it generalizes to high moments: for each neuronal gate $H^l_{i_l}$ exists in $G_l$ in eq. (122), as long as one of its corresponding circuit weights is of an odd power, then it would induce a decay factor $\frac{1}{2}\frac{c}{\sqrt{n}}$. More specifically, in the example of the second moment given previously, in the $i_e \neq j_e$ case, for the two neuronal gates, each circuit weight only appears once, and thus each of them induces a decay factor; in the $i_e = j_e, i_{e-1} \neq j_{e-1}$ case, there is only one neuronal gate, and both of the circuit weights are of odd power, therefore they induce one decay factor; in the $i_e = j_e, i_{e-1} = j_{e-1}$ case, the circuit weight are of even power, and thus no extra decay factor is induced.

Note that the enlargement of the innermost integral makes the second innermost integral the innermost integral, multiplied by a constant, whose value depends on whether gates are shared and the power of the corresponding circuit weights. Consequently, the calculation of the upper bound of higher moments of basis circuits reduces to count the number $p_l$ of neuronal gates at each layer $l$ that satisfy the following condition: at least one of the corresponding circuit weights of the gate is of odd power. Then, we have

$$
\left|\mathbb{E}\left[\prod_{\boldsymbol{i}\in\underline{G}\subset G_t}\Psi^{\bar{l}}_{\boldsymbol{i}}\right]\right| \leq O\left((\frac{1}{2})^{\sum_{l=s}^e p_l}(\frac{c}{\sqrt{n}})^{|\underline{G}|(e-s)+\sum_{l=s}^e p_l}\right).
$$

□

*Proof of proposition 1.* First, we have

$$
\begin{aligned}
&\left|\mathbb{E}\left[e^{i\Psi^{\bar{l}}_{\boldsymbol{i}}t}\right] - \mathbb{E}\left[e^{i\hat{\Psi}^{\bar{l}}_{\boldsymbol{i}}t}\right]\right| \\
=&\left|\mathbb{E}\left[e^{i\Psi^{\bar{l}}_{\boldsymbol{i}}t} - e^{i\hat{\Psi}^{\bar{l}}_{\boldsymbol{i}}t}\right]\right| \\
=&\left|\sum_{k=0}^{+\infty}\frac{m_{2k+1}}{(2k+1)!}(it)^{2k+1}\right|.
\end{aligned}
$$

By lemma 3, we have

$$
|m_{2k+1}| \leq O\left((\frac{1}{2})^{e-s}(\frac{c}{\sqrt{n}})^{(2k+1)(e-s)+(e-s)}\right).
$$

And thus, the moments of the normalized circuits are given as

$$
|(\frac{\sqrt{n}}{c})^{(2k+1)(e-s)}m_{2k+1}| \leq O\left((\frac{1}{2\sqrt{n}})^{e-s}\right).
$$

As a result, we have the difference between the characteristic function of the normalized circuits given as

$$
\begin{aligned}
&\left|\mathbb{E}\left[e^{i(\frac{\sqrt{n}}{c})^{e-s}\Psi^{\bar{l}}_{\boldsymbol{i}}t} - e^{i(\frac{\sqrt{n}}{c})^{e-s}\hat{\Psi}^{\bar{l}}_{\boldsymbol{i}}t}\right]\right| \\
\leq&\left|\sum_{k=0}^{+\infty}O\left((\frac{1}{2\sqrt{n}})^{e-s}\frac{(it)^{2k+1}}{(2k+1)!}\right)\right| \\
=&\left|O\left((\frac{1}{2\sqrt{n}})^{e-s}\sin(t)\right)\right|.
\end{aligned}
$$

□

### 2. *Proof of broken circuit symmetry*

We first present a corollary that characterizes the decay of the first moment to demonstrate the idea of the proof, and then present the proofs of results given in supp. B E 5.

**Corollary 8.** *Let $\Psi^{\bar{l}}_{\boldsymbol{i}}$ be a basis circuit of circuit symmetry, where $\bar{l} = (s, \ldots, e), s < e, s, e \in \mathbb{L}$, and $\boldsymbol{i} \in \otimes_{l\in\bar{l}}[n_l]$. Let $b_l$ denotes the number of "broken" neuronal gates: for gates that at initialization have at least one weight of an odd power, and no long does so at the current state of training. Then, we have*

$$
\left|\mathbb{E}\left[\Psi^{\bar{l}}_{\boldsymbol{i}}\right]\right| \leq O\left((\frac{c}{\sqrt{2n}})^{2(e-s)}(\frac{c}{2\sqrt{n}})^{-b_{\boldsymbol{i}}}\right).
$$

*Proof.* As in the case where the mean of a basis circuit of circuit symmetry is calculated, we write out the integral that computes the moments as follows,

$$
\mathbb{E}\left[\Psi^{\bar{l}}_{\boldsymbol{i}}\right] = \int \psi^{s\sim e}_{\boldsymbol{i}}\prod_{l=s}^{e}\mu_l(\boldsymbol{h}_l|\mathscr{O}_{l-1})\mu(\boldsymbol{W}_l|\mathscr{O}_{l-1})\mu(\boldsymbol{x}_{s-1})d\mathscr{O}_l. \tag{126}
$$

Note that unlike eq. (115) in the proof of lemma 8, the measure of each weight matrix $\boldsymbol{W}_l$ now depends on $\mathscr{O}_{l-1}$, the weights and neuronal gates at previous layers.

For weights $w^l_{i_{l-1}i_l}$ that are of broken weight symmetry, we calculate the upper bound of the integral as in the case where we calculate the upper bound of second order moment in eq. (124). As a result, we would lose a decay factor $\frac{c}{2\sqrt{n}}$: that is, the cancellation induced by weight symmetry does not occur for weights of broken symmetry. For weights that are still of weight symmetry, the calculation is as in the proof of lemma 8, and would give a decay factor $\frac{c}{2\sqrt{n}}$. For concreteness, we calculate the innermost integral for the two cases.

First, suppose that $w^l_{i_{l-1}i_l}, l = e$ is of broken symmetry. Then, we have

$$\left|\mathbb{E}\left[\Psi^{\bar{l}}_{\boldsymbol{i}}|\mathcal{O}_{l-1}\right]\right|$$
$$=\left|\int_{-\infty}^{+\infty} w^l_{i_{l-1}i_l}\frac{1}{Z^l_{i_l}}e^{(\boldsymbol{w}^l_{i_l})^T\boldsymbol{x}^l}\mu(\boldsymbol{W}^l_{\mathbb{I}_l\setminus\{(i_{l-1},i_l)\}}|\mathcal{O}_{l-1})\mu(w_{i_{l-1}i_l}|\mathcal{O}_{l-1})\right.$$
$$\left. d\boldsymbol{W}^l_{\mathbb{I}_l\setminus\{(i_{l-1},i_l)\}}dw_{i_{l-1}i_l}\right|$$
$$=\left|\int_{-\infty}^{+\infty}\frac{c}{\sqrt{n}}\frac{1}{Z^l_{i_l}}e^{(\boldsymbol{w}^l_{i_l})^T\boldsymbol{x}^l}\mu(\boldsymbol{W}^l_{\mathbb{I}_l\setminus\{(i_{l-1},i_l)\}}|\mathcal{O}_{l-1})\mu(w_{i_{l-1}i_l}|\mathcal{O}_{l-1})\right.$$
$$\left. d\boldsymbol{W}^l_{\mathbb{I}_l\setminus\{(i_{l-1},i_l)\}}dw_{i_{l-1}i_l}\right|$$
$$\leq\frac{c}{\sqrt{n}}.$$

Second, suppose that $w^l_{i_{l-1}i_l}, l = e$ is of weight symmetry. Then, the calculation of upper bound is the same with the calculation of $\left|\mathbb{E}\left[\psi^{\bar{l}}_{\boldsymbol{i}}|\mathcal{O}_{l-1}\right]\right|$ in lemma 8.

Consequently, recall that $b_{\boldsymbol{i}}$ is the number of weights of broken symmetry in $\Psi^{\bar{l}}_{\boldsymbol{i}}$, and we have

$$\left|\mathbb{E}\left[\Psi^{\bar{l}}_{\boldsymbol{i}}\right]\right|\leq O\left((\frac{c}{\sqrt{2n}})^{2(e-s)}(\frac{c}{2\sqrt{n}})^{-b_{\boldsymbol{i}}}\right).$$

□

*Proof of corollary 4.* For each weight of broken symmetry, the decay factor induced by the weight symmetry calculated in the proof of lemma 3 does not occur. For the detail why such a decay factor disappears, refer to the proof of corollary 8. Thus, for each distinctive neuronal gate has at least one weight of an odd power at initialization, but does not so at the current state of training, we need to remove the decaying factor. As a result, we have

$$\left|\mathbb{E}\left[\prod_{\boldsymbol{i}\in\underline{G}\subset G_t}\Psi^{\bar{l}}_{\boldsymbol{i}}\right]\right|\leq(\frac{c}{\sqrt{n}})^{|G|(e-s)}(\frac{c}{2\sqrt{n}})^{\Sigma^e_{l=s}p_l-b_l}.$$

□

*Proof of corollary 5.* We first prove the case $k = 1$. The case $k = 2$ is simple generalization of the case $k = 1$.

By lemma 2, the first derivative of a basis circuit is given as

$$\Omega^{\bar{l}\setminus\{l\}}_{\boldsymbol{i}}=\frac{\partial\Psi^{1\sim L}_{\boldsymbol{i}}}{\partial w^l_{i_li_{l-1}}}=\Psi^{1\sim l-1}_{\boldsymbol{i}:l}H^l_{i_l}\Psi^{\wedge l+1\sim L-1}_{\boldsymbol{i}_{l+1:L}}w^L_{i_{L-1}i_L}\mathcal{L}'(\cdot),$$

where we write the circuit weight out explicitly to emphasize that $\mathcal{L}'$ occupies the place that would be a neuronal gate in the previous layers.

To estimate the upper bound of $\left|\mathbb{E}\left[\prod_{\boldsymbol{i}\in\underline{G}\subset I^{\setminus\{l-1,l\}}_{i_{l-1}i_l}}\Omega^{\bar{l}\setminus\{l\}}_{\boldsymbol{i}}\right]\right|$, we still calculate the high dimensional integral. For clarity we still calculate the mean of $\Omega^{\bar{l}\setminus\{l\}}_{\boldsymbol{i}}$ as an example. We assume the weight being differentiated is not at the top layer, and it could be seen easily that the derivation could be trivially generalized to the case the differentiated weight is at the top layer. We calculate the mean of $\Omega^{\bar{l}\setminus\{l\}}_{\boldsymbol{i}}$ as follows.

$$\mathbb{E}\left[\Omega^{\bar{l}\setminus\{l\}}_{\boldsymbol{i}}\right]$$
$$=\int\omega^{\bar{l}\setminus\{l\}}_{\boldsymbol{i}}\prod_{p=s}^{e}\mu_p(\boldsymbol{h}_p|\mathcal{O}_{p-1})\mu(\boldsymbol{W}_p)\mu(\boldsymbol{x}_{s-1})d\mathcal{O}_p$$
$$=\int\mathcal{L}'w^L_{i_{L-1}i_L}\mu(\boldsymbol{W}^L)d\mathcal{O}_L \tag{127}$$
$$\prod_{q=l+1}^{L-1}h^q_{i_q}w^q_{i_{q-1}i_q}\frac{1}{Z_q}e^{\boldsymbol{x}^T_{q-1}\boldsymbol{W}_q\boldsymbol{h}_q}\mu(\boldsymbol{W}^q_{\mathbb{I}_q\setminus\{(i_{q-1},q_l)\}})\mu(w^q_{i_{q-1}i_q})d\mathcal{O}_q \tag{128}$$
$$h^l_{i_l}\frac{1}{Z_l}e^{\boldsymbol{x}^T_{l-1}\boldsymbol{W}_l\boldsymbol{h}_l}\mu(\boldsymbol{W}^l)d\mathcal{O}_l \tag{129}$$
$$\prod_{p=0}^{l-1}h^p_{i_p}w^p_{i_{p-1}i_p}\frac{1}{Z_p}e^{\boldsymbol{x}^T_{p-1}\boldsymbol{W}_p\boldsymbol{h}_p}\mu(\boldsymbol{W}^p_{\mathbb{I}_p\setminus\{(i_{p-1},i_p)\}})\mu(w^p_{i_{p-1}i_p})\mu(\boldsymbol{x},y)d\mathcal{O}_p \tag{130}$$

where eq. (127), eq. (128), eq. (129), eq. (130) are the integrals correspond to $\Psi^{1\sim l-1}_{\boldsymbol{i}:l}, H^l_{i_l}, \Psi^{\wedge l+1\sim L-1}_{\boldsymbol{i}_{l+1:L}}, w^L_{i_{L-1}i_L}\mathcal{L}'(\cdot)$, respectively. For explanation on notations, refer to the proof of lemma 8.

As in the proof of lemma 8, we first calculate the innermost integral. First, we calculate the derivative of $\mathcal{L}$ against $T\boldsymbol{x}$. Recall that

$$\mathcal{L}(y,T\boldsymbol{x})=-y\log\frac{e^{yT\boldsymbol{x}}}{1+e^{T\boldsymbol{x}}}.$$

Also recall that in supp. B D 1, we explained that the top layer neuronal gate $H_L$'s law approximates the law of label random variable $Y$. Therefore, to help relate the decay factor calculation in the intermediate layers, we rewrite the loss function as

$$\mathcal{L}(h_L,T\boldsymbol{x})=-h_L\log\frac{e^{h_LT\boldsymbol{x}}}{1+e^{T\boldsymbol{x}}}.$$

And thus the derivative $\mathcal{L}'$ is given as

$$\mathcal{L}'=-h_L\frac{1+e^{T\boldsymbol{x}}}{e^{h_LT\boldsymbol{x}}}\frac{h_LT\boldsymbol{x}e^{h_LT\boldsymbol{x}}(1+e^{T\boldsymbol{x}})-e^{h_LT\boldsymbol{x}}e^{T\boldsymbol{x}}T\boldsymbol{x}}{(1+e^{T\boldsymbol{x}})^2} \tag{131}$$
$$=-h_L\left(h_LT\boldsymbol{x}-\frac{e^{T\boldsymbol{x}}}{1+e^{T\boldsymbol{x}}}T\boldsymbol{x}\right)$$
$$=\begin{cases}T\boldsymbol{x}(\frac{e^{T\boldsymbol{x}}}{1+e^{T\boldsymbol{x}}}-1) & h_L=1\\ 0 & h_L=0.\end{cases}$$

And if $w^L_{i_{L-1}i_L}$ is of weight symmetry, the absolute of innermost integral eq. (127) is bounded by $\frac{1}{2}(c/\sqrt{n})^2$. More specifically, it satisfies

$$\begin{aligned}
&\left|\int \mathscr{L}' w^L_{i_{L-1}i_L}\mu(\boldsymbol{W}^L)d\mathscr{O}_L\right| \\
\leq &\left|\int_{-\infty}^{+\infty} T\boldsymbol{x}(\frac{1}{Z_L}e^{\boldsymbol{\alpha}^T\boldsymbol{x}_{L-1}}-1)\alpha_{i_{L-1}}\mu(\boldsymbol{\alpha}^L)d\boldsymbol{\alpha}^L\right| \\
= &\left|\int_0^{+\infty} T\boldsymbol{x}\right|\frac{1}{Z_L}e^{\sum_{j_{L-1}\in G^{L-1}_{\neg i_{L-1}}}\alpha_{j_{L-1}}\boldsymbol{x}^{L-1}_{j_{L-1}}}e^{\alpha_{i_{L-1}}x^{L-1}_{i_{L-1}}} \\
&-\frac{1}{Z_{-L}}e^{\sum_{j_{L-1}\in G^{L-1}_{\neg i_{L-1}}}\alpha_{j_{L-1}}\boldsymbol{x}^{L-1}_{j_{L-1}}}e^{-\alpha_{i_{L-1}}x^{L-1}_{i_{L-1}}}\Bigg| \\
&w^L_{i_{L-1}i_L}\mu(\boldsymbol{\alpha})d\boldsymbol{\alpha}\Bigg|
\end{aligned}$$

where in the first inequality, we replace $\boldsymbol{W}_L$ with $\boldsymbol{\alpha}$ because we study DNNs with one output neuron (cf. definition 13); the denotations of $G^{L-1}_{\neg i_{L-1}}, Z_L, Z_{-L}$ are the same with those in the proof of lemma 8; and in the first equality, the $-1$ in eq. (131) has been canceled out because the weight symmetry. Thus, we get the same equation with the case in the intermediate layers, except with an extra term $T\boldsymbol{x}$. By circuit stability assumed at definition 25, $T\boldsymbol{x}$ is bounded a constant. Given that it does not depend on depth, for consistence, we absorbed into the constant $c$. Therefore, we get the same cancellation of the integral in the intermediate layers given in supp. E B 1. As a result, we have the integral to be upper bounded by $\frac{1}{2}(c/\sqrt{n})^2$.

Furthermore, if $w^L_{i_{L-1}i_L}$ is of broken weight symmetry, similarly, we get an upper bound $(c/\sqrt{n})$ as usual. More specifically, the absolute innermost integral is upper bounded by $c/\sqrt{n}$ as integral of an intermediate layer—the absolute of the factor $\frac{e^{Tx}}{1+e^{Tx}}-1$ is less than 1, $Tx$ is less than a constant $c$ by circuit stability, and thus they could be bounded by $c/\sqrt{n}$.

Then, the integral of $\left|\mathbb{E}\left[\Omega^{\bar{l}\setminus\{l\}}_{\boldsymbol{i}}\right]\right|$ is upper bounded by a constant multiplied by an integral composed by eq. (128) eq. (129) eq. (130). Note that eq. (128) is an integral that calculates the basis circuit $\Psi^{l+1\sim L-1}_{\boldsymbol{i}_{l+1:L}}$, which we have done in the proof of corollary 8, and thus is upper bounded by $(\frac{c}{\sqrt{n}})^{(L-l-1)}(\frac{c}{2\sqrt{n}})^{\sum_{l=l+1}^{L-1}1-b_l}$. For the integral eq. (129), observe that $h^l_{i_l}\leq 1$, and thus it is bounded by 1. Lastly, eq. (130) is the integral that calculates the mean of another basis circuit $\Psi^{1\sim l-1}_{\boldsymbol{i}_{:l}}$, and is upper bounded by $(\frac{c}{\sqrt{n}})^{(l-1)}(\frac{c}{2\sqrt{n}})^{\sum_{l=0}^{l-1}1-b_l}$.

Consequently, $\left|\mathbb{E}\left[\Omega^{\bar{l}\setminus\{l\}}_{\boldsymbol{i}}\right]\right|$ is upper bounded by

$$(\frac{c}{\sqrt{n}})^{(L-1)}(\frac{c}{2\sqrt{n}})^{\sum_{l=0,l\neq l'}^{L}1-b_l}.$$

To summarize, the contribution from layer $l$ is missed compared with the decay of a basis circuit because the weight has been differentiated out. Also note that in the derivation, we have assumed that the differentiated weight is not from the top layer. When it is indeed the case, the result is the same, and the calculation is simpler: we do not even need to calculate the integral from eq. (127), and the top layer integral is calculated as the integral from eq. (129); the rest of the integrals are the same.

Therefore, the calculation of the moments of perturbation of basis circuits are the same with that of the moment of basis circuits given in the proof of corollary 4: we simply need to count the neuronal gates described in corollary 4—to clarify, the differentiated out weights of the first moment are simply neuronal gates whose corresponding weights are of zero power. And thus we have

$$\left|\mathbb{E}\left[\prod_{\boldsymbol{i}\in\underline{G}\subset\mathscr{B}_1}\delta^1\Psi^{\bar{l}}_{\boldsymbol{i}}\right]\right|\leq O\left((\frac{c}{\sqrt{n}})^{|\underline{G}|(L-1)}(\frac{c}{2\sqrt{n}})^{p_i-b_{\boldsymbol{i}}}\right),$$

The perturbation of basis circuit of order 1 is the multiplication of two basis circuits

$$\Psi^{1\sim l-1}_{\boldsymbol{i}_{:l}}H^l_{i_l}\Psi^{\wedge l+1\sim L-1}_{\boldsymbol{i}_{l+1:L}}w^L_{i_{L-1}i_L}\mathscr{L}'(\cdot).$$

Recall that by corollary 2, the perturbation of basis circuit of order 2 is simply the multiplication of three basis circuits

$$\Omega^{\bar{l}\setminus\{l,l'\}}_{\boldsymbol{i}}:=\Psi^{1\sim l-1}_{\boldsymbol{i}_{:l}}H^l_{i_l}\Psi^{\wedge l+1\sim l'-1}_{\boldsymbol{i}_{l:l'}}H^{l'}_{i_{l'}}\Psi^{\wedge l'+1\sim L-1}_{\boldsymbol{i}_{l':L}}w^L_{i_{L-1}i_L}\mathscr{L}'(\cdot).$$

Therefore, the upper bound of integrals of the differentiated-out layer, and the top layer apply to the case $k=2$ as well. Compared with the case $k=1$, one more layer is differentiated out, and thus

$$\left|\mathbb{E}\left[\prod_{\boldsymbol{i}\in\underline{G}\subset\mathscr{B}_2}\delta^2\Psi^{\bar{l}}_{\boldsymbol{i}}\right]\right|\leq O\left((\frac{c}{\sqrt{n}})^{|\underline{G}|(L-2)}(\frac{c}{2\sqrt{n}})^{p_i-b_{\boldsymbol{i}}}\right).$$

□

*Proof of theorem 1.* The theorem is a straightforward corollary of proposition 1 and corollary 4. We only need to incorporate the influence of weights of broken symmetry characterized in corollary 4 to the proof of proposition 1. Otherwise, the procedure is identical as that in the proof of proposition 1. □

*Proof of corollary 3.* The corollary is a corollary of corollary 5, as theorem 1 is a corollary of corollary 4. □

## F. REVIEW OF RESULTS FROM RANDOM MATRIX THEORY

In this section, we introduce and collect technical results from random matrix theory (RMT) used in this work. RMT [293] has been born out of the study on the nuclei of heavy atoms, where the spacings between lines in the spectrum of a heavy atom nucleus is postulated to be the same with spacings between eigenvalues of a random matrix [141]. Heavy atoms are classic many-body systems, and as discussed in section II F 4, at the assembly level, DNNs behave like many-body systems in physics, and thus it is reasonable that the mathematics developed there could be applied to the study of DNNs. More specifically, Supplement F A presents the preliminaries, and supp. F B presents the random matrix results used in this work.

## A. Preliminaries

Supplement F A 1 reviews the definition of cumulant. Supplement F A 2 gives an intuitive introduction to the Matrix Dyson Equation. Supplement F A 3 reviews the definitions of cumulant norms used in asm. 3.

### 1. Cumulants

To begin with, we review the definition of multi-set, following the notation in Erdos *et al.* [55].

**Definition 32** (Multiset)**.** *A multiset is an unordered set with possible multiple appearances of the same element. We put an underline under a normal letter (e.g.,* $\underline{\beta}$*) to denote it is a multiset.*

Notice that a normal set can also be taken as a multiset, therefore, given a multiset $\underline{\beta}$, and a set $\mathscr{B}$, $\underline{\beta} \subset \mathscr{B}$ means the underlying set of $\underline{\beta}$, i.e., the unique elements of $\underline{\beta}$ are from $\mathscr{B}$. We also follow our convention that $\boldsymbol{U}_{\underline{\beta}}$ denotes the vector consists of entries at $\underline{\beta}$. We also use a shorthand to denote cumulant between multisets. Given a multiset $\underline{\beta}$, $\kappa(\underline{\beta})$ denotes $\kappa(\beta_1, \dots, \beta_p), \beta_i \in \underline{\beta}, i = 1, \dots, p, p \in \mathbb{N}$. Given two multisets $\underline{\beta}, \underline{\gamma}$, $\kappa(\underline{\beta}, \underline{\gamma})$ denotes $\kappa(\beta_1, \dots, \beta_p, \gamma_1, \dots, \gamma_q), \beta_i \in \underline{\beta}, i = 1, \dots, p, \gamma_j \in \underline{\beta}, j = 1, \dots, q, p, q \in \mathbb{N}$.

**Definition 33** (Cumulant)**.** **Cumulants** *of* $\kappa_{\boldsymbol{m}}$ *of a random vector* $\boldsymbol{w} = (w_1, \dots, w_n)$ *are defined as the coefficients of log-characteristic function*

$$\log \mathbb{E} e^{i t^T \boldsymbol{w}} = \sum_{\boldsymbol{m}} \kappa_{\boldsymbol{m}} \frac{i \boldsymbol{t}^{\boldsymbol{m}}}{\boldsymbol{m}!}$$

*where* $\sum_{\boldsymbol{m}}$ *is the sum over all n-dimensional multi-indices* $\boldsymbol{m} := (m_1, \dots, m_n)$*, and* $\boldsymbol{t}^{\boldsymbol{m}}$ *denotes* $\prod_{i=1}^n t_{m_i}$*.*

To recall, a multi-indices is

**Definition 34** (Multi-index)**.** *a n-dimensional multi-index is a n-tuple*

$$\boldsymbol{m} = (m_1, \dots, m_n)$$

*of non-negative integers. Note that* $|\boldsymbol{m}| = \sum_{i=1}^n m_i$*, and* $\boldsymbol{m}! = \prod_{i=1}^n m_i!$*.*

Similar to the more familiar concept *moment*, cumulant is also a measure of statistical properties of random variables. Particularly, a $k$-order cumulant $\kappa$ characterizes the $k$-way correlations of a set of random variables. We have used the same symbols $\kappa$ for covariance previously. This is because the first order cumulant is just mean, whereas the second order cumulant is covariance. Compared with moments, cumulants have many properties that are conducive to theoretical analysis. For example, for a Gaussian distribution, all cumulants beyond the second order ones are zero, whereas the statement is not true for moments. And for statistical independent random variables, their cumulants are zero.

### 2. Matrix Dyson Equation

Recall that by lemma 7, the eigenspectrum of a matrix $\boldsymbol{H}$ can be obtained from its resolvent matrix $\boldsymbol{G}$. Thus, the problem converts to obtain $\boldsymbol{G}$ if we want to obtain $\mu_{\boldsymbol{H}}$. In this subsection, we give a brief introduction on the high level idea on the analysis of $\boldsymbol{G}$. This analysis is from Erdos *et al.* [55], which analyzes $\mu_{\boldsymbol{H}}$ of a symmetric random matrix with correlations through analyzing $\boldsymbol{G}$.

Given a random matrix $\boldsymbol{H}$, the resolvent $\boldsymbol{G}$ holds an identity by definition

$$\boldsymbol{H}\boldsymbol{G} = \boldsymbol{I} + z\boldsymbol{G} \tag{132}$$

Note that in the above equation $\boldsymbol{G}$ is a function $\boldsymbol{G}(\boldsymbol{H})$ of $\boldsymbol{H}$, and the equation is an equation between random matrices. The key insight is that when the entries $h_\alpha, \alpha \in \mathbb{I}$ are only strongly correlated with a minority of $\boldsymbol{H}_{\mathbb{I} \setminus \{\alpha\}}$, i.e., the existence of sparse dependency, higher order cumulants among the entries of $\boldsymbol{H}\boldsymbol{G}$ are small as $N$ grows large. Thus, eq. (132) can be turned into a solvable equation regarding $\boldsymbol{G}$ that is determined by the statistics up to the second order. This resembles the mean-field methods in physics: the higher order cumulants are considered as fluctuations, and the behaviors of the system concentrate on first order statistical behaviors.

To begin with, we give the original assumption in Erdos *et al.* [55] that is weaker than asm. 1, and has been strengthened to make the eigenspectrum symmetric in this work.

**Assumption 5** (Bounded Mean)**.** $\exists C \in \mathbb{R}, \forall N \in \mathbb{N}, ||\boldsymbol{A}|| \leq C$*, and* $||\boldsymbol{A}||$ *denotes the 2-norm induced operator norm.*

We outline the formal high level logic as follows. To begin with, because $\boldsymbol{H}, \boldsymbol{G}$ both are random matrices, taking the expectation on both sides of eq. (132), we have

$$\mathbb{E}[\boldsymbol{H}\boldsymbol{G}] = \boldsymbol{I} + z\mathbb{E}[\boldsymbol{G}]. \tag{133}$$

The left hand side of the equation could be expanded through a multivariate cumulant expansion given in Erdos *et al.* [55], and when the assumptions given in asm. 5, 2, 3, 4 held, $\mathbb{E}[\boldsymbol{H}\boldsymbol{G}]$ could be expanded as follows

$$\mathbb{E}[\boldsymbol{H}\boldsymbol{G}] = \boldsymbol{A}\mathbb{E}[\boldsymbol{G}] + \mathbb{E}[\mathscr{S}[\boldsymbol{G}]\boldsymbol{G}], \tag{134}$$

where the additional notations in the equation are defined in eq. (102), and the equation holds in the sense as follows.

The equation is established through the varnishing of high moment bound that are formulated through the following norms.

$$\begin{aligned} ||X||_p &:= (\mathbb{E}[|X|^p])^{1/p}, \\ ||\boldsymbol{A}||_p &:= \sup_{||\boldsymbol{x}||, ||\boldsymbol{y}|| \leq 1} ||\langle \boldsymbol{x}, \boldsymbol{A}\boldsymbol{y} \rangle||_p = (\sup_{||\boldsymbol{x}||, ||\boldsymbol{y}|| \leq 1} \mathbb{E}[|\langle \boldsymbol{x}, \boldsymbol{A}\boldsymbol{y} \rangle|^p])^{1/p}. \end{aligned} \tag{135}$$

Let $\boldsymbol{D}$ denote

$$\boldsymbol{D} := (\boldsymbol{H} - \boldsymbol{A})\boldsymbol{G} + \mathscr{S}[\boldsymbol{G}]\boldsymbol{G},$$

then, eq. (134) is equivalent to

$$\mathbb{E}[\boldsymbol{D}] = 0.$$

And it is proved that with a high probability, the following equation

$$||\boldsymbol{D}||_p = 0,$$

holds. It could roughly be understood as the fluctuations induced by cumulants of order higher than the second are negligible—$\mathscr{S}[\boldsymbol{G}]$ contributes to $\mathbb{E}[\boldsymbol{HG}]$ through second order cumulants, i.e., covariance. To give an intuitive explanation on the phenomenon, note that when the dependency between matrix entries are sparse, the majority of the higher order cumulants are zero. And thus as the size $N$ of the matrix grows large, the growth of the influence of higher cumulants starts to be negligible compared with $N$. This is similar to mean-field methods, where the fluctuations higher than the first order are negligible.

Note that $||\boldsymbol{D}||_p$ not only indicates the expectation of $\boldsymbol{D}$ is zero, but also its entries $|d_{ij}|^p$ is zero—we using the expansion of the expectation as an example because the expansion of higher moment norms is more complicated. And thus $\boldsymbol{D}$ is a zero matrix with a high probability, and the following equation holds with a high probability

$$\boldsymbol{HG} = \boldsymbol{AG} + \mathscr{S}[\boldsymbol{G}]\boldsymbol{G}. \tag{136}$$

Substitute the expansion of $\boldsymbol{HG}$ at eq. (136) into eq. (132), we would obtain

$$\boldsymbol{D} := \boldsymbol{I} + (z - \boldsymbol{A} + \mathscr{S}[\boldsymbol{G}])\boldsymbol{G}, \boldsymbol{D} = 0, \tag{137}$$

that holds with a high probability. The equation $\boldsymbol{D} = 0$ is the *Matrix Dyson Equation (MDE)* presented at eq. (103), which we reproduce below.

$$\boldsymbol{I} + (z - \boldsymbol{A} + \mathscr{S}[\boldsymbol{G}])\boldsymbol{G} = \boldsymbol{0}, \Im\boldsymbol{G} \succ \boldsymbol{0}, \Im z > 0 \tag{138}$$

where $\Im\boldsymbol{G} \succ 0$ means $\Im\boldsymbol{G}$ is positive definite. Furthermore, the solution to the MDE is unique (cf. lemma 9).

When a $\boldsymbol{M}$ satisfies $\boldsymbol{D} = 0$ and the previous set of assumptions are satisfied for $\boldsymbol{H}$, $\boldsymbol{M}$ could be considered as the resolvent matrix of $\boldsymbol{H}$ in the sense of the probability bound given later in lemma 9. Thus, we can obtain a class of random matrices whose eigenspectrum $\mu$ can be obtained by solving the MDE.

### 3. *Cumulant norms*

The cumulant norms proposed in Erdos *et al.* [55] are reviewed in this subsection. This subsection merely collects the definitions for readers' reference. And to clarify, the definitions might appear very complicated. However, we do not aim to elaborate all the details of the norms, for two reasons. First, as discussed previously in supp. B G 4 and B H 5, the norms only appear in asm. 3, and serve to qualitatively characterize the phenomena that certain weighted average of the cumulants are finite (cf. supp. B H 3). Thus the quantitative details are a minor concern in this work. Second, a comprehensive description of why the norms are defined exactly in such a form is not viable without reproducing much of the proof in Erdos *et al.* [55], which is a significant digression to the discussion here. And thus we refer interested readers to Erdos *et al.* [55].

To begin with, we motivate their definitions as follows. The sparse dependency among entries might induce the phenomenon that the effects of the higher order cumulants that are not zero is varnishing w.r.t. $N$, but to ensure the phenomenon, merely the smallness of the coupling set sizes is not adequate. In addition, the strength of the correlation between the entries within a coupling set needs to be not dominantly strong such that the local correlations do not dominate the global behavior of the whole matrix. To characterize this phenomenon, a proper characterization of the correlation strength is needed; that is, a norm on cumlants.

Given $k$ entries $\boldsymbol{U}_{\boldsymbol{\alpha}}$ at $\boldsymbol{\alpha} = \{\alpha_i\}_{i=1,\ldots,k}, \alpha_i \in \mathbb{I}$ of matrix $\boldsymbol{U}$, where duplication is allowed, and denote $\kappa(\alpha_1,\ldots,\alpha_k) = \kappa(u_{\alpha_1},\ldots,u_{\alpha_k})$. The cumulant norms defined in Erdos *et al.* [55] are collected below.

**Definition 35** (Cumulant Norms)**.**

$$|||\kappa||| := |||\kappa|||_{\leq R} := \max_{2\leq k\leq R} |||\kappa|||_k,$$
$$|||\kappa|||_k := |||\kappa|||_k^{av} + |||\kappa|||_k^{iso},$$

*where $|||\kappa|||_k^{av}$ and $|||\kappa|||_k^{iso}$ are defined at definition 37 and definition 36.*

To further proceed, the norms defined in eq. (140a) and eq. (141a) need some explanation on the notations. If in place of an index $\alpha \in \mathbb{J}$, a dot $(\cdot)$ is written in a scalar quantity, then the quantity is considered as a vector indexed by the coordinate at the place of the dot. For example, $\kappa(a_1\cdot, a_2b_2)$ is a vector, the $i$-th entry of which is $\kappa(a_1 i, a_2b_2)$ and therefore the inner norms in eq. (141a) indicate vector norms. In contrast, the outer norms indicate the operator norm of the matrix indexed by star $(*)$. More specifically, $||\boldsymbol{A}(*,*)||$ refers to the operator norm of the matrix with matrix elements $\boldsymbol{A}_{ij}$. Thus, $||\,||\kappa(\boldsymbol{x}*,*\cdot)||\,||$ is the operator norm $||\boldsymbol{A}||$ of the matrix $\boldsymbol{A}$ with matrix elements $\boldsymbol{A}_{ij} = ||\kappa(\boldsymbol{x}i, j\cdot)||$, where $\kappa(\boldsymbol{x}b_1, a_2b_2)$ denotes $\sum_{a_1}\kappa(a_1b_1, a_2b_2)x_{a_1}$, where $\boldsymbol{x}$ is a vector.

**Definition 36** (Average Cumulant Norms)**.**

$$|||\kappa|||_2^{av} := |||\kappa(*,*)|||, \tag{140a}$$

$$|||\kappa|||_k^{av} := N^{-2}\sum_{\alpha_1,\ldots,\alpha_k} |\kappa(\alpha_1,\ldots,\alpha_k)|, k \geq 4$$

$$|||\kappa|||_3^{av} := ||\sum_{\alpha_1}|\kappa(\alpha_1,*,*)|\,||+ \inf_{\kappa=\kappa_{dd}+\kappa_{dc}+\kappa_{cd}+\kappa_{cc}} (|||\kappa_{dd}|||_{dd} + |||\kappa_{dc}|||_{dc} + |||\kappa_{cd}|||_{cd} + |||\kappa_{cc}|||_{cc}) \tag{140b}$$

$$|||\kappa|||_{cc} = |||\kappa|||_{dd} := N^{-1}\sqrt{\sum_{b_2,a_3}(\sum_{a_2,b_3}\sum_{\alpha_1}|\kappa(\alpha_1,a_2b_2,a_3b_3)|)^2}$$

$$|||\kappa|||_{cd} := N^{-1}\sqrt{\sum_{b_3,a_1}(\sum_{a_3,b_1}\sum_{\alpha_2}|\kappa(a_1b_1,\alpha_2,a_3b_3)|)^2},$$

$$|||\kappa|||_{dc} := N^{-1}\sqrt{\sum_{b_1,a_2}(\sum_{a_1,b_2}\sum_{\alpha_3}|\kappa(a_1b_1,a_2b_2,\alpha_3)|)^2},$$

*where in eq. (140b), the infimum is taken over all decomposition of $\kappa$ in four partitions $\kappa_{dd}, \kappa_{dc}, \kappa_{cd}, \kappa_{cc}$.*

**Definition 37** (Isotropic Cumulant Norms)**.**

$$|||\kappa|||_2^{iso} := \inf_{\kappa=\kappa_d+\kappa_c} (|||\kappa_d|||_d + |||\kappa_c|||_c), \tag{141a}$$

$$|||\kappa|||_d := \sup_{||\boldsymbol{x}||\le 1} ||||\kappa(\boldsymbol{x}*,\cdot *)||||,$$

$$|||\kappa|||_c := \sup_{||\boldsymbol{x}||\le 1} ||||\kappa(\boldsymbol{x}*,*\cdot)||||$$

$$|||\kappa|||_k^{iso} := ||\sum_{\alpha_1,\ldots,\alpha_{k-2}} |\kappa(\alpha_1,\ldots,\alpha_{k-2},*,*)|||, k\ge 3,$$

*where in eq. (141a) the infimum is taken over all decomposition of $\kappa$ into the sum of $\kappa_c$ and $\kappa_d$.*

**Remark 16.** *The $|||\cdot|||_d, |||\cdot|||_c$ norms in eq. (141a) essentially define different ways that the maximal weighted average of cumulants are characterized. So are $|||\cdot|||_3^{av}$. To use $|||\cdot|||_d, |||\cdot|||_c$ as an example, the calculation in Erdos* et al. *[55] that formulates the norm $|||\cdot|||_d, |||\cdot|||_c$ to estimate the upper bound of quantities resembling the following form.*

$$\boldsymbol{K}_{kl}(\boldsymbol{x},\boldsymbol{y}) = \sum_{ij} x_i \kappa(kl,ij) y_j$$

*where $\boldsymbol{x},\boldsymbol{y} \in \mathbb{R}^n$ and $\boldsymbol{K}$ is a matrix function in $\mathbb{R}^{n\times n} \mapsto \mathbb{R}^{n\times n}$. Two ways exist to estimate the functional norm of $\boldsymbol{K}$ used in Erdos* et al. *[55]: assimilate $\boldsymbol{y}$ by summing up row-wise, i.e., $||\kappa(\boldsymbol{x}*,\cdot *)||$, and consider the summation as an entry of a matrix, then calculating the spectral norm of the resulted matrix; or, assimilate $\boldsymbol{y}$ by summing up column-wise, i.e., $||\kappa(\boldsymbol{x}*,*\cdot)||$, and consider the summation as an entry of a matrix, then calculating the spectral norm of the resulted matrix.*

**Remark 17.** *The decomposition in the eq. (141a), i.e., $\kappa = \kappa_d + \kappa_c$ and eq. (140b), i.e., $\kappa = \kappa_{dd} + \kappa_{dc} + \kappa_{cd} + \kappa_{cc}$ could be understood as a particular way to partition, or group the cumulants. We use the remark 2.8 in Erdos* et al. *[55] to explain the symmetric decomposition. Given a Wigner matrix, the second-order cumulant could be represented as*

$$\kappa(a_1b_1,a_2b_2) = \delta_{a_1,a_2}\delta_{b_1,b_2} + \delta_{a_1,b_2}\delta_{b_1,a_2}$$
$$=: \kappa_d(a_1b_1,a_2b_2) + \kappa_c(a_1b_1,a_2b_2).$$

*Thus, it could be partitioned into two groups, a direct part, and a cross part, to bound separately. Different ways to group the cumulants would lead to different norm values under $|||\cdot|||_d, |||\cdot|||_c$, and thus the partition with the smallest value is taken in the definition. The partitions are resulted from the estimation of the bound of the multivariate cumulant expansion of $\boldsymbol{HG}$ using a Feynman diagramm, which is sophisticated and we refer interested readers to Erdos* et al. *[55].*

### B. Eigenspectrum of symmetric random matrices with sparse dependency

In this section, we collect the previous results on random matrices in the literature that we use in this work. The results are collaged into lemma 9.

Given a symmetric random matrix $\boldsymbol{H}$, when the assumptions 5 2 3 4 are satisfied, we can obtain the the resolvent $\boldsymbol{G}$ of $\boldsymbol{H}$ by obtaining the solution $\boldsymbol{M}$ to the MDE, and $\boldsymbol{M}, \boldsymbol{G}$ satisfy the following properties, which are adopted from Helton *et al.* [53, theorem 2.1], Alt *et al.* [56, theorem 2.5], and Erdos *et al.* [55, theorem 2.2].

**Lemma 9.** *Suppose that assumptions 5 3 2 4 are satisfied for a given symmetric random matrix $\boldsymbol{H}$. Let $\boldsymbol{M}$ be the solution to the Matrix Dyson Equation, i.e., eq. (138), $\mu_{\boldsymbol{M}}$ the probability density function recovered from normalized trace $\frac{1}{N}tr\, \boldsymbol{M}$ through Stieljies inverse lemma 7, and $\mu_{\boldsymbol{H}}$ the empirical spectral distribution of $\boldsymbol{H}$. Then the following statements hold.*

*a) The MDE has a unique solution $\boldsymbol{M} = \boldsymbol{M}(z)$ for all $z \in \mathbb{H}$.*

*b) supp$\mu_{\boldsymbol{M}}$ is a finite union of closed intervals with nonempty interior, where supp$\mu_{\boldsymbol{M}}$ denotes the support of $\mu_{\boldsymbol{H}}$. Moreover, the nonempty interiors are called the* **bulk** *of the eigenvalue density function $\mu_{\boldsymbol{M}}$.*

*c) $\boldsymbol{M}$ is close to the resolvent $\boldsymbol{G}$ of $\boldsymbol{H}$ by the following high probability bound. For any $\gamma, \varepsilon > 0$, there exists $\delta > 0$, such that for all $D > 0$, give any $z \in \mathbb{D}_\gamma^\delta$, we have*

$$P(|tr\ (\boldsymbol{B}(\boldsymbol{G}(z) - \boldsymbol{M}(z)))| \le ||\boldsymbol{B}|| \frac{N^\varepsilon}{(1+|z|)^2 N}) \ge 1 - CN^{-D}$$

*where $\boldsymbol{B}$ is an arbitrary deterministic matrix, $N$ is the dimension of $\boldsymbol{H}$, $C > 0$ is a constant depending on $D, \varepsilon, \gamma$ and constants in asm. 5 2 3. $\varepsilon$ can be chosen small, so $||\boldsymbol{x}||||\boldsymbol{y}||N^\varepsilon/\sqrt{N\Im z}$ approaches zero as N grows. The region $\mathbb{D}_\gamma^\delta$ is roughly the region in the complex plane around the intervals that are inside the support of $\mu_{\boldsymbol{H}}$. Formally, it is defined as*

$$\mathbb{D}_\gamma^\delta := \{z \in \mathbb{H} \mid |z| \le N^{C_0}, \Im z \ge N^{-1+\gamma},$$
$$\mu_{\boldsymbol{H}}(x) + dist(x, supp\mu_{\boldsymbol{H}}) \ge N^{-\delta}\},$$

*where $\mathbb{H}$ is the complex domain, $C_0$ is a constant larger than 100.*

## G. TECHNICAL SUPPLEMENTS OF THE PLASTICITY PHASE

In this section, we supplement the technical details related to the plasticity phase of DNNs. Supplement G A presents the problem decomposition that leads to the restricted class of loss functions (cf. supp. B C 8) studied in this work. Supplement G B presents the proof of the plasticity phase theorem and its corollary.

### A. Problem decomposition

In this section, we explain why the restricted setting described in supp. B C 8 is the first sub-problem of two interdependent sub-problems that composes the general problem.

More specifically, in supp. G A 1, we present the decomposition of Hessian where the Wigner-type matrix studied in this work comes from. In supp. G A 2, we describe the speculation how the general problem, where any loss functions are allowed, could be proved. In supp. G A 3, we explain the rationale behind the restricted setting of this work.

### 1. Decomposition of Hessian

The Hessian of the risk function of DNNs, given at eq. (49), could be decomposed into the sum of a Wigner-type matrix and a Wishart-type matrix. The decomposition has been discussed in works that empirically study the degeneration, i.e., the existence of zero eigenvalues, of Hessian [205, 206]. We present the decomposition in the following.

To begin with, we calculate the Hessian of a loss function composited with a DNN (i.e., $\mathscr{L} \circ T$, where $T$ is given by eq. (48)) on one example $z := (\boldsymbol{x}, y)$. The calculation gives

$$\frac{d^2}{d\boldsymbol{\theta}^2}\mathscr{L}(T(\boldsymbol{x};\boldsymbol{\theta}),y) \tag{142}$$

$$=\mathscr{L}''(T(\boldsymbol{x};\boldsymbol{\theta}),y)\frac{d}{d\boldsymbol{\theta}}T(\boldsymbol{x};\boldsymbol{\theta})\frac{d}{d\boldsymbol{\theta}}T(\boldsymbol{x};\boldsymbol{\theta})^T \tag{143}$$

$$+\mathscr{L}'(T(\boldsymbol{x};\boldsymbol{\theta}),y)\frac{d^2}{d\boldsymbol{\theta}^2}T(\boldsymbol{x};\boldsymbol{\theta}). \tag{144}$$

The sophistication mostly lies in the derivatives of $T$, which we analyze in the following.

The derivative is the sum of a Wigner-type random matrix and a Wishart-type random matrx, as explained in the following. Notice that both the DNN $T$ and the example $z := (\boldsymbol{x}, y)$ are realizations of random elements: $T$ is a realization of the stochastic definition of DNN given at definition 13, and $z$ is a realization of the random variable $Z := (X,Y)$ described in supp. B B 3. Thus, both $\frac{d}{d\boldsymbol{\theta}}T(X;\boldsymbol{\theta})\frac{d}{d\boldsymbol{\theta}}T(X;\boldsymbol{\theta})^T$ and $\frac{d^2}{d\boldsymbol{\theta}^2}T(X;\boldsymbol{\theta})$—notice that we have replaced $\boldsymbol{x}$ with random variable $X$—are random matrices. Denote $\frac{d}{d\boldsymbol{\theta}}T(X;\boldsymbol{\theta})$ as $\boldsymbol{L}$, $\frac{d^2}{d\boldsymbol{\theta}^2}T(X;\boldsymbol{\theta})$ as $\boldsymbol{H}$, and shorten $\mathscr{L}''(T(X;\boldsymbol{\theta}),Y), \mathscr{L}'(T(X;\boldsymbol{\theta}),Y)$ as $\mathscr{L}'', \mathscr{L}'$ respectively. The Hessian of the risk function can be written as

$$\mathscr{L}''\boldsymbol{L}\boldsymbol{L}^T + \mathscr{L}'\boldsymbol{H}. \tag{145}$$

The first random matrix $\mathscr{L}''\boldsymbol{L}\boldsymbol{L}^T$ is a Wishart-type matrix. For a brief discussion on the study of this type of random matrix, interested readers may refer to Sagun *et al.* [206], and the matrix is not our focus in this work—we will explain why in supp. G A 2 shortly. The second random matrix $\mathscr{L}'\boldsymbol{H}$ is a symmetric real random matrix that is the Wigner-type matrix studied in this work, of which a brief introduction is given in supp. B H 1.

By restricting the loss functions to the class $\mathscr{L}_0$ defined at definition 15, $\mathscr{L}''\boldsymbol{L}\boldsymbol{L}^T$ is a zero matrix, and thus only $\mathscr{L}'\boldsymbol{H}$ is left. $\mathscr{L}'\boldsymbol{H}$ is Hessian matrix of DNNs that we study in this work. Next, we speculate how the general setting could be proved, and explain why such a restriction is made.

### 2. Speculation on the proof of the general setting

In this subsection, we first present the speculation on a proof of the general setting, and then discuss empirical works that support the speculation.

As presented at supp. G A 1, the Hessian could be decomposed as the sum of a Wishart-type matrix and a Wigner-type matrix. The summation between the two matrices is a specific interaction between the eigenspaces of the two matrices, and we speculate that the two eigenspaces are of statistically weak dependence such that the negative eigenvalues of the Wigner-type matrix are largely preserved. More specifically, such weak dependence might result from the sparse dependence among neuron assemblies, which is the cornerstone that induces the symmetry of the Wigner-type matrix. The Wishart-type matrix $\mathscr{L}''\boldsymbol{L}\boldsymbol{L}^T$ is the outer product of gradient $\boldsymbol{L}$, which is a vector whose components are neuron assemblies. Correspondingly, the assemblies in $\mathscr{L}''\boldsymbol{L}\boldsymbol{L}^T$ might also sparsely correlate with the ones in the Wigner-type matrix $\mathscr{L}\boldsymbol{H}$. This might induce a sparse correlation between the eigenspaces of the two matrices. Thus, as long as the correlation is sparse enough, the distortion induced by the addition of $\mathscr{L}''\boldsymbol{L}\boldsymbol{L}^T$ is weak, and the negative eigenvalues of $\mathscr{L}'\boldsymbol{H}$ would be preserved.

Previous empirical works also corroborate such a speculation. A similar speculation that $\mathscr{L}''\boldsymbol{L}\boldsymbol{L}^T$ and $\mathscr{L}'\boldsymbol{H}$ are "independent" in the sense of freeness [323] has been previously given in Pennington and Bahri [242] supported with empirical evidence from toy networks. Papyan [139] computes the eigenspectrum for large DNNs used in practice and empirically finds that the eigenspectrum of $\mathscr{L}'\boldsymbol{H}$ is symmetric w.r.t. zero, and the negative part of eigenspectrum of $\mathscr{L}'\boldsymbol{H}$ is largely preserved in the sum $\mathscr{L}''\boldsymbol{L}\boldsymbol{L}^T + \mathscr{L}'\boldsymbol{H}$—the empirical findings of Ghorbani *et al.* [140] also corroborate the results. Furthermore, Papyan [208] finds that the eigenspaces of $\mathscr{L}''\boldsymbol{L}\boldsymbol{L}^T$ concentrates on a small number of eigenvectors (compared with the huge number of dimensions of the Hessian). Such small concentrated eigenspace of $\mathscr{L}''\boldsymbol{L}\boldsymbol{L}^T$ is unlike to annihilate the eigenspace of $\mathscr{L}'\boldsymbol{H}$ with a large number of dimension.

### 3. Rationale of the restriction of the problem

The speculated phenomenon of the general setting suggests that the restricted setting in this work is the first sub-problem of two interdependent sub-problems that composes the general setting. More specifically, notice that the Wishart-type matrix is a positive definite matrix, therefore, the negative eigenvalues, that emerge from the weak interaction of the two matrices and make stationary points saddle points, could only origin from the Wigner-type matrix. Meanwhile, the class of loss functions, that make the Wishart-type matrix zero, also include practical loss functions (e.g., hinge loss) and practical setting (binary classification). Consequently, the problem in the general setting is broken down into two parts: the first is the Wigner-type matrix studied in this work, and the second is to study the interaction of the eigenspace the two matrices. Therefore, the understanding of the Wigner-type matrix is in a critical path to the understanding of the general setting, and the restricted

setting is also practically relevant. As a result, the restricted class of loss function $\mathscr{L}_0$ is studied in this work.

### B. Proof of plasticity phase theorem and its corollary

Supplement G B 1 calculates the matrix form of the Hessian of DNNs, which is the proof of lemma 6. Supplement G B 2 presents the lemmas that lead to the proof of theorem 2 and their proofs. Supplement G B 3 presents the proof of the plasticity phase theorem 2, and the proof of corollary 7.

#### 1. *Hessian of a DNN is a large random matrix*

In this section, we calculate the Hessian $\boldsymbol{H}$ of loss function $\mathscr{L}$ of class $\mathscr{L}_0$ composed upon DNNs with a single output, i.e., $\mathscr{L} \circ T(\boldsymbol{x};\boldsymbol{\theta})$, which is the proof of lemma 6. For a review of matrix calculus, the reader may refer to Magnus and Neudecker [324].

*Proof of lemma 6.* To begin with, note that for clarity, we are calculating the Hessian of the composition of a loss function $\mathscr{L}$ and DNN $T$ on a single example, whereas the empirical risk function eq. (50) is the average of the loss of all examples in the training set, or a batch. Thus, the Hessian of the risk function is the average of the matrices calculated below.

Recall that, the stochastic definition of DNN at supp. B C 6 gives the following definition of DNN

$$T(\boldsymbol{x};\boldsymbol{\theta}) = \boldsymbol{x}^T \overrightarrow{\prod}_{i=1}^{L-1} \boldsymbol{W}_i \mathrm{dg}(\boldsymbol{h}_i)\boldsymbol{\alpha},$$

where the random variables $X, \{H_i\}_{i=1,\ldots,L-1}$ are replaced with their realizations $\boldsymbol{x}, \{\boldsymbol{h}_i\}_{i=1,\ldots,L-1}$. Thus, the first partial differential of $\mathscr{L} \circ T(\boldsymbol{x};\boldsymbol{\theta})$ w.r.t. $\boldsymbol{W}_p, p \in \mathbb{L}$ is

$$\begin{aligned}
&\partial \mathscr{L}(T\boldsymbol{x},y)\\
=&\mathscr{L}'(T\boldsymbol{x},y)\boldsymbol{x}^T \overrightarrow{\prod}_{i=1}^{p-1} (\boldsymbol{W}_i \mathrm{dg}(\boldsymbol{h}_i))\,\partial \mathrm{vec}\boldsymbol{W}_p\\
&\mathrm{dg}(\boldsymbol{h}_p)\overrightarrow{\prod}_{j=p+1}^{L-1}(\boldsymbol{W}_j\mathrm{dg}(\boldsymbol{h}_j))\,\boldsymbol{\alpha}\\
=&\mathscr{L}'(T\boldsymbol{x},y)\boldsymbol{\alpha}^T \overleftarrow{\prod}_{j=p+1}^{L-1}\left(\mathrm{dg}(\boldsymbol{h}_j)\boldsymbol{W}_j^T\right)\mathrm{dg}(\boldsymbol{h}_p)\\
&\otimes \boldsymbol{x}^T \overrightarrow{\prod}_{i=1}^{p-1}(\boldsymbol{W}_i\mathrm{dg}(\boldsymbol{h}_i))\,\partial\mathrm{vec}\boldsymbol{W}_p
\end{aligned} \tag{146}$$

where $\otimes$ denotes Kronecker product.

Recall that in supp. B C 8, in the class $\mathscr{L}_0$ of functions we study, the second sub-derivative of the $\mathscr{L}$ is zero. Thus, when we take the differential w.r.t. the first order differential obtained previously, which abstractly could be written as

$$\begin{aligned}
&\frac{d^2}{d\boldsymbol{\theta}^2}\mathscr{L}(T(\boldsymbol{x};\boldsymbol{\theta}),y)\\
=&\mathscr{L}''(T(\boldsymbol{x};\boldsymbol{\theta}),y)\frac{d}{d\boldsymbol{\theta}}T(\boldsymbol{x};\boldsymbol{\theta})\frac{d}{d\boldsymbol{\theta}}T(\boldsymbol{x};\boldsymbol{\theta})^T\\
&+\mathscr{L}'(T(\boldsymbol{x};\boldsymbol{\theta}),y)\frac{d^2}{d\boldsymbol{\theta}^2}T(\boldsymbol{x};\boldsymbol{\theta}),
\end{aligned}$$

the first term on the right hand side is zero, and only the second term is left. Furthermore, because the Hessian $\boldsymbol{H}$ is symmetric, we only need to compute the block matrices by taking partial differential w.r.t. $\boldsymbol{W}_q$, where $q \in \mathbb{L}, q > p$—taking partial differential w.r.t. $\boldsymbol{W}_p$ again gives zero matrix—which we calculate as follows.

$$\begin{aligned}
&\partial^2\mathscr{L}(T\boldsymbol{x},y)\\
=&\mathscr{L}'(T\boldsymbol{x},y)\Bigg(\Bigg[\mathrm{dg}(\boldsymbol{h}_p)\overrightarrow{\prod}_{j=p+1}^{q-1}(\boldsymbol{W}_j\mathrm{dg}(\boldsymbol{h}_j))\,\partial\mathrm{vec}\boldsymbol{W}_q\\
&\mathrm{dg}(\boldsymbol{h}_q)\overrightarrow{\prod}_{k=q+1}^{L-1}(\boldsymbol{W}_k\mathrm{dg}(\boldsymbol{h}_k))\,\boldsymbol{\alpha}\Bigg]^T\\
&\otimes\boldsymbol{x}^T\overrightarrow{\prod}_{i=1}^{p-1}(\boldsymbol{W}_i\mathrm{dg}(\boldsymbol{h}_i))\Bigg)\partial\mathrm{vec}\boldsymbol{W}_p\\
=&\mathscr{L}'(T\boldsymbol{x},y)\Bigg(\Bigg[\boldsymbol{\alpha}^T\overleftarrow{\prod}_{k=q+1}^{L-1}\left(\mathrm{dg}(\boldsymbol{h}_k)\boldsymbol{W}_k^T\right)\mathrm{dg}(\boldsymbol{h}_q)\\
&\otimes\mathrm{dg}(\boldsymbol{h}_p)\overrightarrow{\prod}_{j=p+1}^{q-1}(\boldsymbol{W}_j\mathrm{dg}(\boldsymbol{h}_j))\,\partial\mathrm{vec}\boldsymbol{W}_q\Bigg]^T\\
&\otimes\boldsymbol{x}^T\overrightarrow{\prod}_{i=1}^{p-1}(\boldsymbol{W}_i\mathrm{dg}(\boldsymbol{h}_i))\Bigg)\partial\mathrm{vec}\boldsymbol{W}_p\\
=&\mathscr{L}'(T\boldsymbol{x},y)(\partial\mathrm{vec}\boldsymbol{W}_q)^T\Bigg(\mathrm{dg}(\boldsymbol{h}_q)\overrightarrow{\prod}_{k=q+1}^{L-1}(\boldsymbol{W}_k\mathrm{dg}(\boldsymbol{h}_k))\,\boldsymbol{\alpha}\\
&\otimes\overleftarrow{\prod}_{j=p+1}^{q-1}\left(\mathrm{dg}(\boldsymbol{h}_j)\boldsymbol{W}_j^T\right)\mathrm{dg}(\boldsymbol{h}_p)\\
&\otimes\boldsymbol{x}^T\overrightarrow{\prod}_{i=1}^{p-1}(\boldsymbol{W}_i\mathrm{dg}(\boldsymbol{h}_i))\Bigg)\partial\mathrm{vec}\boldsymbol{W}_p
\end{aligned}$$

Denote

$$\begin{aligned}
\boldsymbol{H}_{pq} =&\mathscr{L}'(T\boldsymbol{x},y)\mathrm{dg}(\boldsymbol{h}_q)\overrightarrow{\prod}_{k=q+1}^{L-1}(\boldsymbol{W}_k\mathrm{dg}(\boldsymbol{h}_k))\boldsymbol{\alpha}\\
&\otimes\overleftarrow{\prod}_{j=p+1}^{q-1}(\mathrm{dg}(\boldsymbol{h}_j)\boldsymbol{W}_j^T)\mathrm{dg}(\boldsymbol{h}_p)\\
&\otimes\boldsymbol{x}^T\overrightarrow{\prod}_{i=1}^{p-1}(\boldsymbol{W}_i\mathrm{dg}(\boldsymbol{h}_i))
\end{aligned} \tag{147}$$

We have the Hessian $\boldsymbol{H}$ of $\mathscr{L} \circ T(\boldsymbol{x};\boldsymbol{\theta})$ as

$$\boldsymbol{H} = \begin{bmatrix} \boldsymbol{0} & \boldsymbol{H}_{12}^T & \ldots & \boldsymbol{H}_{1L}^T \\ \boldsymbol{H}_{12} & \boldsymbol{0} & \ldots & \boldsymbol{H}_{2L}^T \\ \vdots & \ddots & \ddots & \vdots \\ \boldsymbol{H}_{1L} & \boldsymbol{H}_{2L} & \ldots & \boldsymbol{0} \end{bmatrix} \tag{148}$$

Recall that the empirical risk function eq. (50) is the empirical average of $m$ examples, and thus the Hessian of eq. (50) is the average of $m$ matrices of the above form. Rewrite $\boldsymbol{H}$ as $\boldsymbol{H}_i$ to indicate that $\boldsymbol{H}_i$ is the Hessian of $\mathscr{L} \circ T(\boldsymbol{x}_i;\boldsymbol{\theta})$. The Hessian of empirical risk function eq. (50) is given as

$$\boldsymbol{H} = \sum_{i=1}^{m}\boldsymbol{H}_i. \tag{149}$$

Also, we note that $m$is written as $b$ in the lemma.

Therefore, $\boldsymbol{H}$ is a real symmetric random matrix with correlated entries. □

## 2. Symmetry in Matrix Dyson Equation

In this section, we present and prove a theorem that states when asm. 1 holds, the eigenspectrum obtained from the solution to the MDE is symmetric w.r.t. y-axis. More specifically, we prove the stieltjes transform $m_{\mu_{\boldsymbol{H}}}(z)$ of $\mu_{\boldsymbol{H}}$ satisfies $\Im m_{\mu_{\boldsymbol{H}}}(-z^*) = \Im m_{\mu_{\boldsymbol{H}}}(z)$, where $z^*$ denote the complex conjugate of $z$.

We outline the strategy first. Because the MDE is a nonlinear operator equation, it is not possible to obtain a close-form analytic solution—to get its solution, an iterative algorithm [53] is needed. However, we do are able to obtain qualitative properties by directly analyzing the equation. As soon as we stop trying to solve the equation and turn to study the properties of the solution, the symmetry of the MDE becomes rather obvious.

**Lemma 10.** *Let $\boldsymbol{M}(z), \boldsymbol{M}'(-z^*)$ be the unique solution to the MDE at spectral parameter $z, -z^*$ defined at eq. (138), respectively. Given that $\boldsymbol{A} = \boldsymbol{0}$, we have*

$$\boldsymbol{M}' = -\boldsymbol{M}^*$$

*where $*$ means taking conjugate transpose.*

*Proof.* First, we rewrite the MDE. Note that $\mathscr{S}[\boldsymbol{G}]$ is positivity preserving, i.e., $\forall \boldsymbol{G} \succ \boldsymbol{0}, \mathscr{S}[\boldsymbol{G}] \succ \boldsymbol{0}$ by assumption 4. In addition, we have $\Im z > 0$, thus $\Im(z + \mathscr{S}[\boldsymbol{G}]) \succ \boldsymbol{0}$. Then, by Haagerup and Thorbjørnsen [325, lemma 3.1.(ii)], $z + \mathscr{S}[\boldsymbol{G}]$ is invertable. Thus, we can rewrite the MDE into the following form

$$\boldsymbol{G} = -(z + \mathscr{S}[\boldsymbol{G}])^{-1} \tag{150}$$

Suppose $\boldsymbol{M}$ is a solution to the MDE at spectral parameter $z$. The key to the proof is the fact that $\mathscr{S}[\boldsymbol{G}]$ is linear and commutes with taking conjugate, thus by replacing $\boldsymbol{M}$ with $-\boldsymbol{M}^*$, and $z$ with $-z^*$, we would get the same equation. We show it formally in the following.

First, note that $\mathscr{S}[\boldsymbol{M}]$ is a linear map of $\boldsymbol{M}$, so the we have

$$\mathscr{S}[-\boldsymbol{M}] = -\mathscr{S}[\boldsymbol{M}]$$

Also, $\mathscr{S}[\boldsymbol{M}]$ commutes with $*$, for the fact

$$\mathscr{S}[\boldsymbol{M}^*] = \mathbb{E}[\boldsymbol{U}\boldsymbol{M}^*\boldsymbol{U}] = \mathbb{E}[(\boldsymbol{U}\boldsymbol{M}\boldsymbol{U})^*] = \mathbb{E}[\boldsymbol{U}\boldsymbol{M}\boldsymbol{U}]^* = \mathscr{S}[\boldsymbol{M}]^*$$

Furthermore, $*$ commutes with taking inverse, for the fact

$$\begin{aligned} & \boldsymbol{A}\boldsymbol{A}^{-1} = \boldsymbol{I} \\ \Longrightarrow \quad & (\boldsymbol{A}\boldsymbol{A}^{-1})^* = \boldsymbol{I} \\ \Longrightarrow \quad & \boldsymbol{A}^{-1*}\boldsymbol{A}^* = \boldsymbol{I} \\ \Longrightarrow \quad & \boldsymbol{A}^{-1*} = \boldsymbol{A}^{*-1} \end{aligned}$$

By definition, the solution $\boldsymbol{M}$ satisfies the equation

$$\boldsymbol{M} = -(z + \mathscr{S}[\boldsymbol{M}])^{-1}$$

Replacing $\boldsymbol{M}$ with $-\boldsymbol{M}^*$, $z$ with $-z^*$, we have

$$\begin{aligned} & -\boldsymbol{M}^* = -(-z^* + \mathscr{S}[-\boldsymbol{M}^*])^{-1} \\ \Longrightarrow \quad & \boldsymbol{M}^* = -(z^* + \mathscr{S}[\boldsymbol{M}^*])^{-1} \\ \Longrightarrow \quad & \boldsymbol{M}^* = -(z^* + \mathscr{S}[\boldsymbol{M}]^*)^{-1} \\ \Longrightarrow \quad & \boldsymbol{M}^* = -(z + \mathscr{S}[\boldsymbol{M}])^{-1*} \\ \Longrightarrow \quad & \boldsymbol{M} = -(z + \mathscr{S}[\boldsymbol{M}])^{-1} \end{aligned}$$

After the replacement, we actually get the same equation. Thus, $-\boldsymbol{M}^*, -z^*$ also satisfy eq. (150). Because the pair also satisfies the constrains $\Im \boldsymbol{M} \succ 0, \Im z > 0$, and by lemma 9, the solution is unique, we proved the solution $\boldsymbol{M}'$ at the spectral parameter $-z^*$ is $-\boldsymbol{M}^*$. □

**Lemma 11.** *Let $\boldsymbol{H}$ be a real symmetric random matrix satisfies asm. 2 3 4, and in addition asm. 1 is satisfied. Denote the empirical spectral distribution of $\boldsymbol{H}$ by $\mu_{\boldsymbol{H}}$. Then, $\mu_{\boldsymbol{H}}$ is symmetric w.r.t. y-axis. Furthermore, non-zero eigenvalues always exist, implying $\boldsymbol{H}$ will always have negative eigenvalues.*

*Proof.* By lemma 9, the resolvent $\boldsymbol{G}$ of $\boldsymbol{H}$ is given by the unique solution to eq. (138) at spectral parameter $z$. Let the solution to eq. (138) at spectral parameter $z, -z^*$ be $\boldsymbol{M}, \boldsymbol{M}'$, By lemma 10, we have the solutions satisfies

$$\boldsymbol{M}' = -\boldsymbol{M}^*$$

By lemma 7, the ESD of $\boldsymbol{H}$ at $\Re z$ is given at

$$\mu_{\boldsymbol{H}}(\Re z) = \lim_{\Im z \to 0} \frac{1}{\pi} \Im m_{\mu_{\boldsymbol{H}}}(z)$$

Since $m_{\mu_{\boldsymbol{H}}}(z) = \frac{1}{N} \operatorname{tr} M$, we have

$$\mu_{\boldsymbol{H}}(\Re z) = \lim_{\Im z \to 0} \frac{1}{\pi} \frac{1}{N} \Im \operatorname{tr} M$$

Similarly,

$$\mu_{\boldsymbol{H}}(\Re(-z^*)) = \lim_{\Im(-z^*) \to 0} \frac{1}{\pi} \frac{1}{N} \Im \operatorname{tr} M'$$

Note that

$$\begin{aligned} & \mu_{\boldsymbol{H}}(\Re(-z^*)) = \lim_{\Im(-z^*) \to 0} \frac{1}{\pi} \frac{1}{N} \Im \operatorname{tr} M' \\ \Longrightarrow \quad & \mu_{\boldsymbol{H}}(\Re(-z^*)) = \lim_{\Im(-z^*) \to 0} \frac{1}{\pi} \frac{1}{N} \Im \operatorname{tr} (-M^*) \\ \Longrightarrow \quad & \mu_{\boldsymbol{H}}(-\Re z) = \lim_{\Im z \to 0} \frac{1}{\pi} \frac{1}{N} \Im \operatorname{tr} M \end{aligned}$$

Thus, $\mu_{\boldsymbol{H}}(\lambda), \lambda \in \mathbb{R}$ is symmetric w.r.t. $y$-axis. It follows that for all non-zero eigenvalues, half of them are negative.

By lemma 9.b, there are always bulks in supp$\mu_{\boldsymbol{H}}$, thus there are always non-zero eigenvalues. Because half of the non-zero eigenvalues are negative, it follows $\boldsymbol{H}$ always has negative eigenvalues. □

*3. Proofs of the plasticity phase*

In this section, we give the proofs of theorem 2 and corollary 7 with all the previous results.

*Proof of theorem 2.* The proof here puts together previous results. By lemma 6, the Hessian of a DNN's empirical risk is of the form given in eq. (148). Thus, $\boldsymbol{H}$ is a real symmetric random matrix. If the Hessian of a DNN satisfies asm. 1 2 3 4, by lemma 9, the eigenspectrum $\mu_{\boldsymbol{H}}$ of $\boldsymbol{H}$ is close to the solution $\boldsymbol{M}$ to the MDE defined at eq. (138), in the sense of the probability bound given in lemma 9. Therefore, in the sense of the probability bound eq. (105), and further by lemma 11, $\mu_{\boldsymbol{H}}$ is symmetric w.r.t. $y$-axis and half of its non-zero eigenvalues are negative. Furthermore, $\mu_{\boldsymbol{H}}$ is a finite union of closed intervals with nonempty interior interval. □

*Proof of corollary 7.* The analysis of the Hessian $\boldsymbol{H}$ needs to break down into two phases: (1) for all training examples, at least one example $(x, y)$ has non-zero loss value; (2) and all training samples are classified properly with zero loss values.

*a. Proof of part (a)(b) of the corollary.* We first analyze case (1). Because the loss function $\mathscr{L}$ belongs to function class $\mathscr{L}_0$, $\mathscr{L}$ is convex and is zero at its minimum. When $\mathscr{L}(x,y) \neq 0$, we have $\mathscr{L}'(x,y) \neq 0$, thus $\boldsymbol{H}$ is a nonzero random matrix. Therefore, by theorem 2, for all critical points of $R_m(T)$, $R_m(T)$'s Hessian contains nonzero eigenvalues and half of the non-zero eigenvalues of are negative. It implies all critical points are saddle points. Second, we turn to the case (2). In this case, all training examples are properly classified with the zero loss value. Considering the lower bound of $\mathscr{L}$ is zero, we have reached the global minima. Also, because all critical points in case (1) are saddle points, local minima can only be reached in case (2), implying all local minima are global minima. Thus, the part (a)(b) of the theorem is proved.

*b. Proof of part (c) the theorem.* Note that when the minima are reached, the Hessian $\boldsymbol{H}$ is degenerated into a zero matrix. Thus, each local minimum is not a traditional critical point, but a flat region, where in a local region around the minima in the parameter space, all the eigenvalues are increasingly close to zero as the parameters of the DNN approach the parameters at the infimum. We show it formally in the following. Writing a block $\boldsymbol{H}_{pq}$ (defined at eq. (147)) in the Hessian $\boldsymbol{H}_i$ of one example (defined at eq. (149)) in the form of

$$\boldsymbol{H}_{pq} = \mathscr{L}'(T\boldsymbol{x}, y)\tilde{\boldsymbol{H}}_{pq}$$

where $i$ is the index of the training examples, defined at eq. (50). Then, putting together $\tilde{\boldsymbol{H}}_{pq}$ together to form $\tilde{\boldsymbol{H}}_i$, $\boldsymbol{H}_i$ is rewritten in the form of

$$\boldsymbol{H}_i = \mathscr{L}'(T\boldsymbol{x}_i, y_i)\tilde{\boldsymbol{H}}_i$$

Then the Hessian $\boldsymbol{H}$ (defined at eq. (149)) of the risk function (defined eq. (50)) can be rewritten in the form of

$$\boldsymbol{H} = \frac{1}{m}\sum_{i=1}^{m} \mathscr{L}'(T\boldsymbol{x}_i, y_i)\tilde{\boldsymbol{H}}_i$$

Take the operator norm on the both sides, and we have

$$||\boldsymbol{H}||_2 = ||\frac{1}{m}\sum_{i=1}^{m}\mathscr{L}'(T\boldsymbol{x}_i, y_i)\tilde{\boldsymbol{H}}_i||_2 \leq \frac{1}{m}\sum_{i=1}^{m}|\mathscr{L}'(T\boldsymbol{x}_i, y_i)|\,||\tilde{\boldsymbol{H}}_i||_2.$$

Denote $\max_i\{||\tilde{\boldsymbol{H}}_i||_2\}$ as $\lambda_0$, we have

$$\begin{aligned} ||\boldsymbol{H}||_2 &\leq \frac{1}{m}\sum_{i=1}^{m}|\mathscr{L}'(T\boldsymbol{x}_i, y_i)|\lambda_0 \\ &= \mathbb{E}_m[\mathscr{L}'(TX, Y)]\lambda_0. \end{aligned}$$

The above inequality shows that, as the risk decreases, more examples will have zero loss value, consequently $\mathscr{L}' = 0$, and thus $\mathbb{E}_m[\mathscr{L}']$ will be increasingly small, so is $||\boldsymbol{H}||_2$. At the minima where all $\mathscr{L}' = 0$, the Hessian degenerates into a zero matrix. □

## H. EXPERIMENT SETTING

In this section, we describe the experiment setting of this work. All experiments are run with PyTorch [326].

### A. Experiment details of the eigenspectrum computation

The eigenspectrum is computed with the Lanczos spectrum approximation algorithms [138–140]. We use the Lanczos approximation algorithm described in Papyan [139], which is proposed by Lin *et al.* [138], and implemented contemporarily by Ghorbani *et al.* [140]. The eigenspectrum shown in fig. 8a is computed on the whole training set. When computing the extreme eigenvalues to normalize the eigenspectrum to $[-1, 1]$, we run $M_0 = 128$ iterations with $\kappa = 0.05$. $M_0$ is the iteration number and $\kappa$ is the margin percentage in `Normalization` algorithm (i.e., Algorithm 4) in Papyan [139], respectively. When approximating the eigenspectrum of Hessian with the `LanczosApproxSpec` algorithm (i.e., Algorithm 3) in Papyan [139], we use iteration number $M = 128$, the number of points $K = 1024$, and the number of starting random vector $n_{\text{vec}} = 1$.

### B. Model, training protocols and dataset

*a. Model.* We use a VGG type DNN [75] on the CIFAR10 dataset [327]. The VGG network has 12 layers and 8684684 parameters. The first 10 layers are convolution layers with $3 \times 3$ kernel size and the ReLU activation function, the last two layers are fully connected layers. The output channel number of the 12 layers are $[64, 64, 128, 128, 256, 256, 256, 512, 512, 512, 512, 1]$. Pooling layers with kernel size $[2, 2]$ are applied to convolution layer $2, 4, 7, 10$. Dropout layers are applied to convolution layer $1, 3, 5, 6, 8, 9, 10, 11$. The specification is adopted from the Zagoruyko [328]. We use a version of Batch Normalization (BN) that only subtracts mean and divides standard deviation of the current batch; that is, we do not use the extra $\gamma, \beta$ affine

transformation after normalization, and we do not maintain the global statistics of mean and standard deviation[16].

*b. Training.* No simplification is done on the VGG type DNN. We use hinge loss for binary classification. The DNN is trained with Stochastic Gradient Descent with momentum 0.9. The DNN is trained for 300 epochs. The initial learning rate is 0.05, and decayed at 200th epoch to 0.005, and at 250th epoch to 0.0005. The weights of the network are initialized with i.i.d. normal distribution with standard deviation of 0.0001. No explicit regularization is used, e.g., weight decay [11].

*c. Dataset.* We train the DNN on the CIFAR10 data. Because the DNN does binary classification, we take label 0 as the positive class, and the rest as the negative class. To create a balanced dataset, we use all images that are of label 0, and an equal number of examples of the negative class, which are randomly sampled from the rest of the classes. The training set consists of 10000 examples, and the validation set consists of 2000 examples. The sample is preprocessed to be zero-centered and of unit variance. During training, we zero-pad 4 pixels along each side of the image, and sample a $32 \times 32$ region cropped from the padded image or its horizontal flip; during testing, we use the original non-padded image.

## I. BOOTSTRAPPING METHODS IN EXPERIMENTS

In this section, we describe the bootstrapping methods that experimentally validate the assumptions from supp. B G 6 to B G 7. To clarify slightly, as a result of statistical fluctuations, when cumulants are theoretically zero, it only implies that sample cumulants are random variable of zero mean, and thus in experiments, they are not exactly zero. For example, even for random variables that are independent with each other, their sample cross-cumulants will not be exactly zero, but of some small values fluctuating around zero. Thus, when estimating the mean of Hessian entries, or coupling set size of a particular Hessian entry $u_\alpha$, i.e., the set where $u_\alpha$ correlates with, we need to weed out those fluctuations. This leads us to standard techniques in statistics, i.e, the hypothesis testing and bootstrap. Also, because this section intended to be readable without the knowledge of cumulants, we note that cumulants in this section can be interchanged with covariances, or statistics, without missing the main message.

*a. Outline.* We provide the outline of this section. 1. In supp. I A, we describe the bootstrapping method that obtains bootstrap sample of Hessian entries. From these samples, histograms and statistics of Hessian entries are estimated. 2. In supp. I B, we describe the algorithms that compute the non-zero number of cumulants for supp. B G 7. More specifically, in supp. I B 1, we give the detailed formulas for the statistics/cumulants that we are computed in supp. B G 7. Then, the algorithms are described. Overall, two steps are described. First, we need to have a hypothesis test to determine when a covariance/cumulant is large enough to not to be interpreted as random fluctuations. Second, we need to compute the number of covariances/cumulants that are large enough. The first step is achieved through *percentile bootstrapping* to compute a confidence interval that for cumulants are outside the confidence interval, they are considered to be cross-cumulants of correlated random variables. The second step is achieved by computing the sample mean and standard errors of the number of cumulants that cross the threshold of bootstrap samples. We describe the overall procedure, which is the step two, in supp. I B 2. Then, step one is described in supp. I B 3. 3. We give the details on the parameters used in the experiments in supp. I C.

We also note that the bootstrapping and hypothesis testing techniques used in this section are not the only choice, and they aim to qualitatively validate the theoretical characterizations—this methodological aspect has been explained in section II D 3.

### A. Boostrapping sampling of Hessian entries

The experiments from supp. B G 6 to B G 7 require estimation of the histograms and the statistics of Hessian entries. We estimate the statistics with bootstrapping methods. The details for estimating different statistics are described later in this section, and here, we describe the procedure that we use to obtain bootstrap samples of Hessian entries.

Notice that the random matrix under study is very large. For the Hessian $\boldsymbol{H}$ of the VGG network that we investigate experimentally, it is roughly of the dimension $10^7 \times 10^7$. It is both computationally intractable in term of time and space to compute all the Hessian entries directly. Thus, we use bootstrapping methods to estimate the desired statistics.

More specifically, we draw $B$ independent bootstrap samples $\boldsymbol{H}_b$ of dimension $N_b \times N_b$ and of size $m$ by sampling submatrices from $\boldsymbol{H}$, where $N_b < N$ (actually, $N_b \ll N$ due to computational constraints). Each $\boldsymbol{H}_b$ is a submatrix sampled from the Hessian $\boldsymbol{H}$ by randomly taking $\boldsymbol{H}_{\boldsymbol{i}\boldsymbol{j}^T}$ $\boldsymbol{i}, \boldsymbol{j} \in [\mathbb{N}]^{N_b}$ ($\boldsymbol{i}, \boldsymbol{j}$ are random vectors whose elements are natural numbers less than or equal to $N$). The values of these parameters are given in supp. I C 1.

Some issues need clarifying. First, it is remarkable that such bootstrap sampling that samples a submatrix could provide a stable estimation with low variance, considering it only samples a small population from $N \sim 10^7$ possible dimensions. In retrospect, the phenomenon is reasonable because the circuit symmetry in DNNs is like translation symmetry in physics, and the behaviors of different assemblies (i.e., Hessian entries) are symmetric/repetitive. Therefore, The statistically stable results of the current small-scale experiments qualitatively validate the theoretical characterizations. Second, each bootstrap sample of the $B$ samples has a sample of size $m$, where $m$ is the number of examples in the dataset: each example in the sample would

[16] As explained in supp. C B, BN improves optimization by normalizing the gradient norm to maintain the network at the edge of chaos, and the affine transformation, and the global statistics are not critical for the plasticity phase that enable to DNNs reach zero risk global minima. The affine transformation increases the hypothesis space (i.e., the expressiveness) of DNNs, and the global statistics could be understood as a form of regularization. The inclusion of these extra features improves the test performance, but such complications are undesirable in the current iteration of theoretical study.

realize a Hessian matrix, therefore, for a dataset of size $m$, $m$ independent example of Hessian matrices are realized for each bootstrap sample. Thus, even with a small $B$ value, we have a reasonable sample size. Third, we calculate batch-averaged Hessian/examples because the network is trained by batches of examples instead of individual examples, and further details can be found in supp. I C.

## B. Bootstrapping estimation of non-zero cumulants

### 1. Statistics/cumulants in the experiments

In supp. B G 7, we experimentally study the cumulants among Hessian entries. We give the formulate for the statistics/cumulants we study in the experiment in this section. We compute the cumulants of Hessian entries $u_\alpha, \alpha \in \mathbb{I}$ that are up to the fourth order. We want to rule out the influence of the scale of $u_\alpha$, thus we compute the normalized cumulants by dividing the cumulants by their standard errors. This is a standard practice in statistics, and the normalized cumulants are respectively known as *Pearson correlation coefficients*, *skewness*, and *excess kurtosis*, corresponding respectively to normalized second cumulant, third cumulant and fourth cumulant. We review them in this subsection considering that their high dimensional definitions may not be widely familiar.

Let $\{\boldsymbol{U}_i\}_{i=1,\ldots,m}$ be a sample of size $m$, where each $\boldsymbol{U}_i$ be a random matrix of dimension $N$ with mean subtracted. Let $\sigma(\alpha), \alpha \in \mathbb{I}$ denotes the standard deviation of $u_\alpha$

*a. Normalized second cumulant, or Pearson correlation coefficients.* The second cumulant is the covariance, as mentioned previously, which might be the most standard definition in statistics. It is denoted as $\kappa_2(\alpha, \beta), \alpha, \beta \in \mathbb{I}$, and calculated as

$$\kappa_2(\alpha, \beta) = \frac{1}{m} \sum_{i=1}^{m} u_\alpha^i u_\beta^i.$$

We normalize it by standard deviation, and obtain the normalized second cumulant, or Pearson correlation coefficients.

$$\frac{\kappa_2(\alpha, \beta)}{\sigma(\alpha)\sigma(\beta)} = \frac{1}{n} \sum_{i=1}^{n} \frac{u_\alpha^i u_\beta^i}{\sigma(\alpha)\sigma(\beta)}.$$

*b. Normalized third cumulant, or skewness.* The third cumulant is denoted as $\kappa_3(\alpha, \beta, \gamma), \alpha, \beta, \gamma \in \mathbb{I}$ and calculated as

$$\kappa_3(\alpha, \beta, \gamma) = \frac{1}{m} \sum_{i=1}^{n} u_\alpha^i u_\beta^i u_\gamma^i.$$

Its normalized version is called skewness, and is also a standard definition to measure the asymmetry of a probability distribution. Again, it is obtained by normalizing the third cumulant.

$$\frac{\kappa_3(\alpha, \beta, \gamma)}{\sigma(\alpha)\sigma(\beta)\sigma(\gamma)} = \frac{1}{m} \sum_{i=1}^{m} \frac{u_\alpha^i u_\beta^i u_\gamma^i}{\sigma(\alpha)\sigma(\beta)\sigma(\gamma)}.$$

*c. Normalized fourth cumulant, or excess kurtosis.* The fourth cumulant is write as $\kappa_4(\alpha_1, \alpha_2, \alpha_3, \alpha_4)$ $\alpha_1, \alpha_2, \alpha_3, \alpha_4 \in \mathbb{I}$ and calculated as

$$\begin{aligned}&\kappa_4(\alpha_1, \alpha_2, \alpha_3, \alpha_4)\\ =&\frac{1}{m} \sum_{i=1}^{m} u_{\alpha_1}^i u_{\alpha_2}^i u_{\alpha_3}^i u_{\alpha_4}^i - \kappa_2(\alpha_1, \alpha_2)\kappa_2(\alpha_3, \alpha_4)\\ &- \kappa_2(\alpha_1, \alpha_3)\kappa_2(\alpha_2, \alpha_4) - \kappa_2(\alpha_1, \alpha_4)\kappa_2(\alpha_2, \alpha_3).\end{aligned}$$

Its normalized version is called excess kurtosis, though it might mostly used in one dimensional setting, and is also a standard definition to measure extreme outlines of a probability distribution. Again, it is obtained by normalizing as follows

$$\frac{\kappa_4(\alpha_1, \alpha_2, \alpha_3, \alpha_4)}{\sigma(\alpha_1)\sigma(\alpha_2)\sigma(\alpha_3)\sigma(\alpha_4)}.$$

We also note that high dimensional setting, to characterize the overall behavior of the distribution, varied definitions of kurtosis have been proposed e.g., Koizumi *et al.* [329]. Considering that we only concern with individual cumulants between random variables here, we have adopted the classic definition of normalized kurtosis by Mardia [330].

### 2. Bootstrapping estimation of non-zero cumulants

In this subsection, we describe the procedure that we use to estimate the non-zero cumulants among Hessian entries; that is, the number of cumulants that are from entries that are statistical dependent. We use the bootstrapping estimation of the correlation coefficients as an example to describe the procedure. The estimation of skewness and excess kurtosis is similar, except that in step 2 in algorithm 3, instead of counting non-zero correlation coefficients, we count the non-zero skewness, or excess kurtosis.

In the following, we describe the bootstrapping procedure to estimate the sample mean and standard errors of the non-zero number of correlation coefficients. Recall that $\boldsymbol{H}$ denotes Hessian and $\boldsymbol{H}$ is of dimension $N \times N$.

**Algorithm 3** Bootstrap estimation of non-zero cumulants

1. Obtain a bootstrap sample of Hessian entries according to the procedure described in supp. I A.
2. Compute the correlation coefficients matrix of vec$\boldsymbol{H}_b$.
3. Estimate the number $s_0$ of non-zero correlation coefficients for each bootstrap sample. This is done through bootstrap hypothesis testing described in supp. I B 3.
4. Compute the mean of the number by $s_0/N_b^2$.
5. Estimate the standard deviation of the sample mean of $s_0/N_b^2$.

To clarify, we have not described how to compute the number of non-zero coefficients in algorithm 3, and it is done intentionally. The computation involves a bootstrap hypothesis test, and is described in supp. I B 3. Also the values of the parameters used in experiments is given in supp. I C.

*3. Hypothesis test on correlations through bootstrapping*

We describe how the number of non-zero cumulants in algorithm 3 is computed in this section. We take the value of cumulants as the test statistics. Instead of identifying a confidence interval corresponding to a specific P value, we identify a confidence interval by maintaining that the coupling set size of the assumed distribution of the null hypothesis should be at least two magnitude smaller than the expected given by asm. 2. We explain the strategy using correlation coefficients as follows.

To begin with, we discuss the rationale behind such a hypothesis test. The aim of the test is to test the pair-wise statistical dependence between Hessian entries—thus we do not need sophisticated multivariate hypothesis test [329, 331]. The perform a hypothesis test, a reference is needed to compare with. Given that no information is available on the distribution of Hessian entries, and as discussed in section II D 3, the theoretical characterizations are to qualitatively characterize the behaviors of DNNs in experiments, we utilize the classic choice that the two random variables are of mutually independent Gaussian distribution as the null hypothesis.

In the following, we use the hypothesis testing on the correlation coefficient as an example to describe the null hypothesis. We use a null hypothesis that characterizes the lack of correlations between random variables. That is, if the null hypothesis holds, no correlations are considered to exist between the random variables in the test. We first state our null hypothesis.

*a. Null hypothesis.* Let $X,Y$ be two random variables, and $\{x_i\}_{i=1,\ldots,m}, \{y_i\}_{i=1,\ldots,m}$ be a sample of $X,Y$ respectively. The correlation coefficient $\kappa_2(X,Y)/(\sigma(X)\sigma(Y))$ of $X,Y$ is indistinguishable to the correlation coefficient of two random variables that are of independent normal distributions.

To obtain the analytical expressions of the probability distribution involved in such a null hypothesis is difficult. More specifically, the sample covariance is $\frac{1}{m}\sum_{i=1}^{m} X_i Y_i$, where $X_i, Y_i, i = 1,\ldots,m$ are i.i.d. copies of $X,Y$. When $X,Y$ are of independent normal distributions, the distribution of the sample covariance is a sum of the product of two normal distributions. The calculation of such a distribution still remains an open problem that is being tackled with varied approaches, e.g., Oliveira and Seijas-Macias [332] and Ware and Lad [333]. We use bootstrapping method to avoid actually calculating the distribution. We use the percentile bootstrap to identify a threshold that would give an adequate P value to the above null hypothesis. To proceed, we briefly explain the procedure of percentile bootstrapping.

*b. Percentile bootstrap.* The method constructs a two-sided equal-tailed $1-\alpha$ confidence interval for an estimate $\hat{\theta}$ from an empirical distribution by following the below steps.

**Algorithm 4** Percentile bootstrapping

1. Draw $B$ independent bootstrap samples $z_b$ of size $m$ from the distribution.
2. Estimate the parameter $\theta$ for each bootstrap sample: $\hat{\theta}_b$.
3. Order the bootstrap replications of $\hat{\theta}$ such that $\hat{\theta}_1 \leq \ldots \leq \hat{\theta}_B$. The upper and lower bound confidence bounds are the $B(1-\alpha/2)$th and the $B\alpha/2$th ordered elements, respectively. The estimated $(1-\alpha)$ confidence interval of $\hat{\theta}$ is $[\hat{\theta}_{B\alpha/2}, \hat{\theta}_{B(1-\alpha/2)}]$.

*c. Monte Carlo percentile bootstrap.* Notice that in algorithm 3 for a Hessian $\boldsymbol{H}$ of dimension $N \times N$, even if we bootstrap sample only a $N_b \times N_b$ submatrix of it, there would be $N_b^2(N_b^2-1)$ number of correlation coefficients, which would be a rather large number. In the experiment, it is of the magnitude of $10^8$. Thus, the normal $\alpha$ at the magnitude of 1% is not small enough, since it would pass $10^6$ number of correlation coefficients as non-zero even if entries of $\boldsymbol{H}$ are of Gaussian distribution. Thus, to prevent random fluctuations from interfering the count of non-zero coefficients, we work backward to choose a $\alpha$ through *Monte Carlo simulation* such that in the simulation, $\alpha N_b^2(N_b^2-1)$ would be two orders of magnitude smaller than the estimated number, i.e., the coupling set size $N_b^{1/2}$ in the case of non-zero correlation coefficients.

The procedure to identify a confidence interval through Monte Carlo percentile bootstrapping is given as follows in algorithm 5, and see algorithm 3 for further notations. To choose $\alpha$, $N_b^2(N_b^2-1)$ number of correlation coefficients of independent normally distributed random variables are sampled. The procedure identifies a threshold of the test statistics beyond which the null hypothesis is considered not held. In this case, we do not need to know the exact $\alpha$ of the confidence interval, while at the same time, it is ensured that any correlation coefficients that pass that threshold should be considered to have come from two correlated random variables. Also note that we directly use the $\kappa_2$ to denote correlation coefficient since the samples are of unit variance.

**Algorithm 5** Monte Carlo percentile bootstrapping

1. Draw $B$ independent bootstrap sample $\boldsymbol{H}_0$ of dimension $N_b \times N_b$ and of size $m$, where vec$\boldsymbol{H}_0$ is of multivariate normal distribution $\mathcal{N}(\boldsymbol{0}, \boldsymbol{I})$.
2. Compute the correlation coefficients matrix of vec$\boldsymbol{H}_0$.
3. Identify a threshold $\theta$ of the test statistics, i.e., correlation coefficients, such that the number $s_0 := \sum_{\alpha,\beta\in[N_b]\times[N_b],\alpha\neq\beta} \mathbf{1}_{|\kappa_2(h^0_\alpha, h^0_\beta)|>\theta}$ is least two orders of magnitudes smaller than $N_b^2 N_b^{1/2}$. Notice that $N_b^{1/2}$ is the upper bound of coupling set size in asm. 2, and since each Hessian entry can have up to $N_b^{1/2}$ correlated entries, overall there are $N_b^2 N_b^{1/2}$ of them.
4. Estimate the standard error of $s_0$.

*d. Algorithms for higher order statistics.* The procedure to identify the thresholds for higher order statistics are similar,

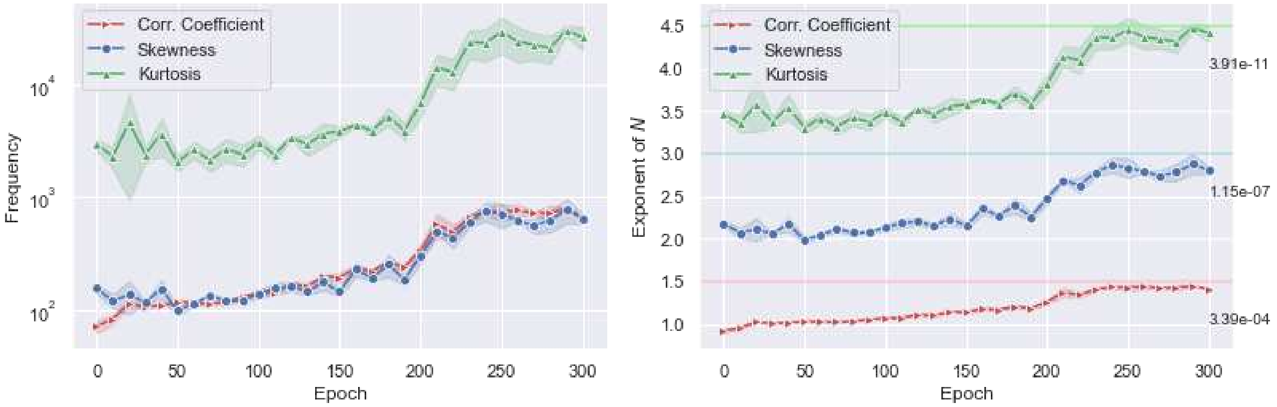


(a) (b)

FIG. 14. Comparison between raw non-zero number of statistics and the number in term of exponent of Hessian dimension $N$. Figure (a) gives the number in absolute value, and (b) in term of exponent of Hessian dimension $N$. More detailed explanations of the figure is given in the caption of fig. 7c.

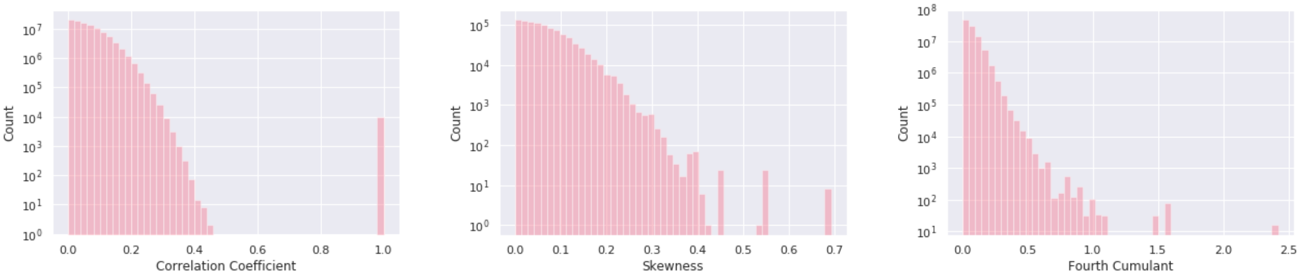


(a) (b) (c)

FIG. 15. Histograms of correlation coefficients, skewness, and excess kurtoses (fourth cumulants) generated in algorithm 5.

and we describe the difference in the following.

1. **Strategy for skewness.** In step 3 of algorithm 5, we identify a threshold $\theta$ of the test statistics, i.e., skewness, such that the number $s_0 := \sum_{\alpha,\beta,\gamma\in[N_b]\times[N_b]\times[N_b]} \mathbf{1}_{|\kappa_3(h^0_\alpha,h^0_\beta,h^0_\gamma)|>\theta}$ is least two magnitudes smaller than $N_b^2 N_b^1$.

2. **Strategy for excess kurtosis.** In step 3 of algorithm 5, we identify a threshold $\theta$ of the test statistics, i.e., excess kurtosis, such that the number $s_0 := \sum_{\alpha_1,\alpha_2,\alpha_3,\alpha_4\in[N_b]\times[N_b]\times[N_b]\times[N_b]} \mathbf{1}_{|\kappa_4(h^0_{\alpha_1},h^0_{\alpha_2},h^0_{\alpha_3},h^0_{\alpha_4})|>\theta}$ is least two magnitudes smaller than $N_b^2 N_b^{3/2}$.

### C. Experiment settings

In this section, we describe the details of parameters in experiments.

#### 1. *Parameters in the bootstrapping algorithms*

The sample size $m$ in supp. I A is $157 = \lceil 10000/64 \rceil$, thus so is the $m$ in algorithm 5. This is because the random matrix in question is the empirical mean of Hessian of individual examples. Thus, each batch of examples in the dataset contributes to an example of a sample. The dataset has 10000 examples, and the batch size is 64. Overall, there are 157 examples in a sample.

When estimate the distribution of Hessian entries' mean, the dimension $N_b$ in supp. I A is 100. So is the dimension $N_b$ of the sampled submatrix $\boldsymbol{H}_b$ when computing the number of non-zero correlation coefficients in algorithm 3. The standard errors of the mean (of the non-zero correlation coefficients) is small enough to give a stable estimation of the exponent of $N_b$, as shown in fig. 14a, where the standard errors are shown as the transparent region around the curve.

When estimating the skewness and excess kurtosis in algorithm 3, the dimension of $N_b$ of $\boldsymbol{H}_b$ is 10. This is because the number of cumulants grows by $N_b^2$ with the order of the cumulants, and we need to reduce the computational time and memory requirement in the experiments on them. Also note

TABLE I. Thresholds of test statistics that if exceeded, the null hypotheses that the random variables are uncorrelated are rejected, and the statistics are considered non-zero. The non-zero number are the numbers of non-zero test statistics under null hypotheses.

| **Test Statistics** | Correlation Coefficients | Skewness | Excess Kurtosis |
|---|---|---|---|
| **Non-zero Number** $s_0$ | $16.00 \pm 6.69$ | $67.80 \pm 73.74$ | $2.20 \pm 2.32$ |
| **Threshold** | 0.4 | 0.4 | 1 |

that despite such a small number, there are $10^6$ skewness values and $10^8$ kurtosis values. The results are also stable, as shown in standard errors in fig. 14a.

Hessian is sampled at the beginning of the DNN training, and every 10 epoch with $B = 3$. To clarify, normally in bootstrapping methods, $B$ is asked to be of order $10^2 \sim 10^3$, however, we use $B = 3$ in the experiments. This is because first, as a random matrix, an example of $\boldsymbol{H}_b$ is an ensemble of $10^8$ of random variables itself, and its behavior is statistically stable; second, each bootstrap sample has to $m$ examples, where $m$ is the size of the dataset—these clarifications have been made in cf. supp. I A. The results are shown in fig. 14a. Note that the coupling set size is given in term of $N^{1/2}$, thus, we translate the non-zero number in term of exponent of $N$, which is fig. 7c in supp. B G 7, and is also reproduced in fig. 14b. The two plots, the raw number and the converted exponents, is given side by side in fig. 14.

### 2. *Thresholds of hypothesis tests*

*a. Threshold for correlation coefficients.* To identify a threshold for correlation coefficients, we sample one $\boldsymbol{H}_0$ described in algorithm 5, and plot its the distribution, as shown in fig. 15a. $N_b^2 N_b^{1/2}$ in this case is $10^5$, which makes the acceptable threshold $0.3 \sim 0.4$, and we pick 0.4 as the null hypothesis threshold. Then, we run algorithm 5 with $B = 5$ and obtain the mean and standard errors of $s_0$ in table I.

*b. Threshold for skewness.* To identify a threshold for skewness, we sample one $\boldsymbol{H}_0$ described in algorithm 5, and plot its the distribution, as shown in fig. 15b. $N_b^2 N_b^1$ in this case is $10^3$, which makes the acceptable threshold around 0.4, and we pick 0.4 as the null hypothesis threshold. Then, we run algorithm 5 with $B = 5$ and obtain the mean and standard errors of $s_0$ in table I.

*c. Threshold for kurtoses.* To identify a threshold for kurtoses, we sample one $\boldsymbol{H}_0$ described in algorithm 5, and plot its the distribution, as shown in fig. 15c. $N_b^2 N_b^{3/2}$ in this case is $10^3\sqrt{10}$, which makes the acceptable threshold around 1, and we pick 1 as the null hypothesis threshold. Then, we run algorithm 5 with $B = 5$ and obtain the mean and standard errors of $s_0$ in table I.
